# Supplementary material for: Optimizing Provenance Computations
Source: arXiv:1701.05513 source file (2017-01-19)
Supplement: Supplementary file 1 [file appendix-cbo.tex]

%%% Local Variables:
%%% mode: latex
%%% TeX-master: "2016-prov-optimizer"
%%% End:

\section{Cost-based Optimization Framework}
\label{sec:cost-based-optim}

%%%%%%%%%%%%%%%%%%%%%%%%%%%%%%%%%%%%%%%%
\begin{Theorem}
Let $q$ be input query. Algorithm~\ref{alg:cbo-skeleton} iterates over all plans that can be created for the given choice points.
\end{Theorem}
%%%%%%%%%%%%%%%%%%%%%%%%%%%%%%%%%%%%%%%%

\begin{proof}
Consider the plan space tree for a query $q$. In the first iteration choice $0$ will be taken for all choice points. Thus, the left-most leaf node will be visited in this iteration. It remains to be shown that if the first $n$ iterations have explored the $n$ leftmost leaf nodes of the plan space tree, that the next iteration will visit the $n+1^{th}$ leaf node. Let $l_i$ denote the $i^{th}$ leaf node and $a$ be the lowest common ancestor of node $l_n$ and $l_{n+1}$. WLOG assume that $l_{n}$ is reached by taking choice $i$ at node $a$. For every node on the path from the $i^{th}$ child of $a$ to $l_n$, the last choice is taken. This is true, because otherwise $a$ cannot be the LCA of $l_n$ and $l_{n+1}$. Assume that somewhere on the path the $j^{th}$ child is chosen at a node with more than $j$ children. Then we can create a new path by moving to $j+1^{th}$ child and taking arbitrary decisions (e.g., always chose the leftmost child) to reach a leaf node that lies between nodes $l_{n}$ and $l_{n+1}$ which contradicts the fact that $l_{n+1}$ is the $n+1^{th}$ leaf node. Using the same argument we know that $l_{n+1}$ is reached by choosing the $i+1^{th}$ child at $a$ and then continuously moving to the leftmost child until $l_{n+1}$ is reached. Since every $a$ is the last node in the path where we have not chosen the last available option, Algorithm~\ref{alg:gen-next-option} will create $p_{next}$ as the prefix of $p_{cur}$ (the path to $l_{n}$) which ends in the $i+1^{th}$ child of $a$. During the next iteration Algorithm~\ref{alg:callback} will take the first choice (leftmost child) for every choice after reaching that child which as shown above leads to $l_{n+1}$.
\end{proof}

%%%%%%%%%%%%%%%%%%%%%%%%%%%%%%%%%%%%%%%%
\begin{Theorem}
Assume a fixed search space traversal order (function $\Call{generateNextChoice}{}$). If the stopping condition $T_{opt} > T_{exe}$ is applied and the duration of an iteration is limited by a constant factor $<< T_{exe}$ then the resulting algorithm is 2-competitive with respect to the optimization goal of minimizing $T_{opt} > T_{exe}$.
\end{Theorem}
%%%%%%%%%%%%%%%%%%%%%%%%%%%%%%%%%%%%%%%%
