# Supplementary material for: Optimizing Provenance Computations
Source: arXiv:1701.05513 source file (2017-01-19)
Supplement: Supplementary file 2 [file appendix-experiments2.tex]

%%%%%%%%%%%%%%%%%%%%%%%%%%%%%%%%%%%%%%%%%%%%%%%%%%%%%%%%%%%%
\section{Experiments}\label{sec:experiments}

%%%%%%%%%%%%%%%%%%%%%%%%%%%%%%%%%%%%%%%%%%%%%%%%%%%%%%%%%%%%
\begin{figure*}[t]
%%%%%%%%%%%%%%%%%%%%
  \begin{minipage}[b]{0.49\linewidth}
  \includegraphics[width=1\linewidth,trim=0 70pt 0 70pt, clip]{figs/experiments_v1/simpleAgg_10MB.pdf}
  \caption{Simple Aggregation Queries - 10MB}
  \label{fig:simple-agg-10MB}  
  \end{minipage}
%%%%%%%%%%%%%%%%%%%%
  \begin{minipage}[b]{0.49\linewidth}
  \includegraphics[width=1\linewidth,trim=0 70pt 0 70pt, clip]{figs/experiments_v1/simpleAgg_100MB.pdf}
  \caption{Simple Aggregation Queries - 100MB}
  \label{fig:simple-agg-100MB}
  \end{minipage}

%%%%%%%%%%%%%%%%%%%%
  \begin{minipage}[b]{0.49\linewidth}
  \includegraphics[width=1\linewidth,trim=0 70pt 0 120pt, clip]{figs/experiments_v1/simpleAgg_1GB.pdf}
  \caption{Simple Aggregation Queries - 1GB}
  \label{fig:simple-agg-1GB}  
  \end{minipage}
%%%%%%%%%%%%%%%%%%%%
  \begin{minipage}[b]{0.49\linewidth}
  \includegraphics[width=1\linewidth,trim=0 70pt 0 120pt, clip]{figs/experiments_v1/simpleAgg_10GB.pdf}
  \caption{Simple Aggregation Queries - 10GB}
  \label{fig:simple-agg-10GB}
  \end{minipage}

\end{figure*}
%%%%%%%%%%%%%%%%%%%%%%%%%%%%%%%%%%%%%%%%%%%%%%%%%%%%%%%%%%%%

%%%%%%%%%%%%%%%%%%%%%%%%%%%%%%%%%%%%%%%%%%%%%%%%%%%%%%%%%%%%
\begin{figure*}[t]
%%%%%%%%%%%%%%%%%%%%
  \begin{minipage}[b]{0.49\linewidth}
  \includegraphics[width=1\linewidth,trim=0 70pt 0 70pt, clip]{figs/experiments_v1/tpch_10MB.pdf}
  \caption{TPCH Queries - 10MB}
  \label{fig:tpch-10MB}  
  \end{minipage}
%%%%%%%%%%%%%%%%%%%%
  \begin{minipage}[b]{0.49\linewidth}
  \includegraphics[width=1\linewidth,trim=0 70pt 0 70pt, clip]{figs/experiments_v1/tpch_100MB.pdf}
  \caption{TPCH Queries - 100MB}
  \label{fig:tpch-100MB}
  \end{minipage}

%%%%%%%%%%%%%%%%%%%%
  \begin{minipage}[b]{0.49\linewidth}
  \includegraphics[width=1\linewidth,trim=0 70pt 0 70pt, clip]{figs/experiments_v1/tpch_1GB.pdf}
  \caption{TPCH Queries - 1GB}
  \label{fig:tpch-1GB}  
  \end{minipage}
%%%%%%%%%%%%%%%%%%%%
  \begin{minipage}[b]{0.49\linewidth}
  \includegraphics[width=1\linewidth,trim=0 70pt 0 70pt, clip]{figs/experiments_v1/tpch_10GB.pdf}
  \caption{TPCH Queries - 10GB}
  \label{fig:tpch-10GB}
  \end{minipage}

\end{figure*}
%%%%%%%%%%%%%%%%%%%%%%%%%%%%%%%%%%%%%%%%%%%%%%%%%%%%%%%%%%%%

Our experimental evaluation focuses on 1) evaluating the effectiveness of cost-based optimization in choosing the best alternative and 2) study the performance improvements gained by using provenance specific transformation rules.
3) estimate the runtime overhead paid to provenance specific transformation rules and cost-based optimization. All experiments were executed on the machine with the configuration shown in Table~\ref{tab:exp-config}.

%%%%%%%%%%%%%%%%%%%%
\begin{table}[t]
\centering
  \begin{tabular}{|c|c|} \hline 
  \rowcolor[gray]{.9}  Name & type \\ \hline 
  CPUs & 2 $\times$ AMD Opteron 4238 (12 cores)   \\ \hline
  RAM & 128 GB   \\ \hline
  Hardware & 4 $\times$ 1TB 7.2K HDs   \\ \hline
  \end{tabular}
\caption{Experiment configuration}
\label{tab:exp-config}
\end{table}
\subsection{Experimental results}

\subsection{Placeholder}
\begin{itemize}
\item
\item
\item
\end{itemize}

%%%%%%%%%%%%%%%%%%%%%%%%%%%%%%%%%%%%%%%%%%%%%%%%%%%%%%%%%%%%
%\subsection{Cost-based Optimization}
\subsection{Compare methods}

To evaluate how effectiveness of  our cost-based optimizer in choosing the lowest cost alternative and how our provenance specific transformation rules improve the performance, for cost-based optimizaion, we compared the performance of queries generated by the cost-based optimizer against queries generated by taking a predetermined choice;
for provenance specific transformation rules, we we compared the performance of queries which activated these rules with deactivated these rules.
We focus on following aspects: 1) selecting the window (\textbf{\textit{Window}}) or join (\textbf{\textit{Join}}) based implementation of rewriting an aggregation operator for provenance computation in GProM. 
2) Selecting to use a selection (\textbf{\textit{Prefliter}}) or a join (\textbf{\textit{HistJoin}}) method to compute parital of provenance. \textbf{\textit{Cost}} is our cost-based optimization which choose the cheapest method between (\textbf{\textit{Window}}) and (\textbf{\textit{Join}})
or between (\textbf{\textit{Prefliter}}) and (\textbf{\textit{HistJoin}}). For each one, we activate provenance specific transformation rules (\textbf{\textit{Opt}}) and deactivate provenance specific transformation rules (\textbf{\textit{NoOpt}}) respectively.  
%We also compared \textit{joinNoOpt} and \textit{windowNoOpt} which are deactivating the heuristic optimizaion respectively.  
% Here we use both simple aggregation queries and TPC-H queries - both executed over TPC-H datasets. 

%For this experiment we use a workload of provenance computations
%for transactions.

\subsection{Dataset and workload}

\subsubsection{Dataset}

\noindent\textbf{TPC-H datasets: }
%For this experiment we use TPC-H datasets. 
The TPC-H benchmark is a standard decision support benchmark. It is consists of suite of bussiness oriented ad-hoc queries and concurrent data modifications.
The queries and the data populating the database have been chosen to have broad industry-wide relevance while maintaining a sufficient degree of ease of implement. This benchmark has following features: large volumes of data and 
queries with a high degree of complexity. We generated TPC-H benchmark conformant datasets of size 10MB, 100MB, 1GB, and 10GB. 

\noindent\textbf{Synthetic datasets: }
We use a relation with five numeric attributes. Values for these attributes are chosen from a uniform distribution.
We created variants $R10K$, $R100K$, and $R1000K$ with 10K, 100K, 1M tuples. For
$R1000K$ we created different sizes of transactional history (this affects
performance, because the database has too store this history to enable time
travel that we need to compute provenance for transactions). Parameter $H0$
indicates no significant history whereas $H1000$ represent $1000\%$ history
which amounts to 10M tuples in case of relation $R1000K$. 
 
\subsubsection{Workloads}

We use three workloads in this experiment. 

\noindent\textbf{Simple aggregation queries: }
This set of queries consist solely of aggregation operations. An aggregation test query consists of \textit{agg} aggregation operations. Each
aggregation operates on the result of its child aggregation. The leaf operation accesses the TCP-H table part. Every aggregation groups the input on a range of primary key attribute values.
The ranges are chosen so that each operation performs approximately the same number of aggregation function computations. This is achieved by grouping on the primary key attribute divided by
$numGrp =  \sqrt[agg]{|part|} $. 

\noindent\textbf{TPC-H queries: }
The TPC-H benchmark consists of 22 queries. We have selected 11 representative queries to evaluate the optimizer over more complex, realistic queries.

\noindent\textbf{Transactions: }
We consider provenance computations for transactions that consist solely of
update statements.  We vary the following parameters: $U$ is the number of
updates per transaction, e.g., $U10$ is a transaction with 10 updates. $T$ is
the number tuples affected by each update. Unless stated otherwise, we use
$T1$. The tuples to be updated are selected randomly using the primary key of
the relation.  All transactions were executed under isolation
level~\texttt{SERIALIZABLE}. Note that these transaction do not exhibit the
exponential expression growth problem we mentioned in the introduction. Our
optimizations can deal with such queries. However, we wanted to compare to the
performance of unoptimized provenance computations which would not be possible
for such queries.

%%%%%%%%%%%%%%%%%%%%%%%%%%%%%%%%%%%%%%%%%%%%%%%%%%%%%%%%%%%%
\subsection{Results}
\noindent\textbf{Simple Aggregation Queries. } 
Fig.~\ref{fig:simple-agg-10MB} to \ref{fig:simple-agg-10GB} shows the results of computing the provenance of the simple aggregation queries use datasets of size 10MB up to 10GB.
We vary the number of aggregation in the query and compare runtime of the \textit{Cost+Opt}, \textit{Window+Opt}, \textit{Join+Opt}, \textit{Window+NoOpt} and \textit{Join+NoOpt} methods mentioned above.

%%%%%%%%%%%%%%%%%%%%%%%%%%%%%%%%%%%%%%%%%%%%%%%%%%%%%%%%%%%%
%\subsubsection{Simple Aggregation Queries}
%\label{sec:simple-aggr-quer}

%In this experiment we computed the provenance of the simple aggregation queries use datasets of size 10MB up to 10GB. 
%We vary the number of aggregation in the query and compare runtime of the \textit{cost}, \textit{window}, \textit{join}, \textit{windowNoOpt} and \textit{joinNoOpt} methods mentioned above.
%The results of this experiment are shown in Fig.~\ref{fig:simple-agg-10MB} to \ref{fig:simple-agg-10GB} (the data set sizes are 10MB, 100MB, 1GB, and 10GB).  

In these figures, the vertical axis shows the running time in seconds (logarithmic scale) whereas the horizontal axis indicates the number of aggregations ranging from 1 to 10.
We can see in every figures \textit{Window+Opt} always get better performance than \textit{Window} which shows our provenance specific transformation rules always improve the performance.
For join method, except for Fig.~\ref{fig:simple-agg-10MB} and~\ref{fig:simple-agg-10GB}, the \textit{Join} get better performance than \textit{Join+Opt}. This is because the database 
generated the different plans and materialized the subquery of \textit{Join}. For cost-based method, we can see that window method consistently outperforms the join based method whatever with \textit{Opt} or with \textit{NoOpt} except for only with 1 or 2 aggregations. The window based method is several orders of magnitude faster than the join method for larger database sizes and higher number of aggregations.
Consistently, the cost-based method was able to recognize the best method showing the same performance as the window method. We manually confirmed that in all these cases the query generated by the cost-based optimizer was the same as the one produced by the window method. 
%  From the result, cost-based does what we supposed to do, the window based one
% is much better than join based one, the cost-based optimizer makes the correct choice.
In some cases we can see the cost-based optimizer was able to generate a query that is cheaper than both the join and window method, for example in figure~\ref{fig:simple-agg-10GB}.
This is because there are several level aggregations in the query, the cost-based method can always choose the best method in different levels.
In any figures, our \textit{Cost+Opt} always outperform than any other method.
Note that in Fig.~\ref{fig:simple-agg-10GB}, we do not report results for the join based methods of Q6 and \textit{Window+NoOpt} and \textit{Join+NoOpt} methods, because they not finish in reasonable time (we interrupted queries running longer than 1 hour).

%%%%%%%%%%%%%%%%%%%%%%%%%%%%%%%%%%%%%%%%%%%%%%%%%%%%%%%%%%%%
%\subsubsection{TPC-H Queries}
%\label{sec:simple-aggr-quer}
\noindent\textbf{TPCH-H Queries. } 
We use the TPC-H queries to determine whether the results for the simple aggregation queries translate to more complex queries and to confirm that there are workloads on which choosing the join method is beneficial.
The results are shown in Fig.~\ref{fig:tpch-10MB} to \ref{fig:tpch-10GB}. 

In these figures, the vertical axis still shows the running time whereas the horizontal axis indicates the query. % Here we use the queries Q1, Q5, Q10 and Q13, because some problem of the Q5 and Q10, we only shows the result of Q1 and Q13 which already give the nice results.
Depending on the datasize and query, there are cases where the join method is superior and others where the window method is superior. Also the runtime difference between these methods are less noticeable presenting a challenge for our cost-based optimizer. 
Nonetheless, the cost-based method has the same cost as the cheapest method in almost all cases. We also can see that \textit{Opt} outperform than \textit{NoOpt} expecially in large size dataset.

%However, there are two exceptions.
%For query Q13 in Fig.~\ref{fig:tpch-1GB}, the cost-based methods shows a runtime that lies between the join method and window method. This is because the database cost model is not perfect, which mislead our optimizer to think that a combination of both methods (each applied for one of the two aggregations in the query) would have the lowest cost. The second exception is query Q13 over the 10GB instance (Fig.~\ref{fig:tpch-10GB}). Here the cost-based optimizer was able to generate a query that is cheaper than both the join and window method. Here the optimizer has chosen to apply the join method for one aggregation in query Q13 and the window for the other. In summary, this experiment demonstrates that our optimizer outperform purely heuristic choices and is able to determine which choice is better even if the performance differences are not as significant as in the previous experiment.
%For query Q5 in Fig.~\ref{fig:tpch-1GB}, here the cost-based optimizer was able to generate a query that is cheaper than both the join and window method. Here the optimizer has chosen to apply the join method for one aggregation in query Q5 and the window for the other. In summary, this experiment demonstrates that our optimizer outperform purely heuristic choices and is able to determine which choice is better even if the performance differences are not as significant as in the previous experiment.

%%%%%%%%%%%%%%%%%%%%%%%%%%%%%%%%%%%%%%%%%%%%%%%%%%%%%%%%%%%%
\begin{figure*}[t]

%%%%%%%%%%%%%%%%%%%%
  \begin{minipage}[b]{0.49\linewidth}
  \includegraphics[width=1\linewidth,trim=0 70pt 0 10pt, clip]{figs/experiments_v1/uSizeNumTupUpdated_overhead.pdf}
  \caption{Transaction Overhead: Updates/Transaction in Different Update Size}
  \label{fig:Transaction Overhead: Updates/Transaction and History Size}  
  \end{minipage}
%%%%%%%%%%%%%%%%%%%%
  \begin{minipage}[b]{0.49\linewidth}
  \includegraphics[width=1\linewidth,trim=0 70pt 0 10pt, clip]{figs/experiments_v1/uSizeNumTupUpdated.pdf}
  \caption{Updates/Transaction and History Size}
  \label{fig:Updates/Transaction-and-History-Size}  
  \end{minipage}
\end{figure*}
%%%%%%%%%%%%%%%%%%%%%%%%%%%%%%%%%%%%%%%%%%%%%%%%%%%%%%%%%%%%

%%%%%%%%%%%%%%%%%%%%%%%%%%%%%%%%%%%%%%%%%%%%%%%%%%%%%%%%%%%%
\begin{figure}[t]
  \centering
  \includegraphics[width=1\linewidth,trim=0 70pt 0 70pt, clip]{figs/experiments_v1/numTupUpdated.pdf}
  \caption{Number Updates/Transaction}
  \label{fig:Number-Updates/Transaction}
\end{figure}
 %%%%%%%%%%%%%%%%%%%%%%%%%%%%%%%%%%%%%%%%%%%%%%%%%%%%%%%%%%%%
 
 %%%%%%%%%%%%%%%%%%%%%%%%%%%%%%%%%%%%%%%%%%%%%%%%%%%%%%%%%%%%
\begin{figure}[t]
  \centering
  \includegraphics[width=1\linewidth,trim=0 70pt 0 70pt, clip]{figs/experiments_v1/numTupUpdated_overhead.pdf}
  \caption{Transaction Overhead: Number Updates/Transaction}
  \label{fig:Transaction Overhead Number Updates/Transaction}
\end{figure}
 %%%%%%%%%%%%%%%%%%%%%%%%%%%%%%%%%%%%%%%%%%%%%%%%%%%%%%%%%%%%

 %%%%%%%%%%%%%%%%%%%%%%%%%%%%%%%%%%%%%%%%%%%%%%%%%%%%%%%%%%%%
\begin{figure*}[t]

%%%%%%%%%%%%%%%%%%%%
  \begin{minipage}[b]{0.49\linewidth}
  \includegraphics[width=1\linewidth,trim=0 70pt 0 30pt, clip]{figs/experiments_v1/tpch_overhead.pdf}
  \caption{TPCH Overhead}
  \label{fig:TPCH Overhead}  
  \end{minipage}
%%%%%%%%%%%%%%%%%%%%
  \begin{minipage}[b]{0.49\linewidth}
  \includegraphics[width=1\linewidth,trim=0 70pt 0 120pt, clip]{figs/experiments_v1/simpleAgg_overhead.pdf}
  \caption{SimpleAgg Overhead}
  \label{fig:SimpleAgg Overhead}  
  \end{minipage}
\end{figure*}
%%%%%%%%%%%%%%%%%%%%%%%%%%%%%%%%%%%%%%%%%%%%%%%%%%%%%%%%%%%%

 %%%%%%%%%%%%%%%%%%%%%%%%%%%%%%%%%%%%%%%%%%%%%%%%%%%%%%%%%%%%
\begin{figure}[t]

%%%%%%%%%%%%%%%%%%%%
  \begin{minipage}[b]{0.49\linewidth}
  \includegraphics[width=1\linewidth,trim=0 70pt 0 70pt, clip]{figs/experiments_v1/TPCH_average1.pdf}
  \caption{TPCH factor 1}
  \label{fig:TPCH-factor1}  
  \end{minipage}
%%%%%%%%%%%%%%%%%%%%
  \begin{minipage}[b]{0.49\linewidth}
  \includegraphics[width=1\linewidth,trim=0 70pt 0 70pt, clip]{figs/experiments_v1/TPCH_average2.pdf}
  \caption{TPCH factor 2}
  \label{fig:TPCH-factor2}  
  \end{minipage}
\end{figure}
\noindent\textbf{Transactions. }
We compute the provenance of transactions varying the number of updates per
transaction ($U1$, $U10$, $U100$, and $U1000$) and the size of the database
($R10K$, $R100K$, and $R1000K$).  
%We use \textit{NoOpt} which denotes non
%heursitic optimization, \textit{OptNoMerg} which denotes applying all heuristic
%optimization rules without the merge rule and \textit{Opt} which denotes
%applying all heuristic optimizaion rules.

%Fig.~\ref{fig:No Significant History} shows the runtime of these provenance
%computations over relations with no significant history ($H0$).  We scale
%linearly in $R$ and $U$. By reducing the amount of data to be processed by the
%reenactment query, without applying the merge rule, \textit{OptNoMerge} can
%always get better performance than \textit{NoOpt}.  By applying projection
%merging, the performance of \textit{Opt} is largely improved compared to
%\textit{OptNoMerge}.

Fig.~\ref{fig:Updates/Transaction-and-History-Size} shows results for varying the
number of updates ($U1$, $U10$, $U100$ and $U1000$) using \textit{R1000K-H10}, \textit{R1000K-H100} and \textit{R1000K-H1000}.
Compared with \textit{NoOpt}, \textit{FilterUpdated+Opt}, \textit{MergingHistJoin+Opt} and \textit{Cost+Opt}, this optimization is
more effective for larger transactions, because the reenactment queries for such
transactions are increasingly complex. The \textit{FilterUpdated+Opt} configuration shows get better performance than
\textit{NoOpt} and with increasement of the number of the updates per transaction the performance was improved largely. 
\textit{Cost+Opt} always choose similar with the \textit{FilterUpdated+Opt}.
%Except for the last one $U1000$, \textit{Opt} get better performance
%than \textit{OptNoMerge}. The \textit{NoOpt} configuration did not finish without a 1 hour threshold.

Fig.~\ref{fig:Number-Updates/Transaction} shows results for $U50$
where each update modifies 10, 100, 1000 or 10000 tuples from relation
\textit{R1000K-H1000}. As evident from Fig.~\ref{fig:Number-Updates/Transaction}, the runtime is not significantly affected when increasing the number
of affected tuples per update. 
%Heuristic optimization always shows better performance than
%heuristic optimization without merging projections.  And active heuristic optimizaion without
%merge can always get better than applying no optimization. Merging projections is quite effective for large number of updates per transactions.
The \textit{FilterUpdated+Opt} get better performance than
\textit{NoOpt} and \textit{Cost+Opt} always choose the same with the \textit{FilterUpdated+Opt}.

Fig.~\ref{fig:TPCH-factor1}, we sum the minimum runtime of each TPCH queries and use this value as a standard. Then we get the sum runtime of window, join and cost respectively and divide by the standard.
We can see the Cost-based method always get better performance compared with the most costly one and sometimes get better performance than both, for example in 10GB size.

Fig.~\ref{fig:TPCH-factor2}, we use the minimum runtime of each TPCH queries as the standard and get the relative value of each method compared to the standard for every TPCH queries. Then we sum the relative value of each method and divide by the number of the TPCH queries.
We can see the Cost-based method always get better performance compared with the most costly one and sometimes get better performance than both, for example in 1GB and 10GB size.

\subsection{Overhead}
In Fig.~\ref{fig:TPCH Overhead} and Fig.~\ref{fig:SimpleAgg Overhead}, we use TPCH queries and simple aggregations to test the overhead of our optimizer.

In Fig.~\ref{fig:TPCH Overhead}, we compared window method, join method and cost-based method all with \textit{Opt} and with \textit{NoOpt}. We can see \textit{Opt} cost a little bit than \textit{NoOpt} in 
every methods \textit{Window}, \textit{Join} and \textit{Cost}. The \textit{Cost} cost more than other methods because its time spend on the estimating the running time. The cost-based method generated many plans and each plan needs database to give an estimated cost. 

In Fig.~\ref{fig:SimpleAgg Overhead}, we compared activating provenance specific transformation rules with deactivating provenance specific transformation rules, we also compared them with cost-based
method which with \textit{Opt} and with \textit{NoOpt}. The \textit{Opt} cost a little bit than \textit{NoOpt} in every methods. With the increasement of the number of aggregations,
the running time of \textit{Cost} gradually increased which because more layers of aggregations means we can generate more plans.

Fig.~\ref{fig:Transaction Overhead Number Updates/Transaction} and~\ref{fig:Transaction Overhead: Updates/Transaction and History Size} shows the overhead of transactions which shows in Fig.~\ref{fig:Number-Updates/Transaction} and~\ref{fig:Updates/Transaction-and-History-Size} respectively. \textit{Opt} still cost a little bit than \textit{NoOpt} and \textit{Cost} cost than other methods. 
\subsection{Summary}

Our experiments confirm the effectiveness of our provenance specific transformation rules and cost-based optimization methods - often improving performance by several orders of magnitude. Our cost-based optimizer was able to pick the right alternatives in almost all cases.

%%% Local Variables:
%%% mode: latex
%%% TeX-master: "2016-prov-optimizer"
%%% End:
