# Supplementary material for: Optimizing Provenance Computations
Source: arXiv:1701.05513 source file (2017-01-19)
Supplement: Supplementary file 3 [file appendix-heuristic.tex]

\section*{Outdated heuristic}
\label{sec:outdated-heuristic}

 %%%%%%%%%%%%%%%%%%%%%%%%%%%%%%%%%%%%%%%%
\begin{figure}[t]
\centering

\subfloat[]{
\begin{tikzpicture}
[op/.style={anchor=south west},
conn/.style={-}]

%\node[op] (p) at (0,3) {$\projection_{name,pid,price}$};
%\node[op] (s) at (0,2) {$\selection_{sName='Merdiers'}$};
\node[op] (s) at (0,3) {$\projection_{id,price,P(sName)}$};

\node[op] (j) at (0,2) {$\join_{id=itemId}$};
\node[op] (p) at (-2,1.6) {$(id,price,sName,itemId,P(sName))$};

\node (r1) at (-1.6,0.6) {$items$};
\node (r2) at (2.5,0.6) {$\projection_{sName,itemId,sName \to P(sName)}$};

\node (r3) at (2.5,-0.6) {$sales$};
%\draw[conn] ($(p.south west) + (2.5mm,0)$) to ($(s.north west) + (2.5mm,0)$);
\draw[conn] ($(s.south west) + (2.5mm,0)$) to ($(j.north west) + (2.5mm,0)$);

\draw[conn] ($(p.south west) + (23mm,0)$) to (r1);
\draw[conn] ($(p.south west) + (23mm,0)$) to (r2);

\draw[conn] ($(r2.south west) + (25mm,0)$) to (r3);
\end{tikzpicture}}

\subfloat[]{
\begin{tikzpicture}
[op/.style={anchor=south west},
conn/.style={-}]

%\node[op] (p) at (0,3) {$\projection_{name,pid,price}$};
%\node[op] (s) at (0,2) {$\selection_{sName='Merdiers'}$};
\node[op] (q) at (0,4) {$\projection_{id,price,P(sName)}$};

\node[op] (s) at (0,3) {$\projection_{id,price,sName \to P(sName)}$};

\node[op] (j) at (0,2) {$\join_{id=itemId}$};
\node[op] (p) at (-1.5,1.6) {$(id,price,sName,itemId)$};

\node (r1) at (-1.6,0.6) {$items$};
\node (r2) at (2.5,0.6) {$\projection_{sName,itemId}$};

\node (r3) at (2.5,-0.6) {$sales$};
%\draw[conn] ($(p.south west) + (2.5mm,0)$) to ($(s.north west) + (2.5mm,0)$);
\draw[conn] ($(q.south west) + (2.5mm,0)$) to ($(s.north west) + (2.5mm,0)$);
\draw[conn] ($(s.south west) + (2.5mm,0)$) to ($(j.north west) + (2.5mm,0)$);

\draw[conn] ($(p.south west) + (18mm,0)$) to (r1);
\draw[conn] ($(p.south west) + (18mm,0)$) to (r2);

\draw[conn] ($(r2.south west) + (12mm,0)$) to (r3);
\end{tikzpicture}}

\caption{Example: pulling up provenance projections}
\label{fig:ex-pullup-provenance-projections}
\end{figure}
%%%%%%%%%%%%%%%%%%%%%%%%%%%%%%%%%%%%%%%%

%%%%%%%%%%%%%%%%%%%%%%%%%%%%%%%%%%%%%%%%
\begin{table}
\centering
  \begin{tabular}{|c|c|} \hline 
\rowcolor[gray]{.9}  Operator $\Diamond$ & Inferred property for the input(s) of $\Diamond$\\ \hline 
  R & $\{\{a\}\mid a \in \schema{R} \}$ \\ \hline
%%%%%%%%%%
  $\selection_ {(\theta_{i} \wedge ... \wedge \theta_{n})}(R)$ & ${\cal E}^* (EC(R) \cup 
\{\{a,b\}\mid \exists i: \theta_{i}=(a=b) \} 
)$

% $\{x \cup \{c\}\mid \theta_{i}=(a=c)(i \in 1:n), \exists x \in EC(R), a \in x \wedge c \in Const \} $ \\
%                                                                & $\cup~\{x \cup y\mid \theta_{i}=(a=c)(i \in 1:n), \exists x,y \in EC(R), a \in x \wedge c \in y \wedge c \in Variable\}$ \\  
%                                                                & $\cup~\{x\mid \theta_{i}=(a=c)(i \in 1:n), \exists x \in EC(R), \not \exists a \in x  \} $
    \\ \hline                                                          
%%%%%%%%%%
%  $\projection_ {a_{1} \rightarrow b_{1},...,a_{n} \rightarrow b_{n}}(R)$ & ${\cal E}^* ( \{\{ b_i, b_j \} \mid \exists E \in EC(R) \wedge a_i \in E \wedge a_j \in E \} \union \{\{b_i\} | i \in \{1,\ldots,n\}\})$ \\
  %& maybe: \\
  %& ${\cal E}^* ( \{\{ b_i, b_j \} \mid \exists x \in EC(R) \wedge a_i \in x \wedge a_j \in x \wedge a_i \neq a_j\}$ \\
  %& $\cup~ \{ \{b_i\} \mid x \in EC(R) \wedge a_i \in x \wedge a_j \in x~ \wedge \not\exists a_j : a_i = a_j  \})$ \\
% $\{ (x - \{a_ {i}\} \cup \{b_ {i}\}) \cap SCH(\projection_ {a_{1} \rightarrow b_{1},...,a_{n} \rightarrow b_{n}(R)})\mid \exists x \in EC(R), a_i \in x, i \in 1:n \} $
%  \hline
%%%%%%%%%%
  $R \join_ {a=b} S$ & ${\cal E}^*(EC(R) \cup EC(S) \cup \{\{a,b\}\}) $\\ \hline
% $ \{x \cup y\mid \exists x \in EC(R), \exists y \in EC(S), a \in x \wedge b \in y \}$\\
%                      & $ \cup~(EC(R)-x)~\cup~(EC(S)-y) $ \\ \hline
%%%%%%%%%%
%  $R \crossprod S$ & $EC(R) \cup EC(S) $\\ \hline
%%%%%%%%%%
  $ _{b_{1},...,b_{n}} \aggregation _{F(a)}(R) $ & $\{  \{ b_{1},...,b_{n} \} \cap E \mid E \in EC(R) \}  \cup \{\{F(a)\}\} $ \\ \hline
  $\duplicate(R)$ & $EC(R) $ \\ \hline
%%%%%%%%%%
%  $R \union S$ & ${\cal E}^* (\{ E \cap E' \mid E \in EC(R) \wedge E' \in EC(S)[\schema{S}/\schema{R}] \}$
  % $R \union S$ & $\{ x \cap y\mid \exists x \in EC(R),\exists y \in EC'(S), EC'(S) = EC(S)_{(b_{i} \rightarrow a_{i})}, i \in \{1,...,n\} \}$
 %   \\ \hline
%%%%%%%%%%
%  $R \intersection S$ & ${\cal E}^*( EC(R) \union EC(S)[\schema{S}/\schema{R}])$ \\ \hline
% EC_{temp} = \{ x \cup y\mid x \in EC(R), y \in EC'(S),EC'(S)=EC(S)_{(b_{i} \rightarrow a_{i})}, x \cap y \neq \emptyset, i \in \{1,...,n\} \}$ \\                                                           & $EC =  EC_{temp}- x, \exists x,y \in EC_{(temp)}, x \subset y $ \\ \hline
%%%%%%%%%%
%  $R \difference S$ & $EC(R)$ \\ \hline
  \end{tabular}
\caption{Bottom-up Inference Of Property \textit{EC}}
\label{tab:bottom-up}

\end{table}
%%%%%%%%%%%%%%%%%%%%%%%%%%%%%%%%%%%%%%%%

%%%%%%%%%%%%%%%%%%%%%%%%%%%%%%%%%%%%%%%%
\begin{table*}
\centering
\caption{Top-down inference of property \textit{EC} (\textit{Equivalence Class}) for the input(s) of operator $\Diamond$}
\label{tab:top-down}
  \begin{tabular}{|c|c|} \hline 
\rowcolor[gray]{.9}  Operator $\Diamond$ & Inferred property \textit{set} of input(s) of $\Diamond$\\ \hline 
%%%%%%%%%%%%%%%%
  %R & $ list_ {R} $ \\ \hline
  %$\selection_ {((a_{1} \Box c_{1}) \wedge...\wedge (a_{n} \Box c_{n}))(R)}$ & $\{ x \cup y|x \in EC(\selection_ {((a_{1} \Box c_{1}) \wedge...\wedge (a_{n} \Box c_{n}))(R)}), $ \\
  % & $y \in EC(\selection_ {((a_{1} \Box c_{1}) \wedge...\wedge (a_{n} \Box c_{n}))(R)}), a_{i} \in x, a_{i} \in y, i \in 1:n \} $ \\ \hline
  $\selection_ {(\theta_{i} \wedge ... \wedge \theta_{n})}(R)$ & $ EC(R) = EC(\selection_ {(\theta_{i} \wedge ... \wedge \theta_{n})}(R))$ 
  
  \\ \hline
%%%%%%%%%%%
  $\projection_ {a_{1} \rightarrow b_{1},...,a_{n} \rightarrow b_{n}(R)}$ & $EC(R) = {\cal E}^* ( \{\{ a_i, a_j \} \mid \exists E \in EC(\projection_ {a_{1} \rightarrow b_{1},...,a_{n} \rightarrow b_{n}}(R)) \wedge b_i \in E \wedge b_j \in E \} \union EC(R))$ \\ \hline
%%%%%%%%%%% 
 $R \join_ {a=b} S$ & $EC(R) = \{E-\schema{S}|E \in EC(R \join_ {a=b} S) \}$   \\ 
                     & $EC(S) = \{E-\schema{R}|E \in EC(R \join_ {a=b} S) \}$ \\ \hline
                     
%%%%%%%%%%%%%
  $R \crossprod S$ & $EC(R) = \{E-\schema{S}|E \in EC(R \join_ {a=b} S) \}$   \\ 
                   & $EC(S) = \{E-\schema{R}|E \in EC(R \join_ {a=b} S) \}$ \\ \hline
%%%%%%%%%%%%%
  $_{b_{1},...,b_{n}} \aggregation _{F(a)}(R)$ & $EC(R) = {\cal E}^*(\{ E \cap \schema{R} |E \in _{b_{1},...,b_{n}} \aggregation _{F(a)}(R)\} \cup EC(R))  $ \\ 
   \hline
%%%%%%%%%%%%  
  $\duplicate(R)$ & $EC(R) = EC(\duplicate(R)) $ \\ \hline
%%%%%%%%%%%%
  $R \union S$ & $ EC(R) = {\cal E}^*(EC(R \union S) \cup EC(R))$ \\ 
                                                   & $ EC(S) = {\cal E}^*(EC(R \union S)[\schema{R}/\schema{S}] \cup EC(S))$ \\ \hline
%%%%%%%%%%%%
  $R \intersection S$ & $ EC(R) = EC(R \intersection S) $  \\ 
                                                          & $ EC(S) = EC(R \intersection S)[\schema{R}/\schema{S}]$\\ \hline
%%%%%%%%%%%
  $R \difference S$ & $ EC(R) = EC(R \difference S) $ \\ 
                                                        & $ EC(S) = EC(R \difference S)[\schema{R}/\schema{S}] $ \\ \hline
%%%%%%%%%%%%%%%%%%%%%%%%
  \end{tabular}
\end{table*}

%%%%%%%%%%%%%%%%%%%%%%%%%%%%%%%%%%%%%%%%
\subsection{Merge Adjacent Projections and Selections}
%\begin{equation}\label{eq:merge-proj}
%   \begin{aligned}
%     &\projection_{e_{1} \rightarrow A_{1},...,e_{n} \rightarrow A_{n}}(\projection_{e'_{1} \rightarrow B_{1},...,e'_{m} \rightarrow B_{m}}(Q)) \rightarrow \\
%        &\projection_{e_{1}[B_{1}/e'_{1},...,B_{m}/e'_{m}] \rightarrow A_{1},...,} \\ 
%        &_{e_{n}[B_{1}/e'_{1},...,B_{m}/e'_{m}] \rightarrow A_{n}}(Q)
%  \end{aligned}
%\end{equation}

%\begin{equation}\label{eq:merge-sel}
%    \selection_ {\theta_1} (\selection_ {\theta_2} (Q))  \rightarrow          
%    \selection_ {\theta_1 \wedge \theta_2}(Q)
%\end{equation}

%Rule~\eqref{eq:merge-proj} merges adjacent projections which is a standard relational algebra equivalence rule. If two projection operators are adjacent, we can merge them into one projection operator by substituting references to attributes in the outer projection with the expressions from the inner projection that define these attributes. The underline idea is that
%trying to combine multiple projection operators into one operator simplifies the query and may open up opportunities for applying additional rules (e.g., removing redundant projections as introduced below). 
Most database systems contain this rule, in constrast to them we do a safety check before applying this rule to avoid the potential exponential blowup in expression size as described in the introduction. Whenever merging projections results in a superlinear increase in expression size, we do not join the projections. In fact, we will force the database system to materialize the intermediate results to prevent it from merging these projections. Since materialization cannot be expressed in relational algebra we do not describe this approach here.
%We use $e$ to denote expressions (e.g., $e_{1}=a+b$ where $a$ and $b$ are attributes). Recall that $e[x/y]$ denotes replacing each occurrence of expression $x$ (usually an attribute) in $e$ with expression $y$.
% The different is that here we add a satisfy check function which the normal database system did have.
%  $e_{1}$ is a calculation expression
% among parameters $B_{1},...,B_{k}$(B is the rename of e).

%%%%%%%%%%%%%%%%%%%%%%%%%%%%%%%%%%%%%%%%%%%%%%%%%%%%%%%%%%%%
\section{Heuristic Optimizations}\label{sec:heuristic}

The heuristic optimizations we introduce in this section are applied to  the relational algebra representation of a query, i.e., after the compilation of a provenance request into relational algebra. We present each rule as $\frac{pre}{q \rightarrow q'}$ which has to be read as ``If condition $pre$ holds, then $q$ can be rewritten as $q'$''. Similar to the approach from Grust et al.~\cite{grust2010let}, we infer properties for the operators of an algebra expression and use these properties in preconditions of rules. For instance, $key(op)$ denotes the candidate keys for the result of an operator $op$.  All rules preserve equivalence, i.e., the input algebra expression is equivalent to the output algebra expression. 

% \footnote{A candidate key of a relation $R$ is a set of attributes from $\schema{R}$ which is a superkey and minimal according to set inclusion. A \textit{superkey} $K$ for relation $R$ is a subset of the attributes of $R$ so that the values of $K$ uniquely identify each tuple of $R$: $\forall t,t' \in R: t.K = t'.K \rightarrow t = t'$.}         

%%%%%%%%%%%%%%%%%%%%%%%%%%%%%%%%%%%%%%%%
\subsection{Property Inference}

We infer properties that hold for operators of an algebra graph. These properties help us to simplify the definition and application of optimization rewrite rules. 
We use bottom-up and top-down traversals of algebra trees (graphs) to compute these properties for each operator in a query. Some properties can be computed in a single top-down or bottom-up traversal whereas others require a top-down and a bottom-up pass.
The properties that we consider in this work are:

\begin{itemize}
\item \textit{set}: set is a boolean property generated top-down. Its value indicates if ancestors of operator in the graph undergo duplicate elimination. Initially, set is true for all operator expect for the root operator. We use set to remove unnecessary duplicate removal operators.
\item \textit{keys}: keys is the set of candidate keys of an operator generated bottom-up. It is used in the duplicate removal heuristic rule. For example, consider a relation $R$ with schema $\{A,B,C,D\}$. If each tuple can be uniquely identified by attribute $\{A\}$ and by attributes $\{B,C\}$, then keys is $\{\{A\},\{B,C\}\}$.
\item \textit{EC}: EC is the short form of Equivalence Class. This property is a set of sets where each set contains attributes (and/or constants) that are guaranteed to have the same value in the output of an operator. For example, consider a relation $R$ which has attributes $\{A,B,C,D\}$ and $EC=\{\{A\},\{B,C\},\{D\}\}$. We know that $B$ and $C$ are the same equivalence class which means $B$ and $C$ have the same value in each tuple of $R$. This property is generated by a bottom-up followed by a top-down traversal.
\item \textit{icols}: This property records which attributes are needed by ancestors of operator $\Diamond$. For example, if relation $R$ has attributes $\{A,B,C,D\}$, in the relational algebra expression $\projection_{A,B}(R)$ we would set  $\textit{icols}(R)=\{A,B\}$, because the projection operator (the only parent operator of $R$) needs attributes $\{A,B\}$ to compute its result. We mainly use \textit{icols} to determine redundant computations (e.g., in $\projection_{A} (\projection_{A, B+C \to D}(R))$ the computation $B+C$ is never used and, thus, can be omitted) and push projections (remove unneeded attributes early on to reduce the size of tuples).
\end{itemize}

For sake of space we do not present the inference rules for all these properties, but instead just discuss the inference rules for one property in detail.

%%%%%%%%%%%%%%%%%%%%%%%%%%%%%%%%%%%%%%%%
\begin{table*}
\centering
\caption{Bottom-up inference of property \textit{EC} (\textit{Equivalence Class}) of operator $\Diamond$}
\label{tab:bottom-up}
  \begin{tabular}{|c|c|} \hline 
\rowcolor[gray]{.9}  Operator $\Diamond$ & Inferred property for the input(s) of $\Diamond$\\ \hline 
  R & $\{\{a\}\mid a \in \schema{R} \}$ \\ \hline
%%%%%%%%%%
  $\selection_ {(\theta_{i} \wedge ... \wedge \theta_{n})}(R)$ & ${\cal E}^* (EC(R) \cup 
\{\{a,b\}\mid \exists i: \theta_{i}=(a=b) \} 
)$

% $\{x \cup \{c\}\mid \theta_{i}=(a=c)(i \in 1:n), \exists x \in EC(R), a \in x \wedge c \in Const \} $ \\
%                                                                & $\cup~\{x \cup y\mid \theta_{i}=(a=c)(i \in 1:n), \exists x,y \in EC(R), a \in x \wedge c \in y \wedge c \in Variable\}$ \\  
%                                                                & $\cup~\{x\mid \theta_{i}=(a=c)(i \in 1:n), \exists x \in EC(R), \not \exists a \in x  \} $
    \\ \hline                                                          
%%%%%%%%%%
  $\projection_ {a_{1} \rightarrow b_{1},...,a_{n} \rightarrow b_{n}}(R)$ & ${\cal E}^* ( \{\{ b_i, b_j \} \mid \exists E \in EC(R) \wedge a_i \in E \wedge a_j \in E \} \union \{\{b_i\} | i \in \{1,\ldots,n\}\})$ \\
  %& maybe: \\
  %& ${\cal E}^* ( \{\{ b_i, b_j \} \mid \exists x \in EC(R) \wedge a_i \in x \wedge a_j \in x \wedge a_i \neq a_j\}$ \\
  %& $\cup~ \{ \{b_i\} \mid x \in EC(R) \wedge a_i \in x \wedge a_j \in x~ \wedge \not\exists a_j : a_i = a_j  \})$ \\
  
% $\{ (x - \{a_ {i}\} \cup \{b_ {i}\}) \cap SCH(\projection_ {a_{1} \rightarrow b_{1},...,a_{n} \rightarrow b_{n}(R)})\mid \exists x \in EC(R), a_i \in x, i \in 1:n \} $
  \hline
%%%%%%%%%%
  $R \join_ {a=b} S$ & ${\cal E}^*(EC(R) \cup EC(S) \cup \{\{a,b\}\}) $\\ \hline
% $ \{x \cup y\mid \exists x \in EC(R), \exists y \in EC(S), a \in x \wedge b \in y \}$\\
%                      & $ \cup~(EC(R)-x)~\cup~(EC(S)-y) $ \\ \hline
%%%%%%%%%%
  $R \crossprod S$ & $EC(R) \cup EC(S) $\\ \hline
%%%%%%%%%%
  $ _{b_{1},...,b_{n}} \aggregation _{F(a)}(R) $ & $\{  \{ b_{1},...,b_{n} \} \cap E \mid E \in EC(R) \}  \cup \{\{F(a)\}\} $ \\ \hline
  $\duplicate(R)$ & $EC(R) $ \\ \hline
%%%%%%%%%%
  $R \union S$ & ${\cal E}^* (\{ E \cap E' \mid E \in EC(R) \wedge E' \in EC(S)[\schema{S}/\schema{R}] \}$
  % $R \union S$ & $\{ x \cap y\mid \exists x \in EC(R),\exists y \in EC'(S), EC'(S) = EC(S)_{(b_{i} \rightarrow a_{i})}, i \in \{1,...,n\} \}$
    \\ \hline
%%%%%%%%%%
  $R \intersection S$ & ${\cal E}^*( EC(R) \union EC(S)[\schema{S}/\schema{R}])$ \\ \hline
% EC_{temp} = \{ x \cup y\mid x \in EC(R), y \in EC'(S),EC'(S)=EC(S)_{(b_{i} \rightarrow a_{i})}, x \cap y \neq \emptyset, i \in \{1,...,n\} \}$ \\ 
%                                                           & $EC =  EC_{temp}- x, \exists x,y \in EC_{(temp)}, x \subset y $ \\ \hline
%%%%%%%%%%
  $R \difference S$ & $EC(R)$ \\ \hline
  \end{tabular}
\end{table*}
%%%%%%%%%%%%%%%%%%%%%%%%%%%%%%%%%%%%%%%%

%%%%%%%%%%%%%%%%%%%%%%%%%%%%%%%%%%%%%%%%
\subsubsection{Equivalence Classes (EC)}

The equivalence class property of an operator stores which attributes in the result of the operator are guaranteed to have equal values. This is useful for heuristic rules that introduce or moves around selection operators.
The set of equivalence classes 
$EC(R)=\{E_{1},E_{2},...,E_{n}\}$ for relation $R$ is a set of sets of attributes (and constants) where each $E_{i}$ is a set of attributes that are equivalent to each other (are guaranteed to have the same values).
For example, consider a relation $R$ with attributes $\{A,B,C\}$. If we know $B=C$ holds for every tuple in $R$, then the equivalence classes for $R$ are: $EC(R) = \{\{A\},\{B,C\}\}$. As an example for why such equivalences hold over the result of query operators consider a query $\selection_{B=C}(R)$. Since every tuple in the result of this selection has to fulfill the selection condition (this follows from the definition of selection), we know that $B=C$ will hold for any result tuple and, thus, attributes $B$ and $B$ will be in the same equivalence class.

We compute equivalence classes in a bottom-up traversal followed by a top-down traversal of a query graph.
Table~\ref{tab:bottom-up} and Table~\ref{tab:top-down} show the inference rules for each operator for the bottom-up and top-down traversal. Recall that $\schema{R}$ denotes the schema of the relation $R$. Before discussing some of these inference rules we discuss a general properties of equivalence classes and present some notation. Equivalence of attributes is transitive, i.e., if $A=B$ and $B=C$ then it follows that $A=C$. Thus, it makes sense to define the equivalence classes of a relation as the maximal sets of attributes so that each two attributes from a class are transitively equivalent to each other. In the inference rules we make use of an operator ${\cal E}^*$ that takes a set of sets of attributes and computes the fix-point of the following operation: merge two sets if they overlap. In other words, this operator merges sets if their attributes should belong to the same equivalence class. Formally, operator ${\cal E}^*$  can be defined as the least fixed-point of operator $\cal E$ shown below:

%\BG{correct layout}
\begin{align*}
{\cal E}(EC) = &\{ E \union E' \mid E \in EC \wedge E' \in EC \wedge E \cap E' \neq \emptyset  \\
&\wedge E \neq E' \} \cup \{ E \mid E \in EC \wedge E' \in EC \\
&~\wedge \not\exists E':  E \cap E' \neq \emptyset \}
\end{align*}

In the following we use $e[x/y]$ to denote replacing each occurrence of expression $x$ (usually an attribute) in $e$ with expression $y$. We use the same notation for lists of replacements, e.g., $e[a/x, b/y]$.
Since $\schema{R}$ stands for the schema of relation $R$, $[\schema{R} / \schema{S}]$ denotes replacing each attribute schema of $R$ with the corresponding (by position) attribute from the schema of $S$. That is, we replace the first attribute of $R$ with the first one from $S$ and so on.
 
% \BG{I do not think we needs this again here. This was already defined in the relational algebra section. F() means the function, such as sum(), min(), max(). e.g., if F(a)=sum(a), it returns the total sum of column a. }

We now describe a few exemplary equivalence class inference rules as shown in Table~\ref{tab:bottom-up} and Table~\ref{tab:top-down}.

%%%%%%%%%%
\parttitle{Selection Bottom-up Rule} Recall that for a selection $\theta$ stands for a condition such as $a<b$ or $a=b$. Consider the inference rules for  a selection $\selection_ {(\theta_{i} \wedge ... \wedge \theta_{n})}(R)$ (Table~\ref{tab:bottom-up}).
 Note that any selection condition can be written in this way. The underline idea is that if $\theta$ is an equality condition such as $a=b$, we have to distinguish  two cases: 1) If $b$ is a constant, we need to add $b$ into the EC which contains $a$ (we call it $EC(R,a)$). 2) If $b$ is a variable, we need to union $EC(R,a)$ with $EC(R,b)$.
The set comprehension $\{\{a,b\}\mid \exists i: \theta_{i}=(a=b) \}$ implements these conditions. If $\theta_i$ if it is an equality comparison, then we generate an EC which contains these two elements. However, $a$ and/or $b$ may already been part of an equivalence class. For this case, we need to union them by using operator ${\cal E}^*$. For example, if relation $R$ has schema $\{A,B,C\}$ and $EC(R)=\{\{A,B\},\{C\}\}$, then $EC(\selection_{A=5 \wedge C<9}(R)) = \{\{A,B,5\},\{C\}\}$.             

%%%%%%%%%%
\parttitle{Join Bottom-up Rule} The rule for join $R \join_ {a=b} S$ (Table~\ref{tab:bottom-up}), has to merge $EC(R,a)$  with $EC(b)$ in relation $S$. Thus, we generate a new EC set $\{\{a,b\}\}$ and union it with $EC(R)$ and $EC(S)$. At last we apply the same last step as for the selection rule, using ${\cal E}^*$ to union ECs which overlap. For example, if relation $R$ has schema $\{A,B,C\}$ with $EC(R)=\{\{A,B\},\{C\}\}$ and relation $S$ has schema $\{D,E,F\}$ with $EC(S)=\{\{D\},\{E,F\}\}$. Then, $EC(R \join_{A=D} S)=\{\{A,B,D\},\{C\},\{E,F\}\}$.     

%%%%%%%%%%
\parttitle{Union Bottom-up Rule} 
In the union rule $R \union S$ (Table~\ref{tab:bottom-up}), we rename the attributes of $S$ in $EC(S)$ to the attribute of $R$ by using $EC(S)[\schema{S}/\schema{R}]$. Then we combine $EC(S)$ with $EC(R)$. Finally, we use ${\cal E}^*$ to merge  overlapping classes. For example, if relation $R$ has schema $\{A,B\}$ with $EC=\{\{A\},\{B\}\}$ and relation $S$ has schema $\{C,D\}$ with $EC=\{\{C,D\}\}$, then $EC(R \union S)=\{\{A\},\{B\}\}$.

%%%%%%%%%%
\parttitle{Union Top-down Rule} 
The top-down rule for union $R \union S$ (Table~\ref{tab:top-down}), because it is a top-down traversal, we combine the existing $EC$ for $R$ (respective $S$) with the information for $EC(R \union S)$.
For $EC(R)$ we 1) combine these sets with $EC(R \union S)$, 2) using $(\cal E)^*$ to get rid of the overlap. For $EC(S)$, we apply the same steps as for $EC(R)$. For example, if relation $R$ has schema $\{A,B\}$ with $EC(R)=\{\{A\},\{B\}\}$ and $S$ with schema $\{C,D\}$ and $EC(S)=\{\{C,D\}\}$ then $EC(R \union S)=\{\{A,B,C\},\{D\}\}$. After applying the top-down rule we get $EC(R)=\{\{A,B\}\}$ and $EC(S)=\{\{C,D\}\}$.

We now describe the rules supported by our current implementation of the heuristic optimizer and motivate why they are useful in the context of our application.

\begin{table*}
\centering
\caption{Top-down inference of property \textit{EC} (\textit{Equivalence Class}) for the input(s) of operator $\Diamond$}
\label{tab:top-down}
  \begin{tabular}{|c|c|} \hline 
\rowcolor[gray]{.9}  Operator $\Diamond$ & Inferred property \textit{set} of input(s) of $\Diamond$\\ \hline 
%%%%%%%%%%%%%%%%
  %R & $ list_ {R} $ \\ \hline
  %$\selection_ {((a_{1} \Box c_{1}) \wedge...\wedge (a_{n} \Box c_{n}))(R)}$ & $\{ x \cup y|x \in EC(\selection_ {((a_{1} \Box c_{1}) \wedge...\wedge (a_{n} \Box c_{n}))(R)}), $ \\
  % & $y \in EC(\selection_ {((a_{1} \Box c_{1}) \wedge...\wedge (a_{n} \Box c_{n}))(R)}), a_{i} \in x, a_{i} \in y, i \in 1:n \} $ \\ \hline
  $\selection_ {(\theta_{i} \wedge ... \wedge \theta_{n})}(R)$ & $ EC(R) = EC(\selection_ {(\theta_{i} \wedge ... \wedge \theta_{n})}(R))$ 
  
  \\ \hline
%%%%%%%%%%%
  $\projection_ {a_{1} \rightarrow b_{1},...,a_{n} \rightarrow b_{n}(R)}$ & $EC(R) = {\cal E}^* ( \{\{ a_i, a_j \} \mid \exists E \in EC(\projection_ {a_{1} \rightarrow b_{1},...,a_{n} \rightarrow b_{n}}(R)) \wedge b_i \in E \wedge b_j \in E \} \union EC(R))$ \\ \hline
%%%%%%%%%%% 
 $R \join_ {a=b} S$ & $EC(R) = \{E-\schema{S}|E \in EC(R \join_ {a=b} S) \}$   \\ 
                     & $EC(S) = \{E-\schema{R}|E \in EC(R \join_ {a=b} S) \}$ \\ \hline
                     
%%%%%%%%%%%%%
  $R \crossprod S$ & $EC(R) = \{E-\schema{S}|E \in EC(R \join_ {a=b} S) \}$   \\ 
                   & $EC(S) = \{E-\schema{R}|E \in EC(R \join_ {a=b} S) \}$ \\ \hline
%%%%%%%%%%%%%
  $_{b_{1},...,b_{n}} \aggregation _{F(a)}(R)$ & $EC(R) = {\cal E}^*(\{ E \cap \schema{R} |E \in _{b_{1},...,b_{n}} \aggregation _{F(a)}(R)\} \cup EC(R))  $ \\ 
   \hline
%%%%%%%%%%%%  
  $\duplicate(R)$ & $EC(R) = EC(\duplicate(R)) $ \\ \hline
%%%%%%%%%%%%
  $R \union S$ & $ EC(R) = {\cal E}^*(EC(R \union S) \cup EC(R))$ \\ 
                                                   & $ EC(S) = {\cal E}^*(EC(R \union S)[\schema{R}/\schema{S}] \cup EC(S))$ \\ \hline
%%%%%%%%%%%%
  $R \intersection S$ & $ EC(R) = EC(R \intersection S) $  \\ 
                                                          & $ EC(S) = EC(R \intersection S)[\schema{R}/\schema{S}]$\\ \hline
%%%%%%%%%%%
  $R \difference S$ & $ EC(R) = EC(R \difference S) $ \\ 
                                                        & $ EC(S) = EC(R \difference S)[\schema{R}/\schema{S}] $ \\ \hline
%%%%%%%%%%%%%%%%%%%%%%%%
  \end{tabular}
\end{table*}

%%%%%%%%%%%%%%%%%%%%%%%%%%%%%%%%%%%%%%%%
\subsection{Merge Adjacent Projections and Selections}
\begin{equation}\label{eq:merge-proj}
   % \frac{.}{\projection_ {a_{1}, a_{2},..., a_{n}} \projection_ {b_{1}, b_{2},..., b_{n}}(R)  \rightarrow \projection_ {a_{1}, a_{2},..., a_{n}}(R)}
   %\projection_ {a_{1},..., a_{n}} (\projection_ {b_{1},..., b_{n}}(R))  \rightarrow \projection_ {a_{1},..., a_{n}}(R)
   \begin{aligned}
     &\projection_{e_{1} \rightarrow A_{1},...,e_{n} \rightarrow A_{n}}(\projection_{e'_{1} \rightarrow B_{1},...,e'_{m} \rightarrow B_{m}}(Q)) \rightarrow \\
        &\projection_{e_{1}[B_{1}/e'_{1},...,B_{m}/e'_{m}] \rightarrow A_{1},...,} \\ 
        &_{e_{n}[B_{1}/e'_{1},...,B_{m}/e'_{m}] \rightarrow A_{n}}(Q)
  \end{aligned}
\end{equation}

\begin{equation}\label{eq:merge-sel}
   % \frac{.}{\selection_ {a_{1}, a_{2},..., a_{n}} \selection_ {b_{1}, b_{2},..., b_{n}}(R)  \rightarrow 
   % \selection_ {a_{1}, a_{2},..., a_{n},b_{1}, b_{2},..., b_{n}}(R)}
    \selection_ {\theta_1} (\selection_ {\theta_2} (Q))  \rightarrow          
    \selection_ {\theta_1 \wedge \theta_2}(Q)
\end{equation}

Rule~\eqref{eq:merge-proj} merges adjacent projections which is a standard relational algebra equivalence rule. If two projection operators are adjacent, we can merge them into one projection operator by substituting references to attributes in the outer projection with the expressions from the inner projection that define these attributes. The underline idea is that
trying to combine multiple projection operators into one operator simplifies the query and may open up opportunities for applying additional rules (e.g., removing redundant projections as introduced below). Note that in constrast to most database systems we do a safety check before applying this rule to avoid the potential exponential blowup in expression size as described in the introduction. Whenever merging projections results in a superlinear increase in expression size, we do not join the projections. In fact, we will force the database system to materialize the intermediate results to prevent it from merging these projections. Since materialization cannot be expressed in relational algebra we do not describe this approach here.

 We use $e$ to denote expressions (e.g., $e_{1}=a+b$ where $a$ and $b$ are attributes). Recall that $e[x/y]$ denotes replacing each occurrence of expression $x$ (usually an attribute) in $e$ with expression $y$.
% The different is that here we add a satisfy check function which the normal database system did have.
%  $e_{1}$ is a calculation expression
% among parameters $B_{1},...,B_{k}$(B is the rename of e).

\begin{Example}
  For example, consider the query $\projection_{a + b \to c} (\projection_{a, d + e \to b}(R))$. Merging projections we get:
$\projection_{a + (d + e) \to c}(R)$. In the inner projection, $d + e$
  is renamed to $b$. Hence, if we merge the projections, then $b$ should be
  replaced with $(d + e)$.
\end{Example}

Rule~\eqref{eq:merge-sel} merges adjacent selections. This is also a textbook equivalence rule. When two selections are adjacent, we can replace them with a single selection which uses the conjunction of the conditions of the two  selections. Its purpose is to reduce the number of the selections, e.g., after introducing a new selection based on the rules presented in Sec.~\ref{sec:selection-move-around}.
Here $\theta$ is  the condition of the selection operator. For example, $\selection_ {a=5} (\selection_ {b<6}(R)) \rightarrow \selection_ {(a=5 \wedge b<6)}(R)$.

%%%%%%%%%%%%%%%%%%%%%%%%%%%%%%%%%%%%%%%%
\subsection{Remove Redundant Projections}
\begin{equation}\label{eq:remove-redund-proj}
    \frac{\schema{R} = \{a_{1},...,a_{n}\}}{\projection_ {a_{1},..., a_{n}}(R)  \rightarrow R} 
\end{equation}

Recall that in rules the expression above the line is a condition. If matching the condition, the rewrite below the line can be applied. 
Rule~\eqref{eq:remove-redund-proj}, is applicable if a projection returns all attributes from schema of the input relation $R$ (the projection projects on all attributes $a_1$,\ldots,$a_n$ from schema \schema{R}). In this case we can just remove the projection operator. 
A user would never write such kind of query, however, after provenance rewriting and applying other heuristic optimizations, we can get  this kind of expressions and this rule helps us to simplify them.

% %%%%%%%%%%%%%%%%%%%%%%%%%%%%%%%%%%%%%%%%

% \iffalse
% \subsection{Selection pushdown}
% \begin{equation}
%     \selection_{p} (\projection_ {a_{1},..., a_{n}} (R)) \rightarrow \projection_ {a_{1},..., a_{n}} (\selection_{p} (R))
% \end{equation}

% \begin{equation}
%     \selection_{a=C} (R \Join_{a=b} S)  \rightarrow (\selection_{a=C}R) \Join_{a=b} S
% \end{equation}

% \begin{equation}
%     \selection_{a=C} (R  \cup  S)  \rightarrow (\selection_{a=C}R) \cup (\selection_{b=C}S)
% \end{equation}
% \fi
% \BG{This becomes redundant if we do selection move-around, remove this subsection (comment out)}

% \iffalse
% explain these rules \\
% \parttitle{Push through projection:} Rule 4, if the selection is based on a projection, we can just
% push down the selection to the below level of the projection. \\

% \parttitle{Push through join:} Rule 5, similar with the push through projection, Just push down the
% selection to the below level of the join operator. The difference is that it contains two cases. One is that 
% when selection condition is same with the join condition, we need to push it down to both sides of the join. 
% Otherwise, we just need to push it down to one side which contains this attribute in the selection condition. \\

% \parttitle{Push through set operators:}
% Push through set operators

% \parttitle{Push through union:} Rule 6, if selection is based on a union operation, we just push the 
% selection down to both sides of the union operation. In one side, we need to change the attribute's name\\
% \fi
%%%%%%%%%%%%%%%%%%%%%%%%%%%%%%%%%%%%%%%%
\subsection{Selection Move-around}\label{sec:selection-move-around}
\begin{equation}\label{eq:select-move-around1}
     \frac{\exists E \in EC(R) \wedge a \in E \wedge b \in E}{R \rightarrow \selection_{a=b}(R)}
\end{equation}

\begin{equation}\label{eq:select-move-around2}
     \frac{\exists E \in EC(R) \wedge a \in E \wedge b \in E}{\selection_{\theta}(R) \rightarrow \selection_{\theta}(\selection_{\theta[a/b]}(R))}
\end{equation}

% \BG{Need explanation here. Selection move-around standard. But we go further than most systems. Also important because beneficial interaction with other rules and properties.}
Selection move-around (a more general form of the textbook selection-pushdown equivalence) enables us to push down selection to reduce the size of intermediate results and to move selections sideways, i.e., from one branch of the query to another.
In Rule~\eqref{eq:select-move-around1}, if attributes $a$ and $b$ both belong to the same equivalence class of $EC(R)$, which implies $a=b$, we can introduce a new selection $\selection_{a=b}$ over $R$.

In Rule~\eqref{eq:select-move-around2}, $a$ and $b$ are attributes of relation $R$, not belong to the same equivalence class of $EC(R)$. If we have a condition containing $a$ (such as $a<5$), we can introduce another selection on a condition which is derived by replacing $a$ with $b$ (e.g., $b<5$).

For example, for the algebra expression shown in Fig.~\ref{fig:ex-selection-move-around}~(a), the left child of the join operator is a selection operator and the attribute $id$ in the condition of selection operator is also in the condition of the join operator. We can replace $id$ with $itemId$ since they are in the same equivalence class and introduce a new selection based on the this condition to the right child of the join operator. The result show in Fig.~\ref{fig:ex-selection-move-around}~(b).  

% \iffalse
% In the Rule 7, if one side of the join operation is selection operation like this format $ \selection_{a \Diamond C} $ and the condition of the join operator
% contains the attribute(a) which in the condition of the selection operator, then we copy the condition and change the attribute a to b, then we add the new
% selection to another side of the join operation.
% \fi

% \BG{As discussed some time ago, replace this with a general rule using the EC propoerty to introduce a new selection and then in the example demonstrate how this can move a selection, e.g., from the left branch to the right branch of a join.}

 %%%%%%%%%%%%%%%%%%%%%%%%%%%%%%%%%%%%%%%%
\begin{figure}[t]
\centering

\subfloat[]{
\begin{tikzpicture}
[op/.style={anchor=south west},
conn/.style={-}]

%\node[op] (p) at (0,3) {$\projection_{name,pid,price}$};
%\node[op] (s) at (0,2) {$\selection_{sName='Merdiers'}$};

\node[op] (j) at (0,2) {$\join_{id=itemId}$};

\node (r1) at (-0.75,1) {$\selection_{id>1}$};
\node (r2) at (1.25,1) {$sales$};

\node (r3) at (-0.75,0) {$items$};
%\draw[conn] ($(p.south west) + (2.5mm,0)$) to ($(s.north west) + (2.5mm,0)$);
%\draw[conn] ($(s.south west) + (2.5mm,0)$) to ($(j.north west) + (2.5mm,0)$);

\draw[conn] ($(j.south west) + (2.5mm,0)$) to (r1);
\draw[conn] ($(j.south west) + (2.5mm,0)$) to (r2);

\draw[conn] ($(r1.south west) + (5.5mm,0)$) to (r3);
\end{tikzpicture}}

\subfloat[]{
\begin{tikzpicture}
[op/.style={anchor=south west},
conn/.style={-}]

%\node[op] (p) at (0,3) {$\projection_{name,pid,price}$};
%\node[op] (s) at (0,2) {$\selection_{sName='Merdiers'}$};

\node[op] (j) at (0,2) {$\join_{id=itemId}$};

\node (r1) at (-0.75,1) {$\selection_{id>1}$};
\node (r2) at (1.25,1) {$\selection_{itemId>1}$};

\node (r3) at (-0.75,0) {$items$};
\node (r4) at (1.25,0) {$sales$};

%\draw[conn] ($(p.south west) + (2.5mm,0)$) to ($(s.north west) + (2.5mm,0)$);
%\draw[conn] ($(s.south west) + (2.5mm,0)$) to ($(j.north west) + (2.5mm,0)$);
\draw[conn] ($(j.south west) + (2.5mm,0)$) to (r1);
\draw[conn] ($(j.south west) + (2.5mm,0)$) to (r2);

\draw[conn] ($(r1.south west) + (5.5mm,0)$) to (r3);
\draw[conn] ($(r2.south west) + (8.5mm,0)$) to (r4);
\end{tikzpicture}}

\caption{Example: selection move around}
\label{fig:ex-selection-move-around}
\end{figure}
%%%%%%%%%%%%%%%%%%%%%%%%%%%%%%%%%%%%%%%%

%%%%%%%%%%%%%%%%%%%%%%%%%%%%%%%%%%%%%%%%
\subsection{Pulling up Provenance Projections}

\begin{equation}\label{eq:pulling-up-provenance-projections}
     \frac{ a \subseteq \schema{\Diamond(\projection_{A}(R))} \wedge b \not\in icols(\Diamond(\projection_{A}(R))) }{\Diamond(\projection_{A,a \to b}(R)) \to  
     \projection_{\schema{\Diamond(\projection_{A}(R))},a \to b}(\Diamond(\projection_A (R)))}
\end{equation}

Query rewrite based provenance as implemented by, e.g., GProM,  propagates provenance by duplicating attributes of the input (projection). This increases the size of tuples in intermediate results which can have a negative effect on performance. This rewrite rule exploits the fact that we can delay this duplication of attribute values if the attribute we are duplicating is still available in the parent of the projection operator duplicating the attribute.

In Rule~\eqref{eq:pulling-up-provenance-projections}
$b$ is an attribute storing provenance that was generated by duplicating attribute $a$. If $a$ is available in schema of $\Diamond(\projection_{A}(R))$ (where $\Diamond$ can be any operator) and $b$ is not needed to compute $\Diamond(\projection_{A}(R))$,
then  we can postpone the projection on $a \to b$ after operator $\Diamond$. 

For example, Fig.~\ref{fig:ex-pullup-provenance-projections}~(a) shows the original algebra tree of a query, we get the provenance of attribute $sName$ by duplicating the attribute $sName$ and rename it to $P(sName)$. Then we join the projection with the relation $items$ and the schema of join operator is $(id,price,sName,itemId,P(sName))$. In this case, we can postpone the duplication of attribute $sName$ and introduce a new projection operator which with duplication of this attribute in the up layer of join operator, the result shows in (b).  
%\BG{make example more concrete}

 %%%%%%%%%%%%%%%%%%%%%%%%%%%%%%%%%%%%%%%%
\begin{figure}[t]
\centering

\subfloat[]{
\begin{tikzpicture}
[op/.style={anchor=south west},
conn/.style={-}]

%\node[op] (p) at (0,3) {$\projection_{name,pid,price}$};
%\node[op] (s) at (0,2) {$\selection_{sName='Merdiers'}$};
\node[op] (s) at (0,3) {$\projection_{id,price,P(sName)}$};

\node[op] (j) at (0,2) {$\join_{id=itemId}$};
\node[op] (p) at (-2,1.6) {$(id,price,sName,itemId,P(sName))$};

\node (r1) at (-1.6,0.6) {$items$};
\node (r2) at (2.5,0.6) {$\projection_{sName,itemId,sName \to P(sName)}$};

\node (r3) at (2.5,-0.6) {$sales$};
%\draw[conn] ($(p.south west) + (2.5mm,0)$) to ($(s.north west) + (2.5mm,0)$);
\draw[conn] ($(s.south west) + (2.5mm,0)$) to ($(j.north west) + (2.5mm,0)$);

\draw[conn] ($(p.south west) + (23mm,0)$) to (r1);
\draw[conn] ($(p.south west) + (23mm,0)$) to (r2);

\draw[conn] ($(r2.south west) + (25mm,0)$) to (r3);
\end{tikzpicture}}

\subfloat[]{
\begin{tikzpicture}
[op/.style={anchor=south west},
conn/.style={-}]

%\node[op] (p) at (0,3) {$\projection_{name,pid,price}$};
%\node[op] (s) at (0,2) {$\selection_{sName='Merdiers'}$};
\node[op] (q) at (0,4) {$\projection_{id,price,P(sName)}$};

\node[op] (s) at (0,3) {$\projection_{id,price,sName \to P(sName)}$};

\node[op] (j) at (0,2) {$\join_{id=itemId}$};
\node[op] (p) at (-1.5,1.6) {$(id,price,sName,itemId)$};

\node (r1) at (-1.6,0.6) {$items$};
\node (r2) at (2.5,0.6) {$\projection_{sName,itemId}$};

\node (r3) at (2.5,-0.6) {$sales$};
%\draw[conn] ($(p.south west) + (2.5mm,0)$) to ($(s.north west) + (2.5mm,0)$);
\draw[conn] ($(q.south west) + (2.5mm,0)$) to ($(s.north west) + (2.5mm,0)$);
\draw[conn] ($(s.south west) + (2.5mm,0)$) to ($(j.north west) + (2.5mm,0)$);

\draw[conn] ($(p.south west) + (18mm,0)$) to (r1);
\draw[conn] ($(p.south west) + (18mm,0)$) to (r2);

\draw[conn] ($(r2.south west) + (12mm,0)$) to (r3);
\end{tikzpicture}}

\caption{Example: pulling up provenance projections}
\label{fig:ex-pullup-provenance-projections}
\end{figure}
%%%%%%%%%%%%%%%%%%%%%%%%%%%%%%%%%%%%%%%%

%%%%%%%%%%%%%%%%%%%%%%%%%%%%%%%%%%%%%%%%%%%%%%%%%%%%%%%%%%%%
\subsection{Duplicate Removal}
\begin{equation}\label{eq:duplicate-remove}
    \frac{keys(R) \neq \emptyset}{\duplicate (R) \rightarrow R} 
\end{equation}

The rationale behind Rule~\eqref{eq:duplicate-remove} is that if relation $R$ has at least one candidate key, then it cannot contain duplicates because the values of the key columns are unique in $R$ (definition of a superkey).
Thus, the duplicate remove operator has no effect and we can safely remove it.

For example, consider the relational algebra expression $\duplicate (R)$ and the $keys$ properity of R is \{\{A\}\}. Here each tuples in relation R is unique. Thus the duplicate remove operator has no effect, we can remove it, i.e., Then $\duplicate (R) \to R$. 

%%%%%%%%%%%%%%%%%%%%%%%%%%%%%%%%%%%%%%%%%%%%%%%%%%%%%%%%%%%%
\subsection{Remove Redundant Columns}
\begin{equation}\label{eq:remove-redundant-columns1}
 \frac{A=icols(R)}{R \rightarrow \projection_A (R)}
\end{equation}

If only some attributes $A$ of relation $R$ are needed by operators that are ancestors of $R$, then we can remove all other attributes by projecting $R$ on $A$.
In Rule~\eqref{eq:remove-redundant-columns1},  $A$ denotes a set of  attributes, e.g., $\{a,b\}$. Recall that $icols(R)$ denotes the set columns or relation $R$ which are needed by ancestors of $R$ in the query.
For example, if relation $R(a,b,c)$ has $icols(R)=\{a, b\}$, then $R \to \projection_{a,b}(R)$.

\begin{equation}\label{eq:window-function}
 \frac{x \not\in icols(\omega_{a \to x} (R))}{\omega_{a \to x}(R) \rightarrow R}
\end{equation}

In Rule~\eqref{eq:window-function}, $\omega$ indicates the window function operator~\cite{windowfun}.
 $\omega_{a \to x} (R)$ stands for applying the window function $a$ over relation $R$ and add result as a new attribute $x$. If $x$ is not needed by any ancestor of $\omega (R)$, then can avoid computing it in the first place.
For example, if we have a relation $R$ with schema $\{b,c\}$, after $\omega_{a\to x} (R)$, the schema changed to $\{b,c,x\}$ where $x$ holds the result of  window function $a$. If $icols(\omega_{a \to x} (R)) =\{b,c\}$, then we can remove the window operator: $\omega_{a/x} \to R$.

%%%%%%%%%%%%%%%%%%%%%%%%%%%%%%%%%%%%%%%%%%%%%%%%%%%%%%%%%%%%
\subsection{Application of Heuristic Rewrites}
\label{sec:interaction-rules}

Right now we use a manually determined fixed order for applying these rules to an input query which is already quite effective. In the furture we would like to replace it by a fix-point computation. However, this requires us to  prove that the fix-point computation is correct first. Also we would like to explore additional rules such as moving window operators.

%%% Local Variables:
%%% mode: latex
%%% TeX-master: "2016-prov-optimizer"
%%% End:
