# Supplementary material for: Optimizing Provenance Computations
Source: arXiv:1701.05513 source file (2017-01-19)
Supplement: Supplementary file 4 [file appendix-introduction2.tex]

\section{Introduction}\label{sec:intro}
% Why PROV and what PROV is
Database provenance as information about the origin of a data  and the transformations that produced it, is critical for debugging of data and queries, auditing, probabilistic databases, establishing authorship, and many other use cases.
%
%  The provenance of a piece of data (or \textit{data item}) may include source and
% intermediate data as well as the transformations involved in producing it. In general, for every application domain where data is heavily 
% transformed, data provenance is of essential importance. Provenance information can be used to estimate the quality of data and trust measures for data, to 
% gain additional insights about it, or to trace errors in transformed data back to its origins. 
%
% For example, consider a relation storing employee salaries. The relation is subjected to complex transactional updates such as 
% calculating tax, applying  tax deductions, multipling rates with
%  working hours, and so on. How do we know the information in the current version of the relation is correct? If one 
% employee salary is wrong, how do we know which update(s) or data did cause that error? Data provenance, by providing a full record of the derivation history of data, makes it possible to track the cause of the  error. 
%
The de-facto standard for database provenance~\cite{BK13,KB12,BC08a,BK02b,KG12,karvounarakis2013collaborative,GK07,GA12} is to model provenance as annotations on data and compute the provenance for the outputs of an operation by executing instrumented versions of the operations that propagate provenance annotations.

%%%%%%%%%%%%%%%%%%%%%%%%%%%%%%%%%%%%%%%%
\begin{figure}[t]
\centering
\begin{minipage}{0.45\linewidth}
\centering
  \subfloat[shop]{%
    \begin{tabular}{c|c|c|} \cline{2-3}
 & \chead name& \chead numEmpl\\\cline{2-3}
   $s_1$ & Walmart & 3\\ \cline{2-3}
   $s_2$ & Cosco & 14 \\ \cline{2-3}
    \end{tabular}}

  \qquad\qquad%

  \subfloat[sale]{%
    \begin{tabular}{c|c|c|} \cline{2-3} 
     & \chead shop& \chead item\\ \cline{2-3}
     $a_1$ & Walmart & Steak\\ \cline{2-3}
     $a_2$ & Walmart & Butter\\ \cline{2-3}
     $a_3$ & Walmart & Bread\\ \cline{2-3}
     $a_4$ & Cosco & Butter \\ \cline{2-3} 
     $a_5$ & Cosco & Bread \\ \cline{2-3}
    \end{tabular}}
\end{minipage}
\begin{minipage}{0.45\linewidth}
\centering
  \subfloat[item]{%
    \begin{tabular}{c|c|c|} \cline{2-3} 
 & \chead id& \chead price\\ \cline{2-3}
     $i_1$ & Steak & 100\\ \cline{2-3} 
     $i_2$ & Butter & 10\\ \cline{2-3}
     $i_3$ & Bread & 25\\ \cline{2-3}
    \end{tabular}}

  \subfloat[result $q$]{%
    \begin{tabular}{c|c|} \cline{2-2}
 &\chead name\\ \cline{2-2} 
 $s_1 \cdot a_1 \cdot i_1$ & \multirow{2}{*}{Walmart} \\ 
$ + s_1 \cdot a_3 \cdot i_3 $&  \\ \cline{2-2}
  $s_2 \cdot a_5 \cdot i_3$& Cosco \\  \cline{2-2}
    \end{tabular}}
\end{minipage}
\caption{Example Database}
\label{fig:Example-database}

\end{figure}
%%%%%%%%%%%%%%%%%%%%%%%%%%%%%%%%%%%%%%%%

%%%%%%%%%%%%%%%%%%%%%%%%%%%%%%%%%%%%%%%%%%%%%%%%%%%%%%%%
\begin{figure*}[t]
\centering
  \begin{tabular}{c|c||c|c||c|c||c|c|} 
&\multicolumn{1}{c||}{\bf result} & \multicolumn{2}{c||}{\bf prov. shop} & \multicolumn{2}{c||}{\bf prov. sales} & \multicolumn{2}{c}{\bf prov. items}\\ \cline{2-8} 
%%%%%%%%%%
 & \chead  name& \chead P(name)& \chead P(numEmpl)& \chead P(shop)& \chead P(item)& \chead P(id)& \chead P(price)\\ \cline{2-8} 
%%%%%%%%%%
 $s_1 \cdot a_1 \cdot i_1$  &  Walmart  & Walmart & 3 & Walmart & Steak & Steak & 100\\ \cline{2-8} 
$s_3 \cdot a_3 \cdot i_3 $&  Walmart  & Walmart & 3 & Walmart & Butter & Butter & 10\\ \cline{2-8} 
 $s_2 \cdot a_5 \cdot i_3$&  Cosco  & Cosco & 14 & Cosco & Bread & Bread & 25\\ \cline{2-8} 
  \end{tabular}
\caption{Example Relational Encoding of Provenance Annotations}
\label{fig:provenance-result-example-database}

\end{figure*}
%%%%%%%%%%%%%%%%%%%%%%%%%%%%%%%%%%%%%%%%%%%%%%%%%%%%%%%%%%%%%%%%%

Implementations of  database provenance  such as in Perm~\cite{glavic2013using}, GProM~\cite{arab2014generic}, DBNotes~\cite{BC05a}, LogicBlox~\cite{GA12}, Datalog Debugging~\cite{KL12}, Orchestra~\cite{karvounarakis2013collaborative}, and DistTape~\cite{ZM13} use a relational encoding of provenance annotations. These systems typically compile provenance requests for a query $q$ into a query that propagates  input annotations to produce the result of $q$ annotated with provenance (to be precise, the relational encoding of this annotated relation). This approach is often called \textit{query rewriting}. Compiling query languages (e.g., queries with provenance semantics) into standard relational query languages (e.g., SQL) has also been successfully applied translating  XQuery into SQL over a shredded relational representation of SQL~\cite{grust2010let}, using a database as a co-processor for a functional programming language~\cite{GU13}, compiling languages over nested collections into SQL~\cite{CL14}, and in object relational mappers and language integrated queries (LINQ~\cite{MB06}).

Provenance rewrites and many of the other aforementioned techniques generate queries with 
unusual access patterns and operator sequences. % Even sophisticated database optimizers are often not capable of producing efficient plans for such queries.
For example, 
after provenance rewriting, the generated query expression may contain a large number of window operations interleaved with joins. Normal database queries written by humans or automatically generated by tools (e.g., reporting tools)  usually do not exhibit this kind of patterns. 
Most database optimizers are incapable of simplifying such queries and will not explore relevant parts of the plan space. 
Thus, while provenance rewrites enable easy implementation of provenance support for databases without the need to modify the database system itself, their performance is often far from optimal.
In this work we address this problem though the development of novel optimization techniques targeted at such queries, a flexible cost-based optimization framework, and the  implementation of these techniques in a our database provenance middleware  called \textit{GProM}. 

We now give a brief introduction to provenance and rewrite-based provenance computation and then show simplified versions of two examples we encountered in our previous work with provenance systems that demonstrate the need for  provenance-specific optimizations.

%%%%%%%%%%%%%%%%%%%%%%%%%%%%%%%%%%%%%%%%%%%%%%%%%%%%%%%%%%%%
\subsection{Rewrite-based Provenance Computation}
\label{sec:rewr-based-prov}

An important type of provenance supported by most provenance-aware database approaches is data dependency information for queries, i.e., to track for each output of a query from which inputs it was derived. The example below introduces provenance polynomials~\cite{karvounarakis2012semiring}, one of the most influential provenance models, used for representing this type of information. Furthermore, we introduce a relational encoding of this type of annotations and how to use the rewrite approach to compute provenance according to this model by executing SQL queries.

\begin{Example}\label{ex:simple-prov-ex}
Fig.~\ref{fig:Example-database} shows an example sales database. Consider the following query expressed in relational algebra which returns the names of shops which have sold items that cost more than \$20. 
$$
\projection_ {name} (shop \join_{name=shop} sale \join_{item=id} \selection_{price > 20}(item))
$$
The result of this query is shown in Fig.~\ref{fig:Example-database}. Both shops from the input relations are in the result. Using provenance polynomials to represent provenance, each tuple in the database is annotated with a variable representing an identifier for this tuple. In the example, these annotations are shown to the left of each tuple. The outputs of the query are annotated with polynomials over the variables annotating the input tuples. The annotations of a query result tuple explains how the tuple was derived by combining input tuples. Intuitively, the addition operation corresponds to alternative use of tuples such as in a union or projection and multiplication represents conjunctive usage (e.g., join). For example, the query result $(Walmart)$ was derived by joining tuples $s_1$,  $a_1$, and $i_1$ ($s_1 \cdot a_1 \cdot i_1$) or alternatively by joining tuples $s_1$,  $a_3$, and $i_3$ ($s_1 \cdot a_3 \cdot i_3$). Fig.~\ref{fig:provenance-result-example-database} shows a possible relational encoding (this is the actual encoding used by the Perm~\cite{glavic2013using} and GProM~\cite{arab2014generic} systems) of this query result annotated with provenance: variables are represented by the tuple they are annotating, multiplication is represented by concatenating the encoding of the variables that are multiplied, and addition is represented by encoding each summand as a separate tuple.\footnote{The full details of this encoding are beyond the scope of this paper, e.g., the encoding requires that the input polynomial is normalized into a sum of products. The interested reader is referred to~\cite{glavic2013using}.} This encoding can be computed using a different relational algebra expression, e.g., the one shown below, which adds input attributes to the final projection and renames them (represented as $\to$) to mark them as provenance attributes. 
\begin{align*}
q_{join} &= shop \join_{name=shop} sale \join_{item=id} \selection_{price > 20}(item)\\
q &= \projection_{name,name \to P(name),numEmp \to P(numEmp), \ldots} (q_{join})
\end{align*}
In fact, such a query can be generated for any SPJ (Select-Project-Join) input query (and beyond) based on a set of algebraic rewrite rules (see~\cite{glavic2013using} for details).
% In the first tuple,
% the $sum(price)$ is 120, in the second tuple, the $sum(price)$ is 50. The user may decide to request the provenance of these tuples to understand from which inputs they were derived.
% But if only provide the result tuples, how do we know where and how 
% to get the result 120 and 50 in these tuples. 
% Using, e.g., GProm, we get provenance as shown in Table~\ref{fig:provenance-result-example-database}. Here each result tuple of the query is paired with tuples from the provenance. Attributes from the input relations have been renamed to indicated that they store provenance (here represented by $P(name)$).
% From the first three rows we can see that the sum $120$ was computed by adding the prices of three input tuple combinations ($100
% +10+10$). Note that the original result tuple has been duplicated to fit in all its provenance. Similarly, for the second result tuple (the last two tuple in the provenance) the sum $50$ was computed based on two tuples from the input ($50=25+25$). Also we can see which input tuples have been joined together by the query before the aggregation. 
\end{Example}
%%%%%%%%%%%%%%%%%%%%%%%%%%%%%%%%%%%%%%%%

%%%%%%%%%%%%%%%%%%%%%%%%%%%%%%%%%%%%%%%%
\begin{figure}[t]
  \centering
\includegraphics[width=1\columnwidth]{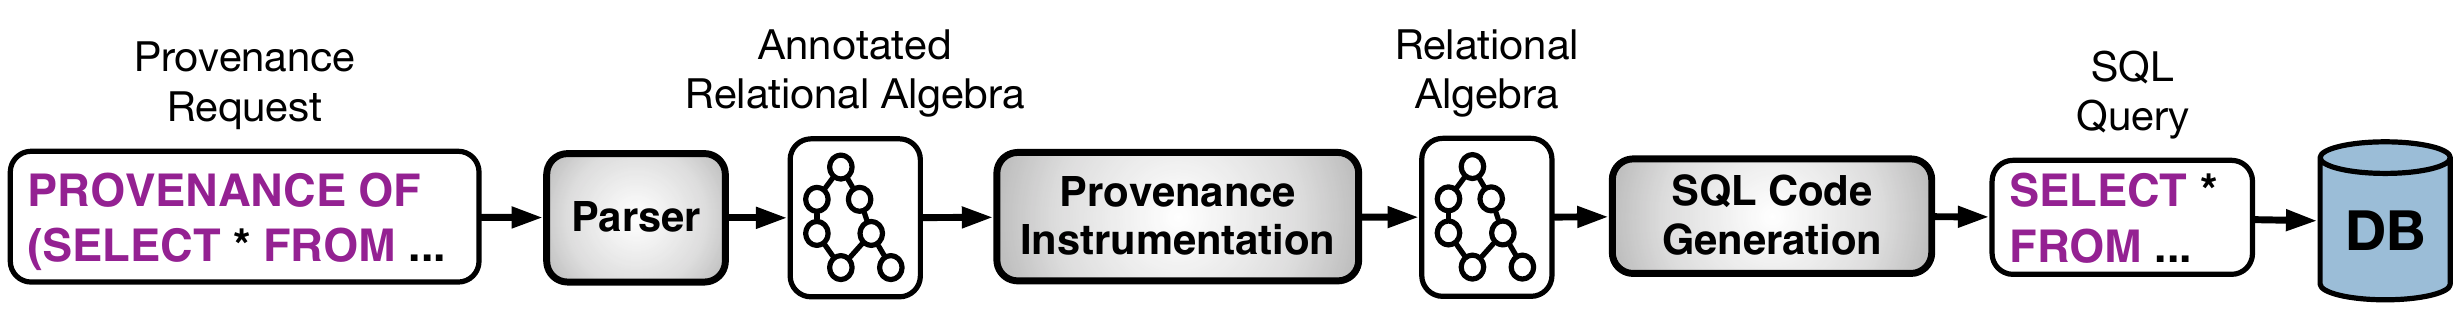}
  \caption{Rewrite-based Approach for Provenance Computation}
  \label{fig:general-rewrite-approach}
\end{figure}
%%%%%%%%%%%%%%%%%%%%%%%%%%%%%%%%%%%%%%%%
%%%%%%%%%%%%%%%%%%%%%%%%%%%%%%%%%%%%%%%%
\begin{figure}
\centering
\includegraphics[width=0.7\columnwidth]{figs/new_architecture.pdf}
\caption{GProM Architecture}
\label{fig:GProm-arch}
\end{figure}
%%%%%%%%%%%%%%%%%%%%%%%%%%%%%%%%%%%%%%%%

The above example, illustrates the general idea of representing provenance as annotations on data, encoding these annotations using the standard relational model, and computing this representation by executing a query in a standard relational query language. As mentioned earlier this approach is applied by many relational provenance systems. For instance, another example is the DBNotes system where annotations at the attribute level are propagated according to the Where-provenance~\cite{CC09} model introduced by Buneman and Tan. 

While the query used for provenance computation in Ex.~\ref{ex:simple-prov-ex} is rather straightforward and is likely to be optimized in a similar fashion as the input query, this is not true for more complex provenance computations. In the following we present examples for such complex expressions and explain why they are hard to optimize, even for sophisticated query optimizers such as the ones found in commercial systems. In the following we will consider a rewrite-based provenance approach as shown in Fig.~\ref{fig:general-rewrite-approach} where incoming provenance requests are compiled into relational algebra graphs (we use graphs instead of trees because they enable explicit encoding of reuse of subexpressions) which are then transformed into SQL (or any other suitable query language) and executed by a backend database system. The optimization framework we develop in this work is applicable to this generic framework and variations thereof (e.g., even if another intermediate compilation step is added this does not effect the applicability of the approach). We implement this general framework in GProM (see Fig.~\ref{fig:GProm-arch}), our generic provenance middleware that can run over multiple backend systems (including Oracle and PostgreSQL) and supports different frontends.  The default frontend of the system provides an extension of SQL with provenance requests, but a proof-of-concept datalog frontend also exists. All frontends translate queries in the frontend language into relational algebra graphs that are used as a universal intermediate language for representing computations. These algebra graphs are translated into the backend database's SQL dialect using a backend specific code generation module.

% As mentioned before, GProM also supports provenance computation for transactions. 
% If user want to request the provenance for a transaction $T$, the transaction
%   reenactor of GProM extracts the list of SQL statements executed by $T$ from the audit log of the backend database
%   and constructs a reenactment query $q(T)$ that simulates the effects of these
%   statements. We use the provenance rewriter to rewrite $q(T)$ into a query
%   $q(T)+$ that computes the provenances of the reenacted transaction.

%%%%%%%%%%%%%%%%%%%%%%%%%%%%%%%%%%%%%%%%
\newsavebox{\transactionExOne}
\begin{lrbox}{\transactionExOne}
\begin{lstlisting}
UPDATE R SET A=A-5 WHERE B=2;
UPDATE R SET A=A+1 WHERE B=1;
COMMIT;
\end{lstlisting}
\end{lrbox}

%%%%%%%%%%%%%%%%%%%%%%%%%%%%%%%%%%%%%%%%
\newsavebox{\transactionProv}
\begin{lrbox}{\transactionProv}
\begin{lstlisting}
SELECT CASE WHEN B=1 THEN A+1 
            ELSE A 
       END AS A, 
       B
FROM (SELECT CASE WHEN B=2 THEN A-5 
                  ELSE A 
             END AS A, 
             B
      FROM R);
\end{lstlisting}
\end{lrbox}

%%%%%%%%%%
\begin{figure}[t]
\centering

\subfloat[Example Transaction $T_1$]{
\centering
\usebox{\transactionExOne}
}

%\BG{Correct the graph}

\subfloat[Relation $R$ before and after Transaction $T_1$]{
\centering
  \begin{minipage}{0.45\linewidth}
\centering
  Before $T_1$\\[2mm]
  \begin{tabular}{|c|c|} \hline 
  \rowcolor[gray]{.9}  A & B\\ \hline 
  2 & 1   \\ \hline
  3 & 2   \\ \hline
  4 & 2   \\ \hline
  \end{tabular}  
  \end{minipage}
  \begin{minipage}{0.45\linewidth}
  After $T_1$\\[2mm]
      \begin{tabular}{|c|c|} \hline 
  \rowcolor[gray]{.9}  A & B\\ \hline 
  3 & 1   \\ \hline
  -2 & 2   \\ \hline
  -1 & 2   \\ \hline
  \end{tabular}
  \end{minipage}
}

\subfloat[Simplified Provenance Computation for $T_1$]{
\begin{minipage}{1.0\linewidth}
\centering
\usebox{\transactionProv}
  % \begin{tikzpicture} [op/.style={anchor=south west}, conn/.style={-}]

  %   \node[op] (p) at (0,2.6)
  %   {$\projection_{if(B=1)~then~A+1~else~A \rightarrow A, B}$}; 

  %   \node[op] (s) at (0,1.85) 
  %   {$\projection_{if(B=2)~then~A-5~else~A \rightarrow A, B}$};

  %   \node[op] (j) at (0,1.2) {$R$};

  %   \draw[conn] ($(p.south west) + (2.5mm,0)$) to
  %   ($(s.north west) + (2.5mm,0)$); \draw[conn] ($(s.south west) + (2.5mm,0)$)
  %   to ($(j.north west) + (2.5mm,0)$);

  % \end{tikzpicture}
\end{minipage}
}

%\BG{correct the data in the after table}
\caption{Simplified Transaction Provenance Computation}
\label{fig:Heuristic-example}
\end{figure}
%%%%%%%%%%%%%%%%%%%%%%%%%%%%%%%%%%%%%%%%

%%%%%%%%%%%%%%%%%%%%%%%%%%%%%%%%%%%%%%%%%%%%%%%%%%%%%%%%%%%%
\subsection{Motivating the Need for  Heuristic Optimization}
\label{sec:need-heuristic}

We motivate the need for heuristic optimizations by means of a simplified real world example we encountered in GProM when generating queries that retroactively compute the provenance of transactional updates (this approach called \textit{reenactment} was sketched in~\cite{arab2014generic}). This example illustrates the dire need for optimization, because the unoptimized query computing provenance has an execution time (we tested Oracle and PostgreSQL) that is infinite for all practical purposes while the optimized query runs in milliseconds.
% Because the provenance rewrite policy, the $q(T)^+$ we got is complex and
% redundant.  We need to optimize it before translate it to SQL expression and
% send the SQL expression into the database. 

%%%%%%%%%%%%%%%%%%%%%%%%%%%%%%%%%%%%%%%%%%
\begin{Example}\label{ex:ex-Heuristic} 
Fig.~\ref{fig:Heuristic-example}(a) shows an SQL transaction $T_1$ consisting of two updates. Fig.~\ref{fig:Heuristic-example}(c) shows the relation $R$ before and after executing transaction $T_1$.
When using GProM to retroactively compute the provenance of this transaction, the system would generate a so-called reenactment query which simulates the transaction's updates and then instruments this query to propagate provenance annotations. A simplified version of this query is shown in Fig.~\ref{ex:ex-Heuristic}(b).  If this query is run over the version of relation $R$ before the update, then the result will be the version $R$ produced by transaction $T_1$. 
Basically, each update is simulated by using the \lstinline!CASE! construct to update an attribute value if the update's condition is fulfilled. For a transaction with more than two updates there would be one such subquery for each update. While this query looks harmless enough and naively evaluating it without any optimization would be linear in the size of relation $R$ and the number of subqueries (updates of the transaction), this query will run in exponential time in the number of updates if executed using PostgreSQL or Oracle (and presumably other systems\footnote{For example, SQLite will throw an error because the maximum expression tree depth (1000) is reached.}). For PostgreSQL, since the source code is available we traced the cause of this problem: PostgreSQL will eagerly merge subqueries into a parent query if possible. This requires replacing references to attributes in the outer query with their definition in the inner query. For instance, in the example each reference to $A$ in the outer query will be replaced by the \lstinline!CASE! expression of the inner query. This case expression references $A$ twice. Thus, in the resulting expression the attribute $A$ from relation $R$ is referenced 4 times. While for two level this is not really a problem, consider what would happen if we would have $n$ instead of $2$ levels. The resulting 
expression size would be exponentially large (in $n$), because every merge step doubles the number of references to $A$. 
This problem may seem esoteric, but it turned out to be a major road blocker for implementing provenance tracking for transactions. In fact, many issues with optimizing provenance computations expressed in SQL are based on operator patterns that are uncommon enough to not be the focus of optimizer developers. 
The example problem can be solved by applying two heuristic rewrite rules. The first rule factors references to attributes in projection expressions. For instance, \lstinline!CASE WHEN B=2 THEN A+1 ELSE A END! can be rewritten as \lstinline!A + CASE WHEN B=2 THEN 0 ELSE 1 END!. After attribute factoring, subqueries can safely be merged in most cases. Furthermore, we determine when merging is unsafe and force the database to materialize intermediate results in this case. 
% One heuristic rule that I have implemented in GProM is factoring of attribute references to reduce the total number of references to attributes in projection expressions. Applied to, e.g., $if(B=1)~then~A+1~else~A$ we can factor the common reference to $A$ in the \textit{then} and \textit{else} branch to get $A + (if(B=1)~then~+1~else~0)$. 
%  If do not have optimizer, this query runs in linear time to the height and the size of the R. Normal database did not do
% a safity check, because not many people write write this kind of query.
\end{Example}
%%%%%%%%%%%%%%%%%%%%%%%%%%%%%%%%%%%%%%%%%

The above example demonstrates the need for heuristic optimizations. The rewrite rules in this example either simplify the query or are needed to avoid very bad plans. Rules that may improve performance and never degrade performance should be always applied if their preconditions are met, e.g., not all expression allow for attribute factoring. The heuristic optimization techniques we devise in this work consist of algebraic equivalence rules , some of which require inference of properties for operators in a query to test their preconditions. 
In additional to rules that are novel (or at least atypical) we also implement standard equivalences. The reason for implementing these standard rules (which may be applied in similar form by the database optimizer) is that it may be necessary to apply a standard rule to open up opportunities for applying our optimizer's novel rules.

%%%%%%%%%%%%%%%%%%%%%%%%%%%%%%%%%%%%%%%%%%%%%%%%%%%%%%%%%%%%
\subsection{Motivating the Need for Cost-based Optimization}
\label{sec:the-need-cost-based}

Heuristic rules are a great tool for simplifying provenance computations as well as rewriting them into a form that is easy to understand and optimize by standard database optimizers. 
However, this approach is not applicable if we have to choose between alternative ways of expressing a provenance computation and none of these choices is clearly superior. Ideally, we want to be able to make an informed choice based on which choice has the lower expected cost for the query at hand. 

%%%%%%%%%%%%%%%%%%%%%%%%%%%%%%%%%%%%%%%%%%
\begin{Example}\label{ex:ex-Cost-based} 
GProM implements two different ways of computing the provenance of an aggregation operator - one joins the aggregation result with the provenance of the aggregation's input on the group by attributes to pair each aggregation result with its provenance (we call this method \textit{join} in the following)  and the other one uses analytical functions (the \lstinline!OVER()! window definition in SQL) to compute the aggregation functions over provenance directly. There is no clear winner among these two methods,
their performance depends on the size of the input database, value distributions of attributes, and the structure of the query. Preferring one over the others using a heuristic rule will not be beneficial in this case.
A cost-based optimizer, however, can determine which method is better for an input query. Theoretically, a database optimizer could be able to determine that these two ways of expressing the provenance computation are equivalent. However, in practice we have not observed any optimizer to apply such equivalences. As we will demonstrate in the experimental evaluation, the cost of these two ways of computing the provenance of aggregation operators are significantly different. % (sometimes many orders of magnitude).
% our cost-based optimizer is capable of making the right choice.
% In this case, our optimization system can merge the projections or selections together. This is belong to the heuristic
% optimization. It through applying several optimization rules and try to simplify the complex query expression to a single query sentence. Maybe it is a long query sentence, 
% but its performance should better than the complex one. As usual, even thorough by applying somes rule it can get a good performance in 99\% cases, however, for some rules in some cases, 
% it is still unclear applying the rules is good or not. In this case, we need to apply the cost-based optimizaion. The cost-based optimizer send the rewritted query to the 
% Oracle and let Oracle determine which one can get the best performance. Another example of why we need the optimizer is that when doing the provenance rewriting, the provenance
% rewritter can have several ways to rewrite the query, we don't know which one can get a better performance. The normal database optimizer can't solve it. So we can let the
% cost-based optimizer to determine which way is the best.
\end{Example}
%%%%%%%%%%%%%%%%%%%%%%%%%%%%%%%%%%%%%%%%%%

The above example shows that there is a need for making cost-based decisions during rewriting (i.e., during the compilation step that turns a query with annotated semantics into a regular relational query). Thus, an optimizer is needed that can generate alternative plans based on this type of decisions. Furthermore, there may also be instances where we would want to apply algebraic transformations in a cost-based manner. That is, our optimizer should support both decisions at the rewriting stage, but also over the generated relational algebra expression. % \BG{Add Example}

%%%%%%%%%%%%%%%%%%%%%%%%%%%%%%%%%%%%%%%%%%%%%%%%%%%%%%%%%%%%
\subsection{Solution Overview and Contributions}
\label{sec:solut-overv-contr}

We now give a brief overview of our solution and present the main contributions of this work. The modified GProM architecture including our optimizer is shown in Fig.~\ref{fig:cbo-arch}. We make three main contributions in this work that will be discussed in more detail in the following: 

\begin{itemize}
\item We develop provenance-specific transformation rules that have the potential of significantly improving the performance of provenance computations. 

\item We develop a callback-based, non-invasive, cost-based optimization framework that is agnostic to the shape of the plan space and allows any type of optimization choices to be made with minimal changes to existing code.

\item We implement the framework and provenance specific optimizations in our database independent provenance middelware GProM (\textbf{G}eneric \textbf{Pro}venance \textbf{M}iddleware). We evaluate the effectiveness of the approach over several different provenance tasks and demonstrate that it is essential for achieving good performance (often improving performance by several orders of magnitude).
\end{itemize}

%%%%%%%%%%%%%%%%%%%%%%%%%%%%%%%%%%%%%%%%
\begin{figure}[t]
\centering
\includegraphics[width=1\columnwidth]{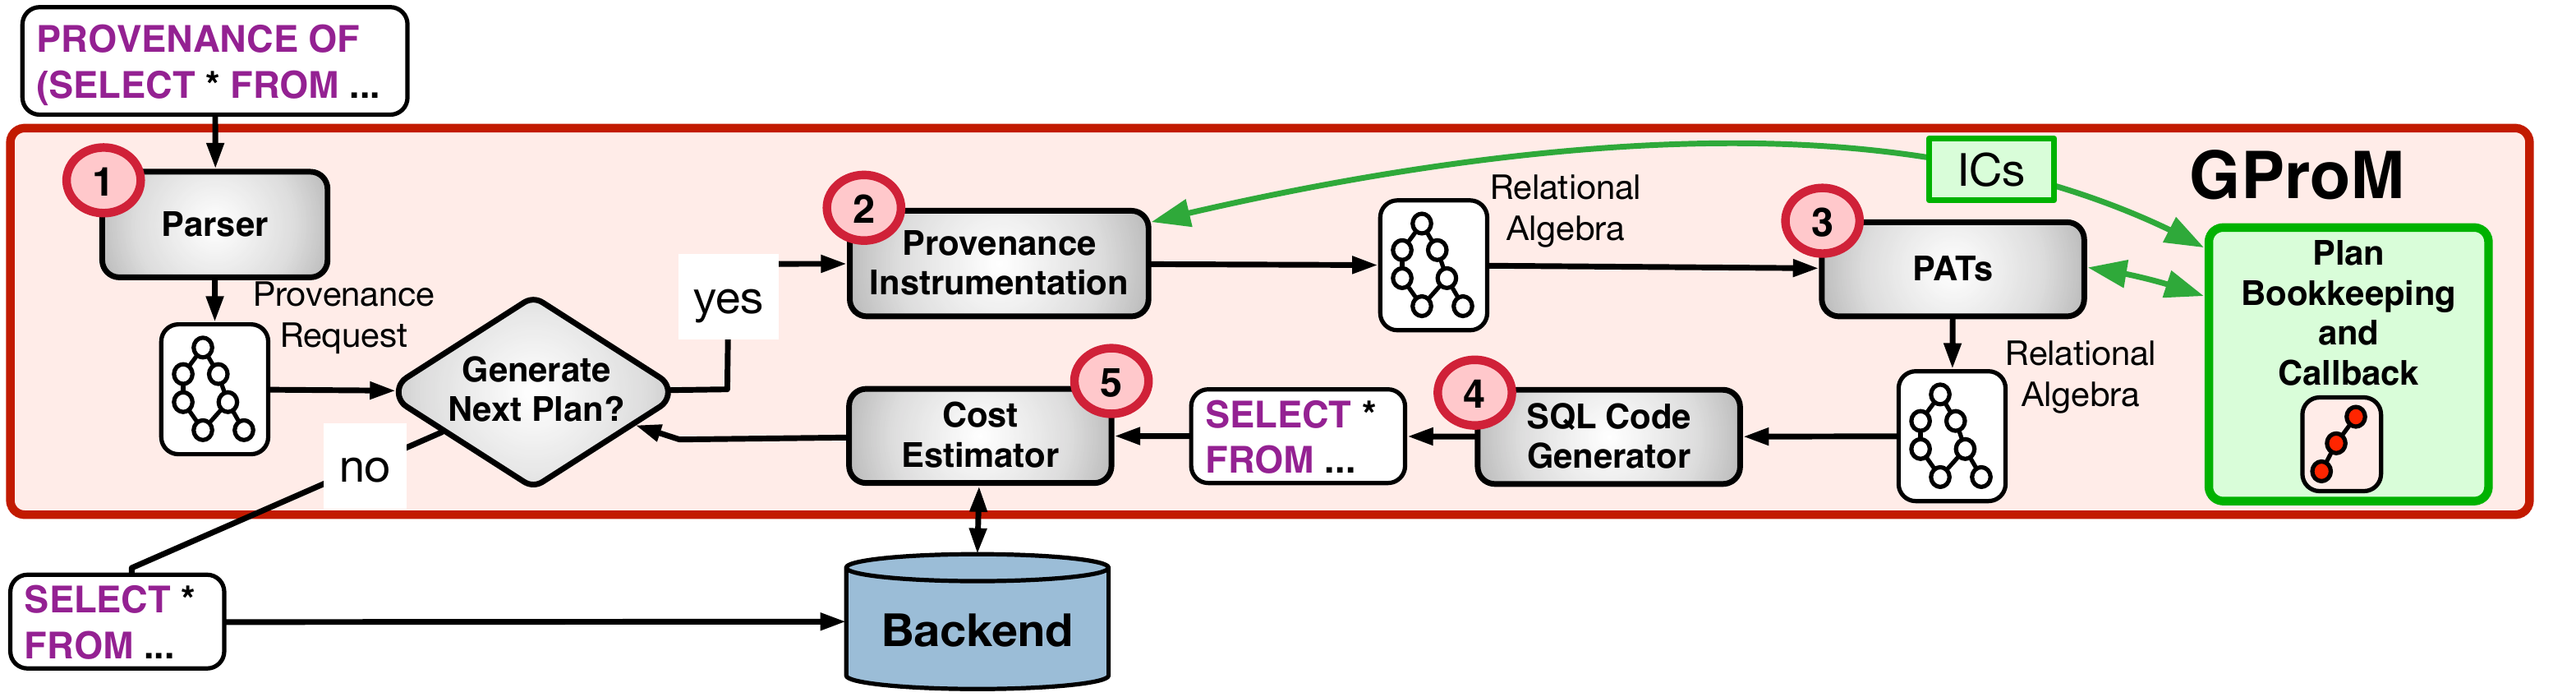}
\caption{GProM with Cost-based Optimizer}
\label{fig:cbo-arch}
\end{figure}
%%%%%%%%%%%%%%%%%%%%%%%%%%%%%%%%%%%%%%%%

%%%%%%%%%%%%%%%%%%%%%%%%%%%%%%%%%%%%%%%%
\parttitle{Provenance Specific Optimizations}
Our first major contribution is the development % of equivalence rules at the algebraic level as well as at the level of translation between the input language and relational algebra  (e.g., as in the join vs. window aggregation example) which are helpful to improve the performance of provenance computation.
 % We develop
of transformation rules based on algebraic equivalences targeted specifically at provenance tasks and transformation rules that exploit equivalent ways of expressing provenance computations.

We introduce two methods for the computing provenance of an aggregation operator: one that uses a join (this rule was first introduced in Perm~\cite{glavic2013using}) to combine the original aggregation with the provenance of the aggregation input and one which uses window functions to directly compute the aggregation functions over the input annotated with provenance. While the window method is often more performant than the join method, there are also cases where the oposite is true. Thus, cost-based optimization should be applied to chose between these methods. 

We present two methods for excluding unrelated tuples from the provenance computation early on when computing provenance for transactions. The first method filters tuples based on the conditions of the updates applied by a transaction. The other method determines which tuples were updated by the transaction by using a temporal database running a query over the version of the database after transaction commit (this is possible using a transaction identifier column available in most database that stores which transaction  created a tuple version) and then joins this set of tuples with the version of the database before transaction start to exclude tuples which did not get updated by the transaction.

We identify beneficial heuristic optimization rules which are usually not applied by database systems, but are very effective for speeding up provenance computations. For instance, these include factoring of references to attributes in projection expressions to enable safe merging of projections without blow-off in expression size (as shown in Fig.~\ref{fig:Heuristic-example}, pull up projections that duplicate attribues to create provenance annotations, and removal of unnecessary duplicate removal operators and window functions (SQL \lstinline!OVER! clause).
Following the approach presented in ~\cite{grust2010let} we infer properties such as  candidate keys  for each operator in an algebra graph. These properties are used as preconditions in algebraic equivalences. This has the advantage of simplifying the algebraic rewrite rules, because the definition is divided into two simpler parts, and  it allows us to check non-local information in the rules. For example, we can delete a duplicate removal operator if its result is subjected to duplicate removal downstream from the operator. Unlike, e.g., commutativity of joins which can be represented as a small localized rewrite, expressing such a rule as an algebraic rewrite would be cumbersome, because we cannot make any assumption about what and how many operators are on the path from the operator to the next duplicate removal operator.

%%%%%%%%%%%%%%%%%%%%%%%%%%%%%%%%%%%%%%%%%%%%%%%%%%%%%%%%%%%%
\parttitle{Cost-based Optimization Framework}
Our second contribution is the development of a general framework for cost-based optimization. Fig.~\ref{fig:cbo-arch} gives an overview of our framework and how it is implemented with GProM.  While our approach is similar to cost-based query transformation that has been studied extensively, it has several unique characteristics that distinguish it from previous work. First of, our optimizer is \textbf{plan-space agonistic}. In fact it is only made aware of optimization choices at run-time through a \textbf{callback interface}. That is, the optimizer repeatedly calls the provenance rewriter and SQL code generator to produce an SQL query that is costed using the backend database system. The provenance rewriter and SQL code generator are responsible for informing the optimizer about available optimization choices using the callback interface. We refer to components that use the optimizer as \textit{clients}. The optimizer responds to a call from a client by instructing the client which of the available alternatives to choose. During each pass from provenance request to SQL statement (we call this an \textbf{iteration}), the optimizer keeps track of which choices had to be made (we call this \textbf{choice points}), which alternative options were available for each choice, and which alternatives were chosen. This information is sufficient to iteratively enumerate the whole plan space by making different choices during each iteration. Since costing a plan requires the database backend to optimizing a query, the number of alternative queries that can compared by our optimizer within reasonable time is limited. In addition to exploring traditional randomized search approaches, we also support an approach that balances optimization vs. execution time, i.e., the approach keeps track of how much time has been spend on optimization so far and  the expected runtime of the current best plan and will stop optimization when optimization time exceeds expected runtime. Under the assumption that cost is estimated correctly, this guarantees that our approach will never spend more than twice the amount of time as an approach that knows upfront when to stop the optimization process to minimize the sum of execution time and optimization.

Our approach provides a great level of flexibility in what types of optimization decision can be supported. For example, optimization choices can be made early on while constructing a query that implements a provenance request, i.e., we can make choices before any relational algebra expression has been constructed. These types of choices may completely alter the resulting algebra expression, so expressing them as transformation rules over relational algebra expressions would be complicated since it would require to write a transformation rule that affects large parts of a potentially large algebra expression (and to develop a mechanism to pass the information about the applicability of this rewrite from the provenance rewriter to the algebraic optimization stage). In constrast, using our approach this only requires adding a few lines of code in the provenance rewriter to inform the optimizer about the availability to choose among alternative options. This kind of choices are not limited to deciding among alternative ways of expressing a provenance computation (as in Ex.~\ref{ex:ex-Cost-based}) and whether to apply an algebraic equivalence transformation, but can also be used to control strategies for applying rules. For instance, if we have a set of transformation rules that result in a different query if applied top-down or bottom-up to an input algebra graph, we can use the optimizer to choose among a top-down and bottom-up application strategy. Other examples of strategic decisions that can be encoded as optimization choices in our framework are application order of algebraic equivalence transformations or number of iterations if an algebraic transformation can be applied repetitively.

% We present the first optimizer for rewrite-based provenance approaches. Our optimizer applies both heuristic and cost-based rules to optimize provenance computations for execution on a relational database.

Similar to cost-based query transformation, our approach coexists with the database optimizer: we use the database optimizer to benefit from decades of research on relational query optimization where it is effective (e.g., join reordering) and use our optimizer to address the database optimizer's shortcomings with respect to provenance computations. For example, we rewrite queries to fit the database system's expectations and, thus, enable the database system to successfully optimize them. Furthermore, we use our optimizer to choose among alternative ways of expressing a provenance computation which are not recognized as equivalent, even by sophisticated database optimizers.

%%%%%%%%%%%%%%%%%%%%%%%%%%%%%%%%%%%%%%%%
\parttitle{Implementation and Experimental Evaluation}
We have implemented our provenance optimization techniques and the cost-based optimization framework in the GProM generic provenance middleware and evaluate their effectiveness over different types of provenance computation tasks focusing on provenance computation for queries and transactions. Our experiments confirm that using our approach we can significantly improve efficiency for different types of rewrite-based provenance computations. The provenance-specific optimizations are often necessary to get reasonable performance even for small database instances. In fact, the inacceptable performance of rewritten queries was the main motivation for this work.

The remainder of this paper is organized as follows. We present background in Sec.~\ref{sec:background}. Related work is covered in Sec. ~\ref{sec:relatedwork}.
The provenance-specific optimizations and the cost-based optimization framework are presented in Sec.~\ref{sec:heuristic} and~\ref{sec:cbo}, respectively. The experimental 
evaluation of our work is discussed in Sec.~\ref{sec:experiments}. We conclude in Sec.~\ref{sec:conclusion}.

%%%%%%%%%%%%%%%%%%%%%%%%%%%%%%%%%%%%%%%%
%\begin{figure}[!htb]
%\centering
%\BG{Replace this later with latex code to make it easier to change}
%\includegraphics[width=0.4\textwidth,bb=50 0 500 300]{figs/Picture1.jpg}
%\caption{Example database}
%\label{fig:digraph}
%\end{figure}
%%%%%%%%%%%%%%%%%%%%%%%%%%%%%%%%%%%%%%%%

%%% Local Variables:
%%% mode: latex
%%% TeX-master: "2016-prov-optimizer"
%%% End:
