# Supplementary material for: Optimizing Provenance Computations
Source: arXiv:1701.05513 source file (2017-01-19)
Supplement: Supplementary file 5 [file appendix-oldintro.tex]

\section*{Old Intro}
\label{sec:old-intro}

%%%%%%%%%%%%%%%%%%%%%%%%%%%%%%%%%%%%%%%%%%%%%%%%%%%%%%%%%%%%
\subsection{Requirements for the Optimizer}
\label{sec:requirements}

We now discuss our requirements for our optimizer for provenance computations as well as our proposed solution and contributions.

\begin{itemize}
\item \textbf{R1}: 
Optimizer should be non-invasive, in the sense, that new optimization choices can be added inside a component such as the provenance rewriter without requiring major modifications to this components. 

\item \textbf{R2}: 
We want to stop the cost-based optimizaion at anytime to balance the optimization and query cost in case the optimizaion takes too much time. 

Anytime (we can stop anytime and execute the current plan):If there are only few plans, it is fine. Just comparing each plan  don't take too much time. But it is possible there are millions of plans, we can't compare every one, it will consume too much time. 
%Thus we need to balance optimization and query cost. 

\item \textbf{R3}: 
%Can use DB optimizer for cost estimation (i.e., plans have to be SQL queries) The result after our optimization are still SQL queries.
The optimizer should be able utilize the database optimizer as the cost estimation model. 

\item \textbf{R4}: 
We want to minimize the time spend on optimization plus the time for executing the query. 
%Goal is to minimize $T_{opt} + T_{exe(P_{best})}$ $T_{opt}$. means the time used to optimize the query where the $T_{exe(P_{best})}$ means the query execution time.
\end{itemize}

 Not specific to a particular provenance model and approach: It should be possible to use the optimizer for a wide range of provenance model and techniques. Note that we explicitly expect task specific optimization rules, but it should be easy to add new rules specific to a task and integrate them with existing rules

 The optimizer should be search space agnostic, i.e., adding new optimization choices should not require modifications to the optimizer

 Peaceful co-existence with a database optimizer: The optimizer should avoid application of heuristic rules that hinder optimization or are likely to be undone by the database optimizer. For instance, it would be pointless to attempt to fix a certain join order in the SQL query send to the database backend, because the database optimizer will explore all (or most) possible join orders anyways. As an example of an heuristic rewrite with potentially negative effects, consider a rule that inserts 

Enable optimization during the compilation process and

%%%%%%%%%%%%%%%%%%%%%%%%%%%%%%%%%%%%%%%%%%%%%%%%%%%%%%%%%%%%
\subsubsection{Cost-based Optimization}\label{sec:cbo}

% \BG{
% Want to make informed choices between different options for computing provenance, i.e., cost-based choices. The DBMS optimizer does this already for the SQL queries we generate, but is often not successful because these queries are unusual (refer back to intro where there should be examples for that). 

% \textbf{Desiderata for optimizer:}

% \textbullet Non-invasive (make cost based choices in any component related to query rewrite with minor modifications (tell the optimizer about it).

% \textbullet Anytime (we can stop anytime and execute the current plan): balances optimization and query cost

% \textbullet Can use DB optimizer for cost estimation (i.e., plans have to be SQL queries)

% \textbullet Goal is to minimize $T_{opt} + T_{exe(P_{best})}$
% }

The basic idea of cost-based optimization is to evaluate each plan and get the lowest cost plan to execute. Each plan is constructed by two parts: one part is want to make informed 
choices between different options for implementing provenance computation. The second part is determining which heuristic rules to apply. 

Starting from what we get from the parser, we can doing the provenance rewriting and the heuristic optimizaion. We can make choices between alterative ways of computing provenance of certain operators as well as the whether we want to apply certain heuristic optimization or not. For one of this process the choices we take in the end determine what plan we get. Eventually we want to look at different plans generated by taking different choices. 

The requirement for our cost-based optimizer are:

Estimating the cost of queries has a long tradition in databases and database systems apply quite sophisticated methods to estimate the cost of alterative plans for executing a user query. Trying to replicate this functionality in our middleware would be tedious. Even more important, there is no one cost for a given SQL query, because the cost will vary dramatically across different plans for this query. Thus, to be able to compute a meaning full cost estimate for queries we would have to effectively implement a fully fledged database optimizer in our system - which is not possible within the scope of a research project. Finally, our cost model would differ from the database backends cost model and, thus, what we believe to be the lowest cost plan may not be the plan that is chosen by the backend database. Our solution to this problem is to let our cost-based optimizer generate alternative SQL queries and use the database backend's optimizer to generate the best plan for each query and give us a cost estimate. We then execute the query with the lowest estimated cost. The only drawback of this approach is that the overhead we pay per generated query is to high to allow for an exploration of a large plan space. We address this problem by 1) only make choices where the choice is likely to significantly affect runtime and 2) by stopping optimization when the ratio between time spend on optimization and expected run time of the current best plan becomes to large. Since, we wanted to integrate cost-based choices with existing rewrite code (and future rewrite methods) one major goal in developing the cost-based optimizer was to minimize the change to existing code. Our optimizer runs independently of the rewrite code and only require changes of a few lines of code to register a new choice.

%%%%%%%%%%%%%%%%%%%%%%%%%%%%%%%%%%%%%%%%%
\subsubsection{External Query Rewrite Optimization Problem}
%\BG{State what input is, given an input query and set of choice points assume a function $g$ (generatePlan) exists that generates plans by making choices that have not been explored before. Let $P_i$ be the plan generated by the $i^{th}$ call to generatePlan. Assume we know the cost $T_{exp}(P)$ (time needed to execute the plan) of each plan $P$ and there is a cost associated with calling generatePlan. For simplicity assume that generateNext has a fixed cost $c$.

%\textbullet We want to minimize $T_{exp}(P) + T_{opt}$ where $T_{opt} = n \times c$ where $n$ is the number of times we have called generatePlan. 

%\textbullet Then state this is an online problem (as you do)

%\textbullet Then definition of the online query rewrite optimization problem. Find 

%}

Given an input query and set of choice points, we use the function $g$ (generatePlan) to generates plans by making choices that have not been explored before. 
Let $P_i$ be the plan generated by the $i^{th}$ call to generatePlan. Assume we know the cost $T_{exp}(P)$ (time needed to execute the plan) of each plan $P$ and 
there is a cost associated with calling generatePlan. For simplicity assume that generateNext has a fixed cost $c$. 
Our goal is to minimize $T_{exp}(P) + T_{opt}$ where $T_{opt} = n \times c$ where $n$ is the number of times we have called generatePlan. 
This is an online problem: they model, in particular, that the input in an iteractive system does not arrive as a batch but as a sequence of input portions and that the 
system must react in response to each incoming portion. Moreover, they take into account that at any point in time future input is unknown\cite{onlinep}. 
We define our online query rewrite optimizaion problem in Definition~\ref{online-query-rewrite-opt-prom}.

\begin{Definition}\label{online-query-rewrite-opt-prom}
 \begin{align*}
 &\operatorname*{arg\,min}_{n}(\min_{i \in \{1,n\}}(T_{exp}(P_i)) + T_{opt})\\
 &T_{opt} = n \times c
 \end{align*}
\end{Definition}

For this problem, we aim to minimize the time for optimization plus the time for executing the query.
We know this is online problem, after each generate plan, we make choice either executing the current best plan or continue to generate a new plan. However, if we continue, we do not know whether the additional plans we explore will be cheaper or not.
For online algorithm, the exists the concept of competitiveness, algorithm is called N competitive if the solution that produces is at most N time worse, the best solution algorithm can produce the full knowledge of the fulture~\cite{online}.
%The problem we are considering here is that we have input query and some choice points in rewrite which means we have alternative way to rewrite the query where multiple choice points maybe applicatable to query.  
%Based on choosing different choice to use in each choice point, we can generate multiple different plans which have different cost. Our object is to look for algorithm to find the best plan to minimize the total cost(the optimization cost plus the query executing cost). 
%We call this problem here is the external query rewrite optimization problem.

%%% Local Variables:
%%% mode: latex
%%% TeX-master: "2016-prov-optimizer"
%%% End:
