# Supplementary material for: Optimizing Provenance Computations
Source: arXiv:1701.05513 source file (2017-01-19)
Supplement: Supplementary file 6 [file appendix_no_used_experiment.tex]

\begin{table*}
\centering
  \begin{tabular}{|c|r|r|r|r|r|} \hline 
\rowcolor[gray]{.9}  Queries & NoOpt+Join & Opt+Join & NoOpt+Window & Opt+Window & Cost+Opt\\ \hline 
TPC-H 1G & 173053.17 & 199.62 & 173041.27 & 250.18 &  235.79 \\ \hline 
TPC-H 10G & 175371.02 & 2033.71 & 175530.53 & 2247.39 & 2196.01 \\ \hline 
SAgg 1G & 4.79 & 20.21 & 4.38 & 2.69 & 0.81 \\ \hline 
SAgg 10G & 44.06 & 524.78 & 42.62 & 27.47 & 7.65\\ \hline 
Export 10M & 310.49 &  0.25 & & & 0.25  \\ \hline 
Export 100M & 3136.93 & 0.27 & & & 0.26 \\ \hline 
Export 1G & 21600 & 0.28 & & & 0.28   \\ \hline 
Export 10G & 21600 & 3.03 & & & 3.029 \\ \hline 
GameProvenace & 583.96 & 736.50 &  &  & 437.75 \\ \hline 
HSU/T & 55.11 & 69.50 &  & 8.91034945 & 8.96 \\ \hline 
TAPU & 30.13 & 26.08 &  & 12.98 & 12.89 \\ \hline 
  \end{tabular}
\caption{Overview : Sum Performance Relative to Best}
\label{tab:overview-sum}

\end{table*}
%%%%%%%%%%%%%%%%%%%%%%%%%%%%%%%%%%%%%%%%

%%%%%%%%%%%%%%%%%%%%%%%%%%%%%%%%%%%%%%%%
\begin{table*}
\centering
  \begin{tabular}{|c|r|r|r|r|r|} \hline 
\rowcolor[gray]{.9}  Queries & NoOpt+Join & Opt+Join & NoOpt+Window & Opt+Window & Cost+Opt\\ \hline 
TPC-H 1G & 173053.17 & 199.62 & 173041.27 & 250.18 &  235.79 \\ \hline 
TPC-H 10G & 175371.02 & 2033.71 & 175530.53 & 2247.39 & 2196.01 \\ \hline 
SAgg 1G & 4.79 & 20.21 & 4.38 & 2.69 & 0.81 \\ \hline 
SAgg 10G & 44.06 & 524.78 & 42.62& 27.47 & 7.65 \\ \hline 
  \end{tabular}
\caption{Overview : Sum Performance Relative to Best SimpleAgg and TPC-H}
\label{tab:overview-sum-sagg-tpch}
\end{table*}
%%%%%%%%%%%%%%%%%%%%%%%%%%%%%%%%%%%%%%%%

\clearpage

%%%%%%%%%%%%%%%%%%%%%%%%%%%%%%%%%%%%%%%%
\begin{table*}
\centering
  \begin{tabular}{|c|r|r|r|r|} \hline 
\rowcolor[gray]{.9}  Queries & FilterUpdated+NoOpt & HistJoin+Opt & FilterUpdated+Opt & Cost+Opt\\ \hline 
HSU/T & 55.11 & 69.50 &  8.91 & 8.96 \\ \hline 
TAPU & 30.13 & 26.08 & 12.94 & 12.89 \\ \hline 
  \end{tabular}
\caption{Overview : Sum Performance Relative to Best Transactions}
\label{tab:overview-sum-transaction}

\end{table*}
%%%%%%%%%%%%%%%%%%%%%%%%%%%%%%%%%%%%%%%%

%%%%%%%%%%%%%%%%%%%%%%%%%%%%%%%%%%%%%%%%
\begin{table*}
\centering
  \begin{tabular}{|c|r|r|r|} \hline 
\rowcolor[gray]{.9}  Queries & NoOpt & Opt & Cost+Opt \\ \hline 
Export 10M & 310.49 &  0.25&  0.25 \\ \hline 
Export 100M & 3136.94 & 0.27 &  0.26  \\ \hline 
Export 1G & 21600 & 0.28 &  0.28   \\ \hline 
Export 10G & 21600 & 3.03 &  3.01  \\ \hline 
GameProvenace & 583.96 & 736.50 & 437.75 \\ \hline 
  \end{tabular}
\caption{Overview : Sum Performance Relative to Best Export and Game Provenance}
\label{tab:overview-sum-export-gp}

\end{table*}
%%%%%%%%%%%%%%%%%%%%%%%%%%%%%%%%%%%%%%%%

%%%%%%%%%%%%%%%%%%%%%%%%%%%%%%%%%%%%%%%%
\begin{table*}
\centering
  \begin{tabular}{|c|r|r|r|r|r|} \hline 
\rowcolor[gray]{.9}  Queries & NoOpt+Join & Opt+Join & NoOpt+Window & Opt+Window & Cost+Opt\\ \hline 
TPC-H 1G & 1  & 0.18673  & 0.95545 & 0.22028 &  0.20337 \\ \hline 
TPC-H 10G & 1  & 0.19831 & 0.97512 & 0.17962 & 0.17359 \\ \hline 
SAgg 1G & 1 & 3.92735 & 0.94562 & 0.60015 & 0.26071 \\ \hline 
SAgg 10G & 1 & 9.14778 & 0.98444 & 0.65539 & 0.26549 \\ \hline 
Export 10M & 1 & 0.00082 &  &  & 0.00081 \\ \hline 
Export 100M & 1 & 8.49555E-05 &  &  & 8.44245E-05 \\ \hline 
Export 1G & 1 & 1.31823E-05 &  &  & 1.31874E-05 \\ \hline 
Export 10G & 1 & 0.00014 &  &  & 0.00014 \\ \hline 
GameProvenace & 1 & 1.95320 &  &  & 1.31972 \\ \hline 
HSU/T & 1 & 6.00826 &  & 0.66744 & 0.67033 \\ \hline 
TAPU & 1 & 1.77671 &  & 0.65361 & 0.65187 \\ \hline 
  \end{tabular}
\caption{Overview : Average Performance Relative to Best}
\label{tab:overview-avg}

\end{table*}
%%%%%%%%%%%%%%%%%%%%%%%%%%%%%%%%%%%%%%%%

\clearpage

%%%%%%%%%%%%%%%%%%%%%%%%%%%%%%%%%%%%%%%%
\begin{table*}
\centering
  \begin{tabular}{|c|r|r|r|r|r|} \hline 
\rowcolor[gray]{.9}  Queries & NoOpt+Join & Opt+Join & NoOpt+Window & Opt+Window & Cost+Opt\\ \hline 
TPC-H 1G & 1  & 0.187  & 0.955 & 0.220 &  0.203\\ \hline 
TPC-H 10G & 1  & 0.198 & 0.975  & 0.180 & 0.174 \\ \hline 
SAgg 1G & 1 & \cellcolor{green}3.927 & 0.946 & 0.600 & 0.261 \\ \hline 
SAgg 10G & 1 & \cellcolor{green}9.148 & 0.984 & 0.655 & 0.265 \\ \hline 
  \end{tabular}
\caption{Overview : Average Performance Relative to Best SimpleAgg and TPC-H}
\label{tab:overview-avg-simple-agg-tpch}

\end{table*}
%%%%%%%%%%%%%%%%%%%%%%%%%%%%%%%%%%%%%%%%

%%%%%%%%%%%%%%%%%%%%%%%%%%%%%%%%%%%%%%%%
\begin{table*}
\centering
  \begin{tabular}{|c|r|r|r|r|} \hline 
\rowcolor[gray]{.9}  Queries & FilterUpdated+NoOpt & HistJoin+Opt & FilterUpdated+Opt & Cost+Opt\\ \hline 
HSU/T & 1 & \cellcolor{green}6.008 & 0.667 & 0.670 \\ \hline 
TAPU & 1 & \cellcolor{green}1.777 & 0.654 & 0.652 \\ \hline 
  \end{tabular}
\caption{Overview : Average Performance Relative to Best Transactions}
\label{tab:overview-avg-transaction}

\end{table*}
%%%%%%%%%%%%%%%%%%%%%%%%%%%%%%%%%%%%%%%%

%%%%%%%%%%%%%%%%%%%%%%%%%%%%%%%%%%%%%%%%
\begin{table*}
\centering
  \begin{tabular}{|c|r|r|r|} \hline 
\rowcolor[gray]{.9}  Queries & NoOpt & Opt & Cost+Opt \\ \hline 
Export 10M & 1 & 0.00082 & 0.00081 \\ \hline 
Export 100M & 1 & \cellcolor{green}8.49555E-05 & \cellcolor{green}8.44245E-05 \\ \hline 
Export 1G & 1 & \cellcolor{green}1.31823E-05 & \cellcolor{green}1.31874E-05 \\ \hline 
Export 10G & 1 & 0.00014 & 0.00014 \\ \hline 
GameProvenace & 1 & \cellcolor{green}1.95320 & \cellcolor{green}1.31974 \\ \hline 
  \end{tabular}
\caption{Overview : Sum Average Relative to Best Export and Game Provenance}
\label{tab:overview-avg-export-gp}

\end{table*}
%%%%%%%%%%%%%%%%%%%%%%%%%%%%%%%%%%%%%%%%

%%%%%%%%%%%%%%%%%%%%%%%%%%%%%%%%%%%%%%%%%%%%%%%%%%%%%%%%%%%%
\begin{figure*}[t]
%%%%%%%%%%%%%%%%%%%%
  \begin{minipage}[b]{0.49\linewidth}
  \includegraphics[width=1\linewidth,trim=0 80pt 0 100pt, clip]{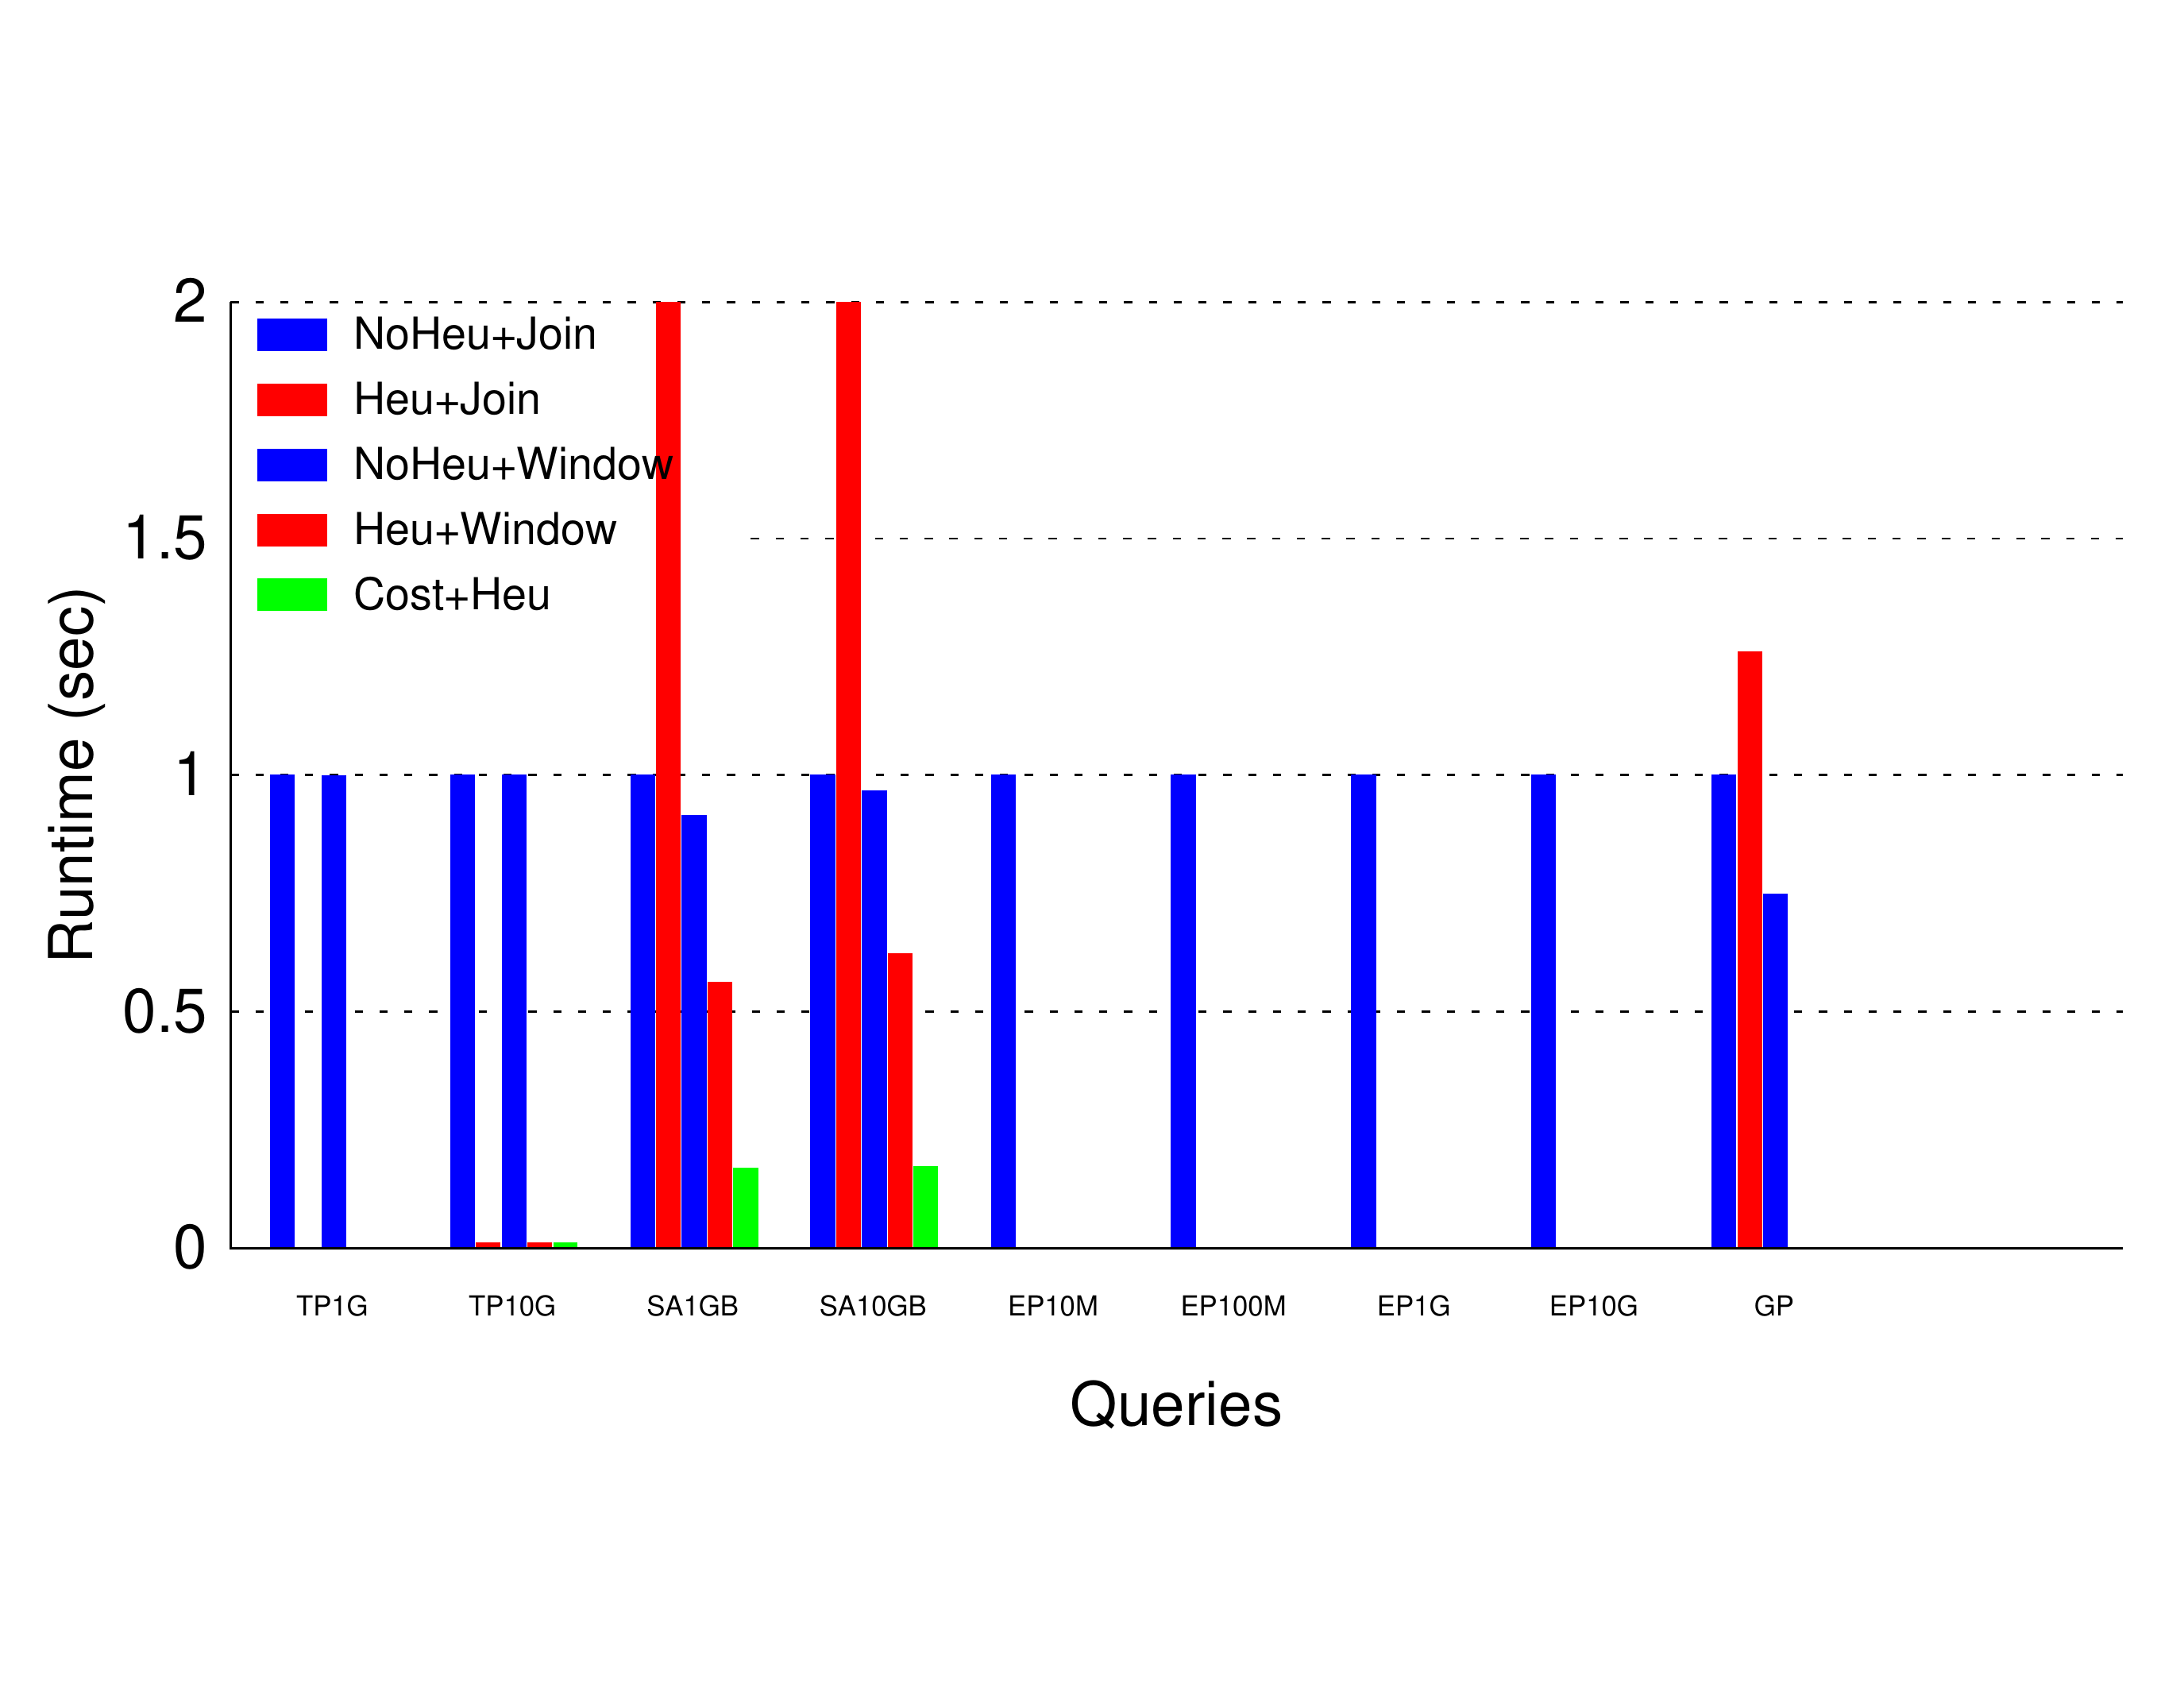}\\[-7mm]
  \caption{Overview : Sum Performance Relative to Best}
  \label{fig:overview-sum}  
  \end{minipage}
%%%%%%%%%%%%%%%%%%%
  \begin{minipage}[b]{0.49\linewidth}
  \includegraphics[width=1\linewidth,trim=0 80pt 0 100pt, clip]{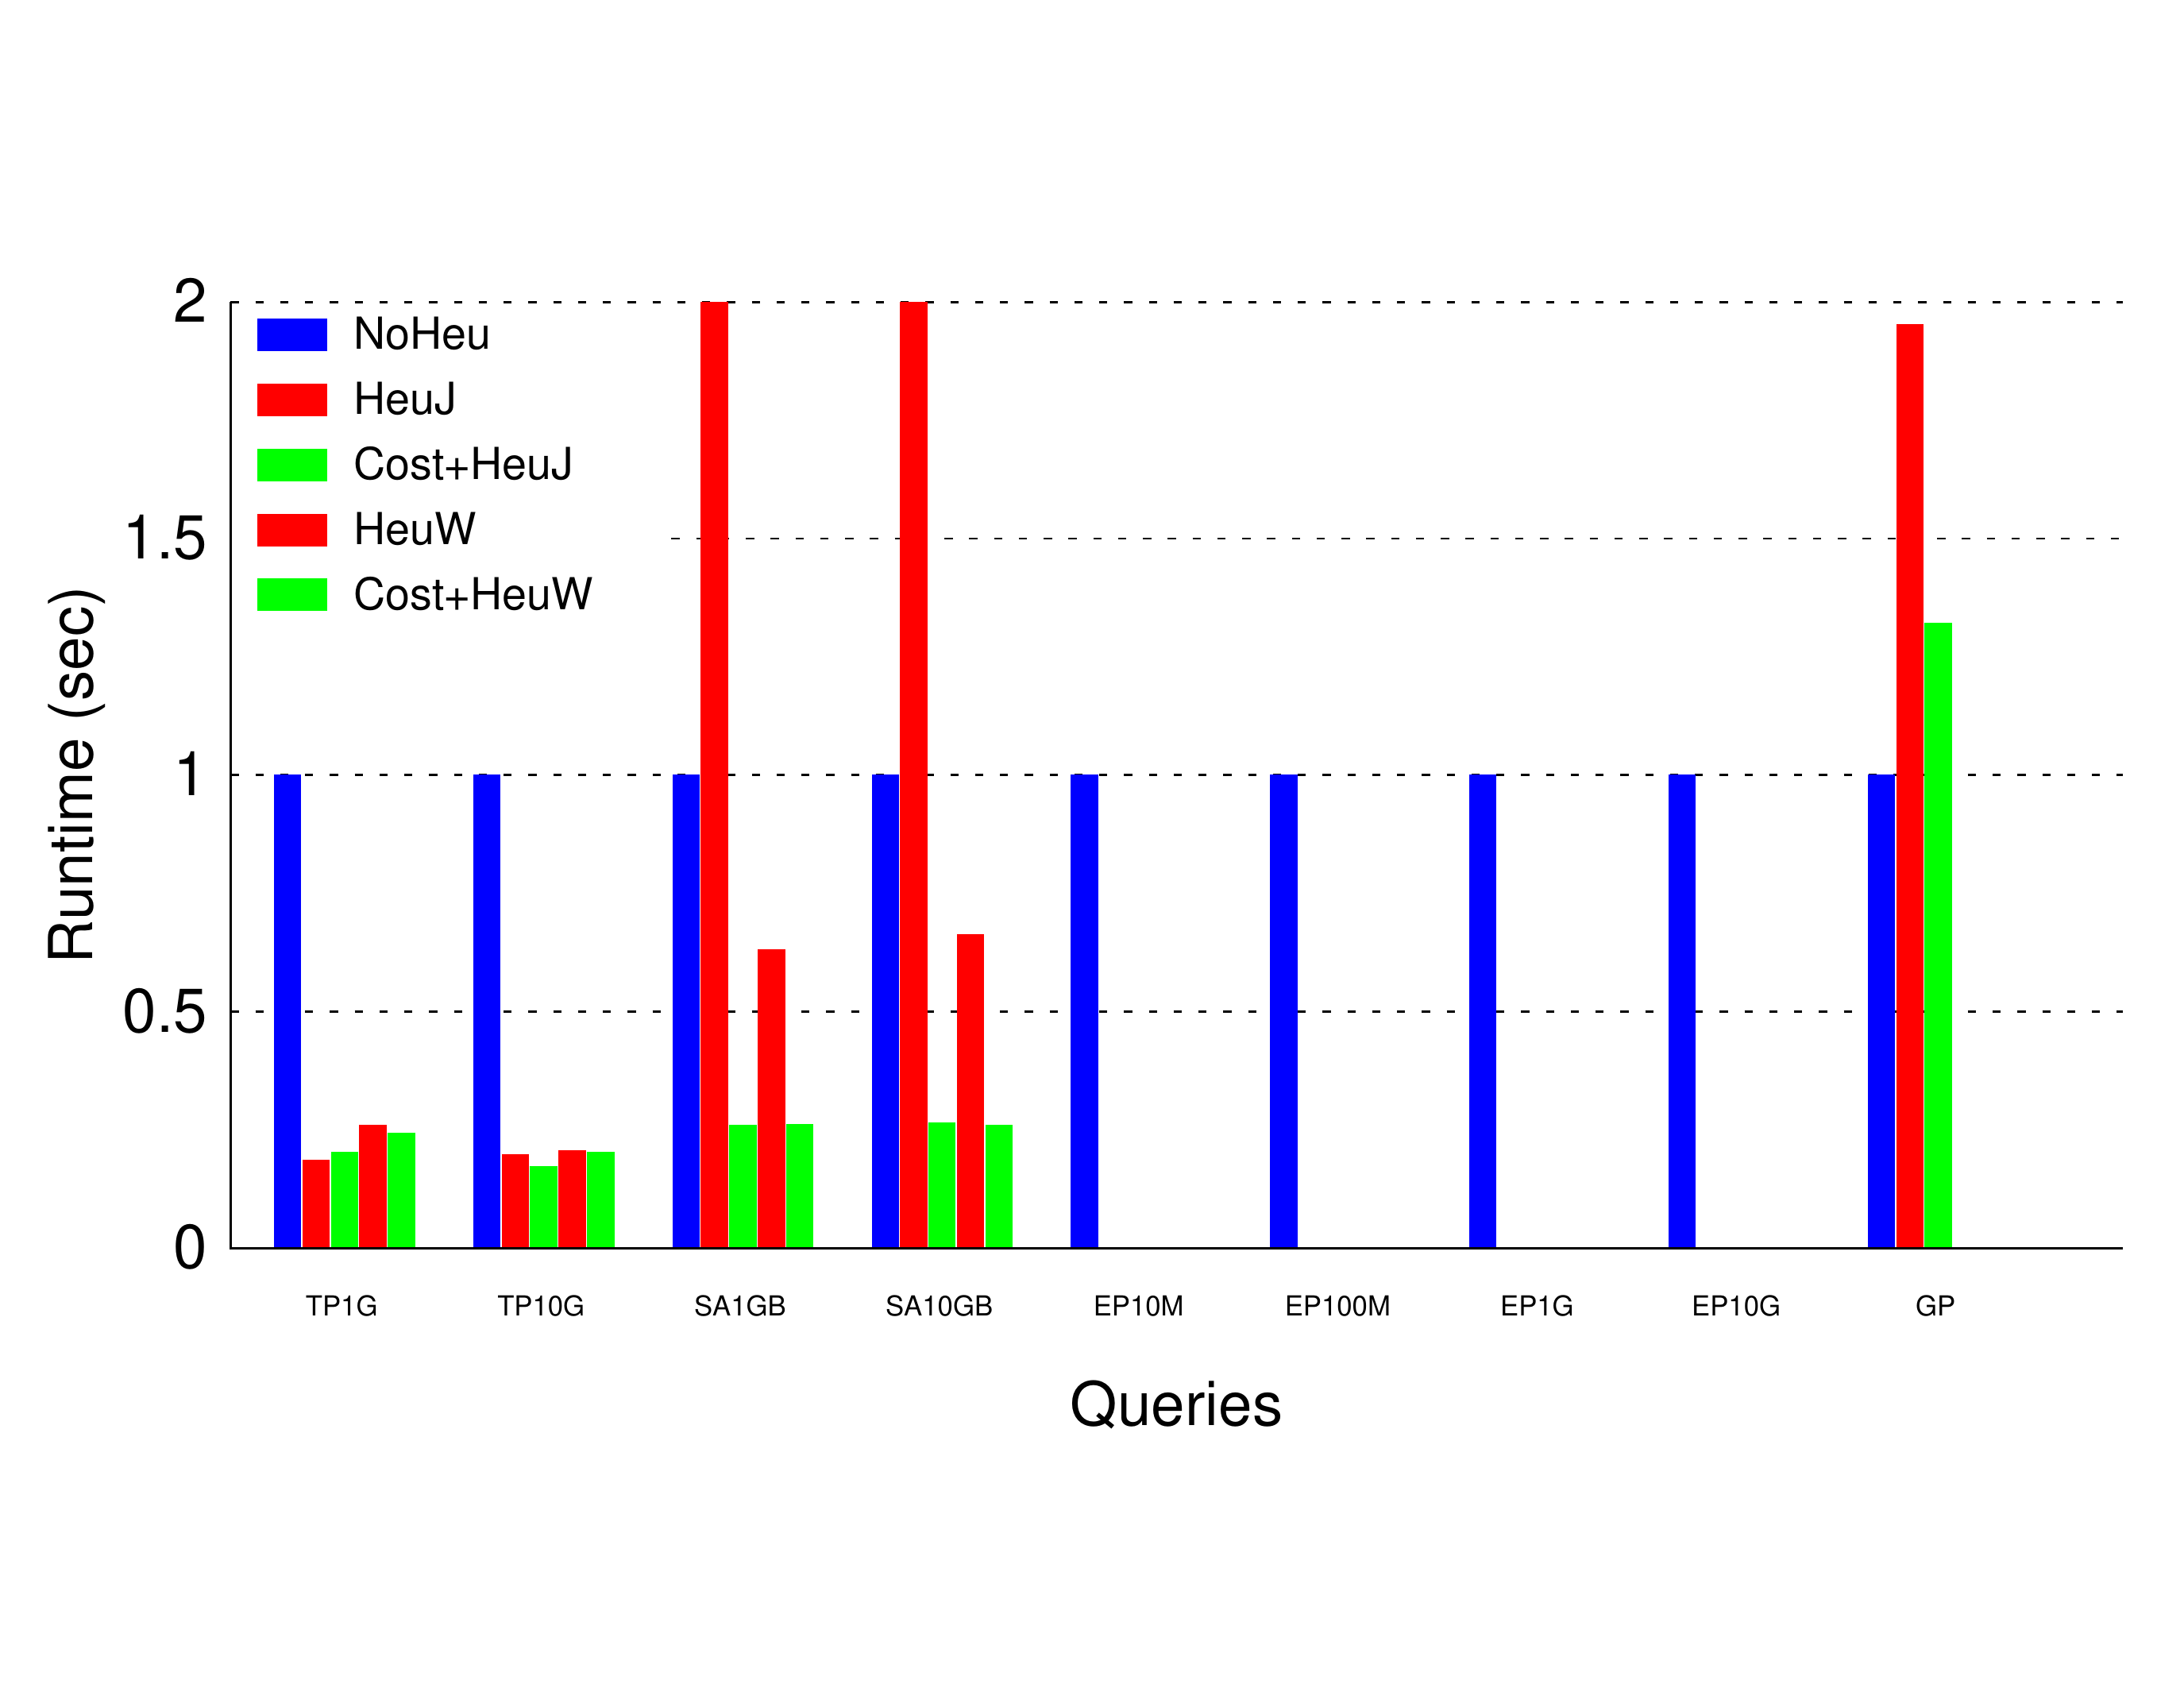}\\[-7mm] 
  \caption{Overview : Average Performance Relative to Best}
  \label{fig:overview-avg}
  \end{minipage}
\end{figure*}
% %%%%%%%%%%%%%%%%%%%%%%%%%%%%%%%%%%%%%%%%%%%%%%%%%%%%%%%%%%%%

%%%%%%%%%%%%%%%%%%%%%%%%%%%%%%%%%%%%%%%%%%%%%%%%%%%%%%%%%%%%
\begin{figure*}[t]
%%%%%%%%%%%%%%%%%%%%
  \begin{minipage}[b]{0.49\linewidth}
  \includegraphics[width=1\linewidth,trim=0 80pt 0 100pt, clip]{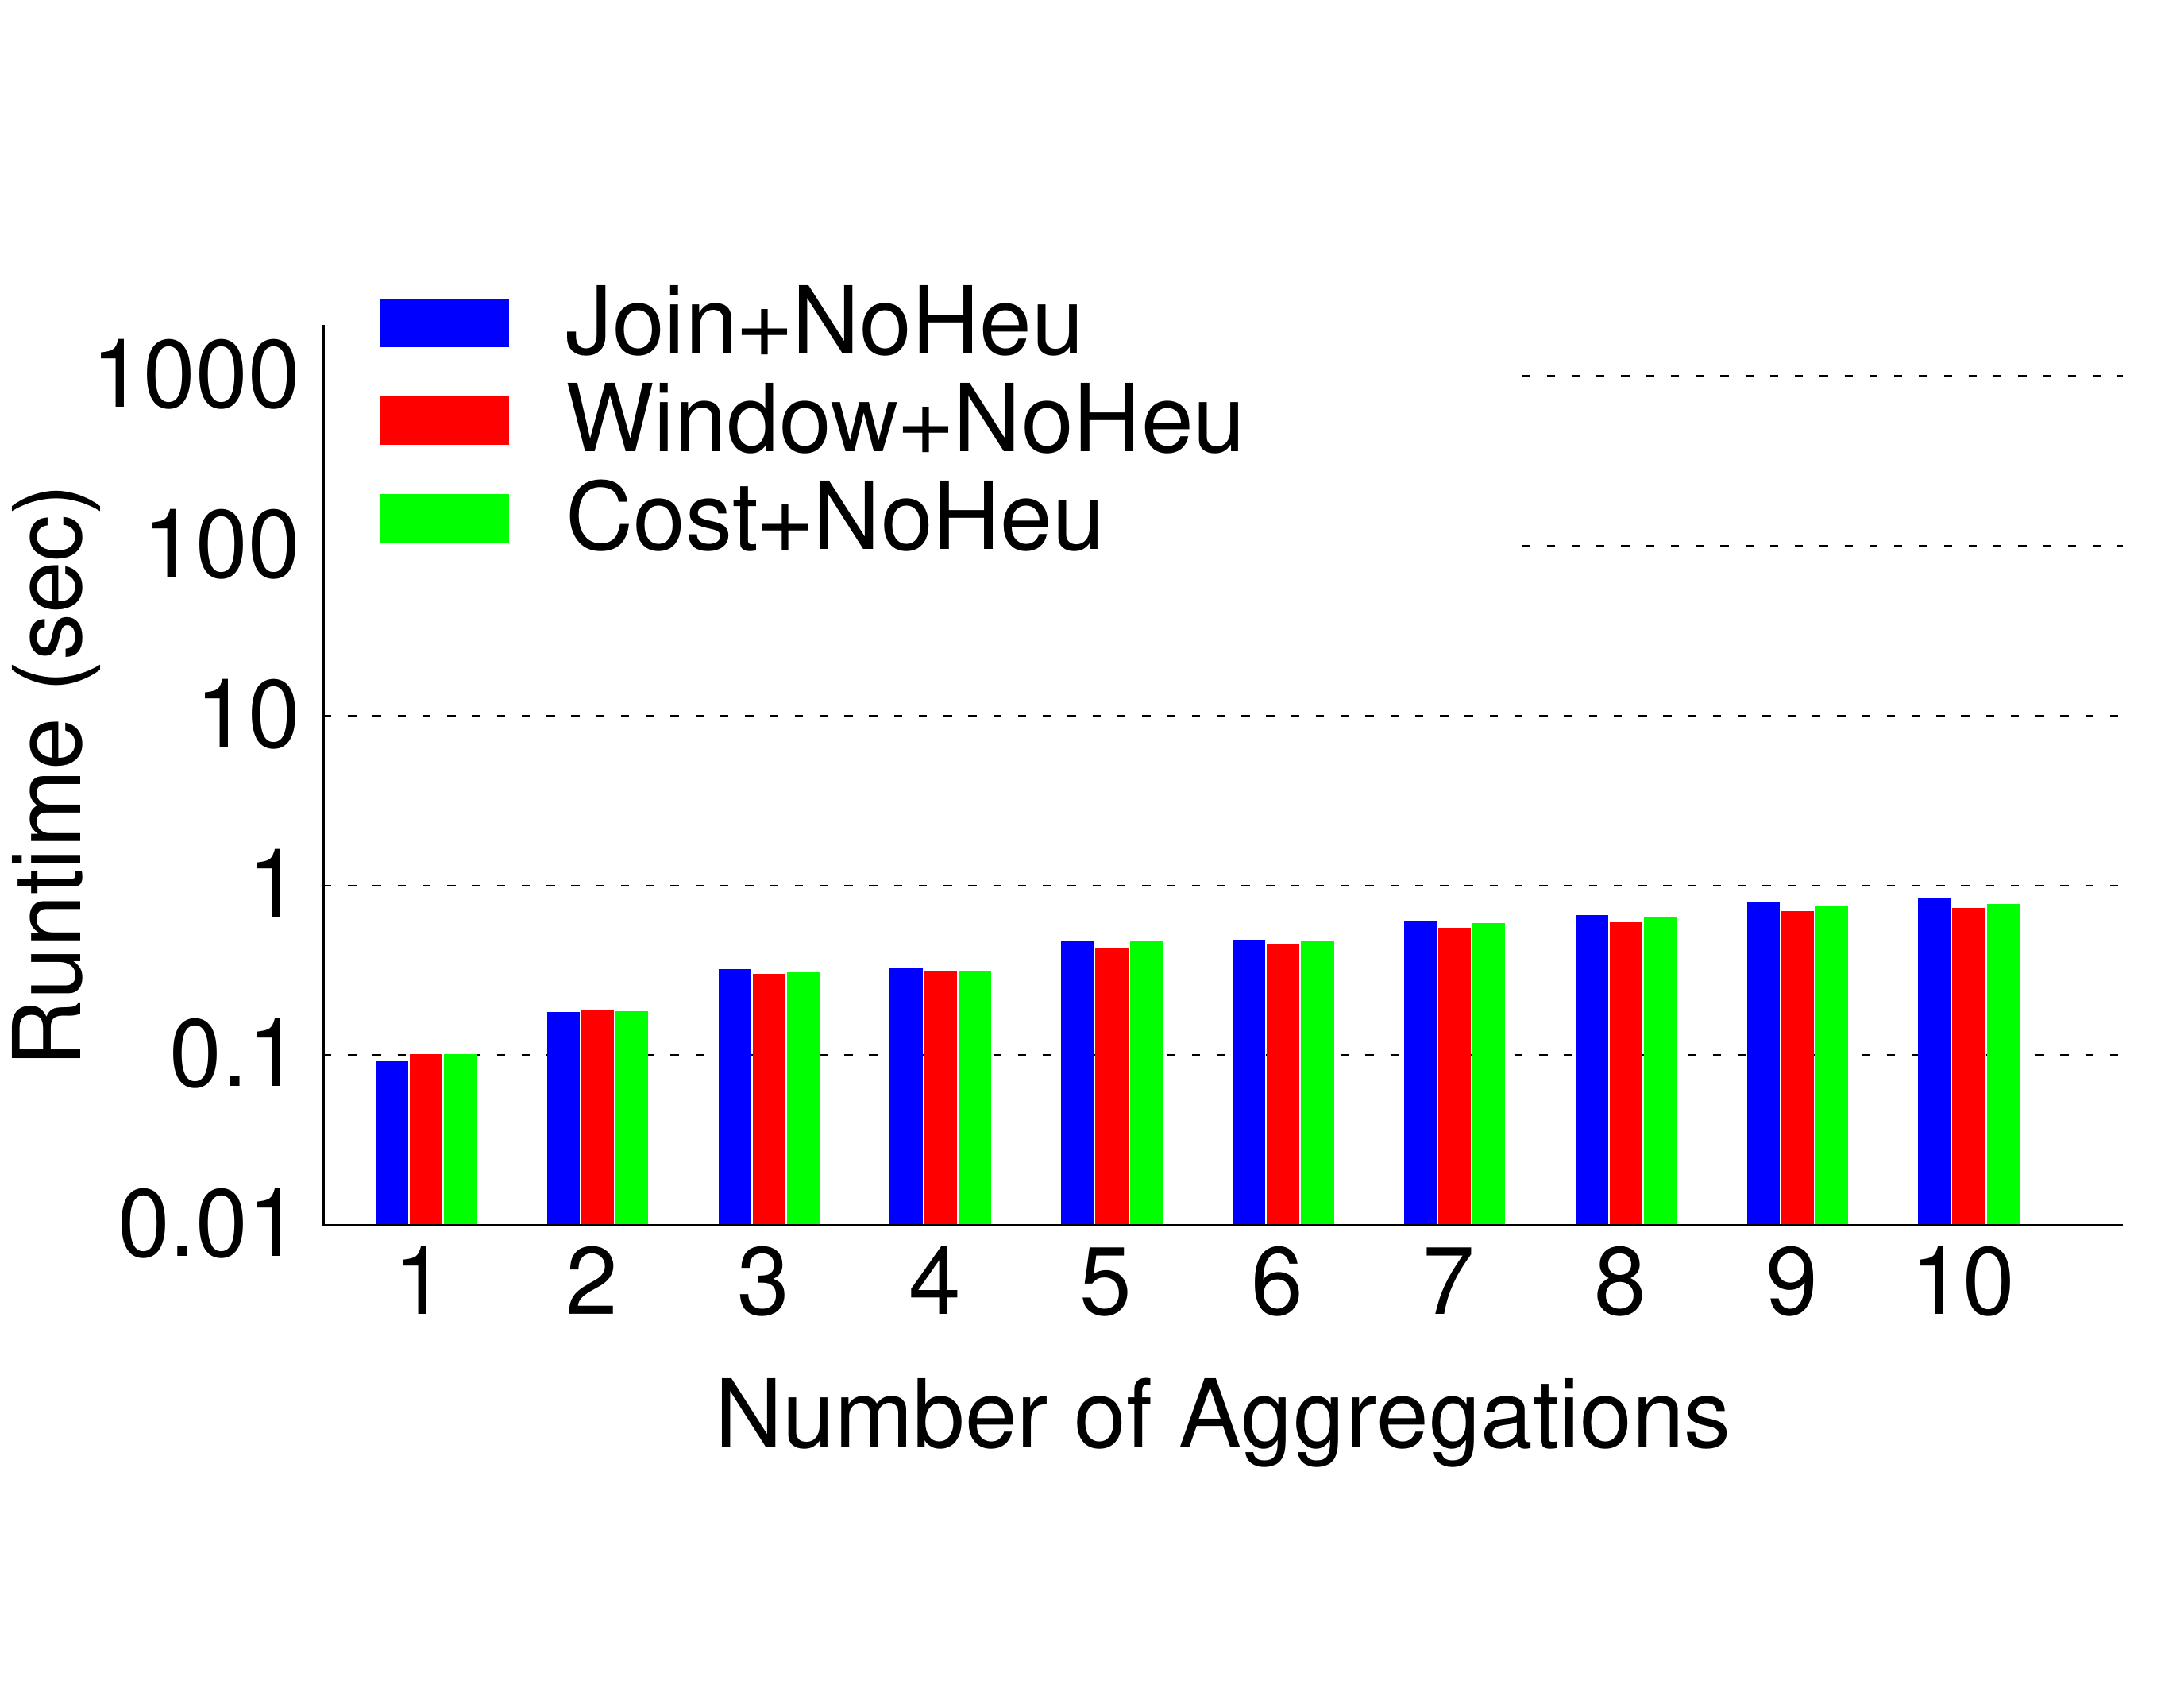}\\[-7mm]
  \caption{Simple Agg. - NoOpt - 1GB}
  \label{fig:simple-agg-noopt-1GB}  
  \end{minipage}
%%%%%%%%%%%%%%%%%%%
  \begin{minipage}[b]{0.49\linewidth}
  \includegraphics[width=1\linewidth,trim=0 80pt 0 100pt, clip]{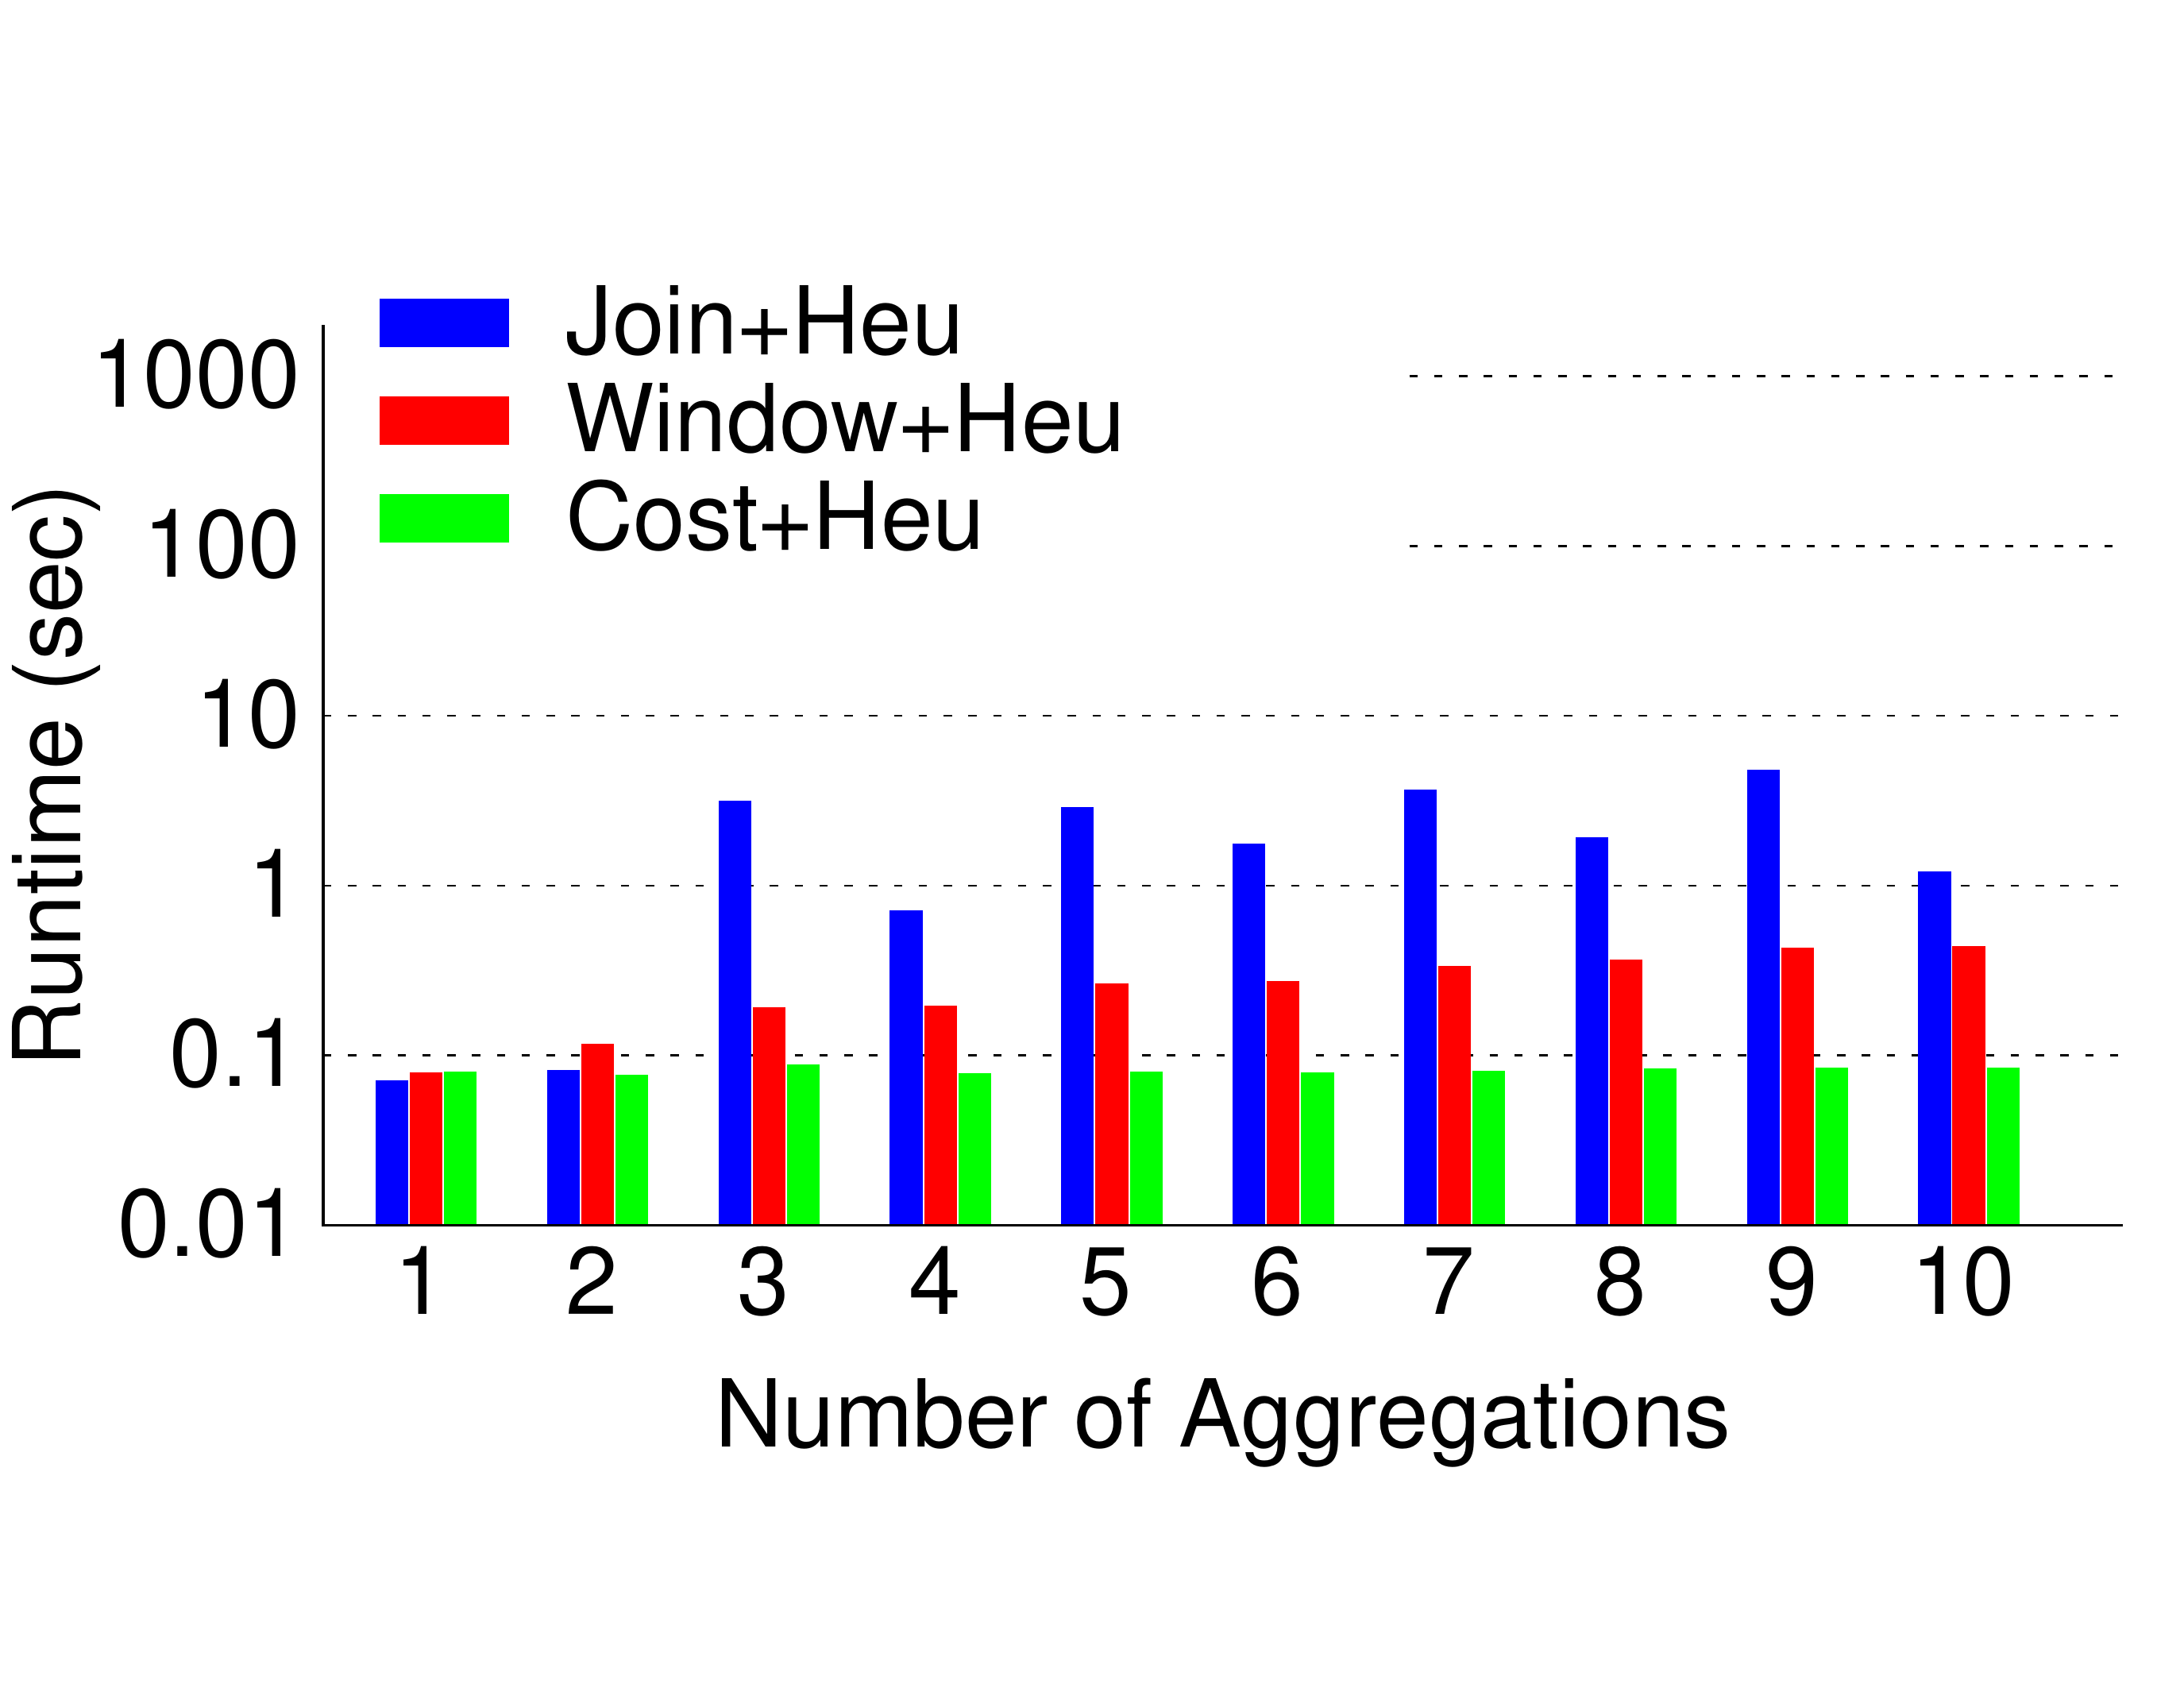}\\[-7mm] 
  \caption{Simple Agg. - Opt - 1GB}
  \label{fig:simple-agg-opt-1GB}
  \end{minipage}
\end{figure*}
% %%%%%%%%%%%%%%%%%%%%%%%%%%%%%%%%%%%%%%%%%%%%%%%%%%%%%%%%%%%%

%%%%%%%%%%%%%%%%%%%%%%%%%%%%%%%%%%%%%%%%%%%%%%%%%%%%%%%%%%%%
\begin{figure*}[t]
%%%%%%%%%%%%%%%%%%%%
  \begin{minipage}[b]{0.49\linewidth}
  \includegraphics[width=1\linewidth,trim=0 80pt 0 100pt, clip]{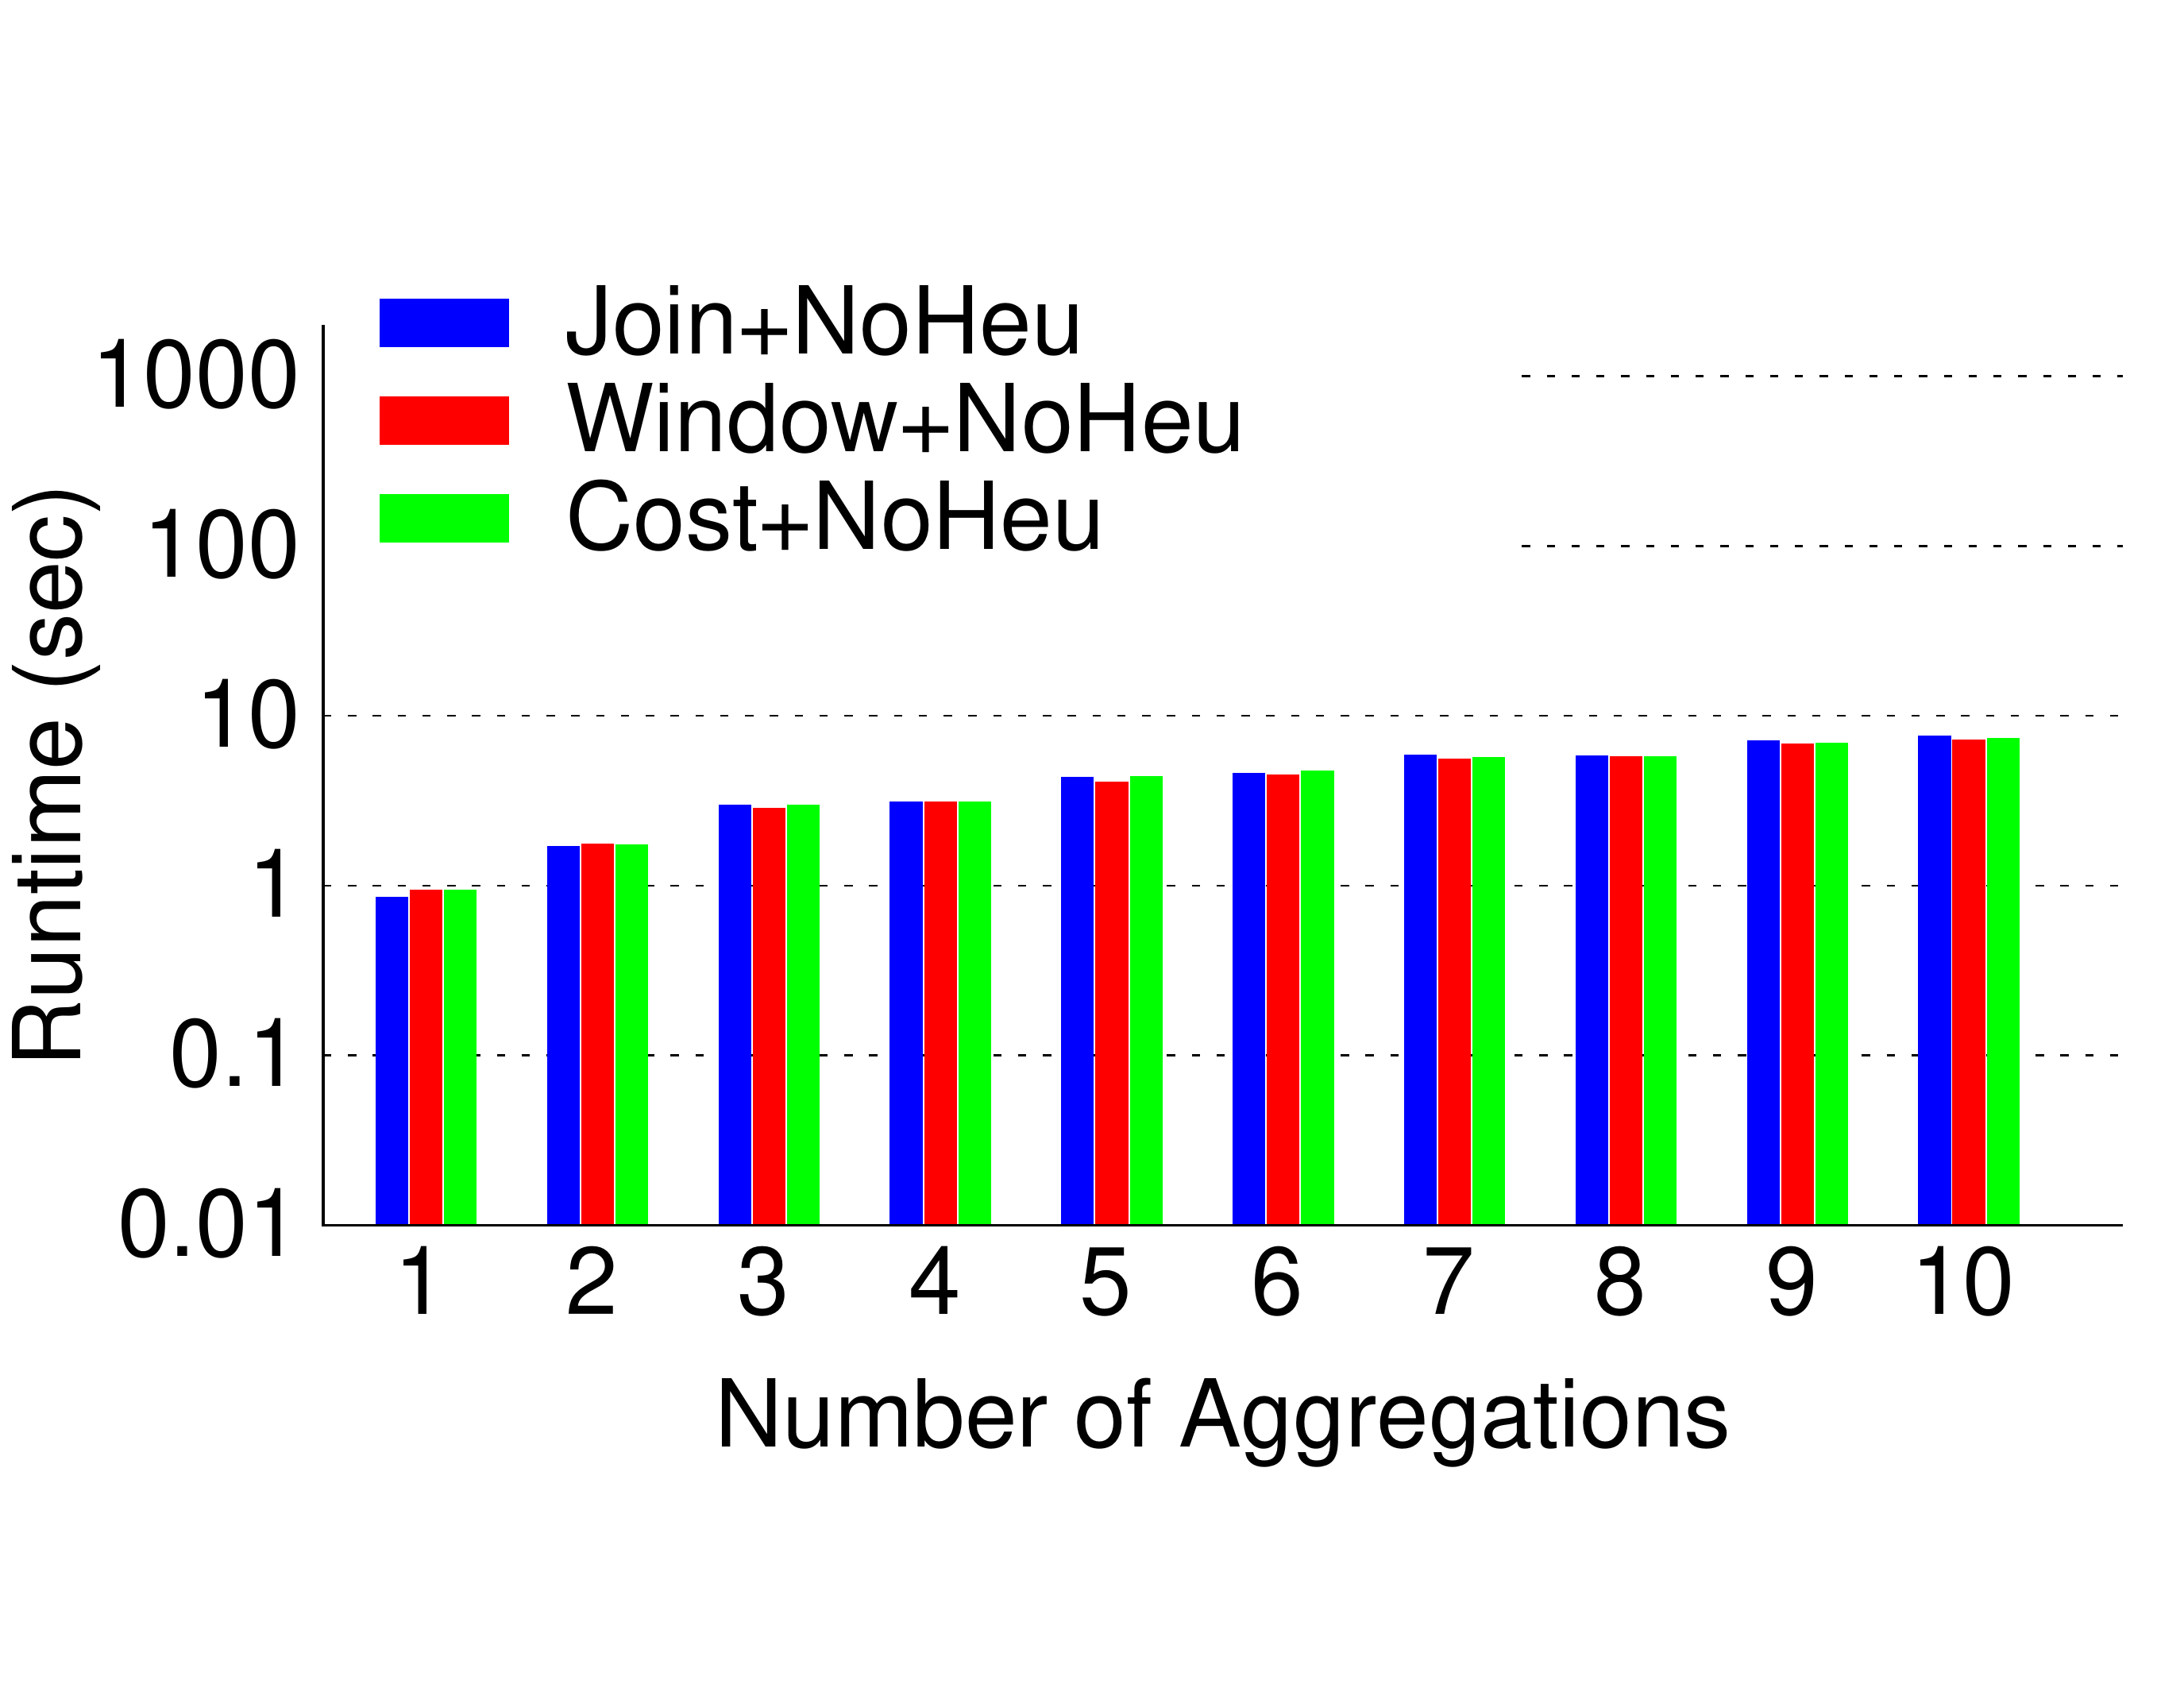}\\[-7mm]
  \caption{Simple Agg. - NoOpt - 10GB}
  \label{fig:simple-agg-noopt-10GB}  
  \end{minipage}
%%%%%%%%%%%%%%%%%%%
  \begin{minipage}[b]{0.49\linewidth}
  \includegraphics[width=1\linewidth,trim=0 80pt 0 100pt, clip]{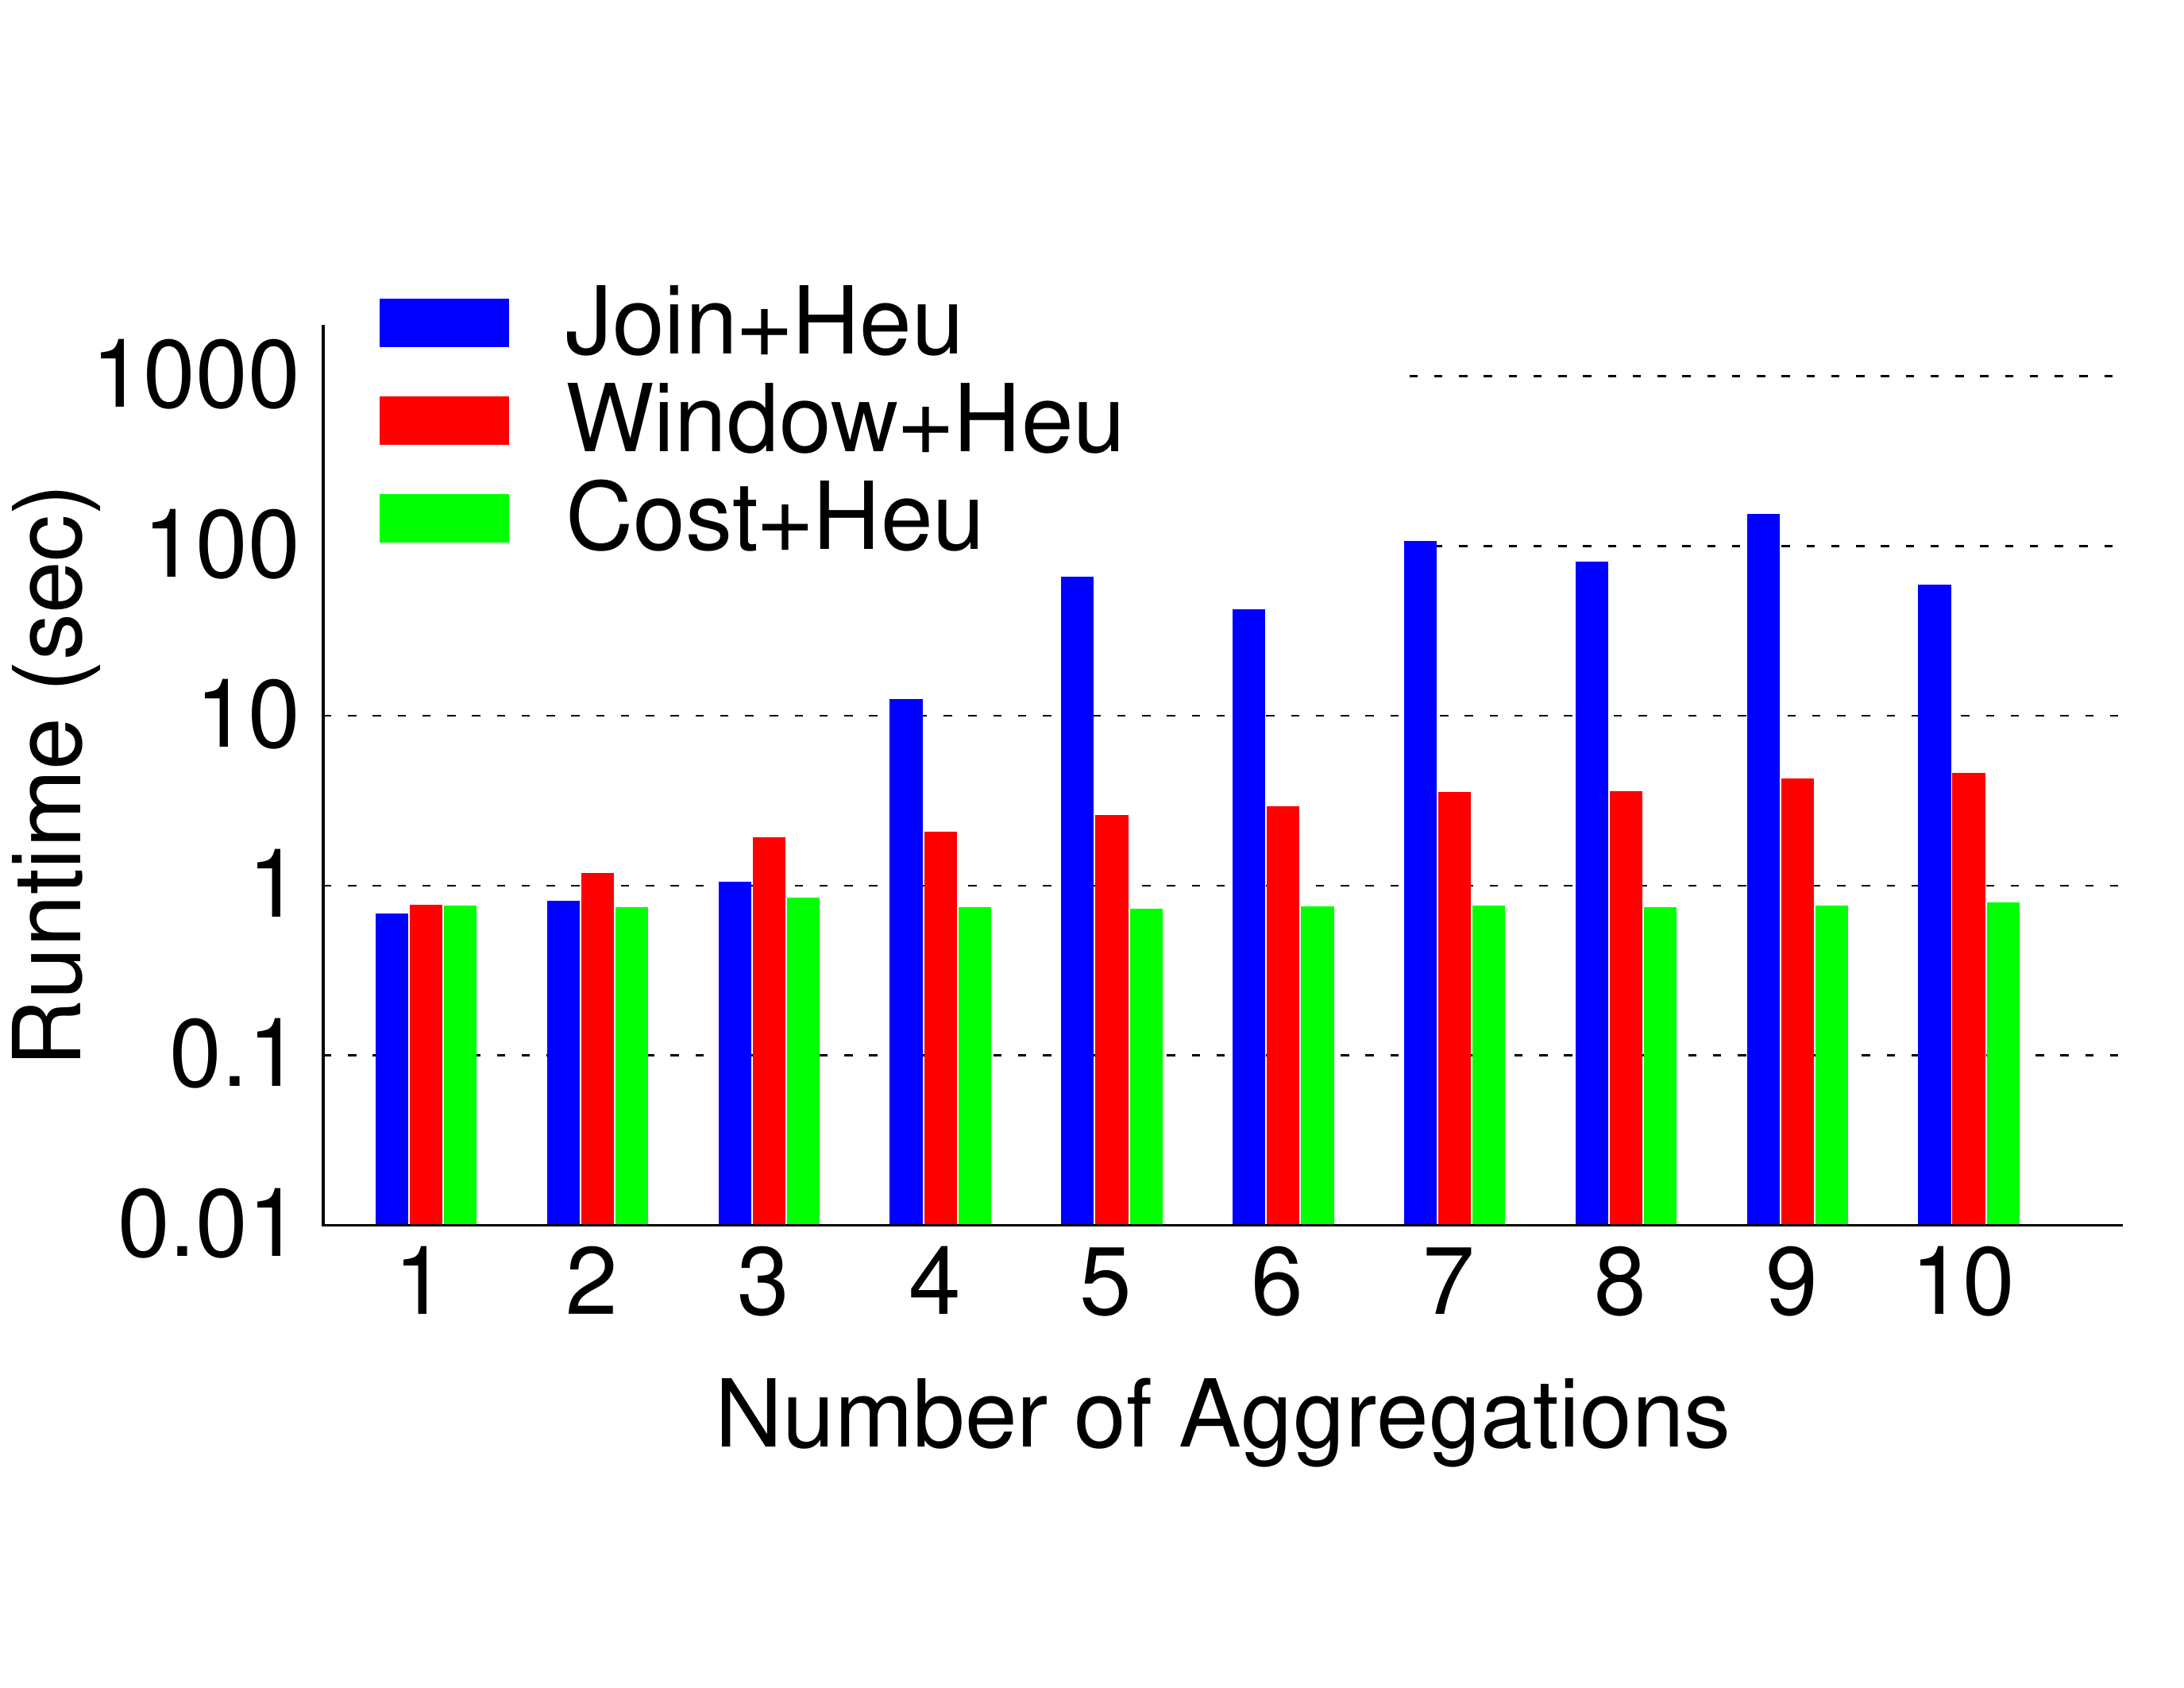}\\[-7mm] 
  \caption{Simple Agg. - Opt - 10GB}
  \label{fig:simple-agg-opt-10GB}
  \end{minipage}
\end{figure*}
% %%%%%%%%%%%%%%%%%%%%%%%%%%%%%%%%%%%%%%%%%%%%%%%%%%%%%%%%%%%%

%%%%%%%%%%%%%%%%%%%%%%%%%%%%%%%%%%%%%%%%%%%%%%%%%%%%%%%%%%%%
\begin{figure*}[t]
%%%%%%%%%%%%%%%%%%%%
  \begin{minipage}[b]{0.49\linewidth}
  \includegraphics[width=1\linewidth,trim=0 80pt 0 100pt, clip]{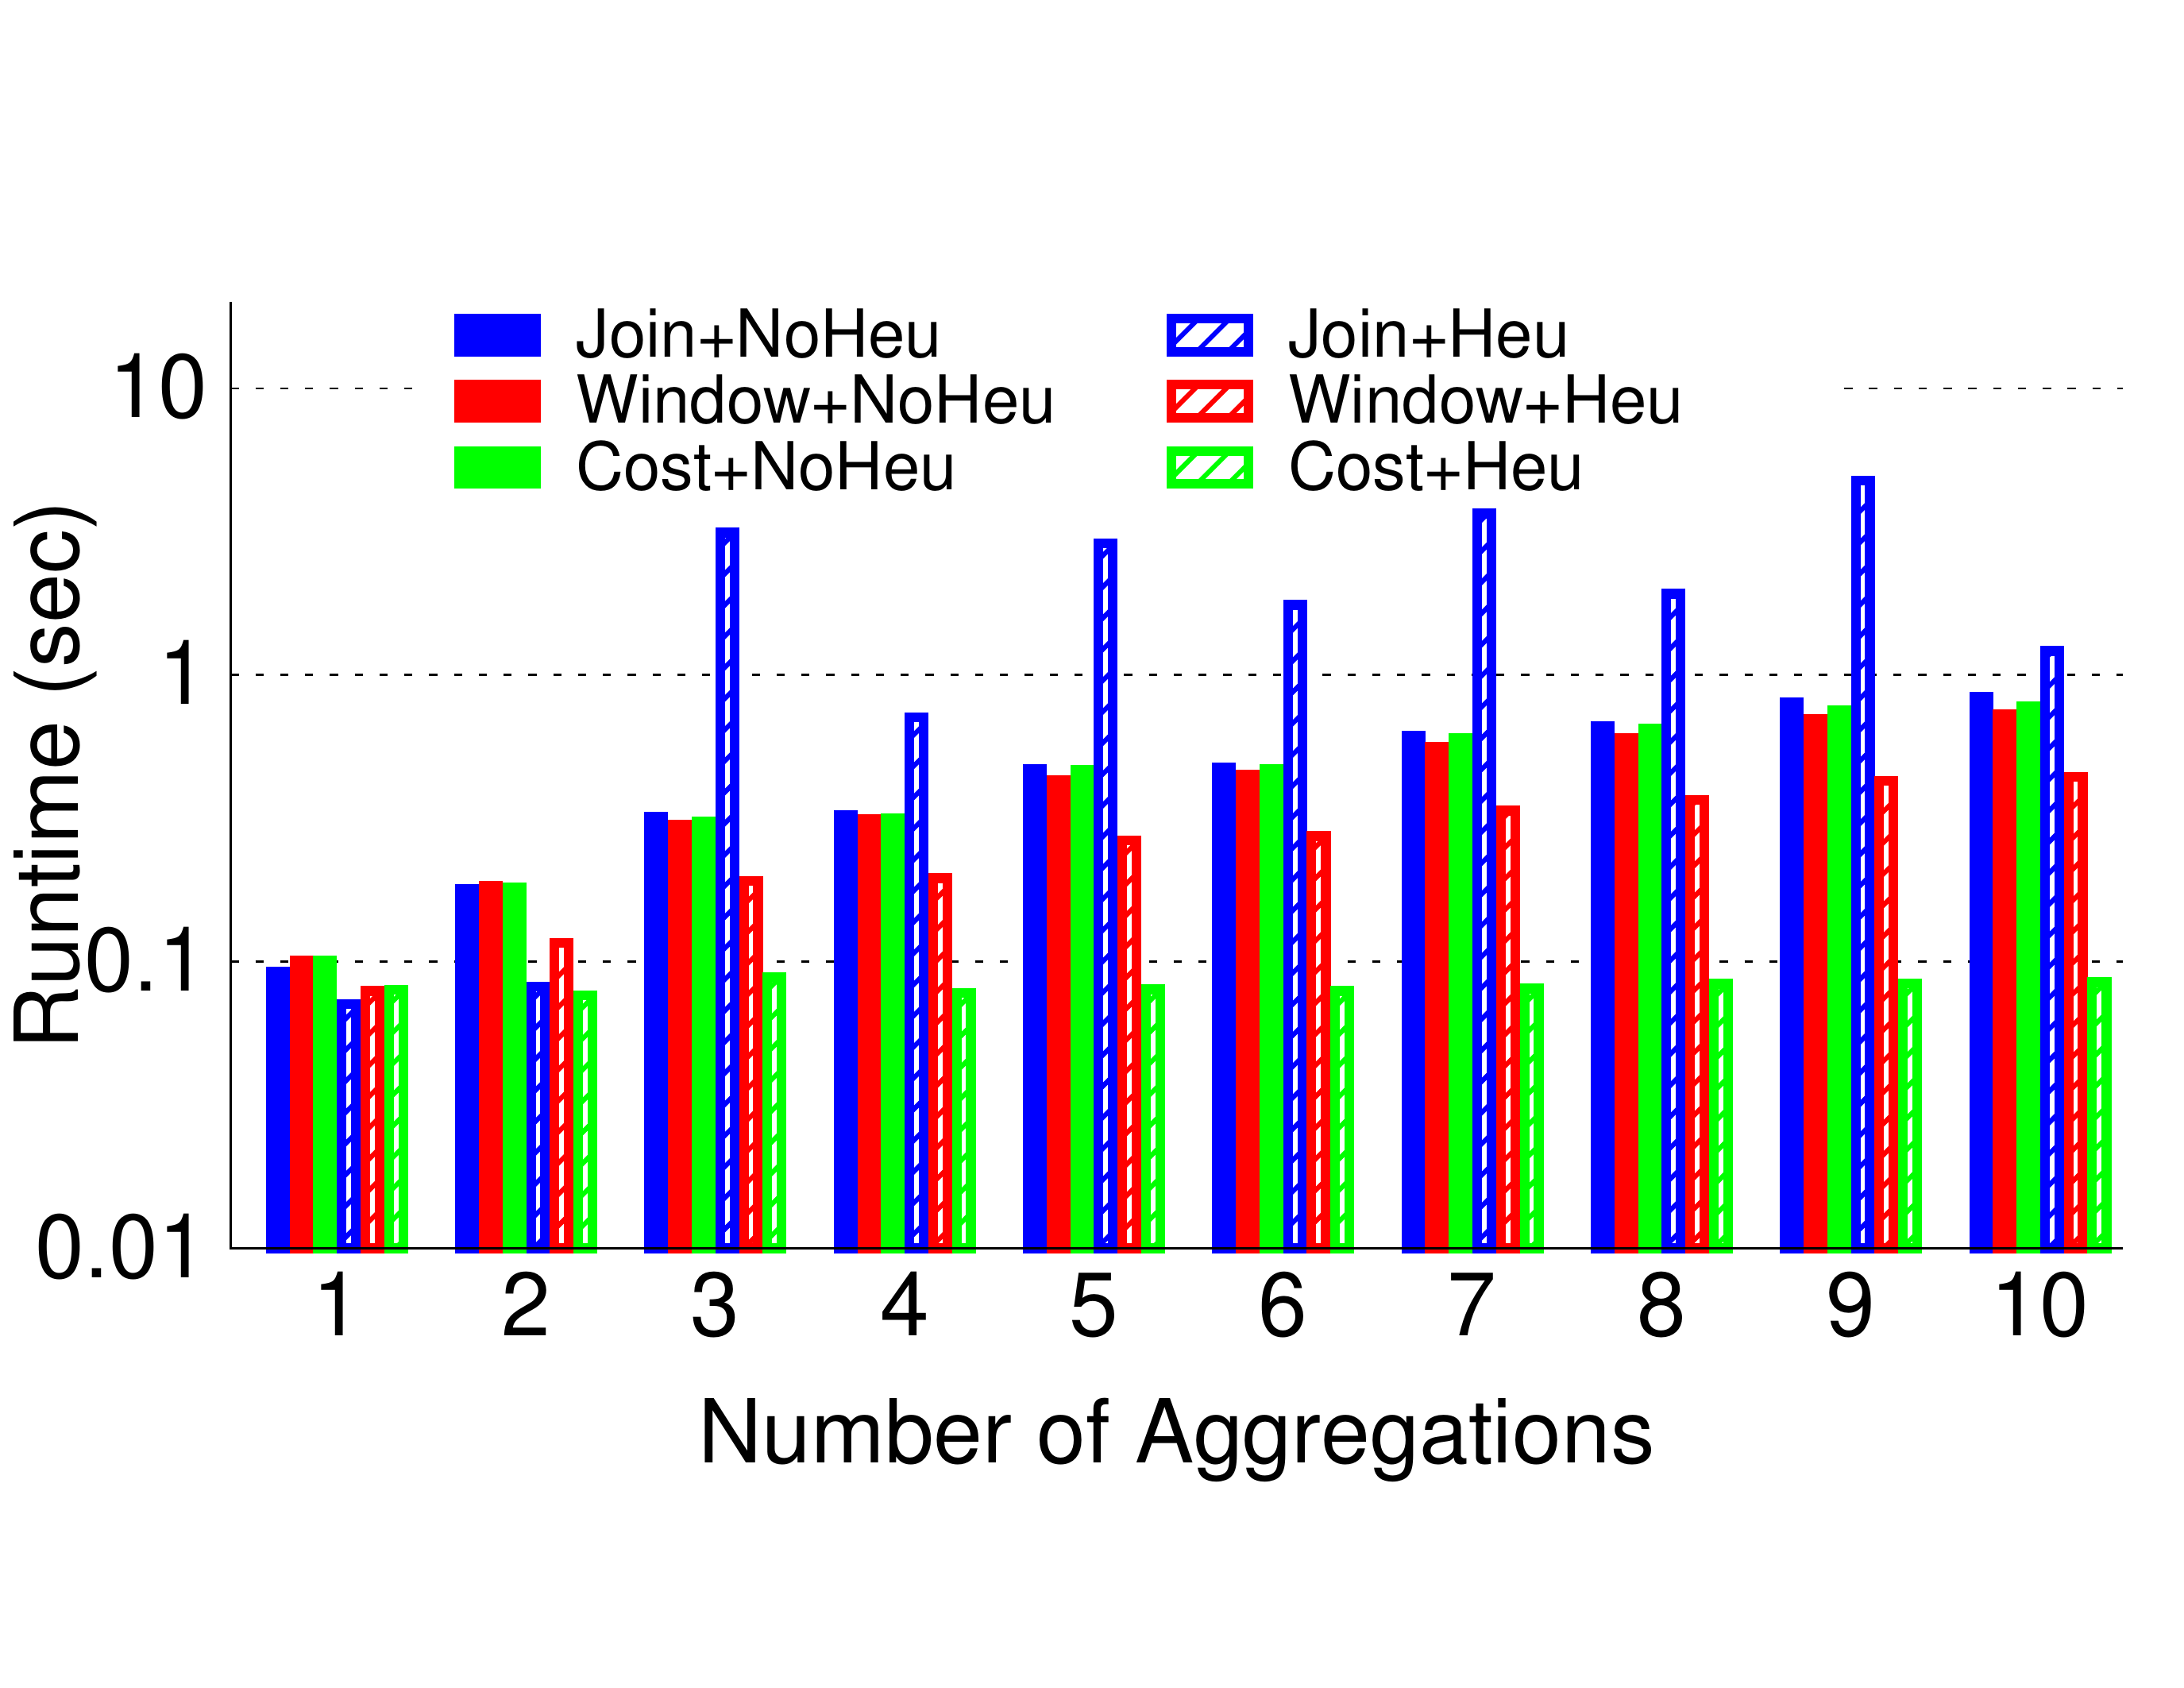}\\[-7mm]
  \caption{Simple Agg.  - 1GB}
  \label{fig:simpleAgg-comb-1GB}  
  \end{minipage}
%%%%%%%%%%%%%%%%%%%
  \begin{minipage}[b]{0.49\linewidth}
  \includegraphics[width=1\linewidth,trim=0 80pt 0 100pt, clip]{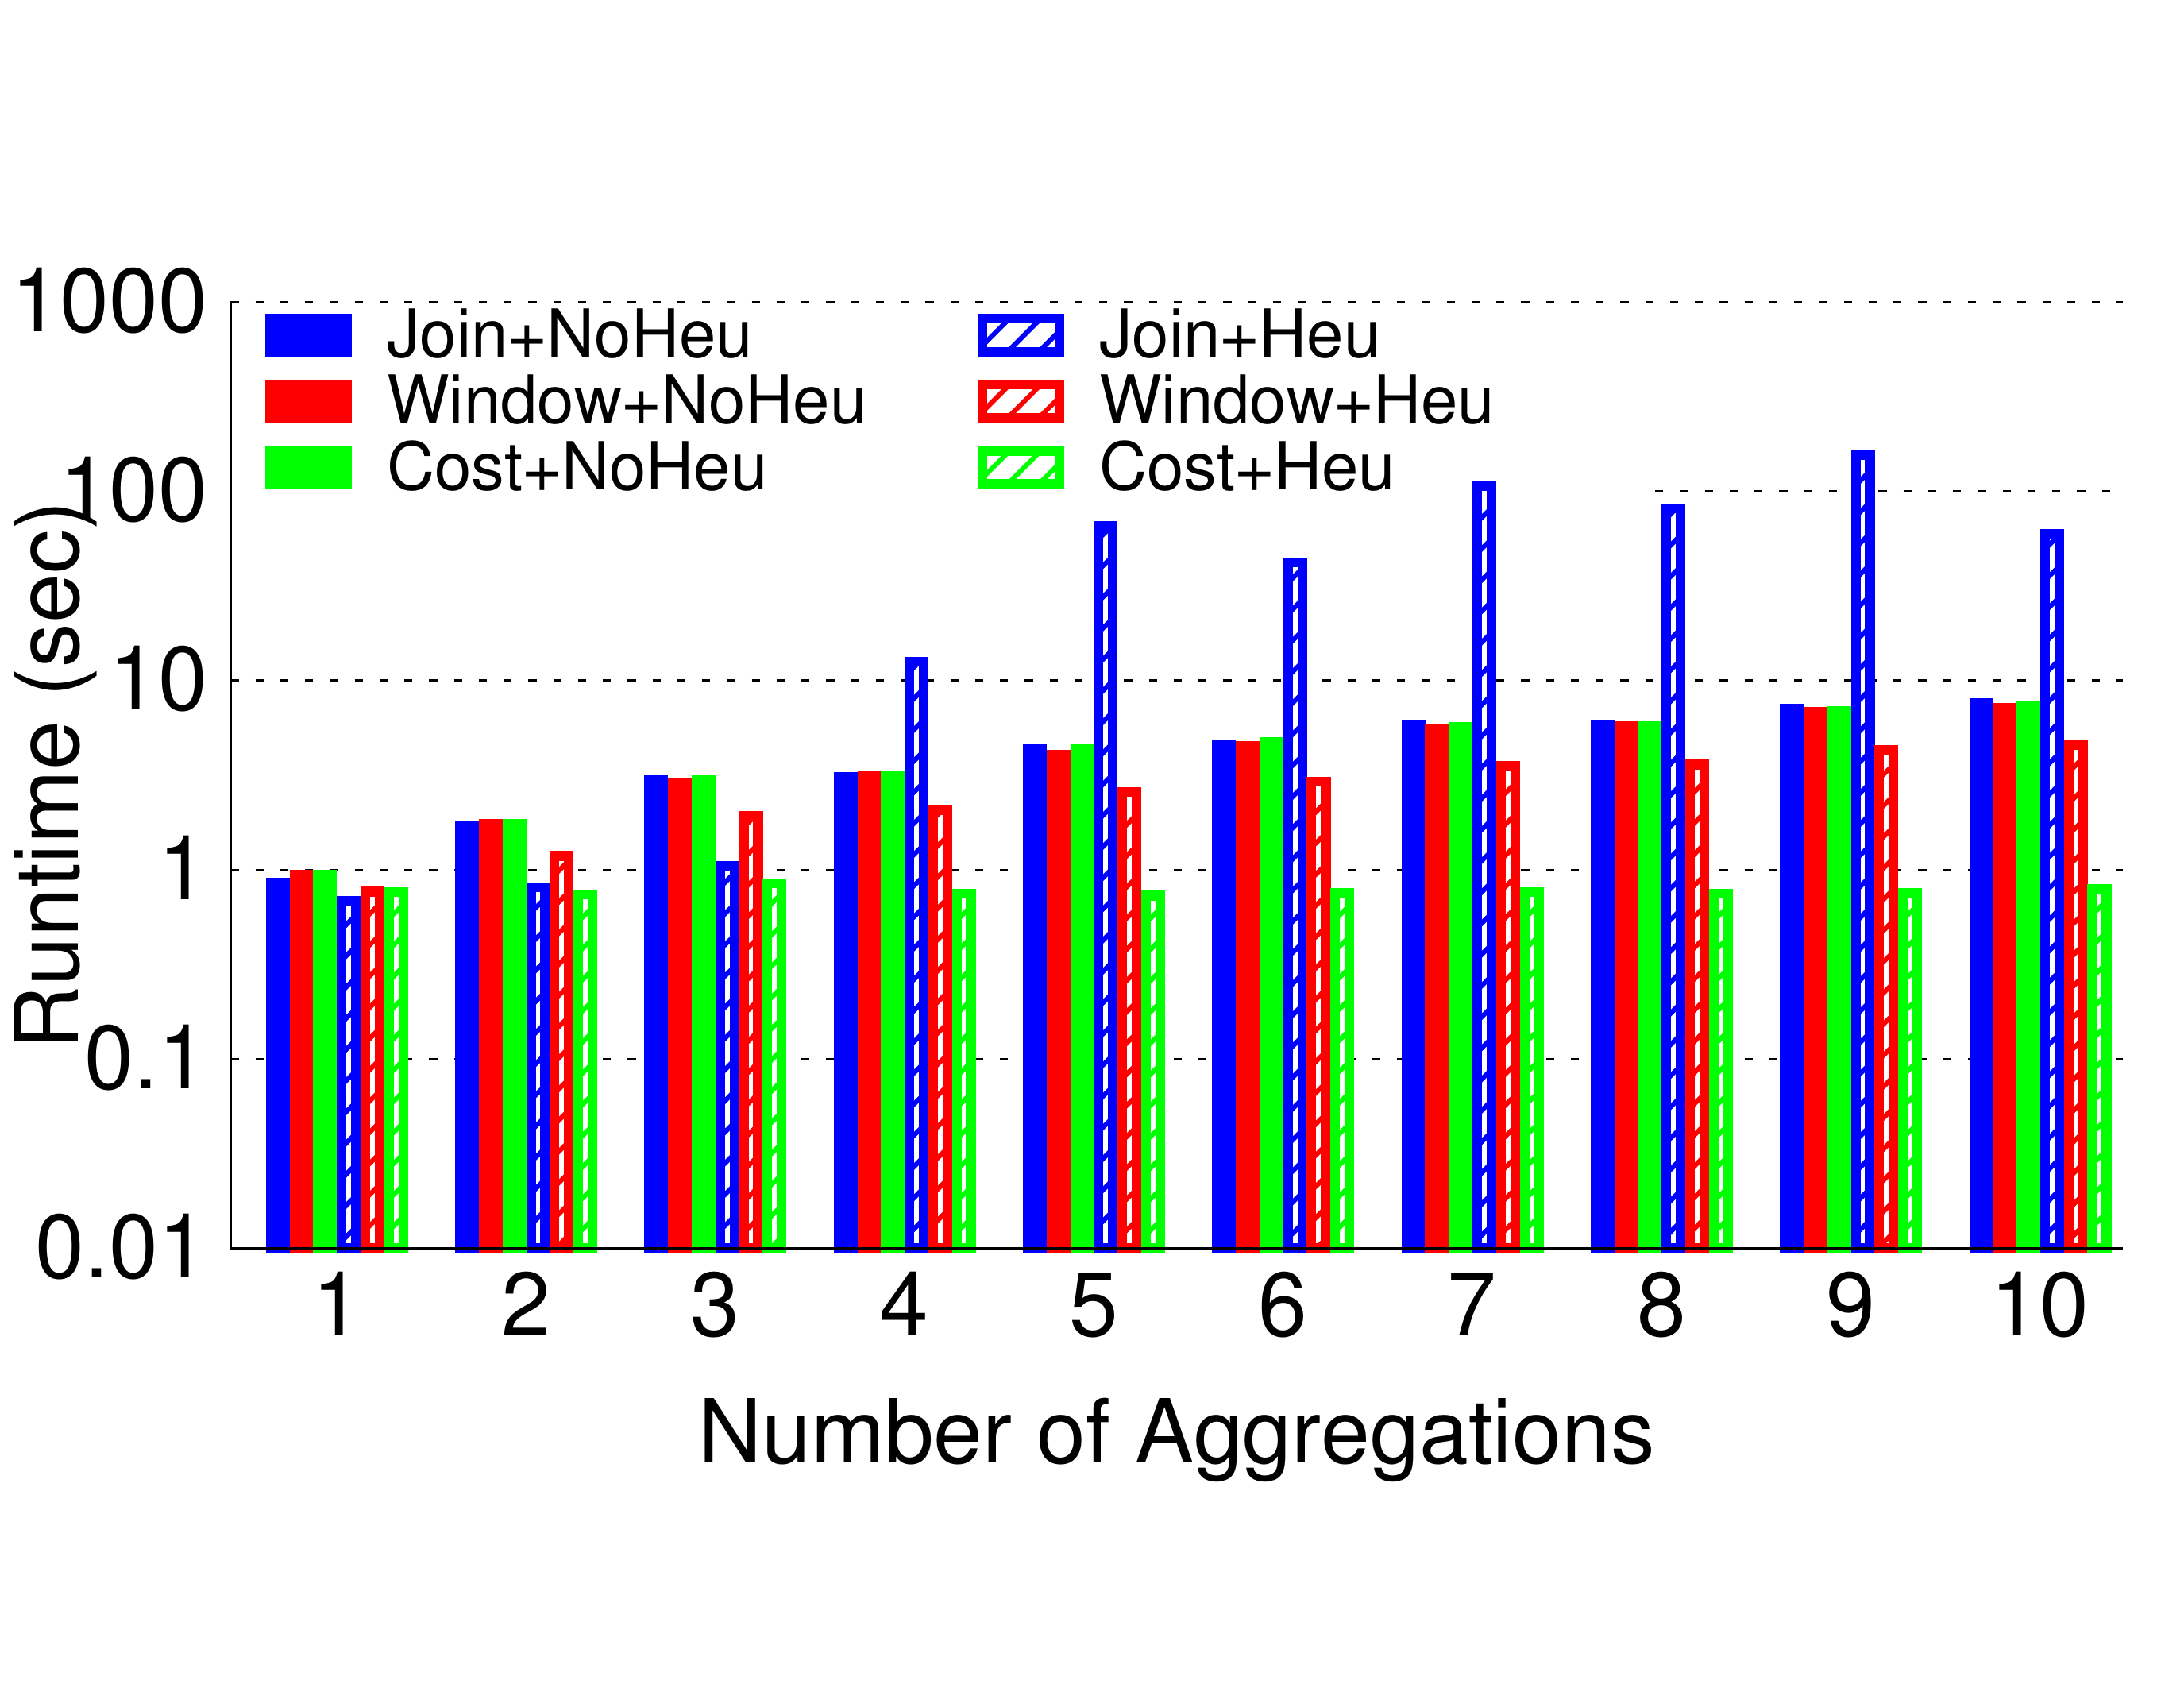}\\[-7mm] 
  \caption{Simple Agg. - 10GB}
  \label{fig:simpleAgg-comb-10GB}
  \end{minipage}
\end{figure*}
% %%%%%%%%%%%%%%%%%%%%%%%%%%%%%%%%%%%%%%%%%%%%%%%%%%%%%%%%%%%%

\clearpage   

%%%%%%%%%%%%%%%%%%%%%%%%%%%%%%%%%%%%%%%%%%%%%%%%%%%%%%%%%%%%
\begin{figure*}[t]
%%%%%%%%%%%%%%%%%%%%
  \begin{minipage}[b]{0.49\linewidth}
  \includegraphics[width=1\linewidth,trim=0 80pt 0 100pt, clip]{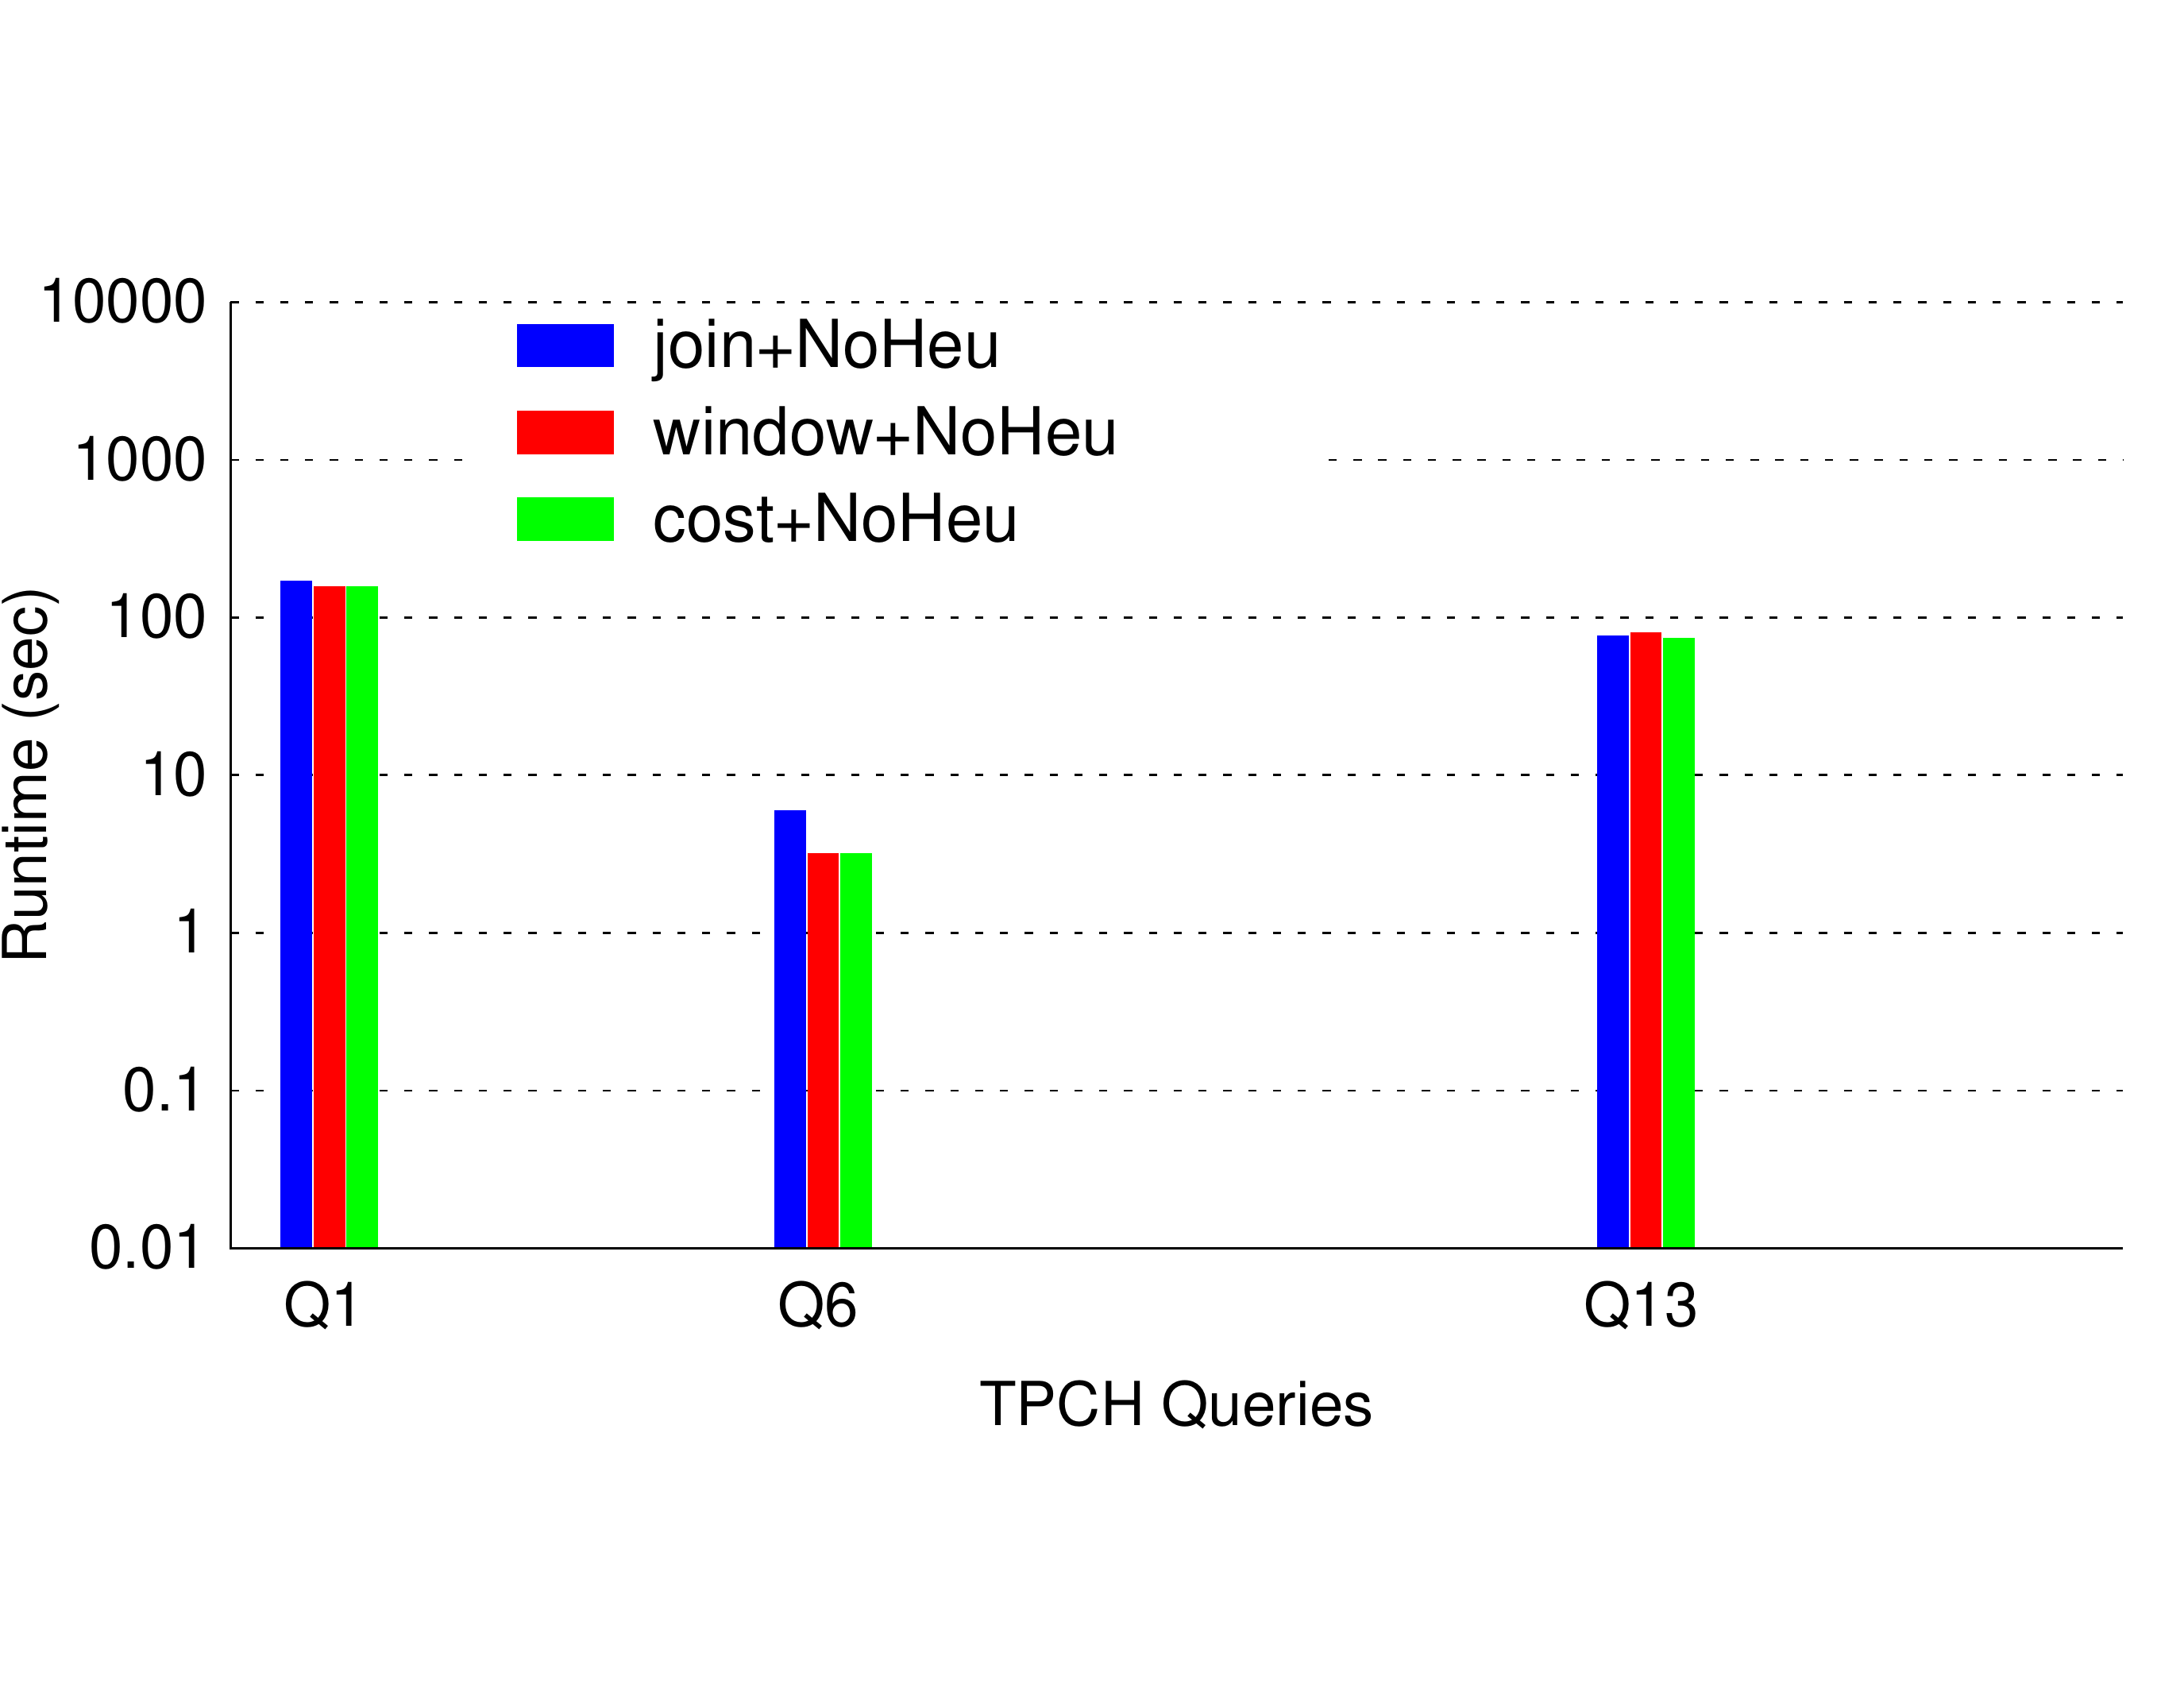}\\[-7mm]
  \caption{TPC-H Queries - NoOpt - 1GB}
  \label{fig:tpch-noopt-1GB}  
  \end{minipage}
%%%%%%%%%%%%%%%%%%%
  \begin{minipage}[b]{0.49\linewidth}
  \includegraphics[width=1\linewidth,trim=0 80pt 0 100pt, clip]{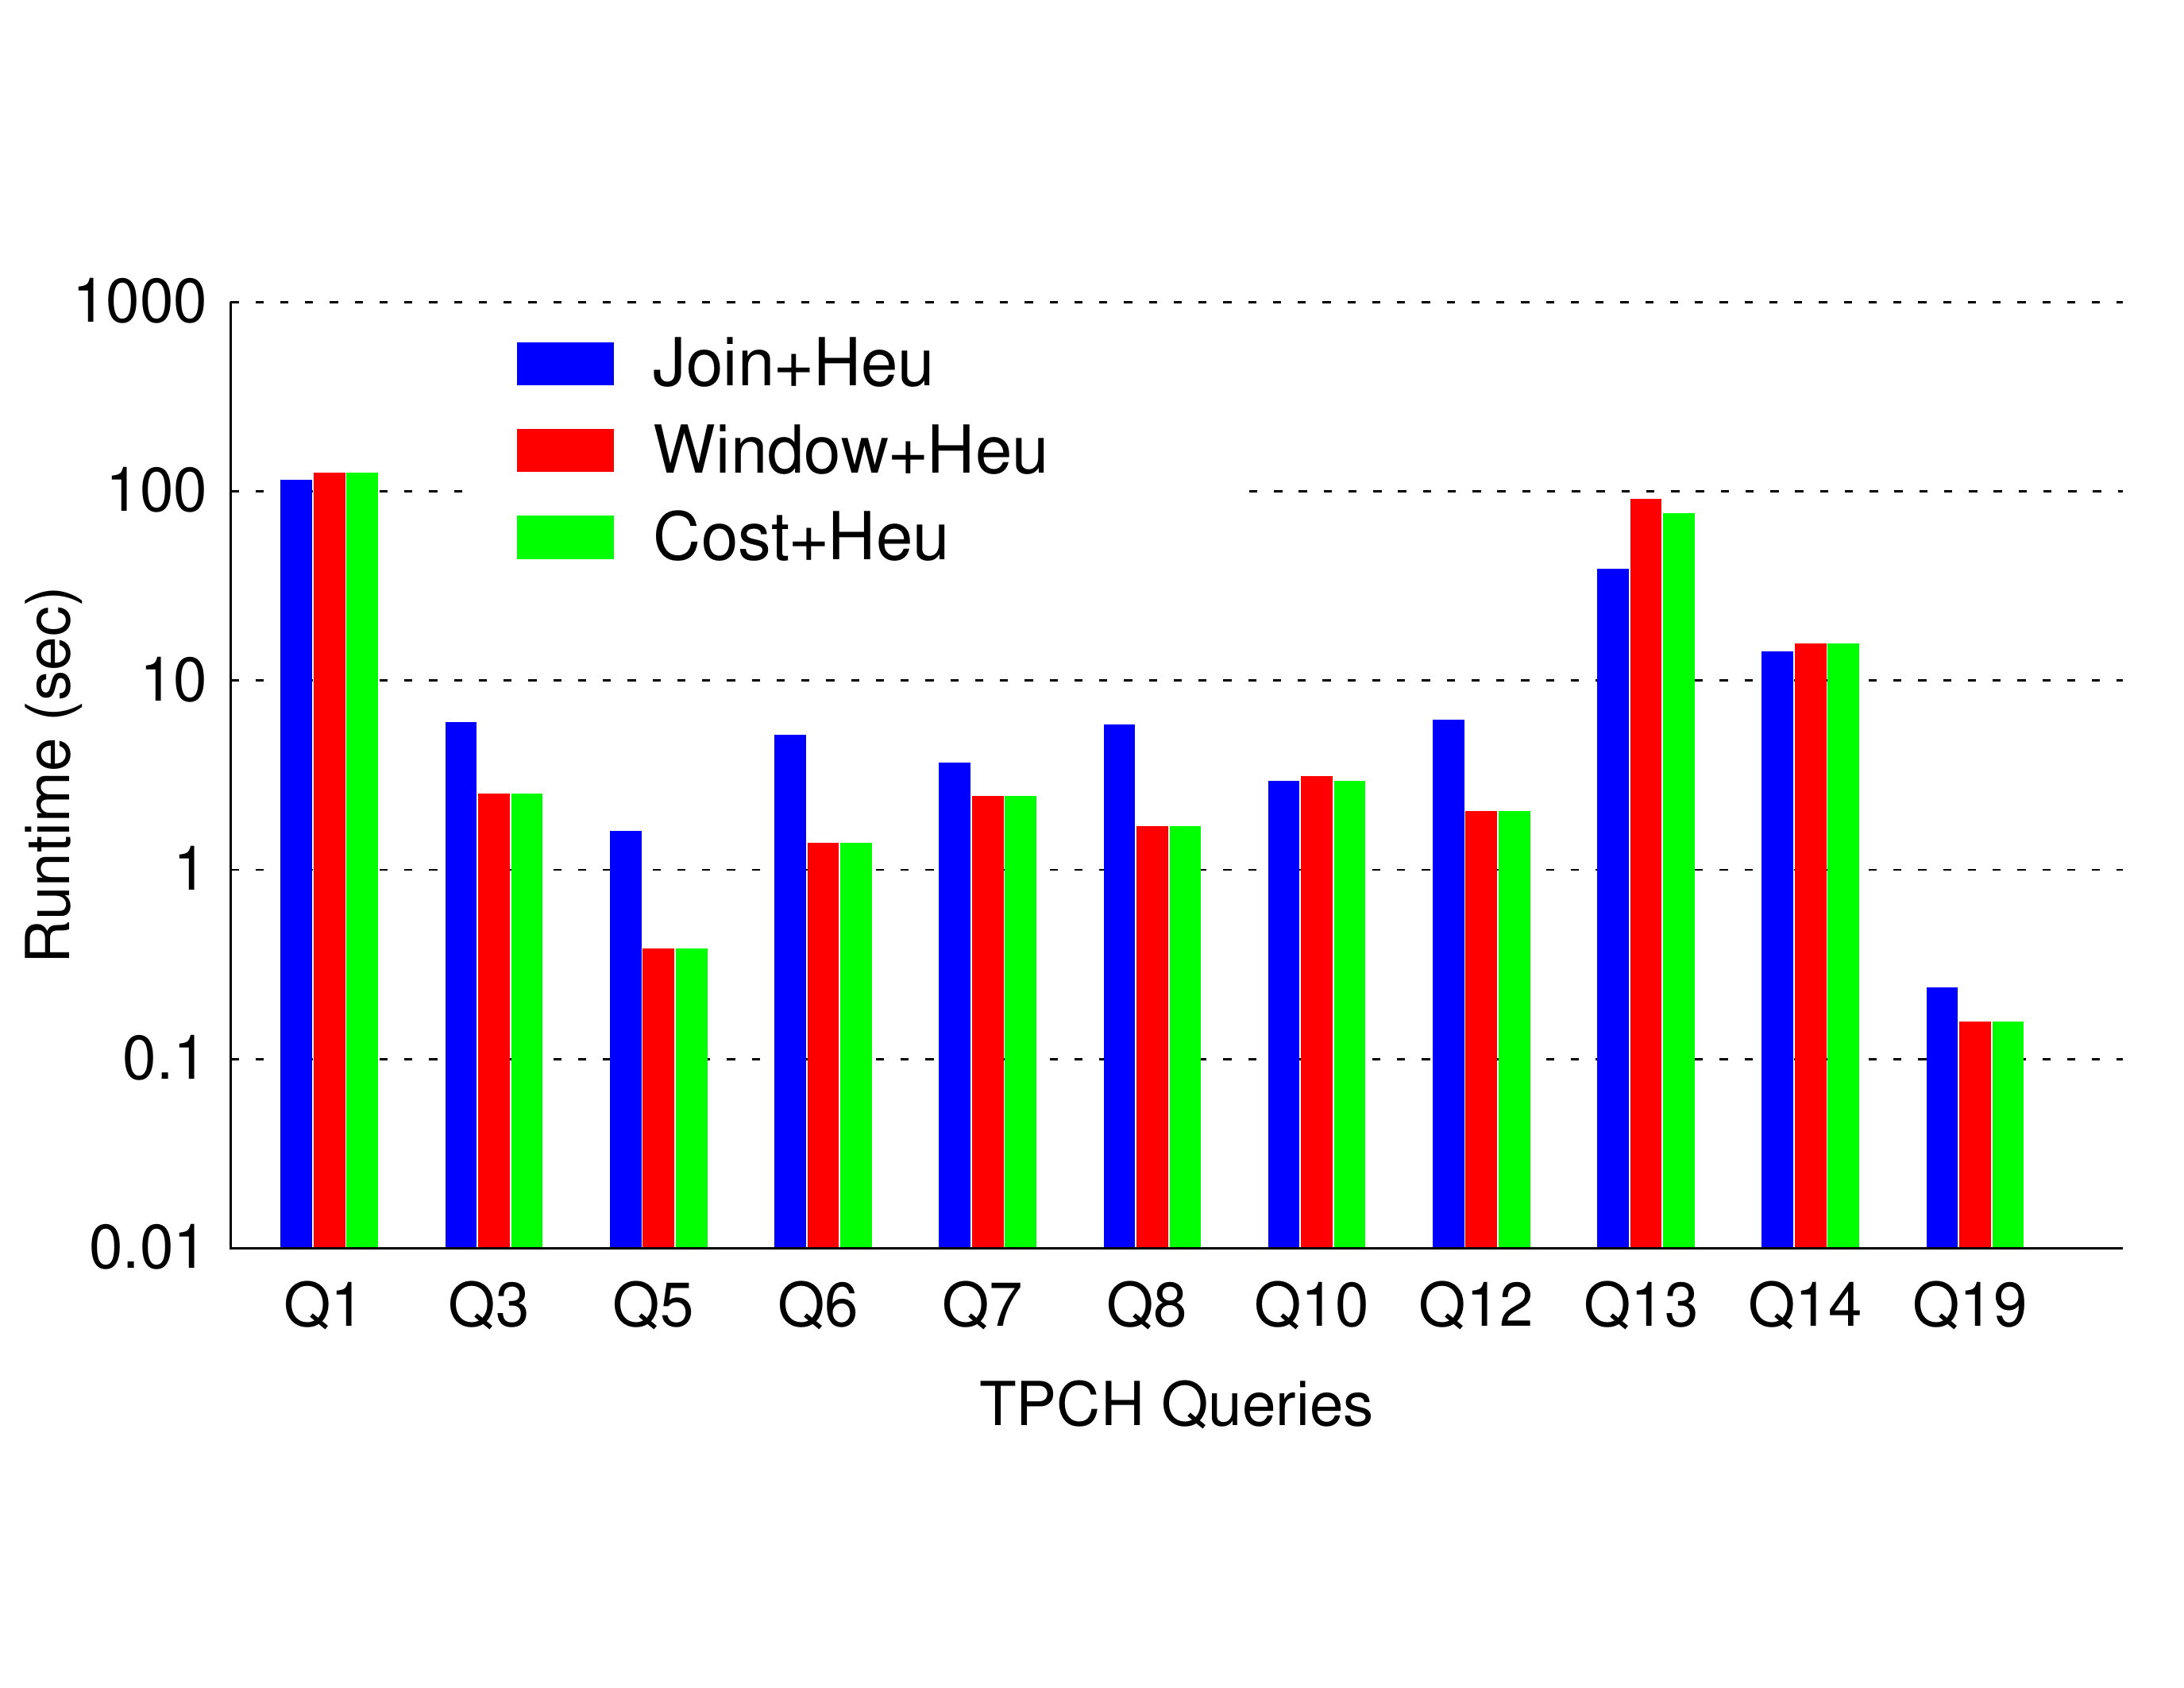}\\[-7mm] 
  \caption{TPC-H Queries - Opt - 1GB}
  \label{fig:tpch-opt-1GB}
  \end{minipage}
\end{figure*}
% %%%%%%%%%%%%%%%%%%%%%%%%%%%%%%%%%%%%%%%%%%%%%%%%%%%%%%%%%%%%  

%%%%%%%%%%%%%%%%%%%%%%%%%%%%%%%%%%%%%%%%%%%%%%%%%%%%%%%%%%%%
\begin{figure*}[t]
%%%%%%%%%%%%%%%%%%%%
  \begin{minipage}[b]{0.49\linewidth}
  \includegraphics[width=1\linewidth,trim=0 80pt 0 100pt, clip]{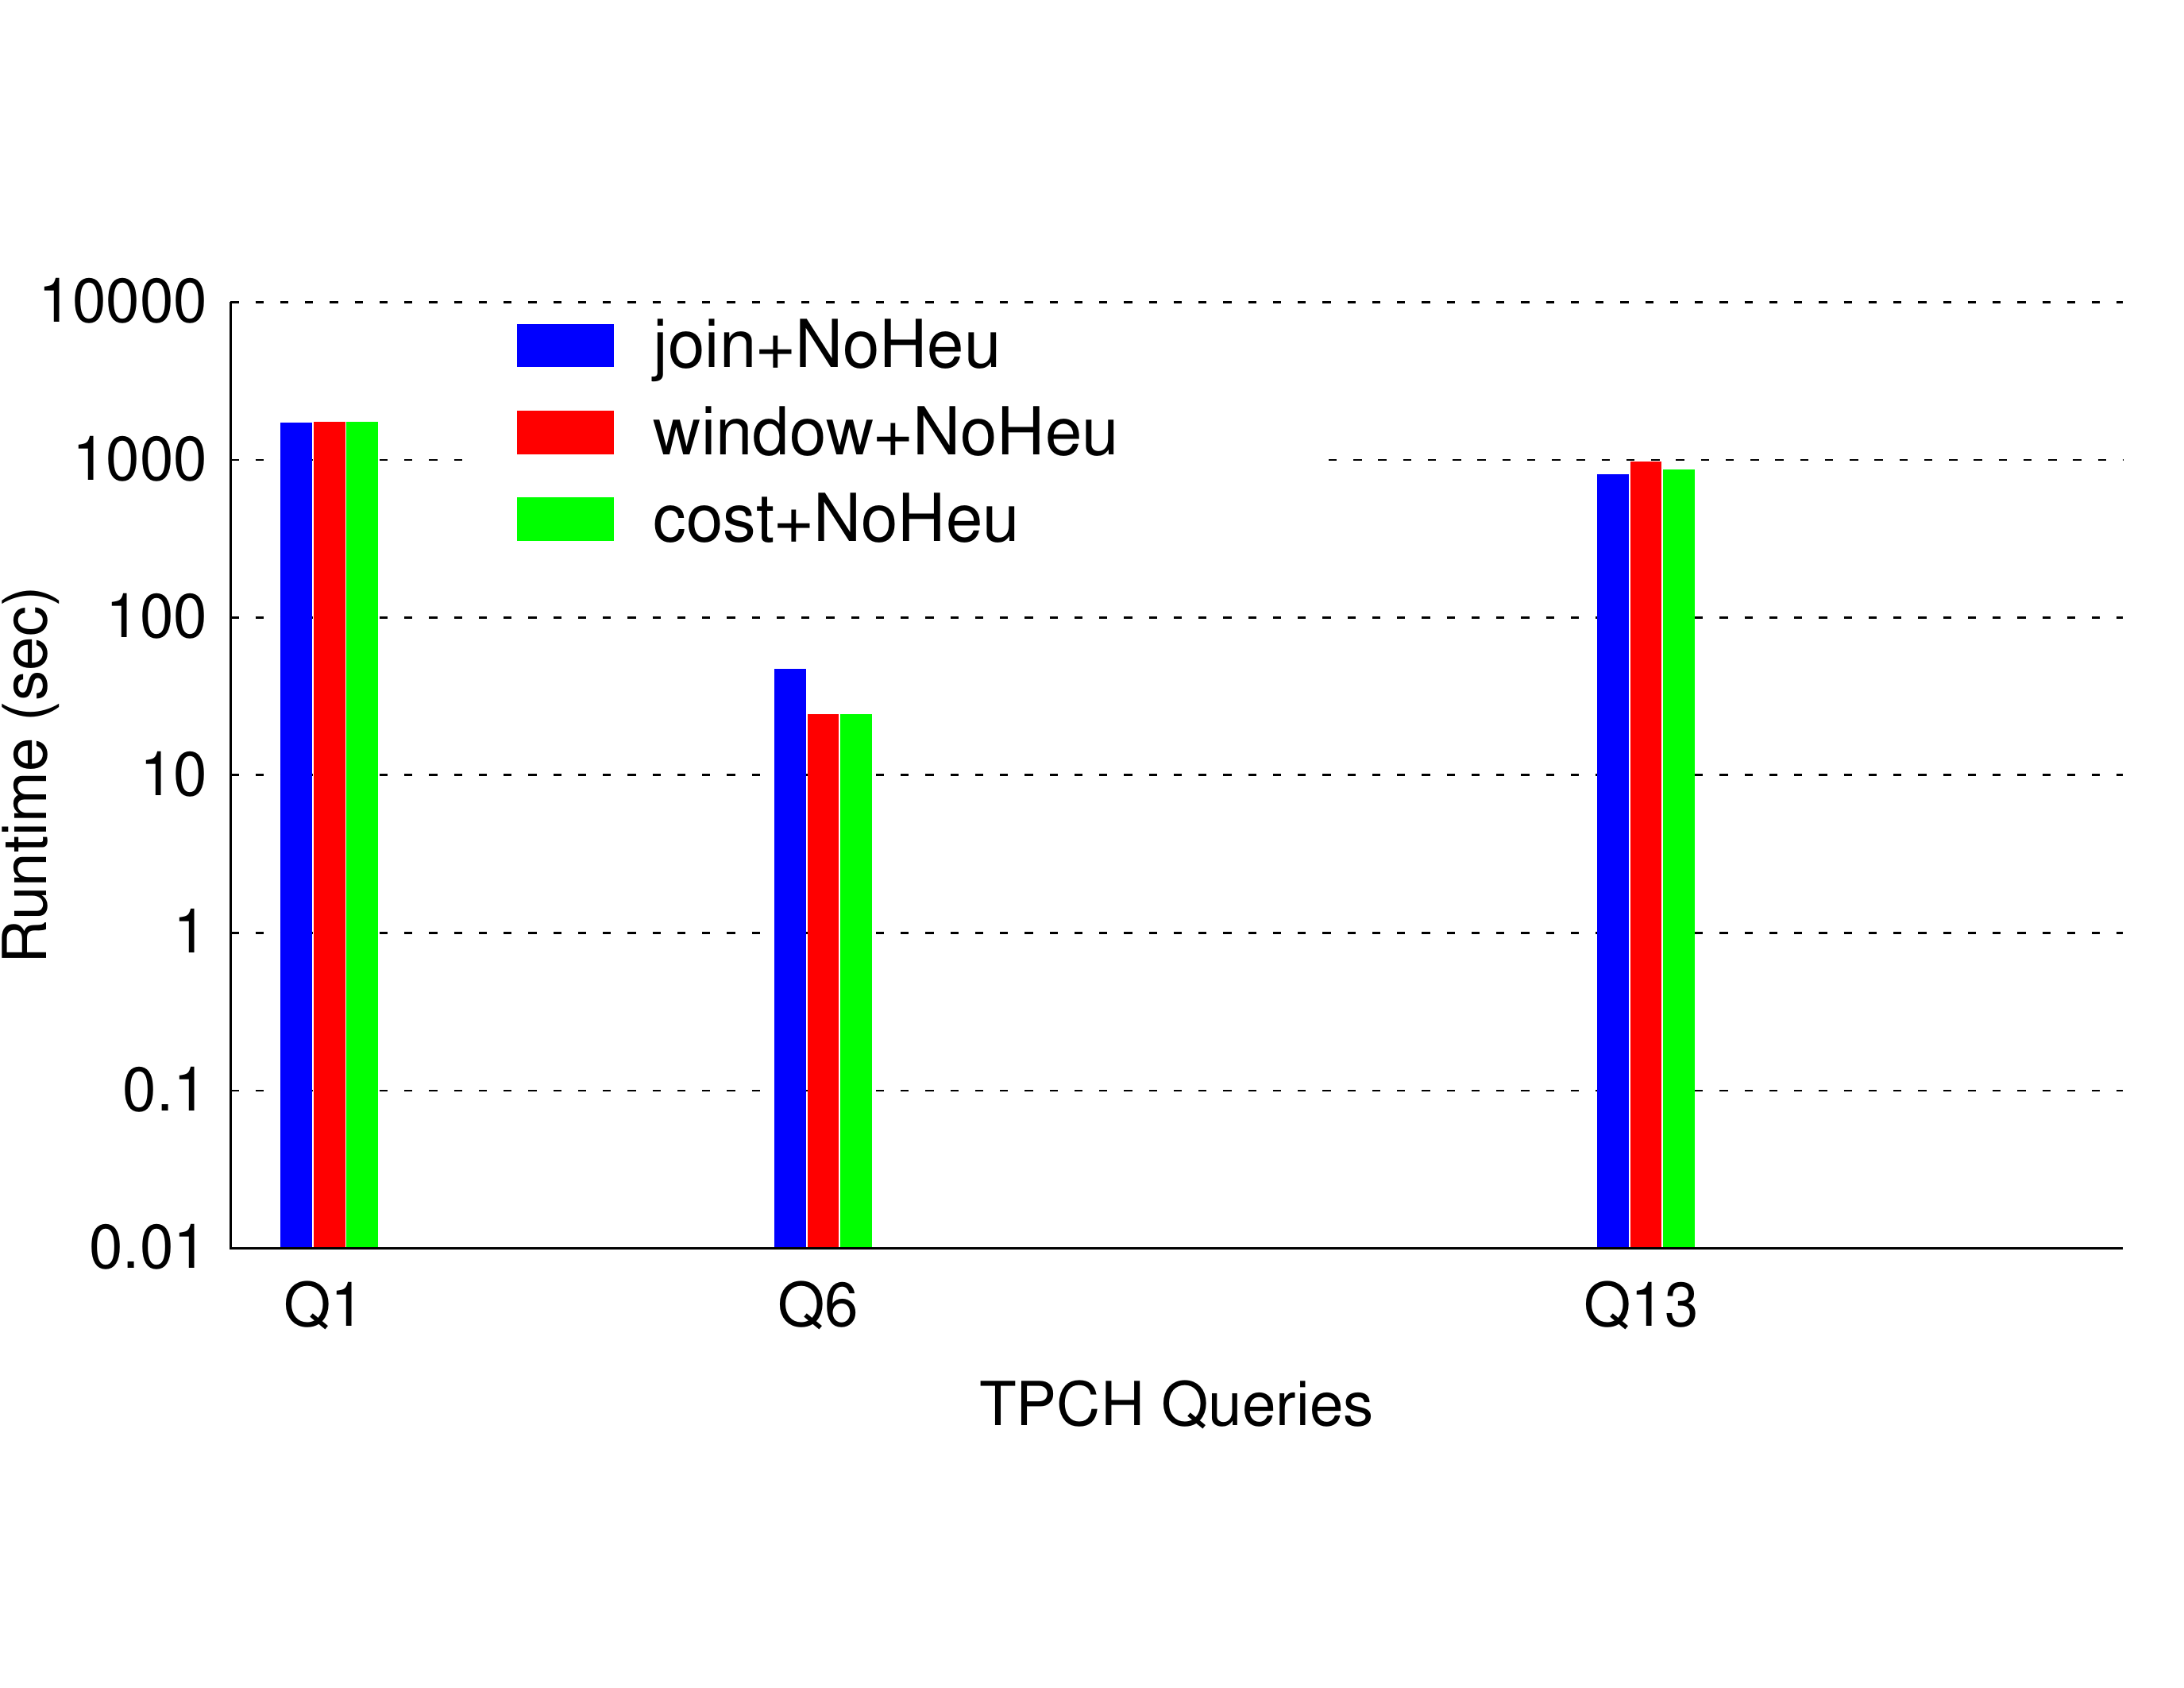}\\[-7mm]
  \caption{TPC-H Queries - NoOpt - 10GB}
  \label{fig:tpch-noopt-10GB}  
  \end{minipage}
%%%%%%%%%%%%%%%%%%%
  \begin{minipage}[b]{0.49\linewidth}
  \includegraphics[width=1\linewidth,trim=0 80pt 0 100pt, clip]{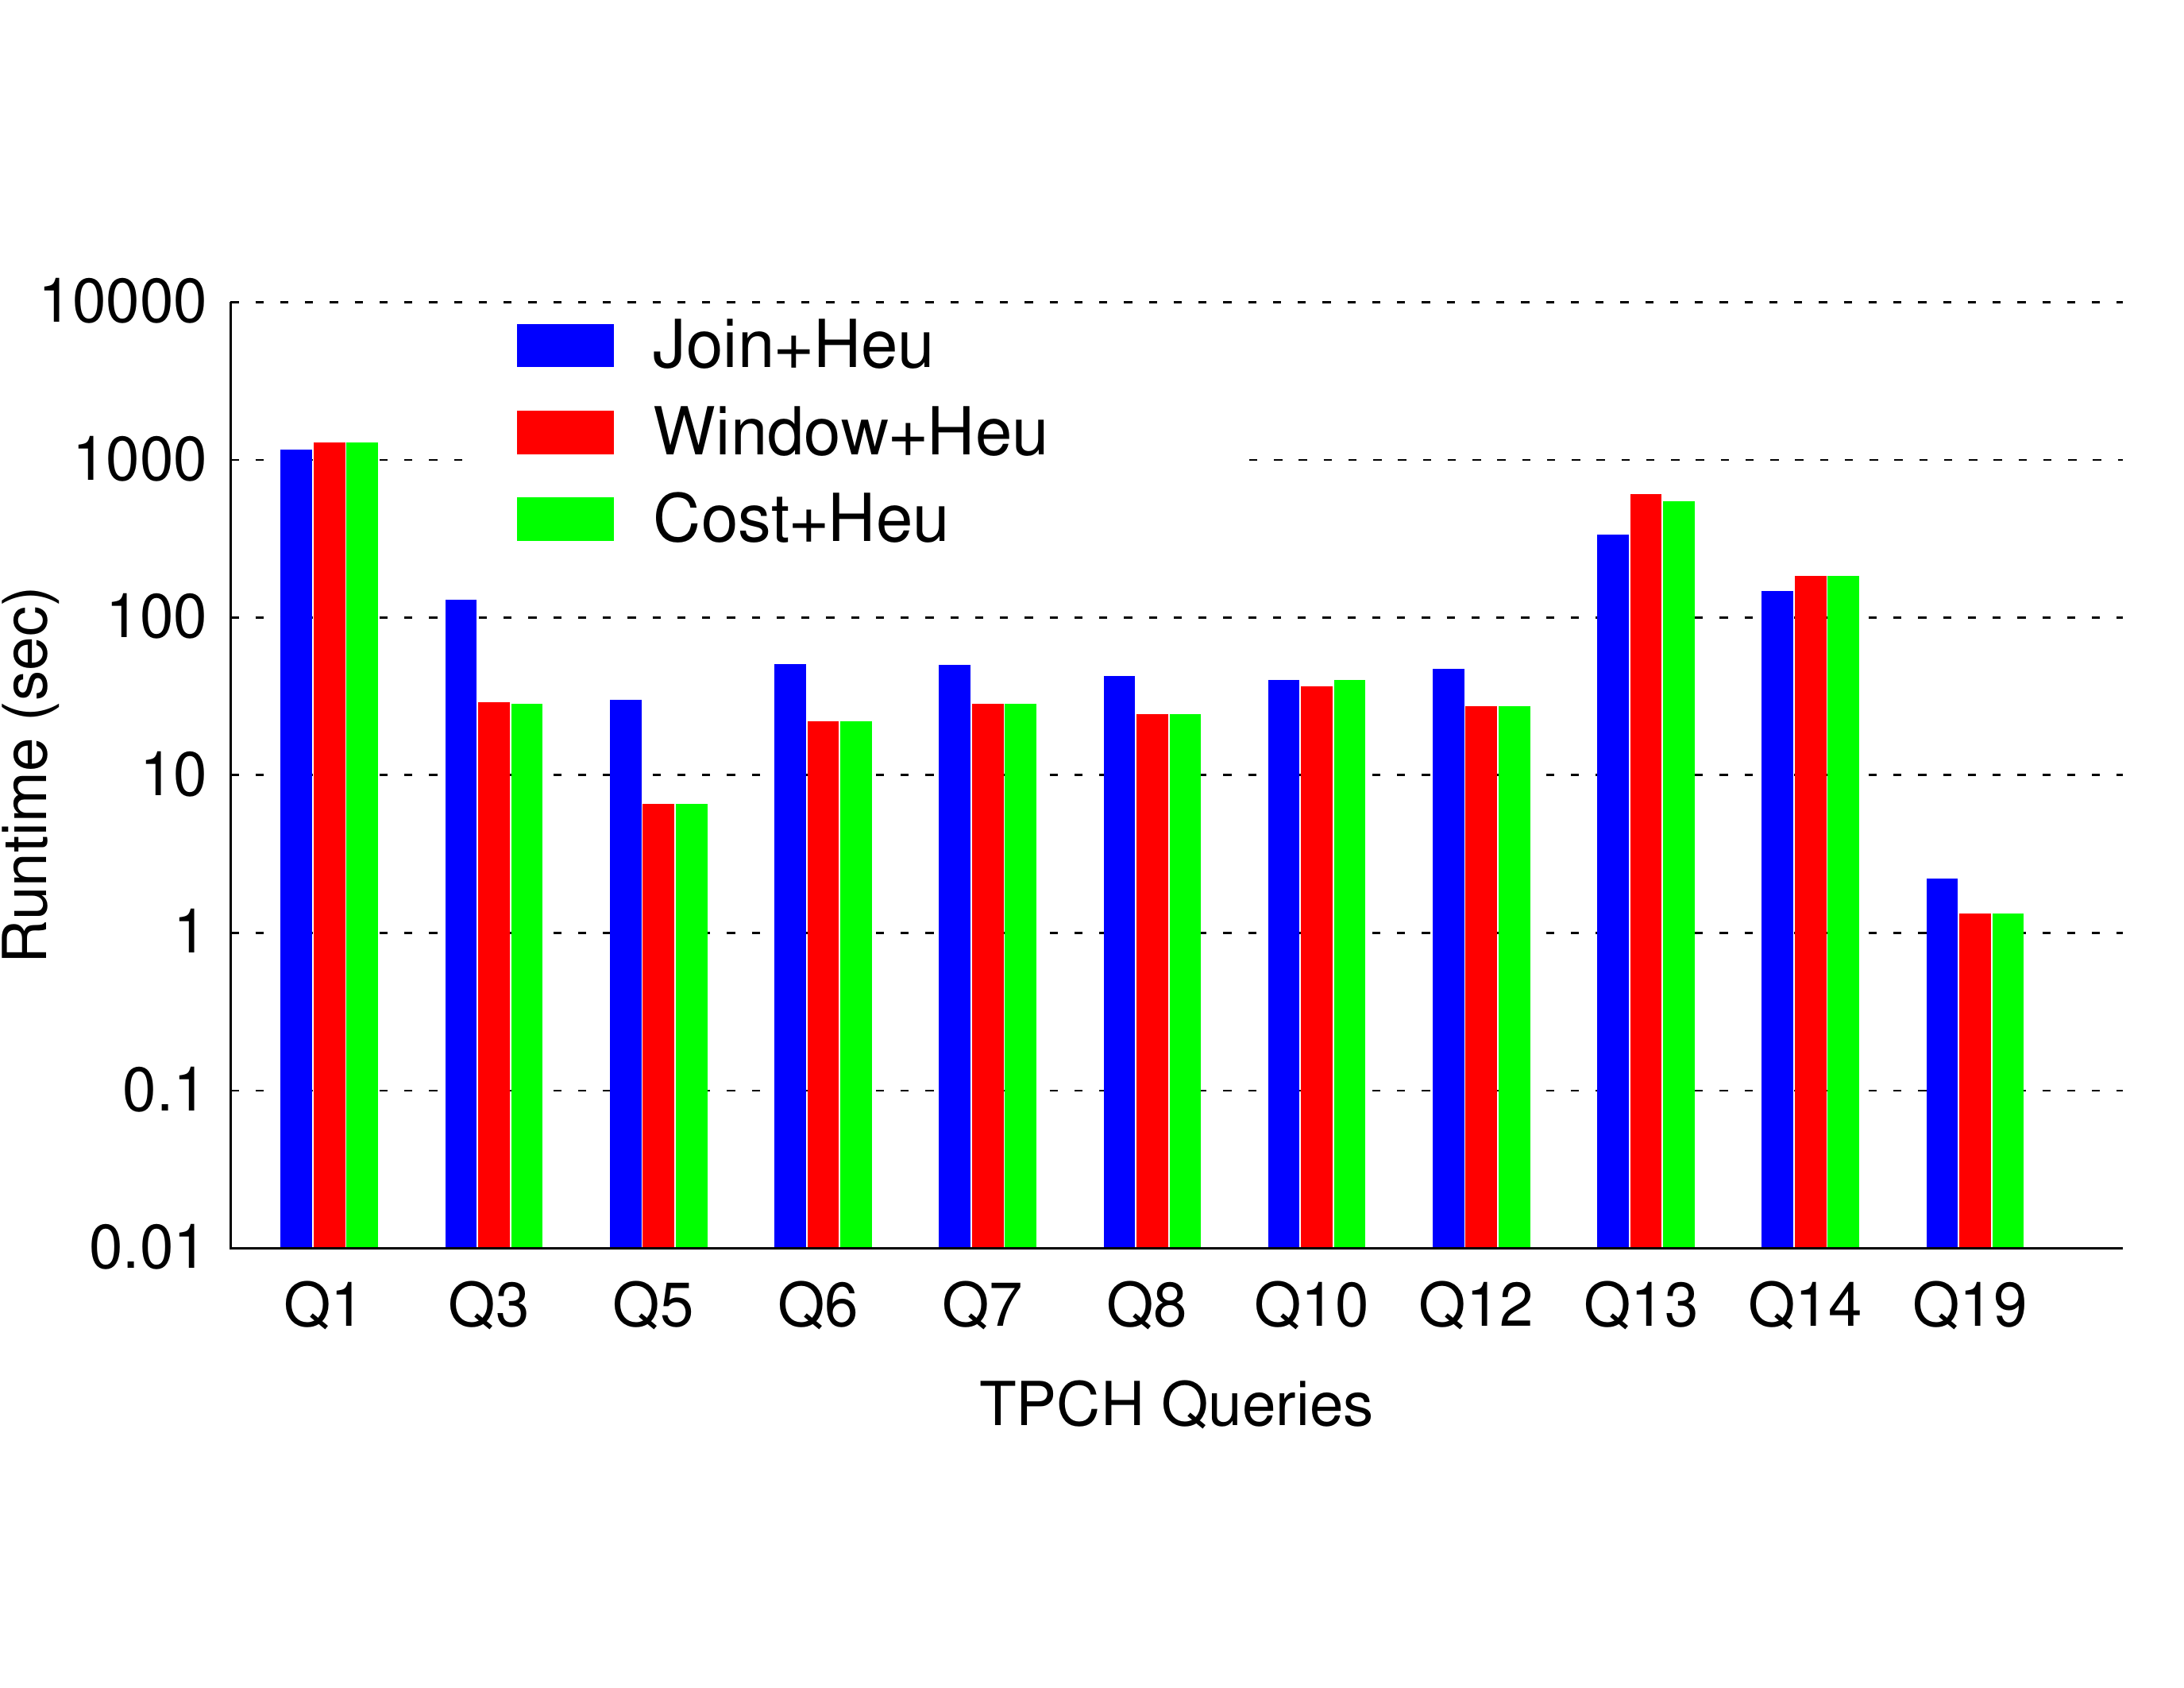}\\[-7mm] 
  \caption{TPC-H Queries - Opt - 10GB}
  \label{fig:tpch-opt-10GB}
  \end{minipage}
\end{figure*}
% %%%%%%%%%%%%%%%%%%%%%%%%%%%%%%%%%%%%%%%%%%%%%%%%%%%%%%%%%%%%

%%%%%%%%%%%%%%%%%%%%%%%%%%%%%%%%%%%%%%%%%%%%%%%%%%%%%%%%%%%%
\begin{figure*}[t]
%%%%%%%%%%%%%%%%%%%%
  \begin{minipage}[b]{0.49\linewidth}
  \includegraphics[width=1\linewidth,trim=0 80pt 0 100pt, clip]{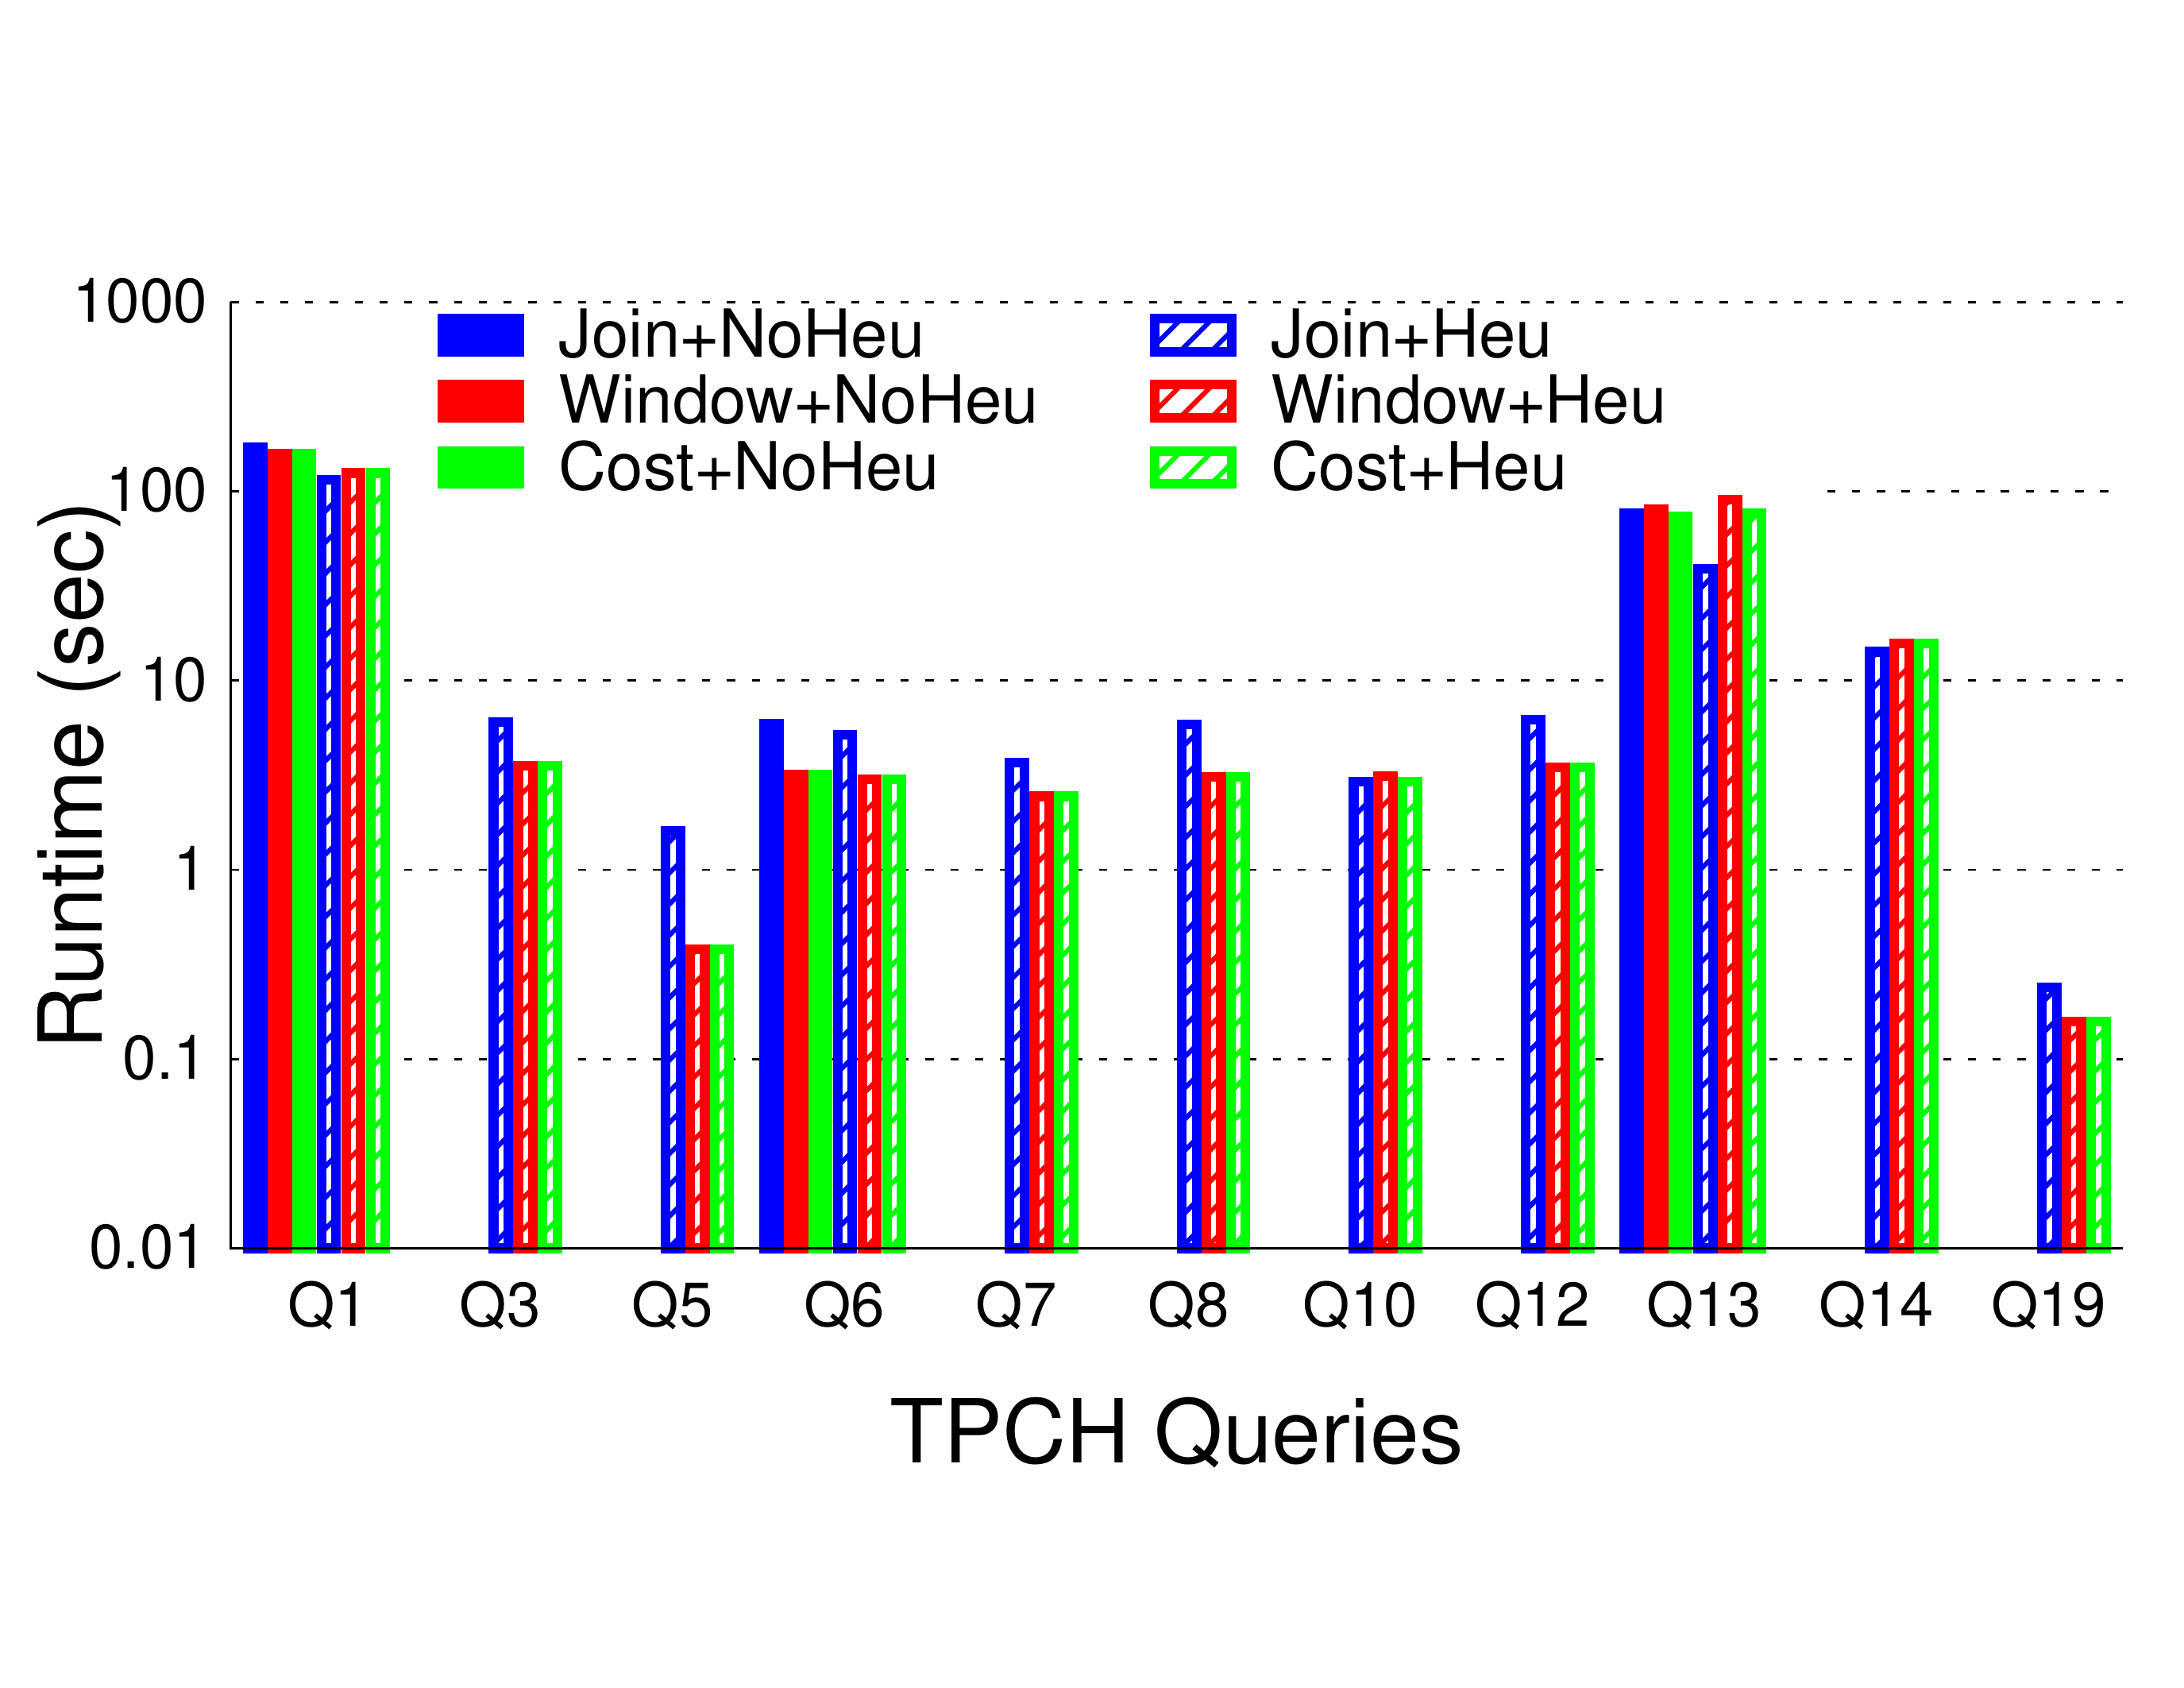}\\[-7mm]
  \caption{TPC-H Queries.  - 1GB}
  \label{fig:tpch-comb-1GB}  
  \end{minipage}
%%%%%%%%%%%%%%%%%%%
  \begin{minipage}[b]{0.49\linewidth}
  \includegraphics[width=1\linewidth,trim=0 80pt 0 100pt, clip]{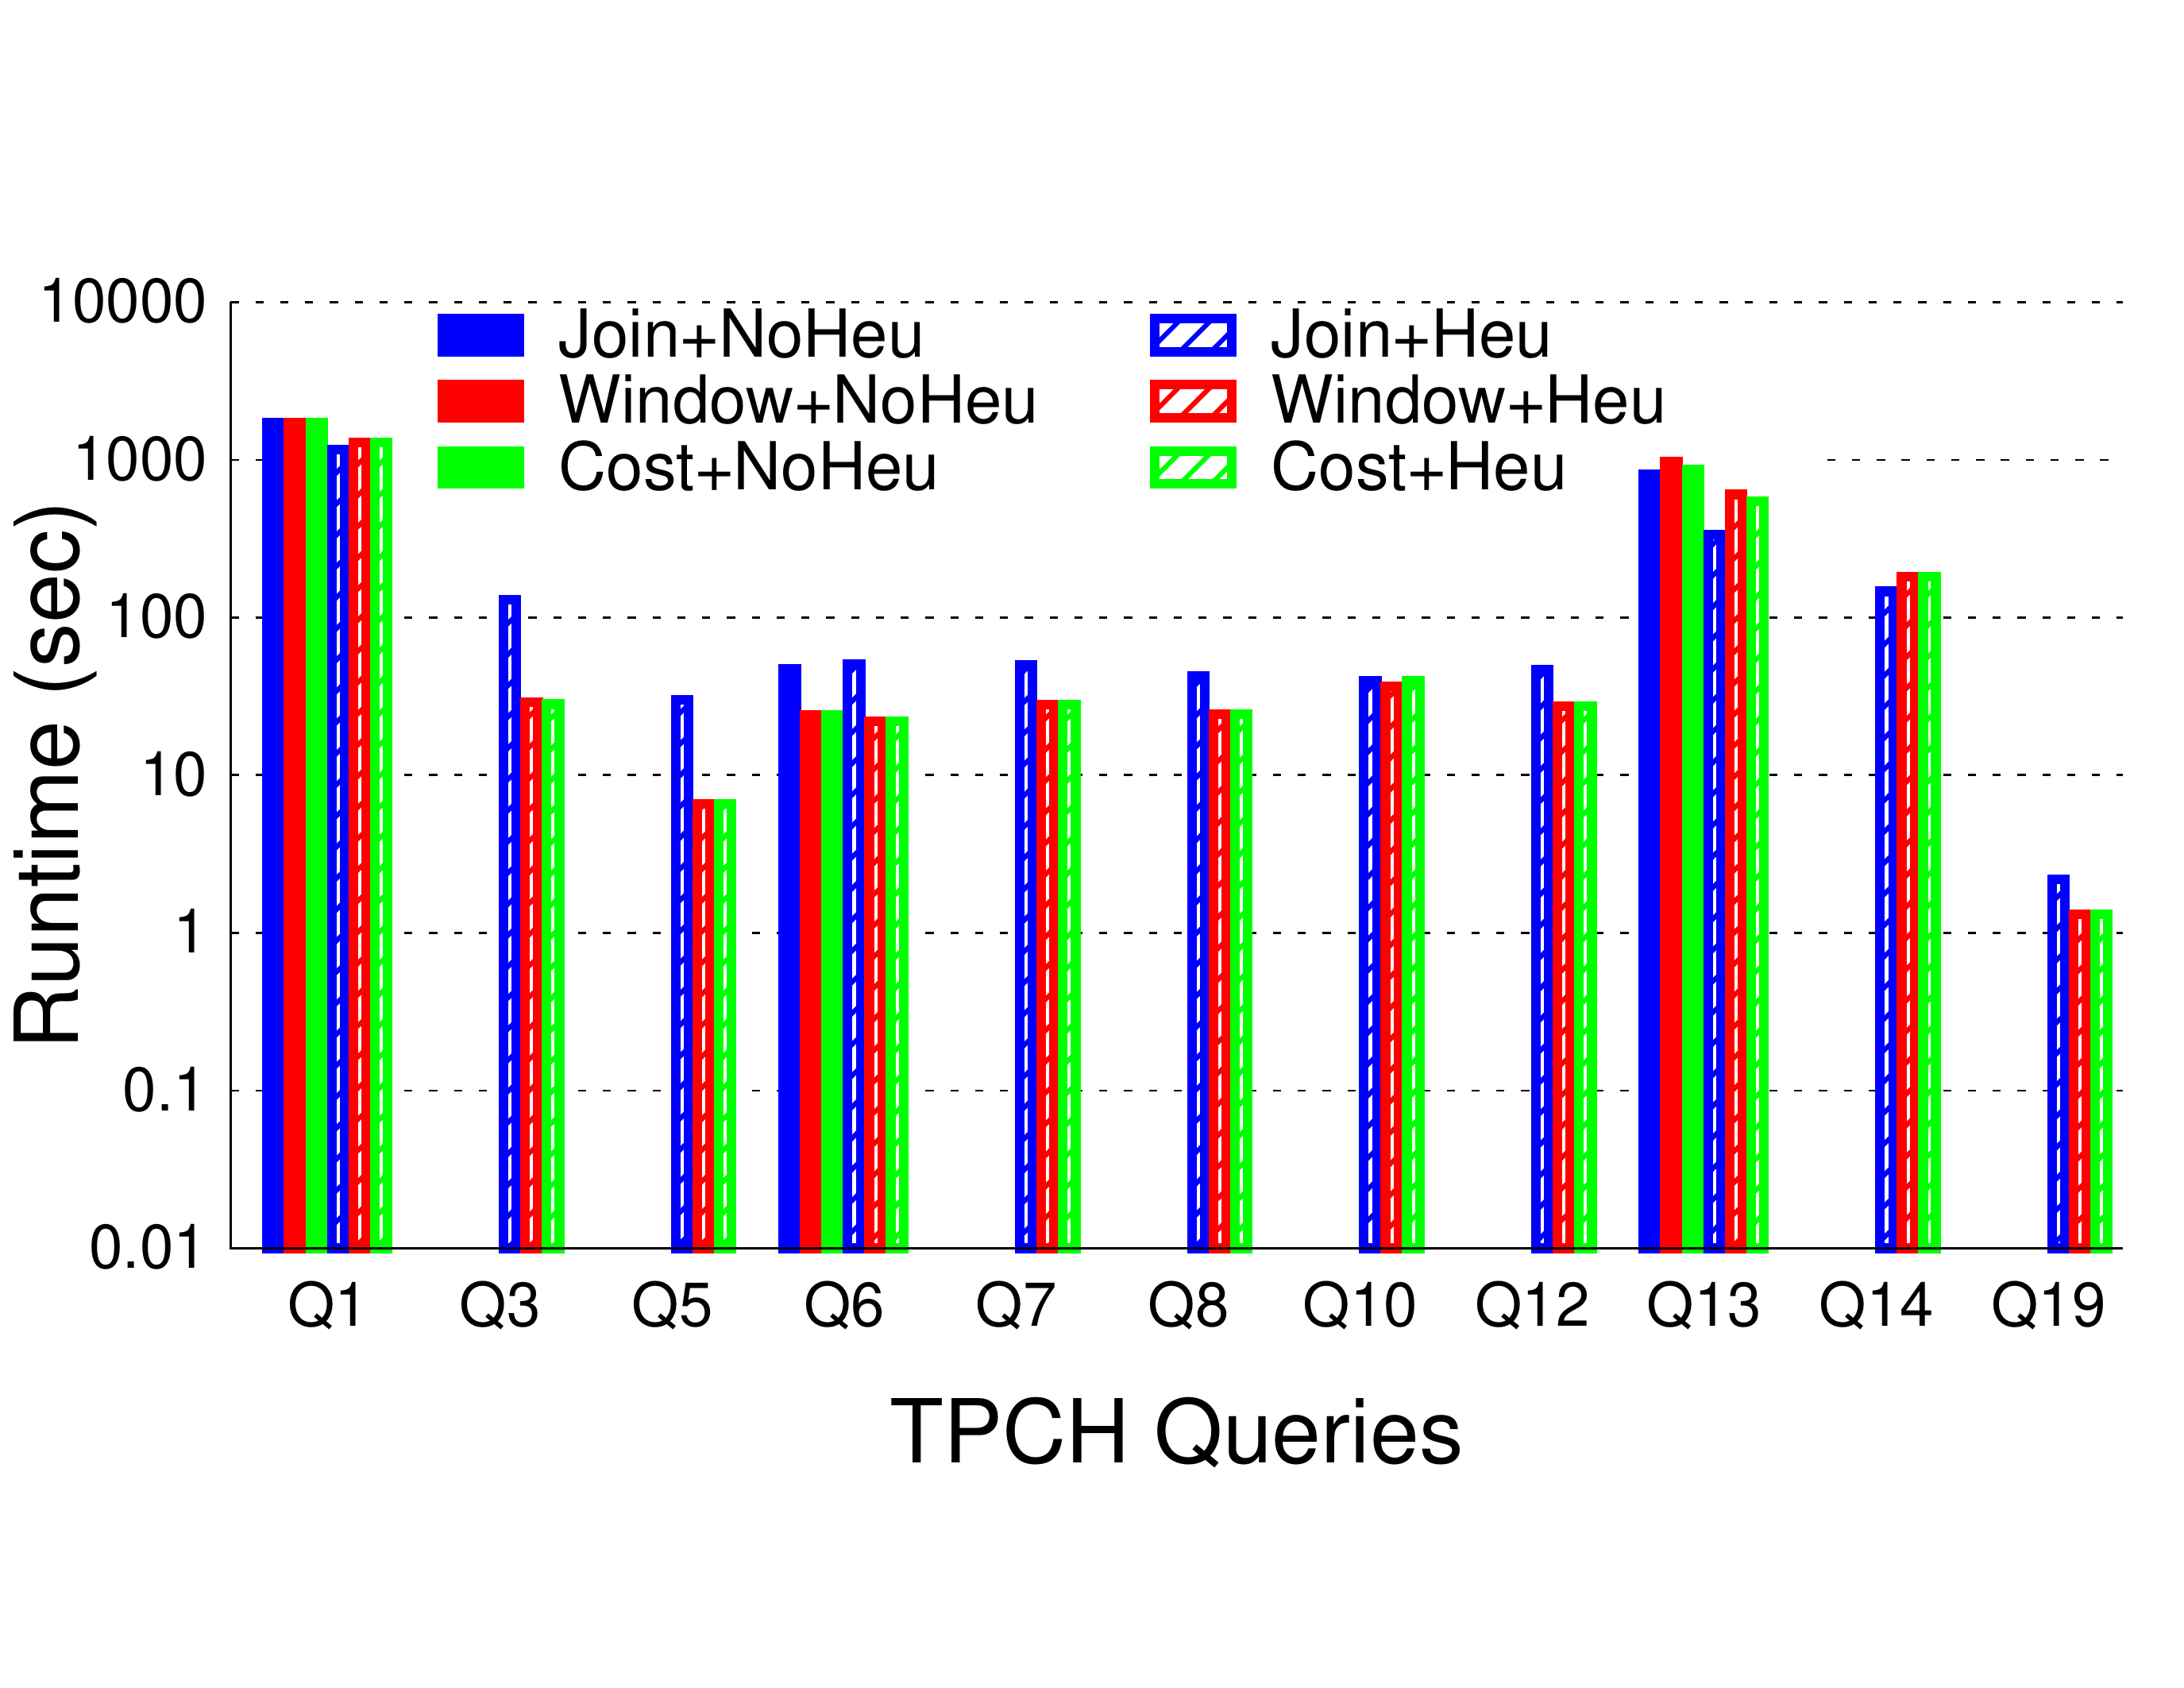}\\[-7mm] 
  \caption{TPC-H Queries. - 10GB}
  \label{fig:tpch-comb-10GB}
  \end{minipage}
\end{figure*}
% %%%%%%%%%%%%%%%%%%%%%%%%%%%%%%%%%%%%%%%%%%%%%%%%%%%%%%%%%%%%

%%%%%%%%%%%%%%%%%%%%%%%%%%%%%%%%%%%%%%%%%%%%%%%%%%%%%%%%%%%%
\begin{figure*}[t]
%%%%%%%%%%%%%%%%%%%%
  \begin{minipage}[b]{0.49\linewidth}
  \includegraphics[width=1\linewidth,trim=0 80pt 0 100pt, clip]{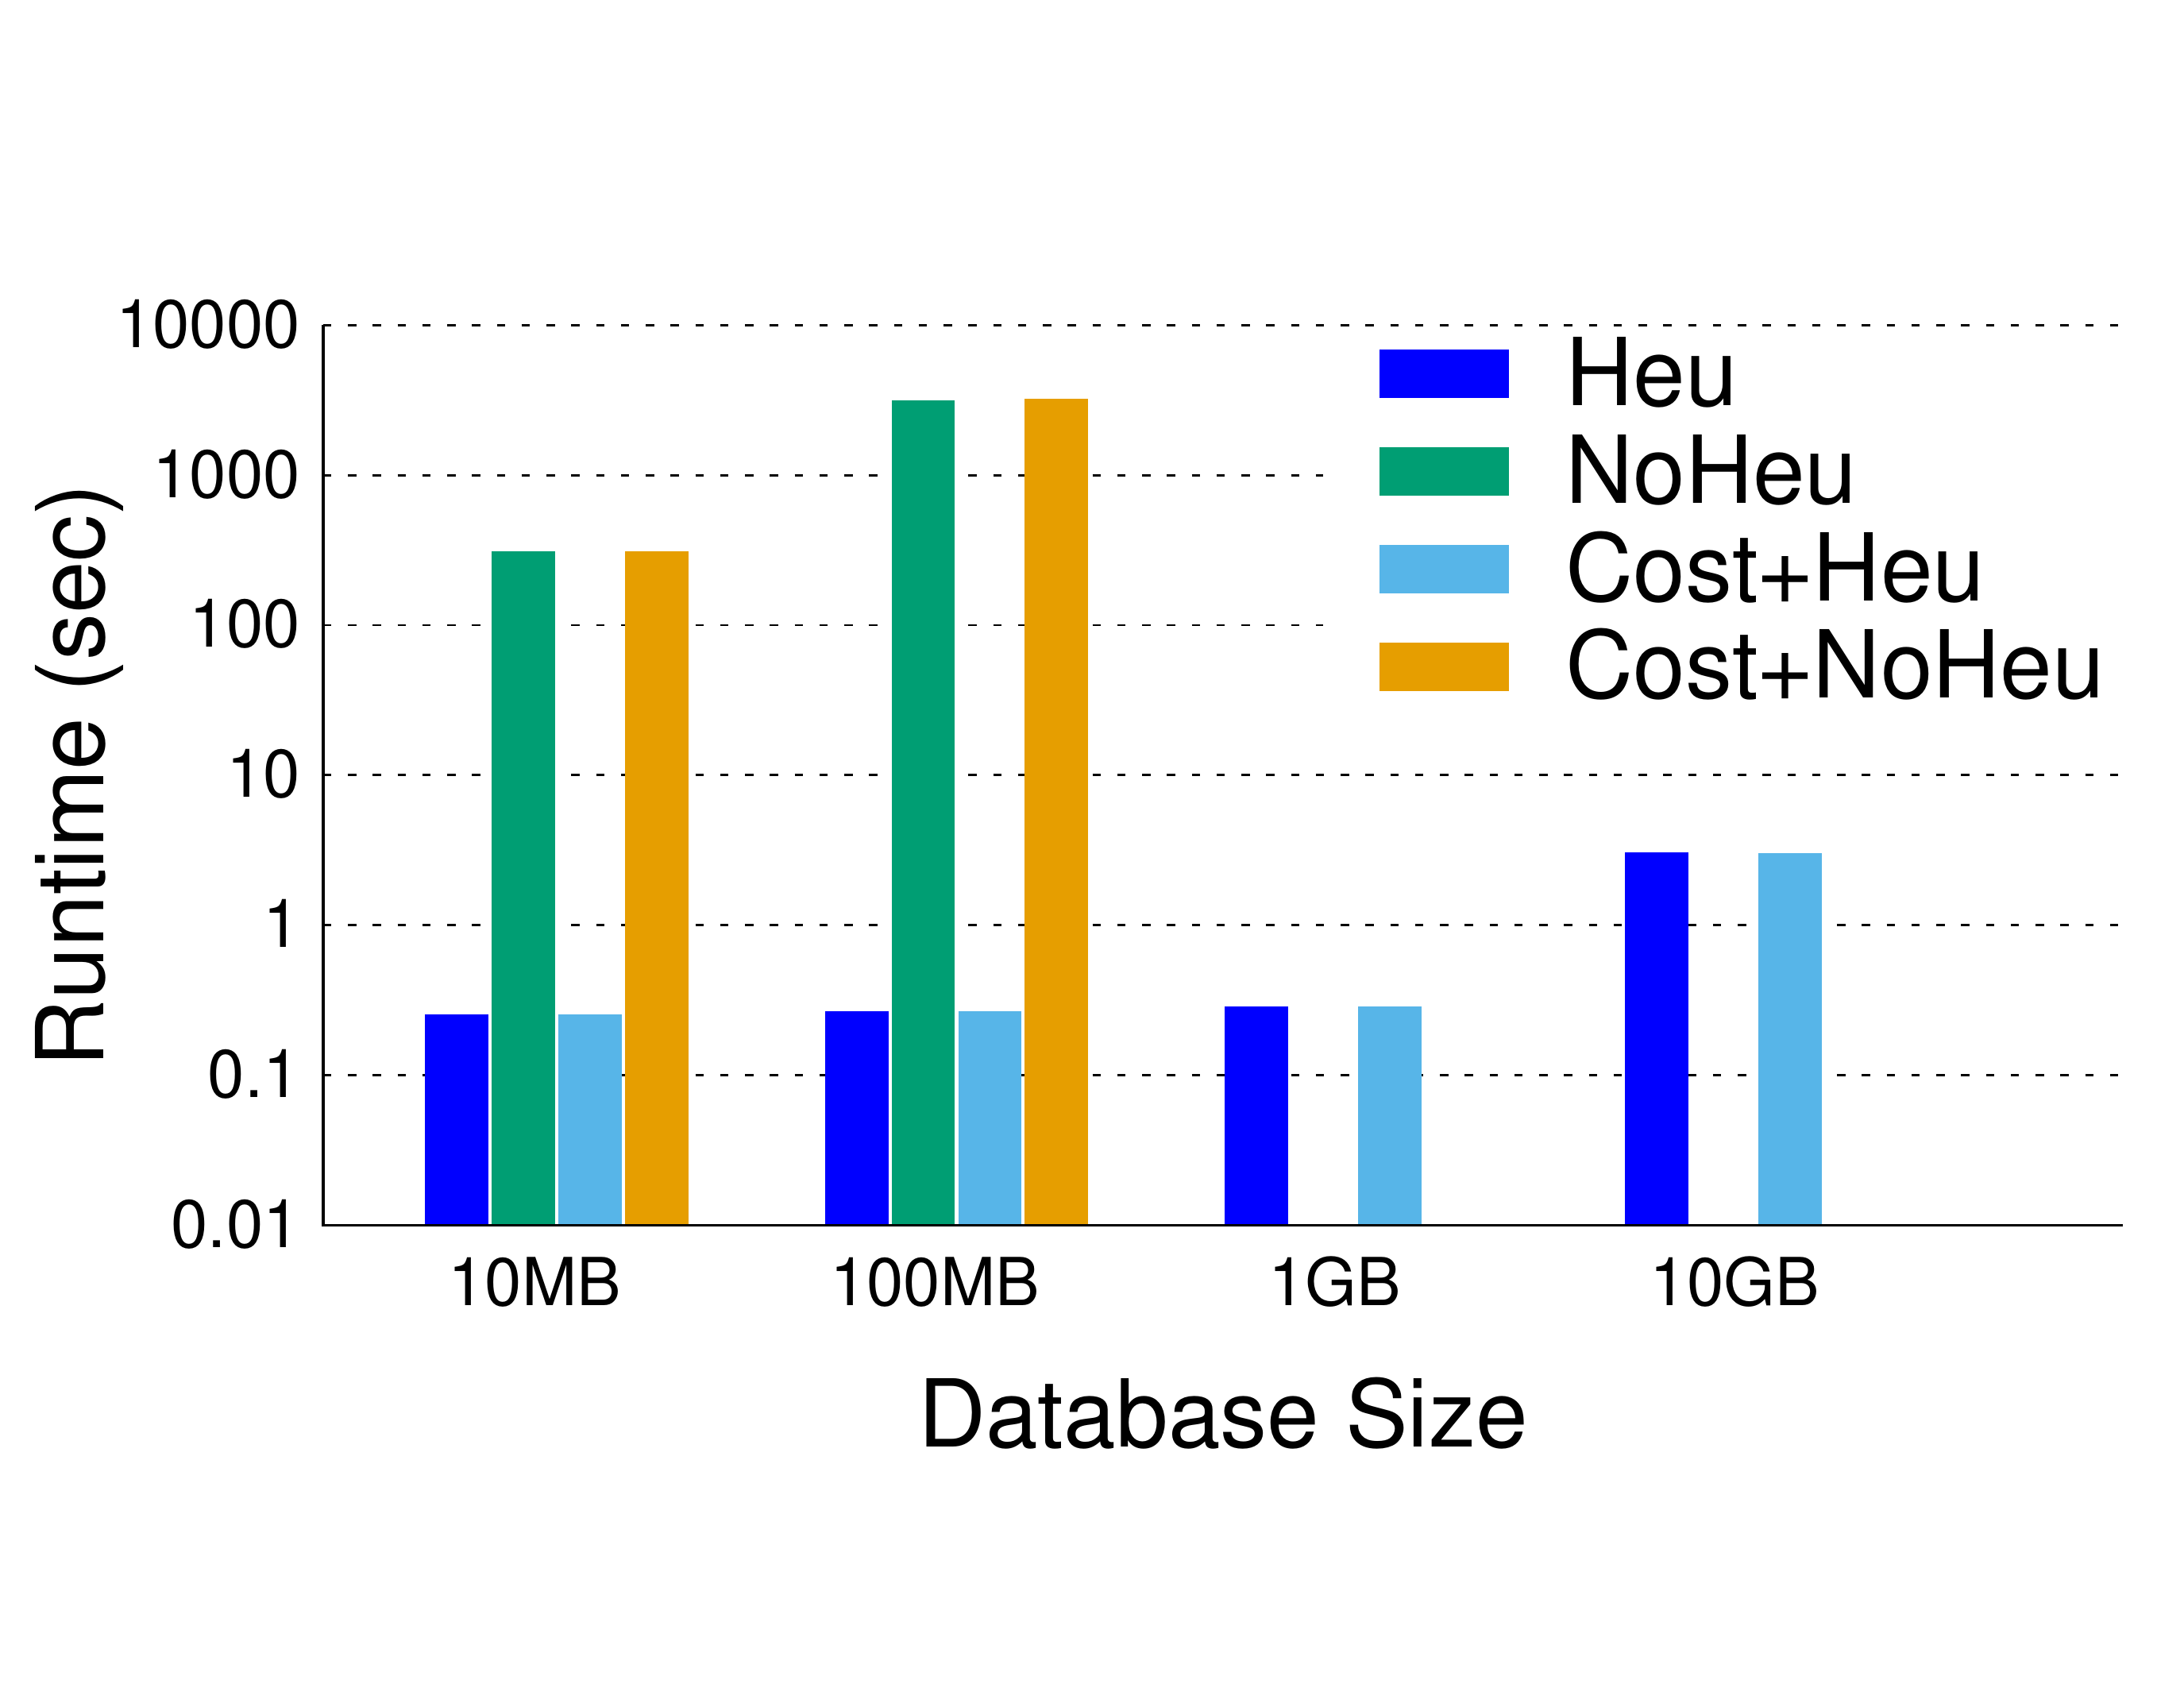}\\[-7mm]
  \caption{Export}
  \label{fig:export}  
  \end{minipage}
%%%%%%%%%%%%%%%%%%%
  \begin{minipage}[b]{0.49\linewidth}
  \includegraphics[width=1\linewidth,trim=0 80pt 0 100pt, clip]{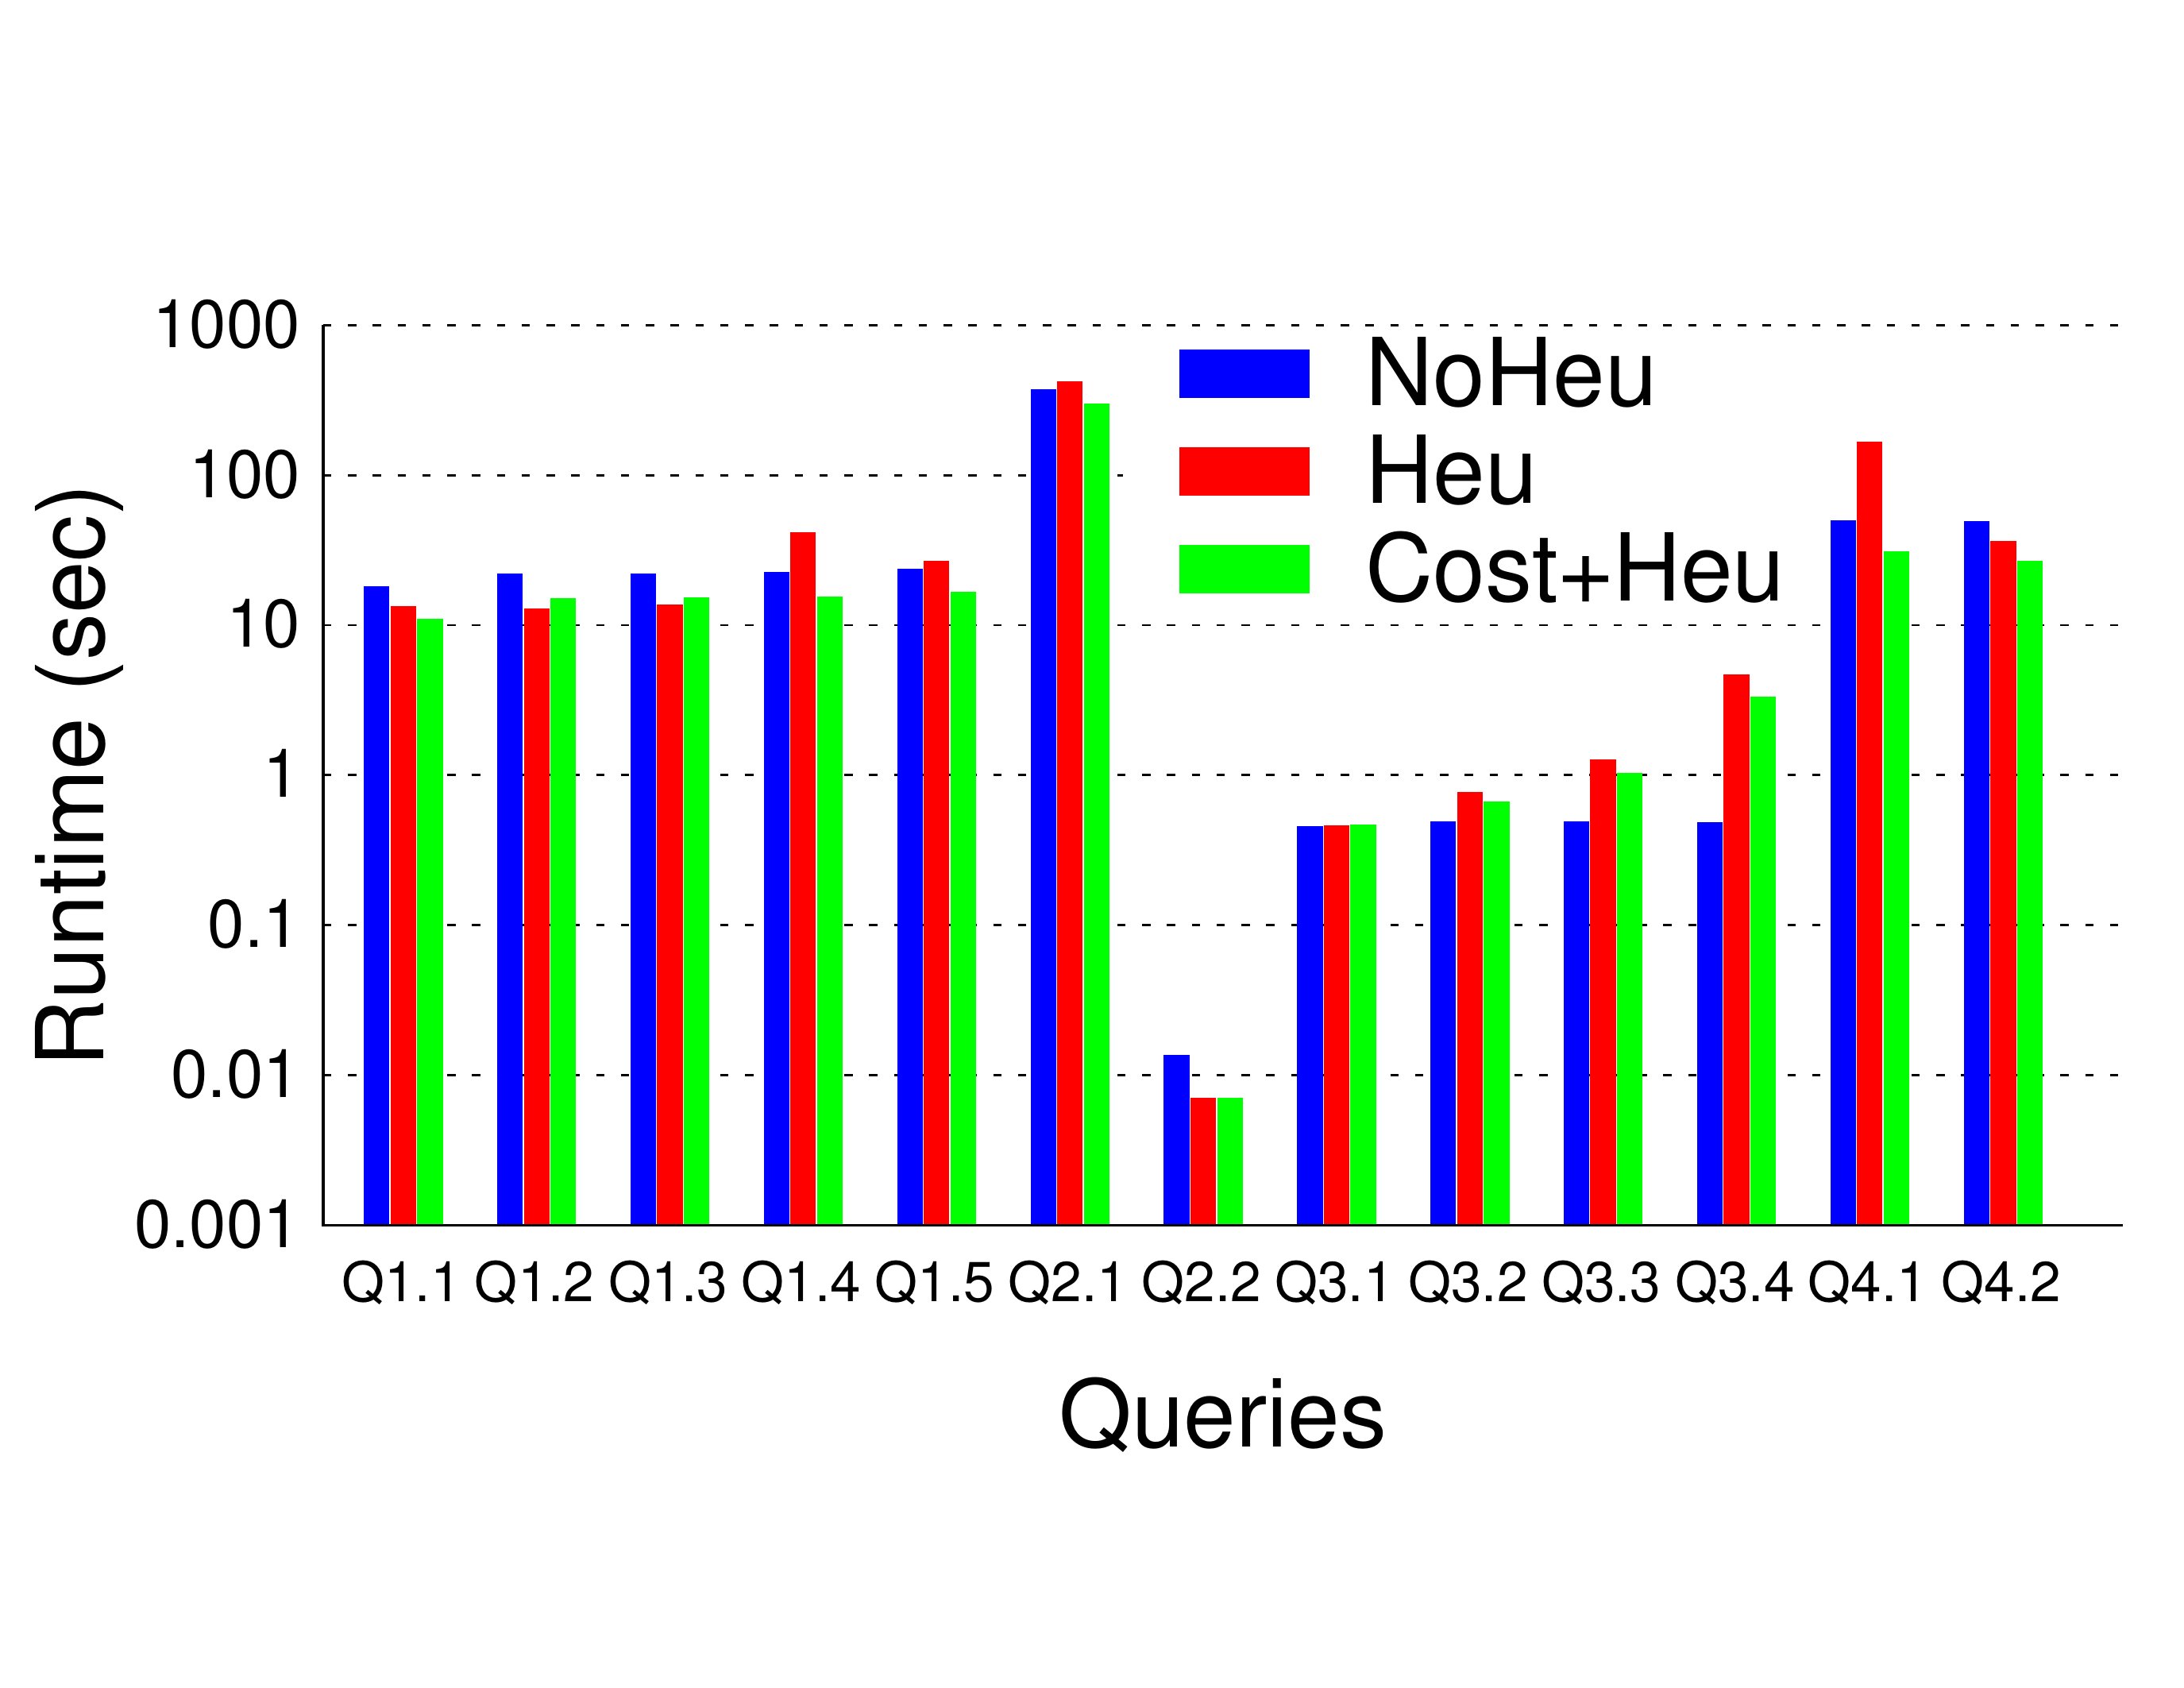}\\[-7mm] 
  \caption{Provenance Game}
  \label{fig:provenance-game}
  \end{minipage}
\end{figure*}
% %%%%%%%%%%%%%%%%%%%%%%%%%%%%%%%%%%%%%%%%%%%%%%%%%%%%%%%%%%%%

%%%%%%%%%%%%%%%%%%%%%%%%%%%%%%%%%%%%%%%%%%%%%%%%%%%%%%%%%%%%
\begin{figure*}[t]
%%%%%%%%%%%%%%%%%%%%
  \begin{minipage}[b]{0.49\linewidth}
  \includegraphics[width=1\linewidth,trim=0 80pt 0 100pt, clip]{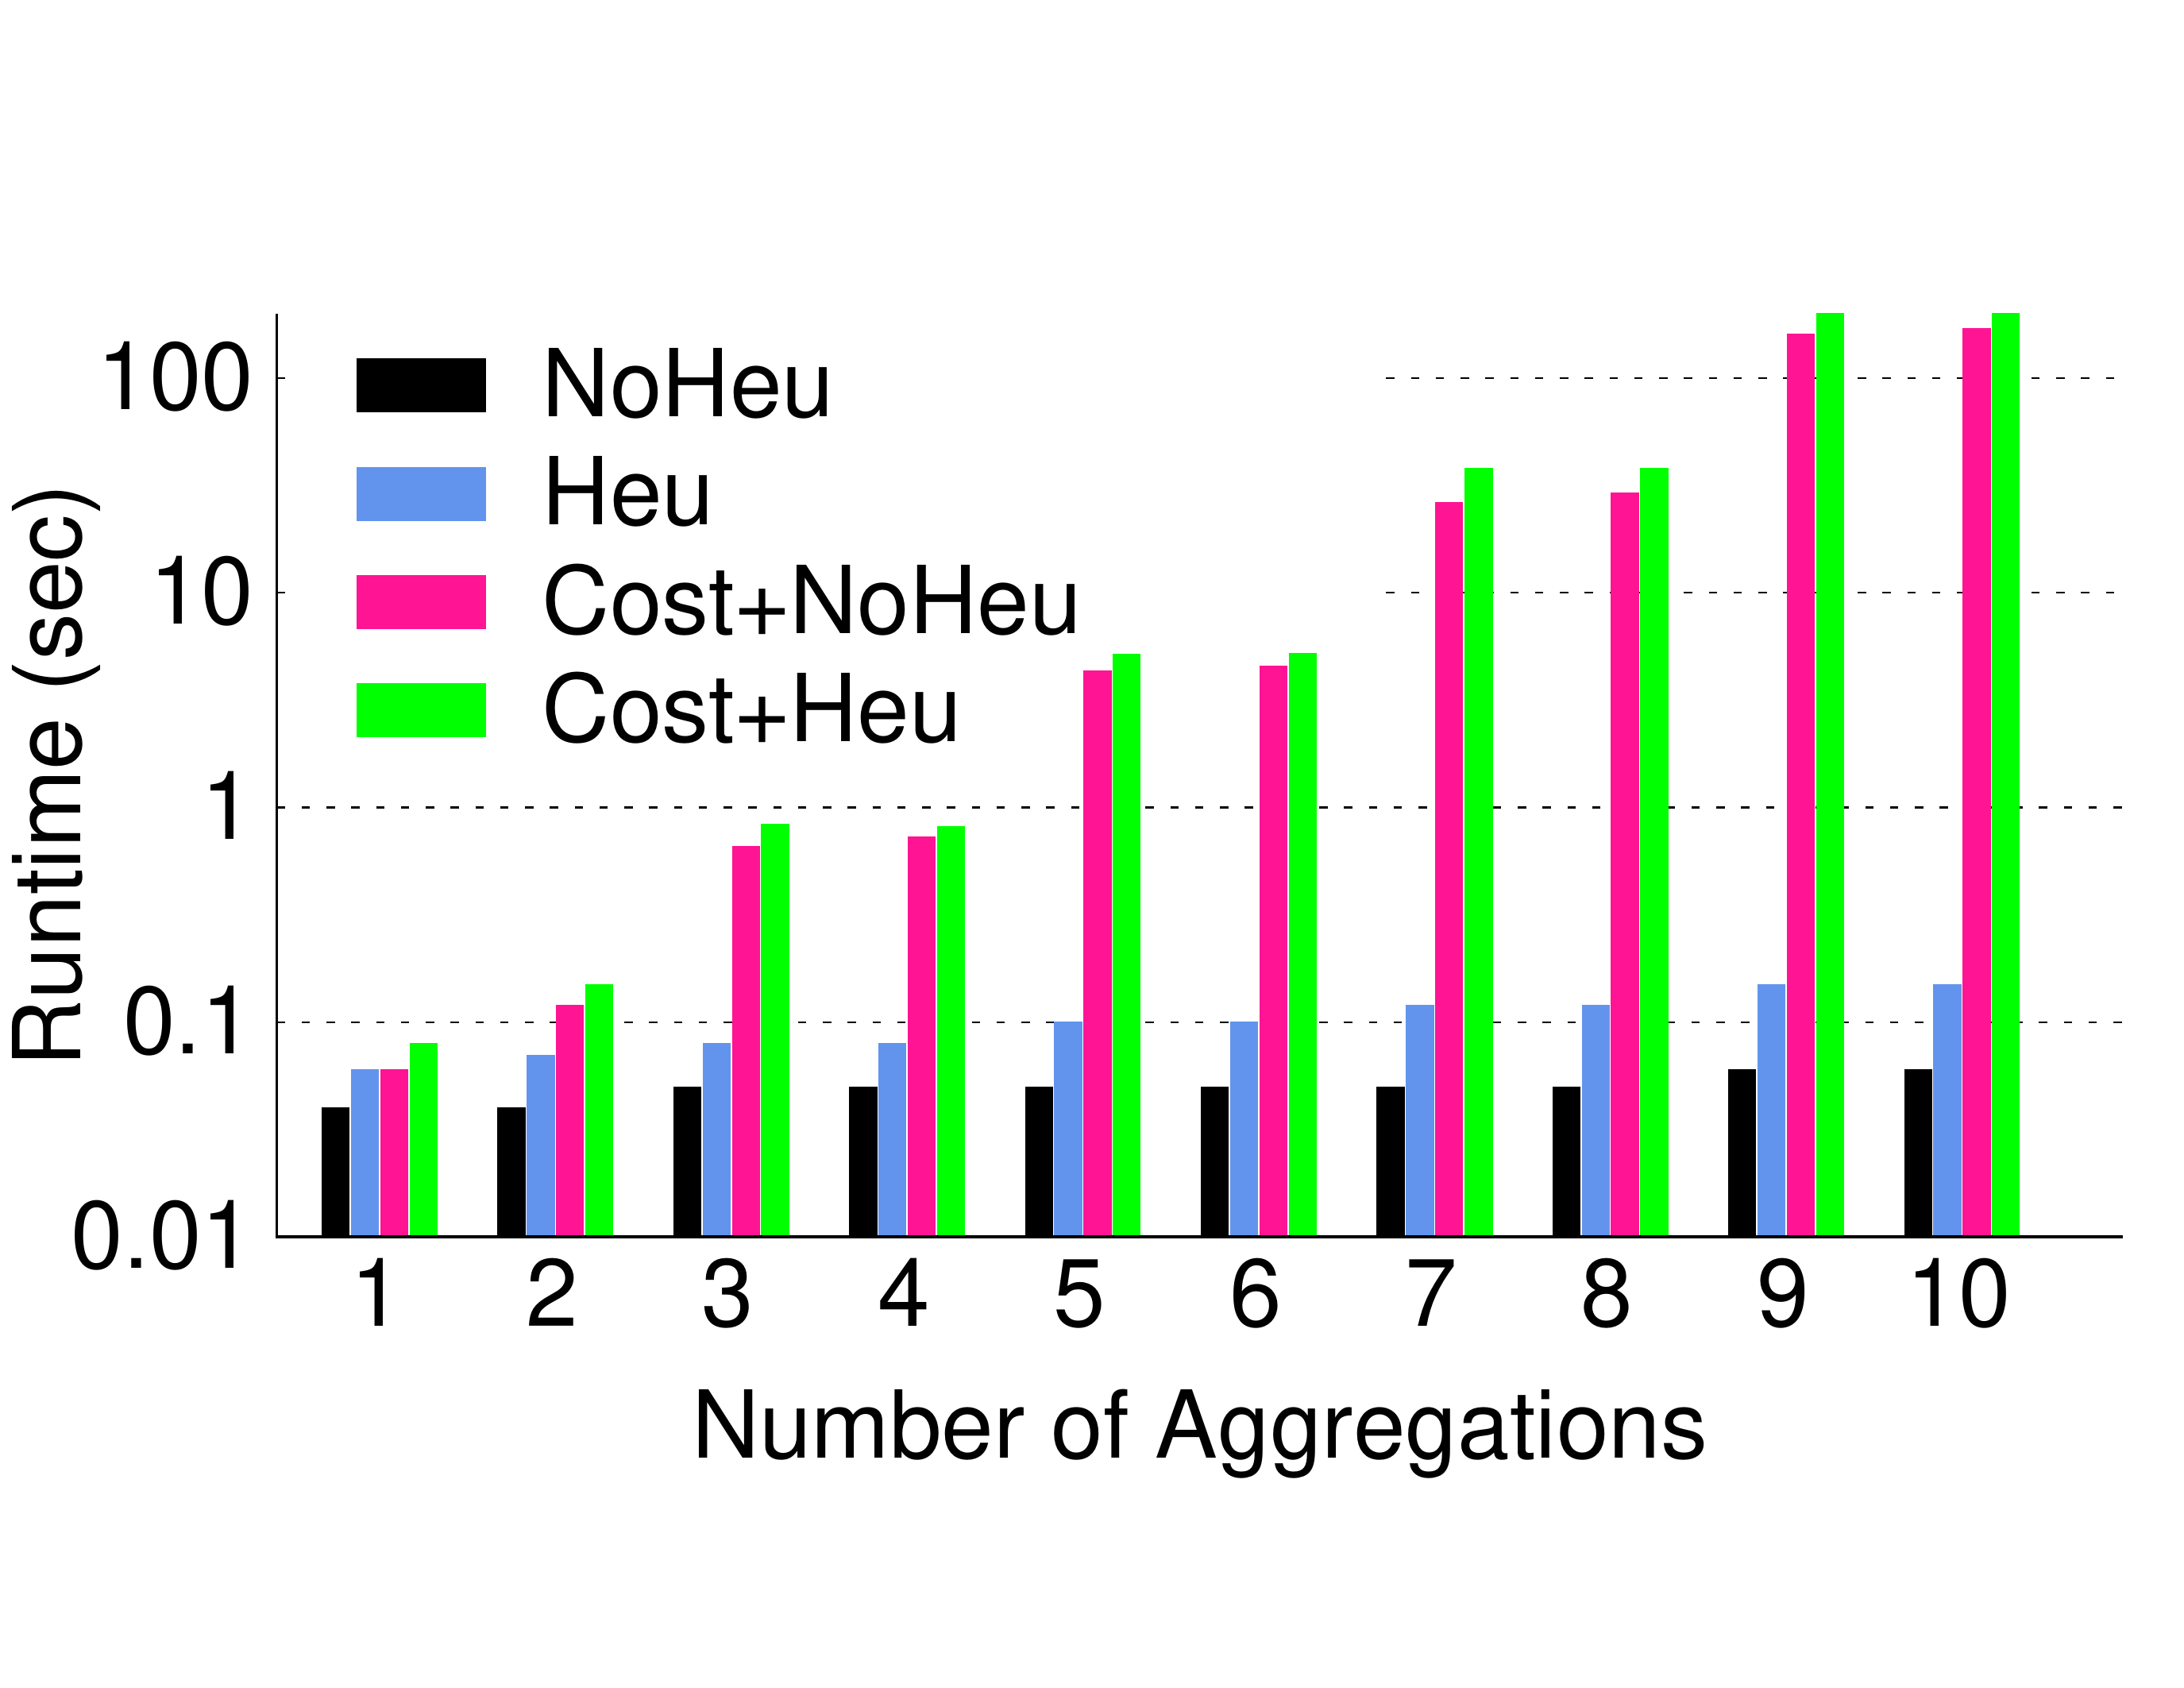}\\[-7mm]
  \caption{Simple Agg. Overhead}
  \label{fig:simple-agg-overhead}  
  \end{minipage}
%%%%%%%%%%%%%%%%%%%
  \begin{minipage}[b]{0.49\linewidth}
  \includegraphics[width=1\linewidth,trim=0 80pt 0 100pt, clip]{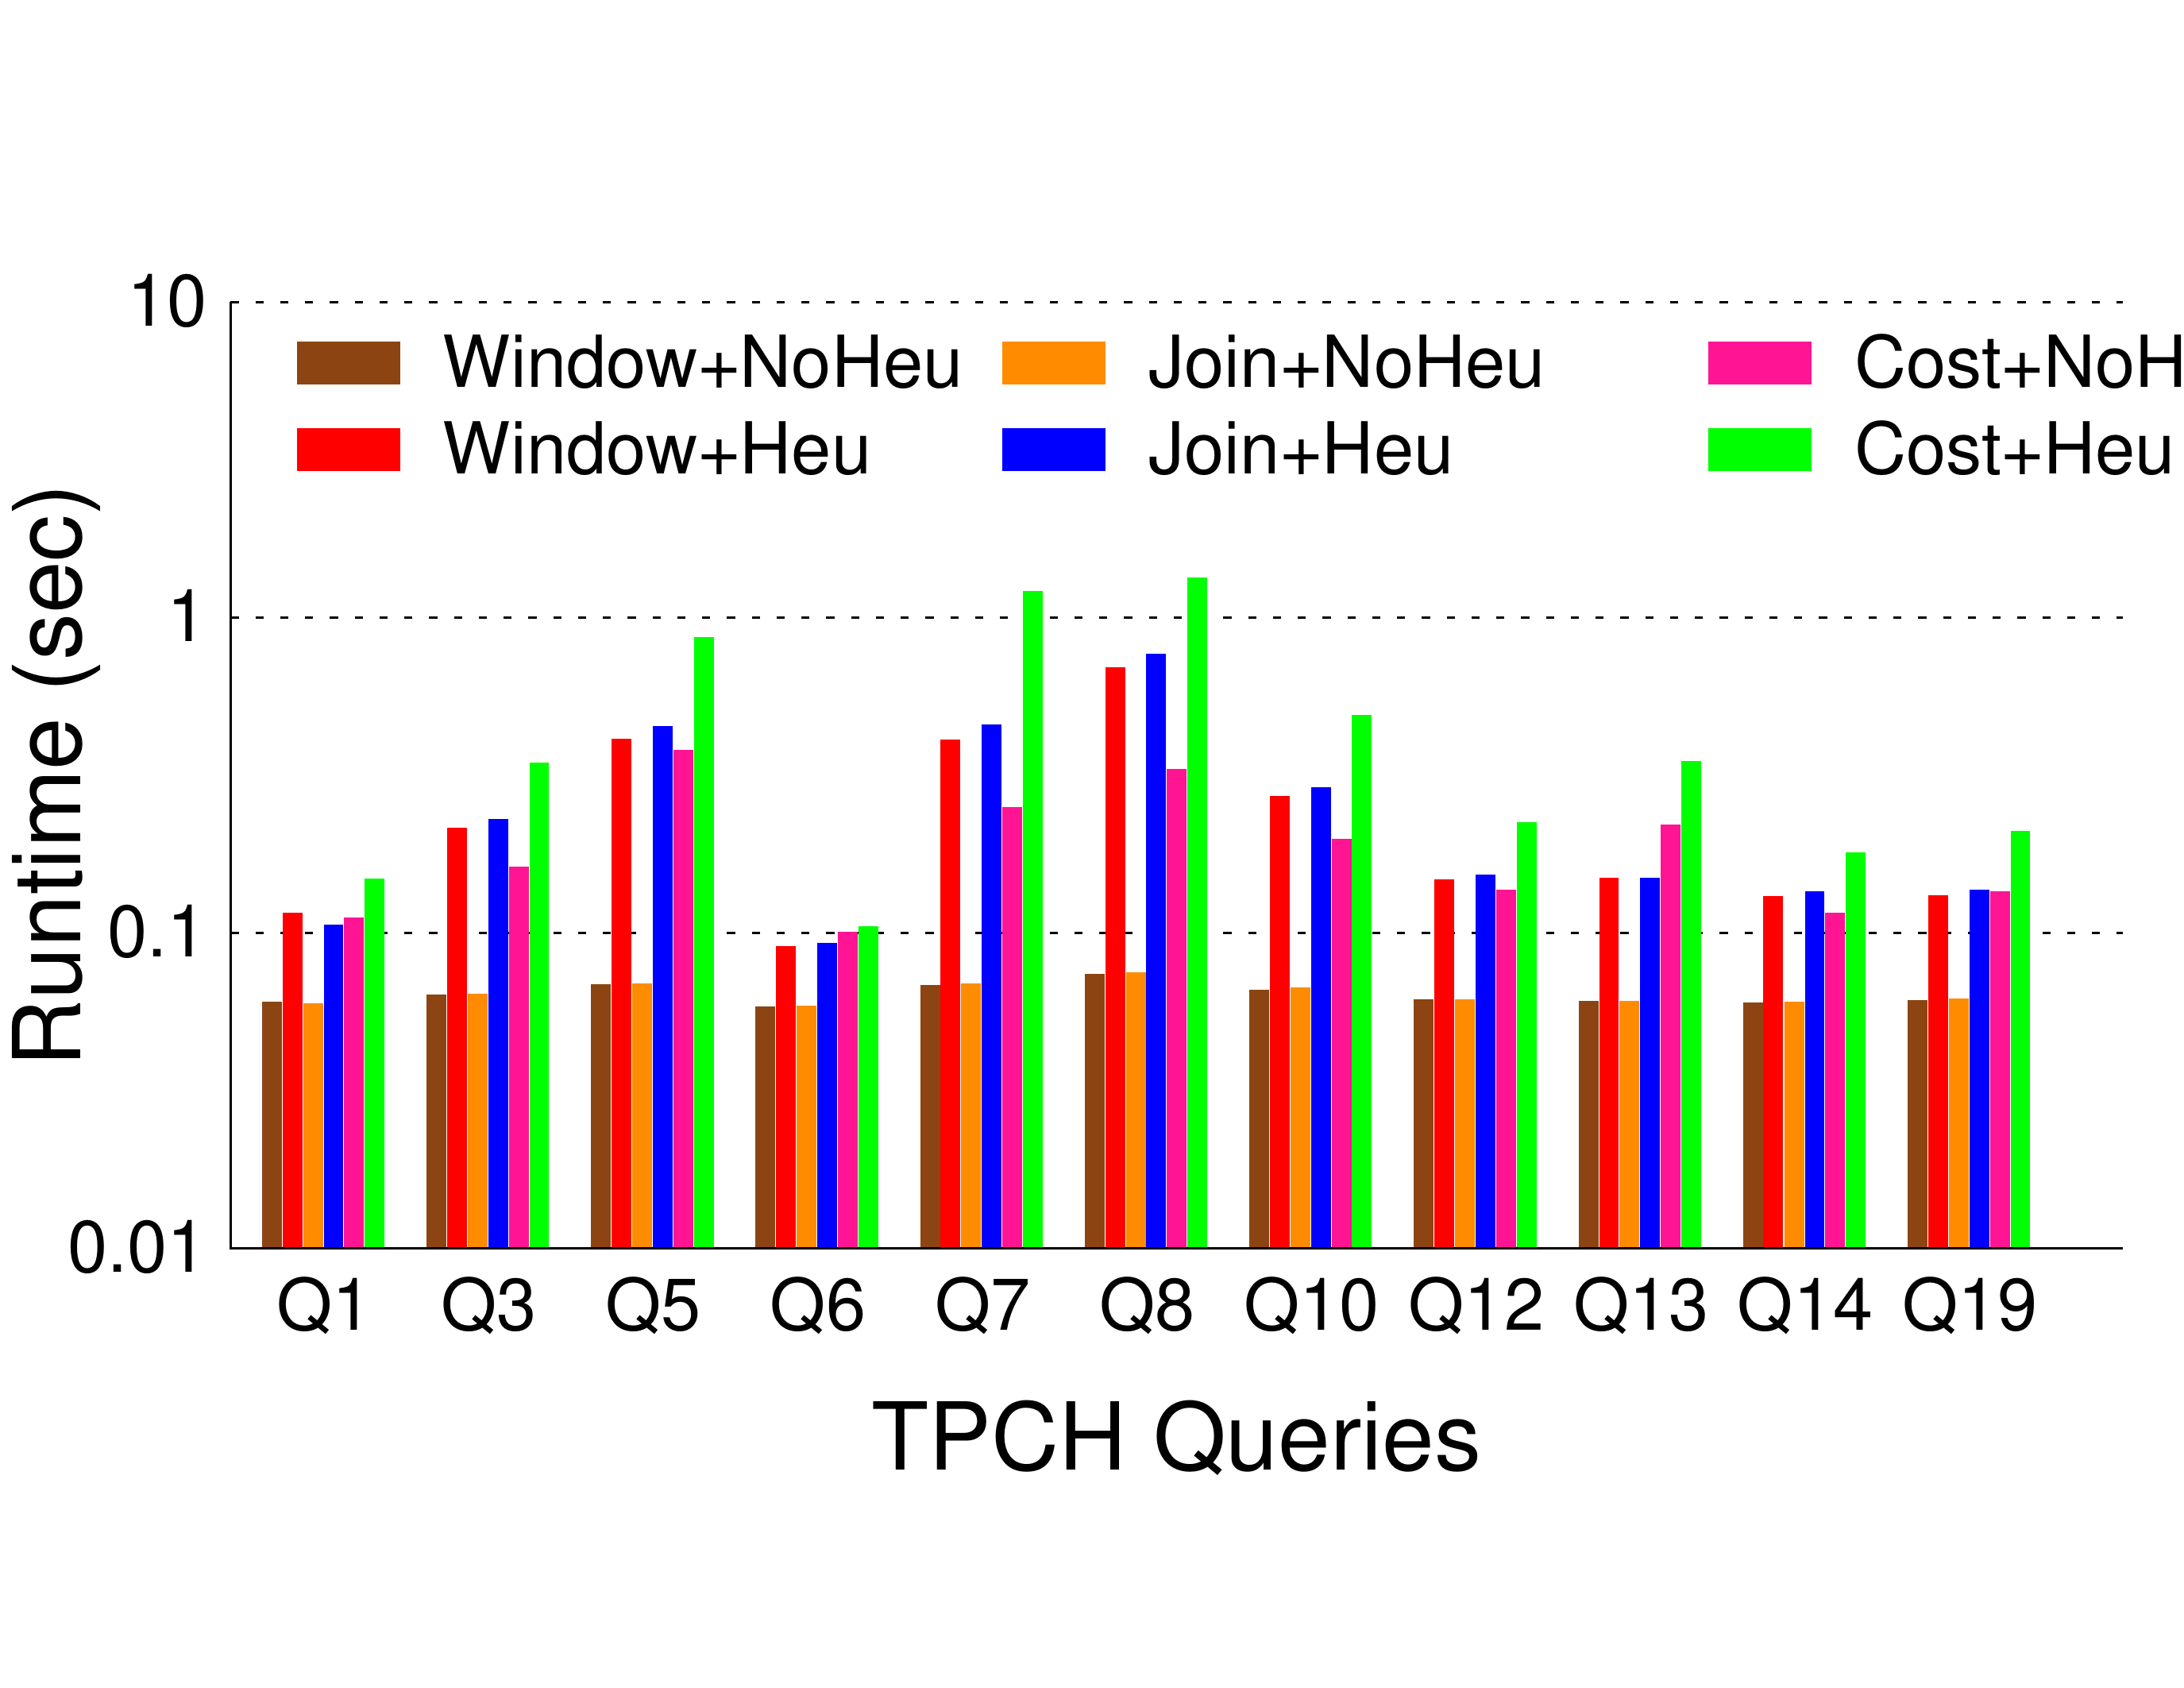}\\[-7mm] 
  \caption{TPC-H Overhead}
  \label{fig:tpch-overhead}
  \end{minipage}
\end{figure*}
% %%%%%%%%%%%%%%%%%%%%%%%%%%%%%%%%%%%%%%%%%%%%%%%%%%%%%%%%%%%%

%%%%%%%%%%%%%%%%%%%%%%%%%%%%%%%%%%%%%%%%%%%%%%%%%%%%%%%%%%%%
%\begin{figure*}[t]
%%%%%%%%%%%%%%%%%%%%
 % \begin{minipage}[b]{0.49\linewidth}
  %\includegraphics[width=1\linewidth,trim=0 80pt 0 100pt, clip]{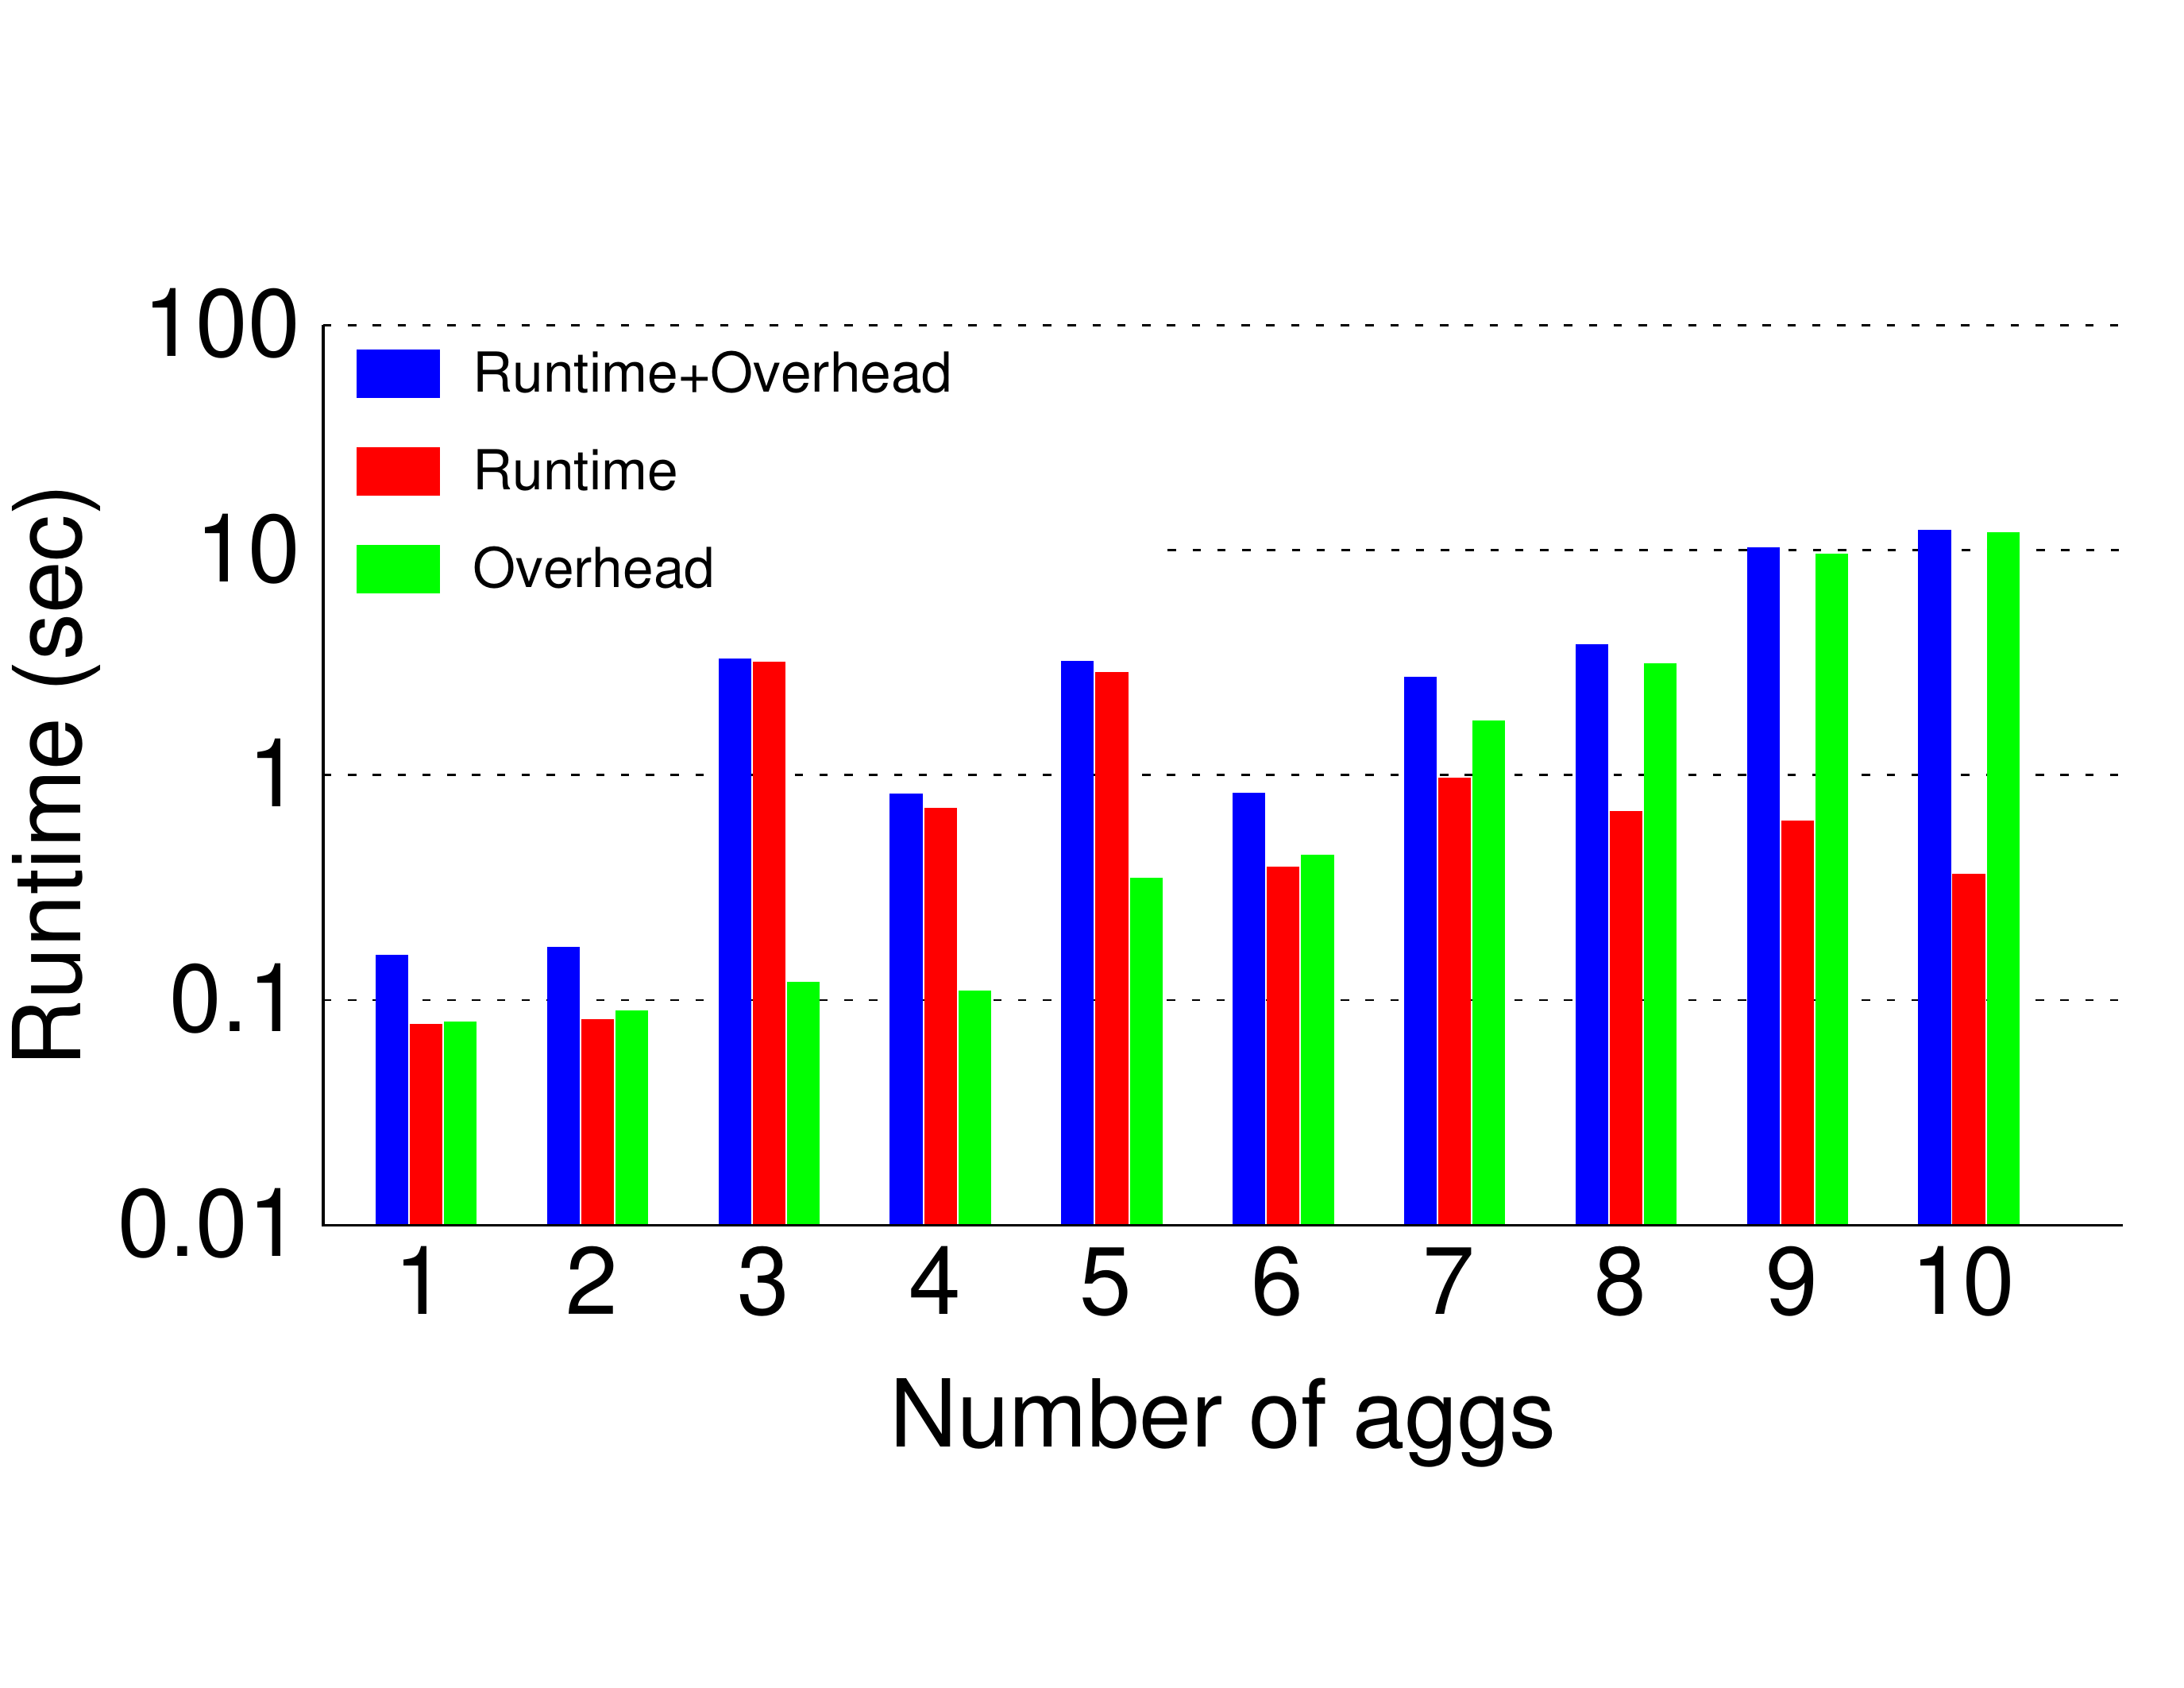}\\[-7mm]
  %\caption{Exhaustive Simple Agg.  Runtime + Overhead - 1GB}
  %\label{fig:exh-simple-agg-runtime-overhead}  
  %\end{minipage}
%%%%%%%%%%%%%%%%%%%
  %\begin{minipage}[b]{0.49\linewidth}
  %\includegraphics[width=1\linewidth,trim=0 80pt 0 100pt, clip]{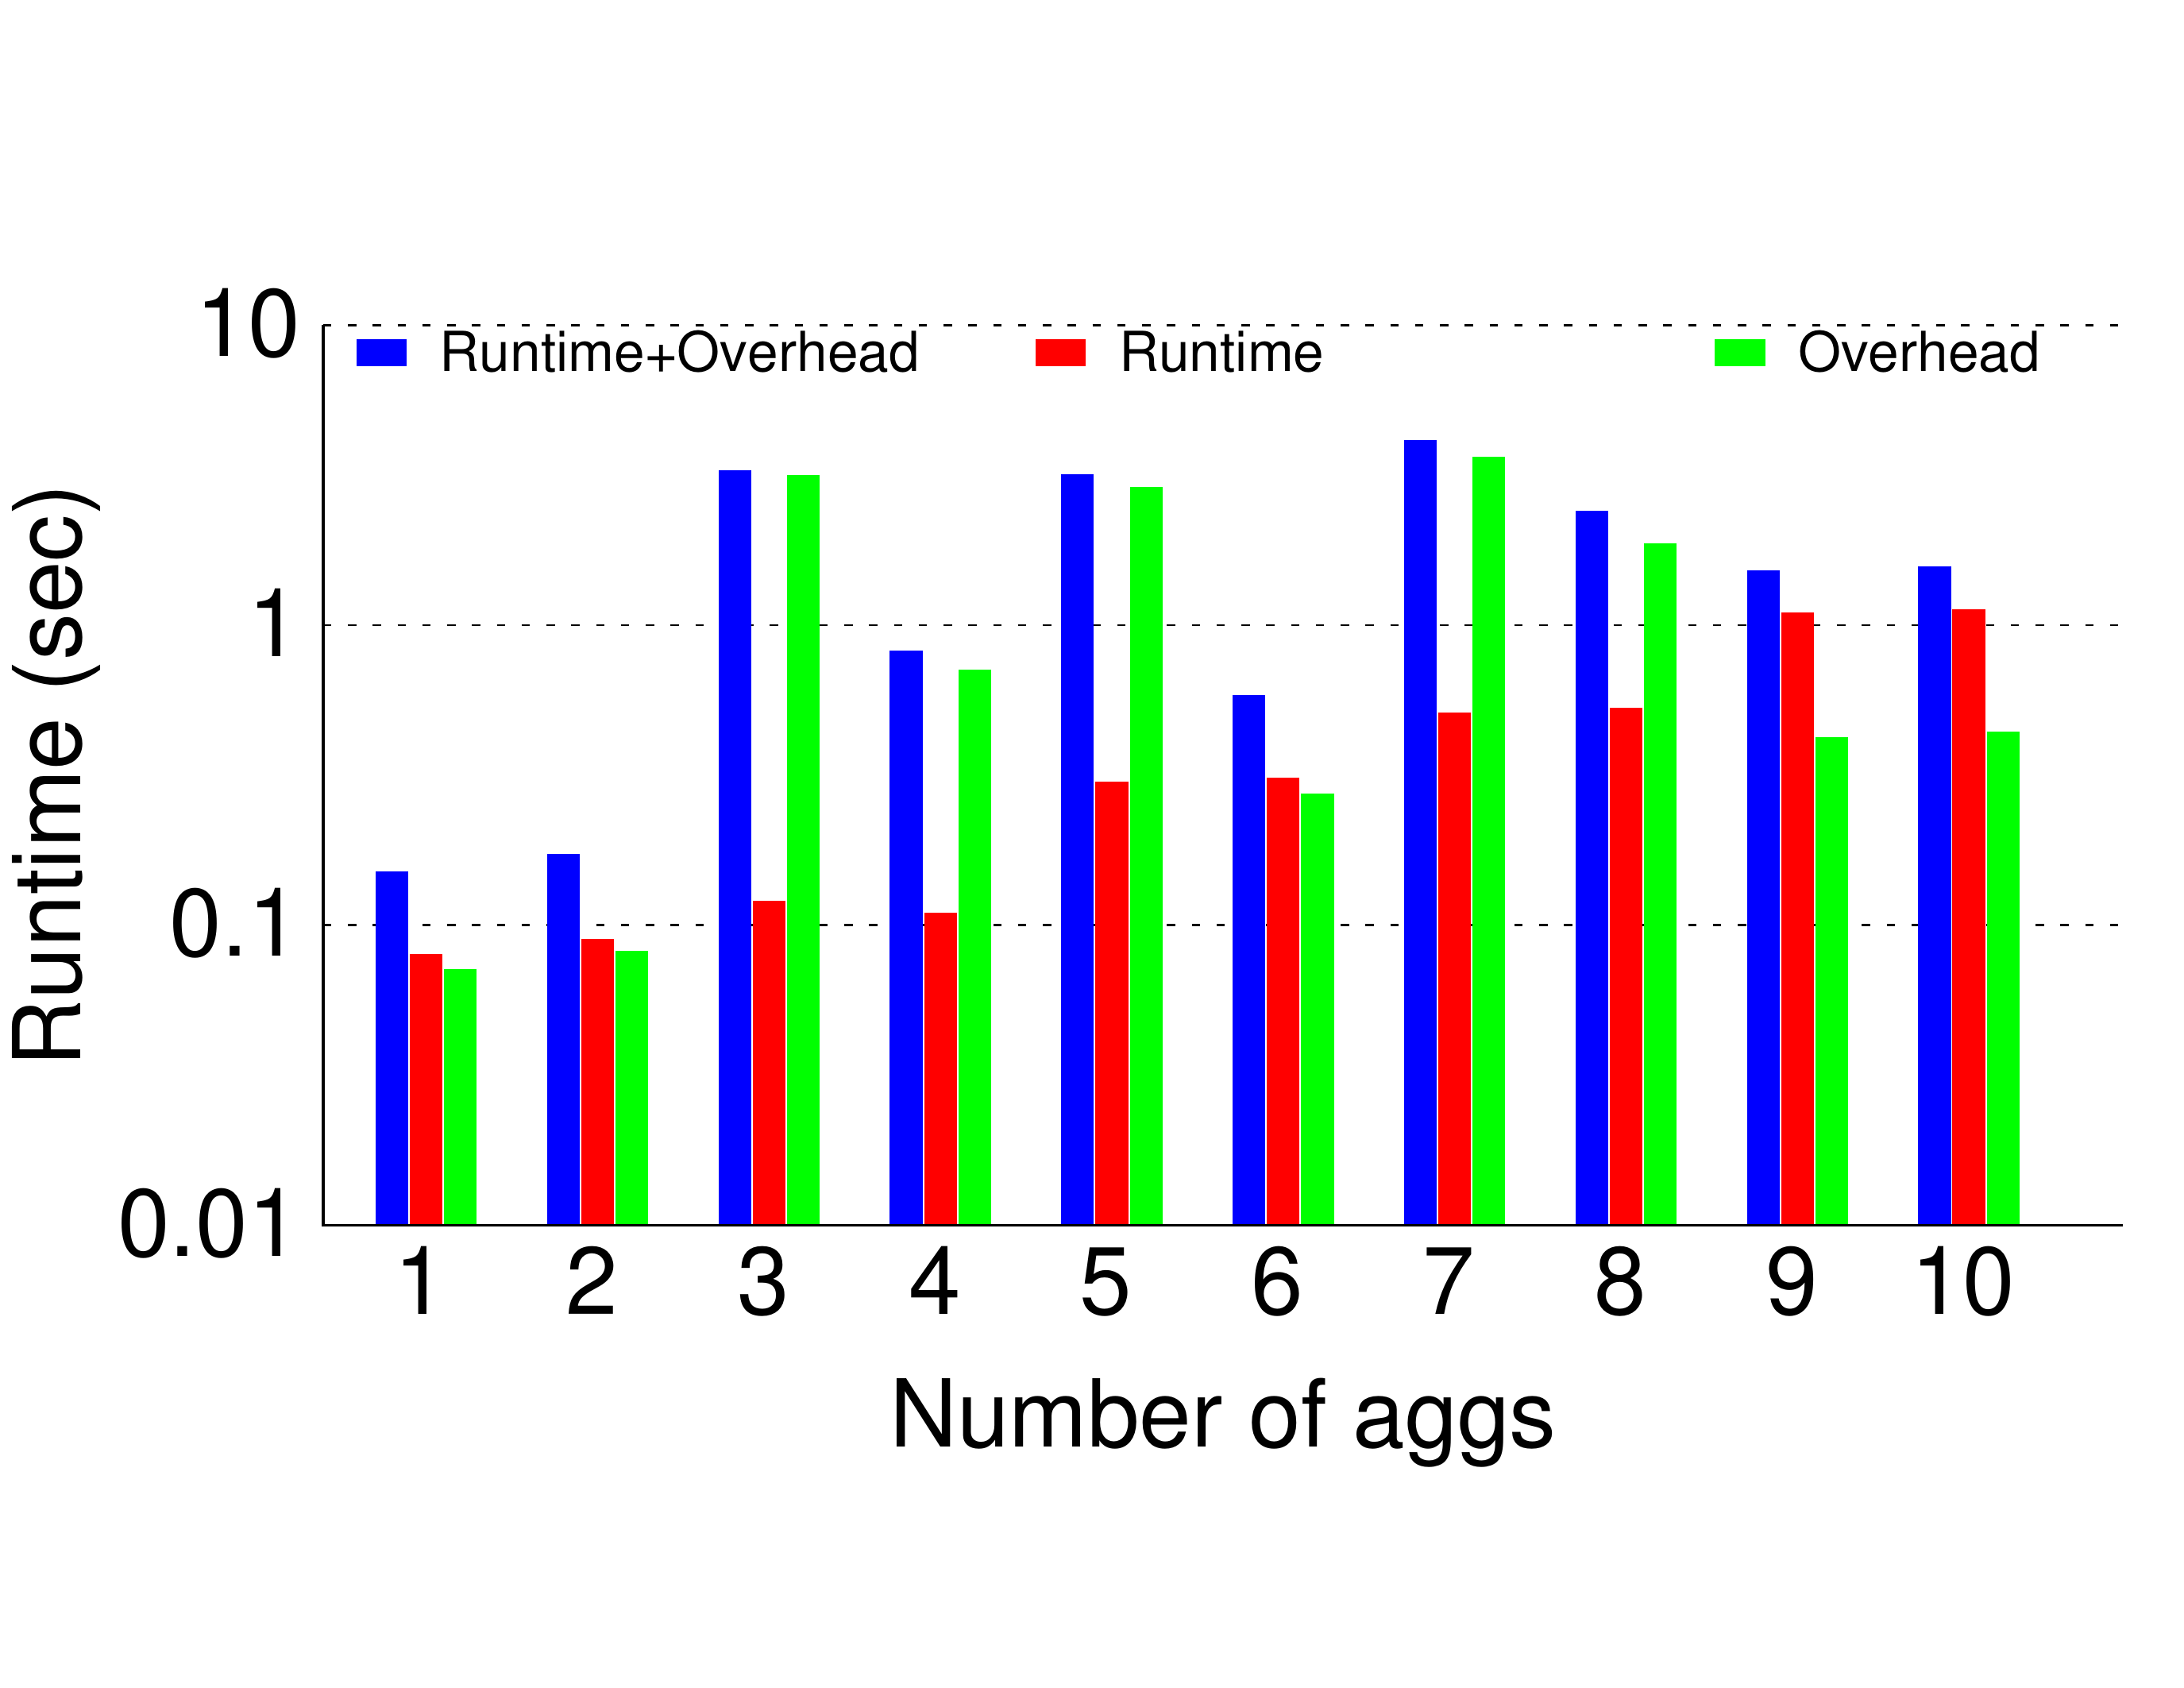}\\[-7mm] 
  %\caption{Balance Simple Agg.  Runtime + Overhead - 1GB}
  %\label{fig:bal-simple-agg-runtime-overhead}
  %\end{minipage}
%\end{figure*}
% %%%%%%%%%%%%%%%%%%%%%%%%%%%%%%%%%%%%%%%%%%%%%%%%%%%%%%%%%%%%

%%%%%%%%%%%%%%%%%%%%%%%%%%%%%%%%%%%%%%%%%%%%%%%%%%%%%%%%%%%%
\begin{figure*}[t]
%%%%%%%%%%%%%%%%%%%%
  \begin{minipage}[b]{0.49\linewidth}
  \includegraphics[width=1\linewidth,trim=0 80pt 0 100pt, clip]{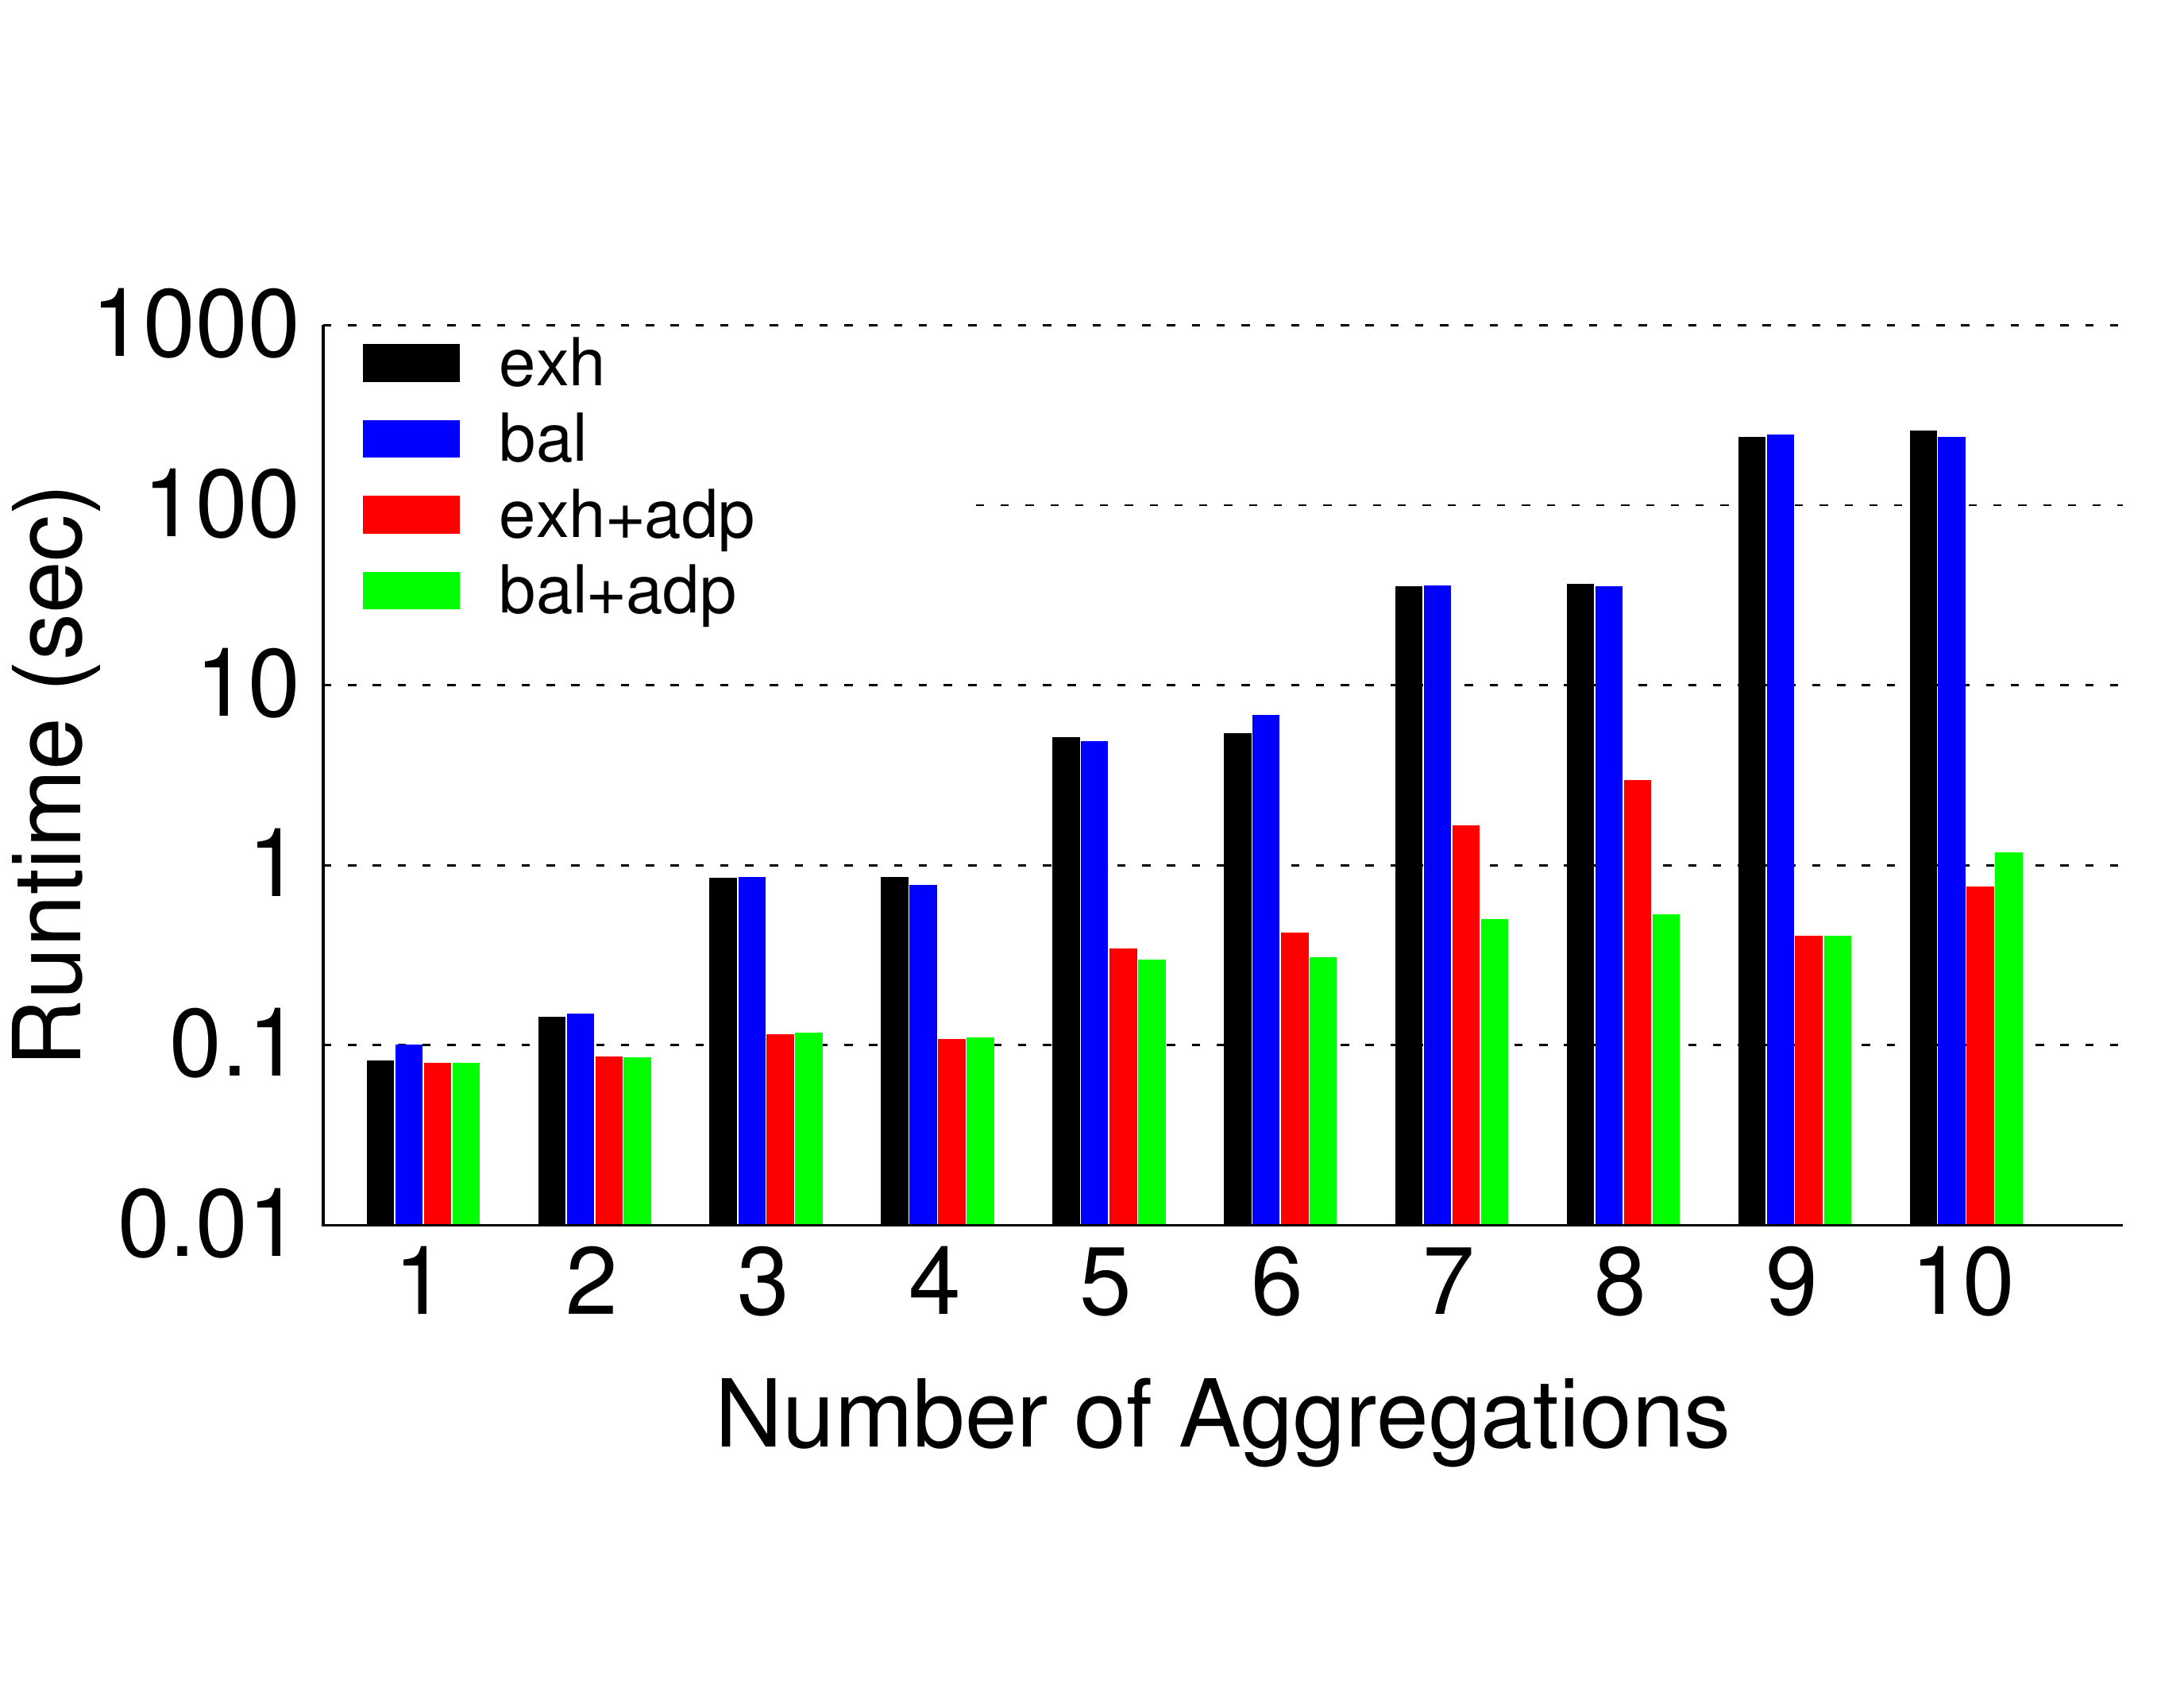}\\[-7mm]
  \caption{Exhaustive Simple Agg. Overhead - 1GB}
  \label{fig:exh-simple-agg-overhead-sty}  
  \end{minipage}
%%%%%%%%%%%%%%%%%%%
  \begin{minipage}[b]{0.49\linewidth}
  \includegraphics[width=1\linewidth,trim=0 80pt 0 100pt, clip]{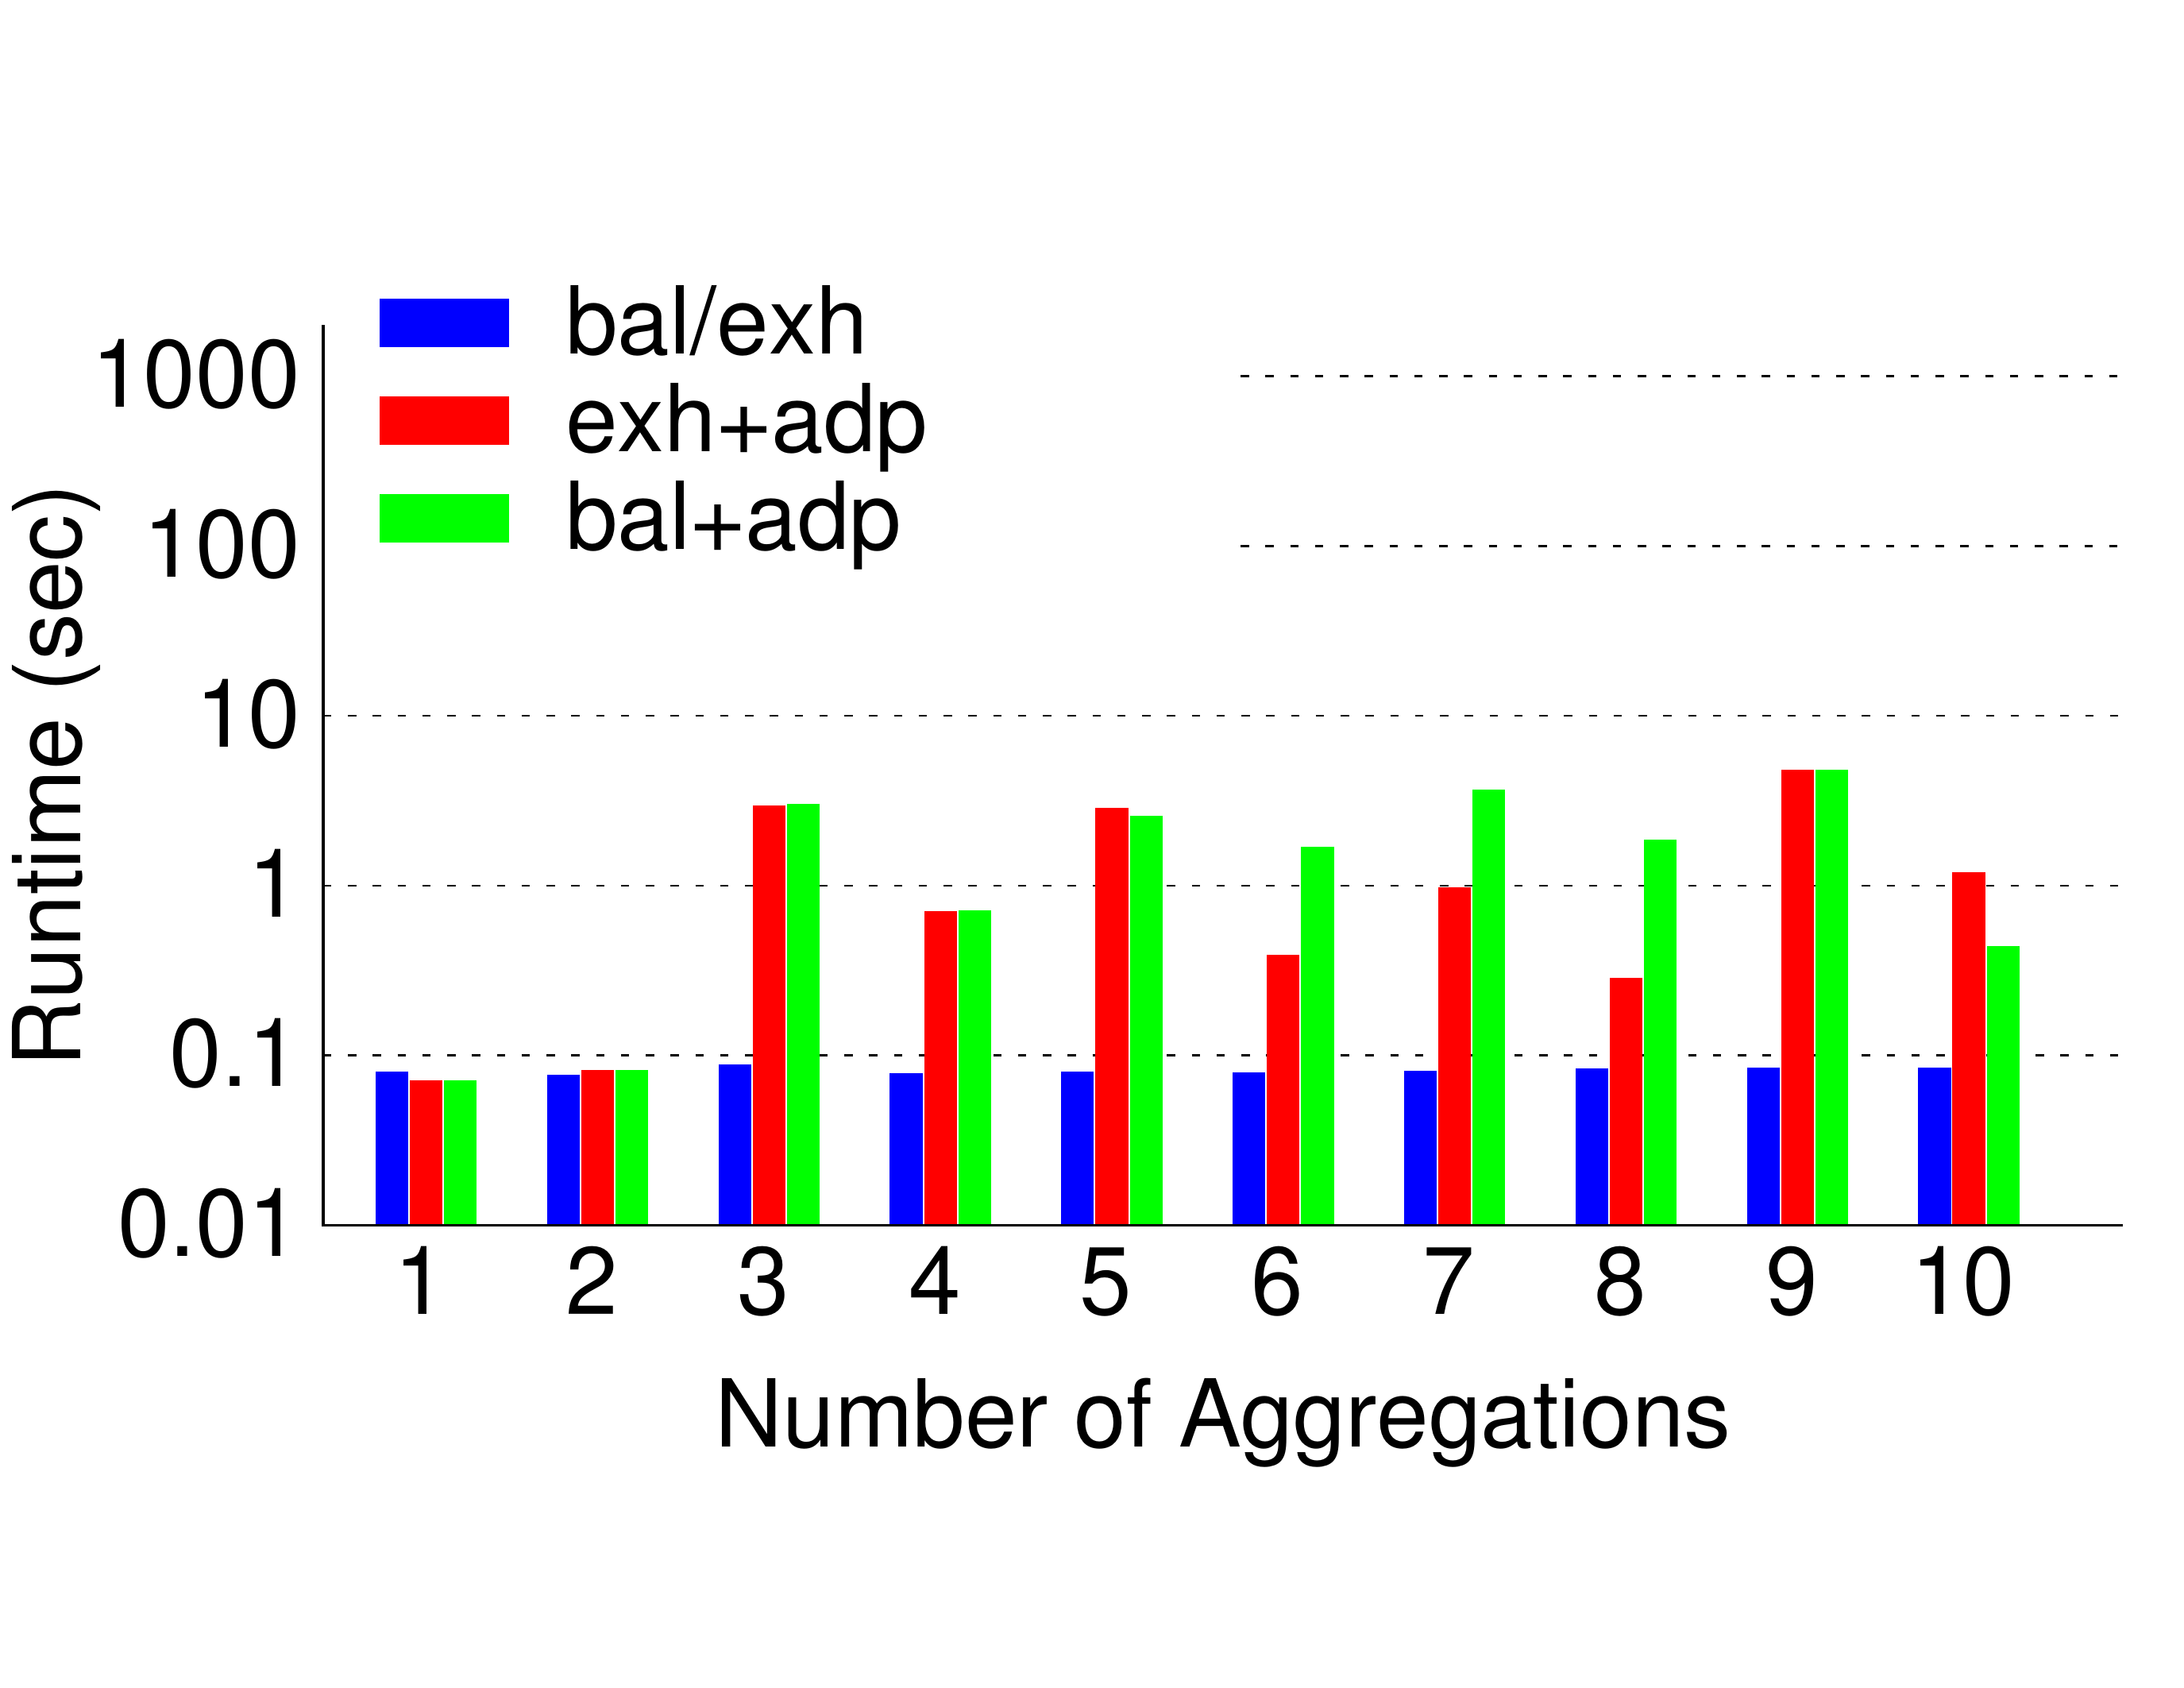}\\[-7mm] 
  \caption{Simple Agg. Runtime - 1GB}
  \label{fig:bal-simple-agg-runtime-sty}
  \end{minipage}
\end{figure*}
% %%%%%%%%%%%%%%%%%%%%%%%%%%%%%%%%%%%%%%%%%%%%%%%%%%%%%%%%%%%%

%%%%%%%%%%%%%%%%%%%%%%%%%%%%%%%%%%%%%%%%%%%%%%%%%%%%%%%%%%%%
\begin{figure*}[t]
%%%%%%%%%%%%%%%%%%%%
  \begin{minipage}[b]{0.49\linewidth}
  \includegraphics[width=1\linewidth,trim=0 80pt 0 100pt, clip]{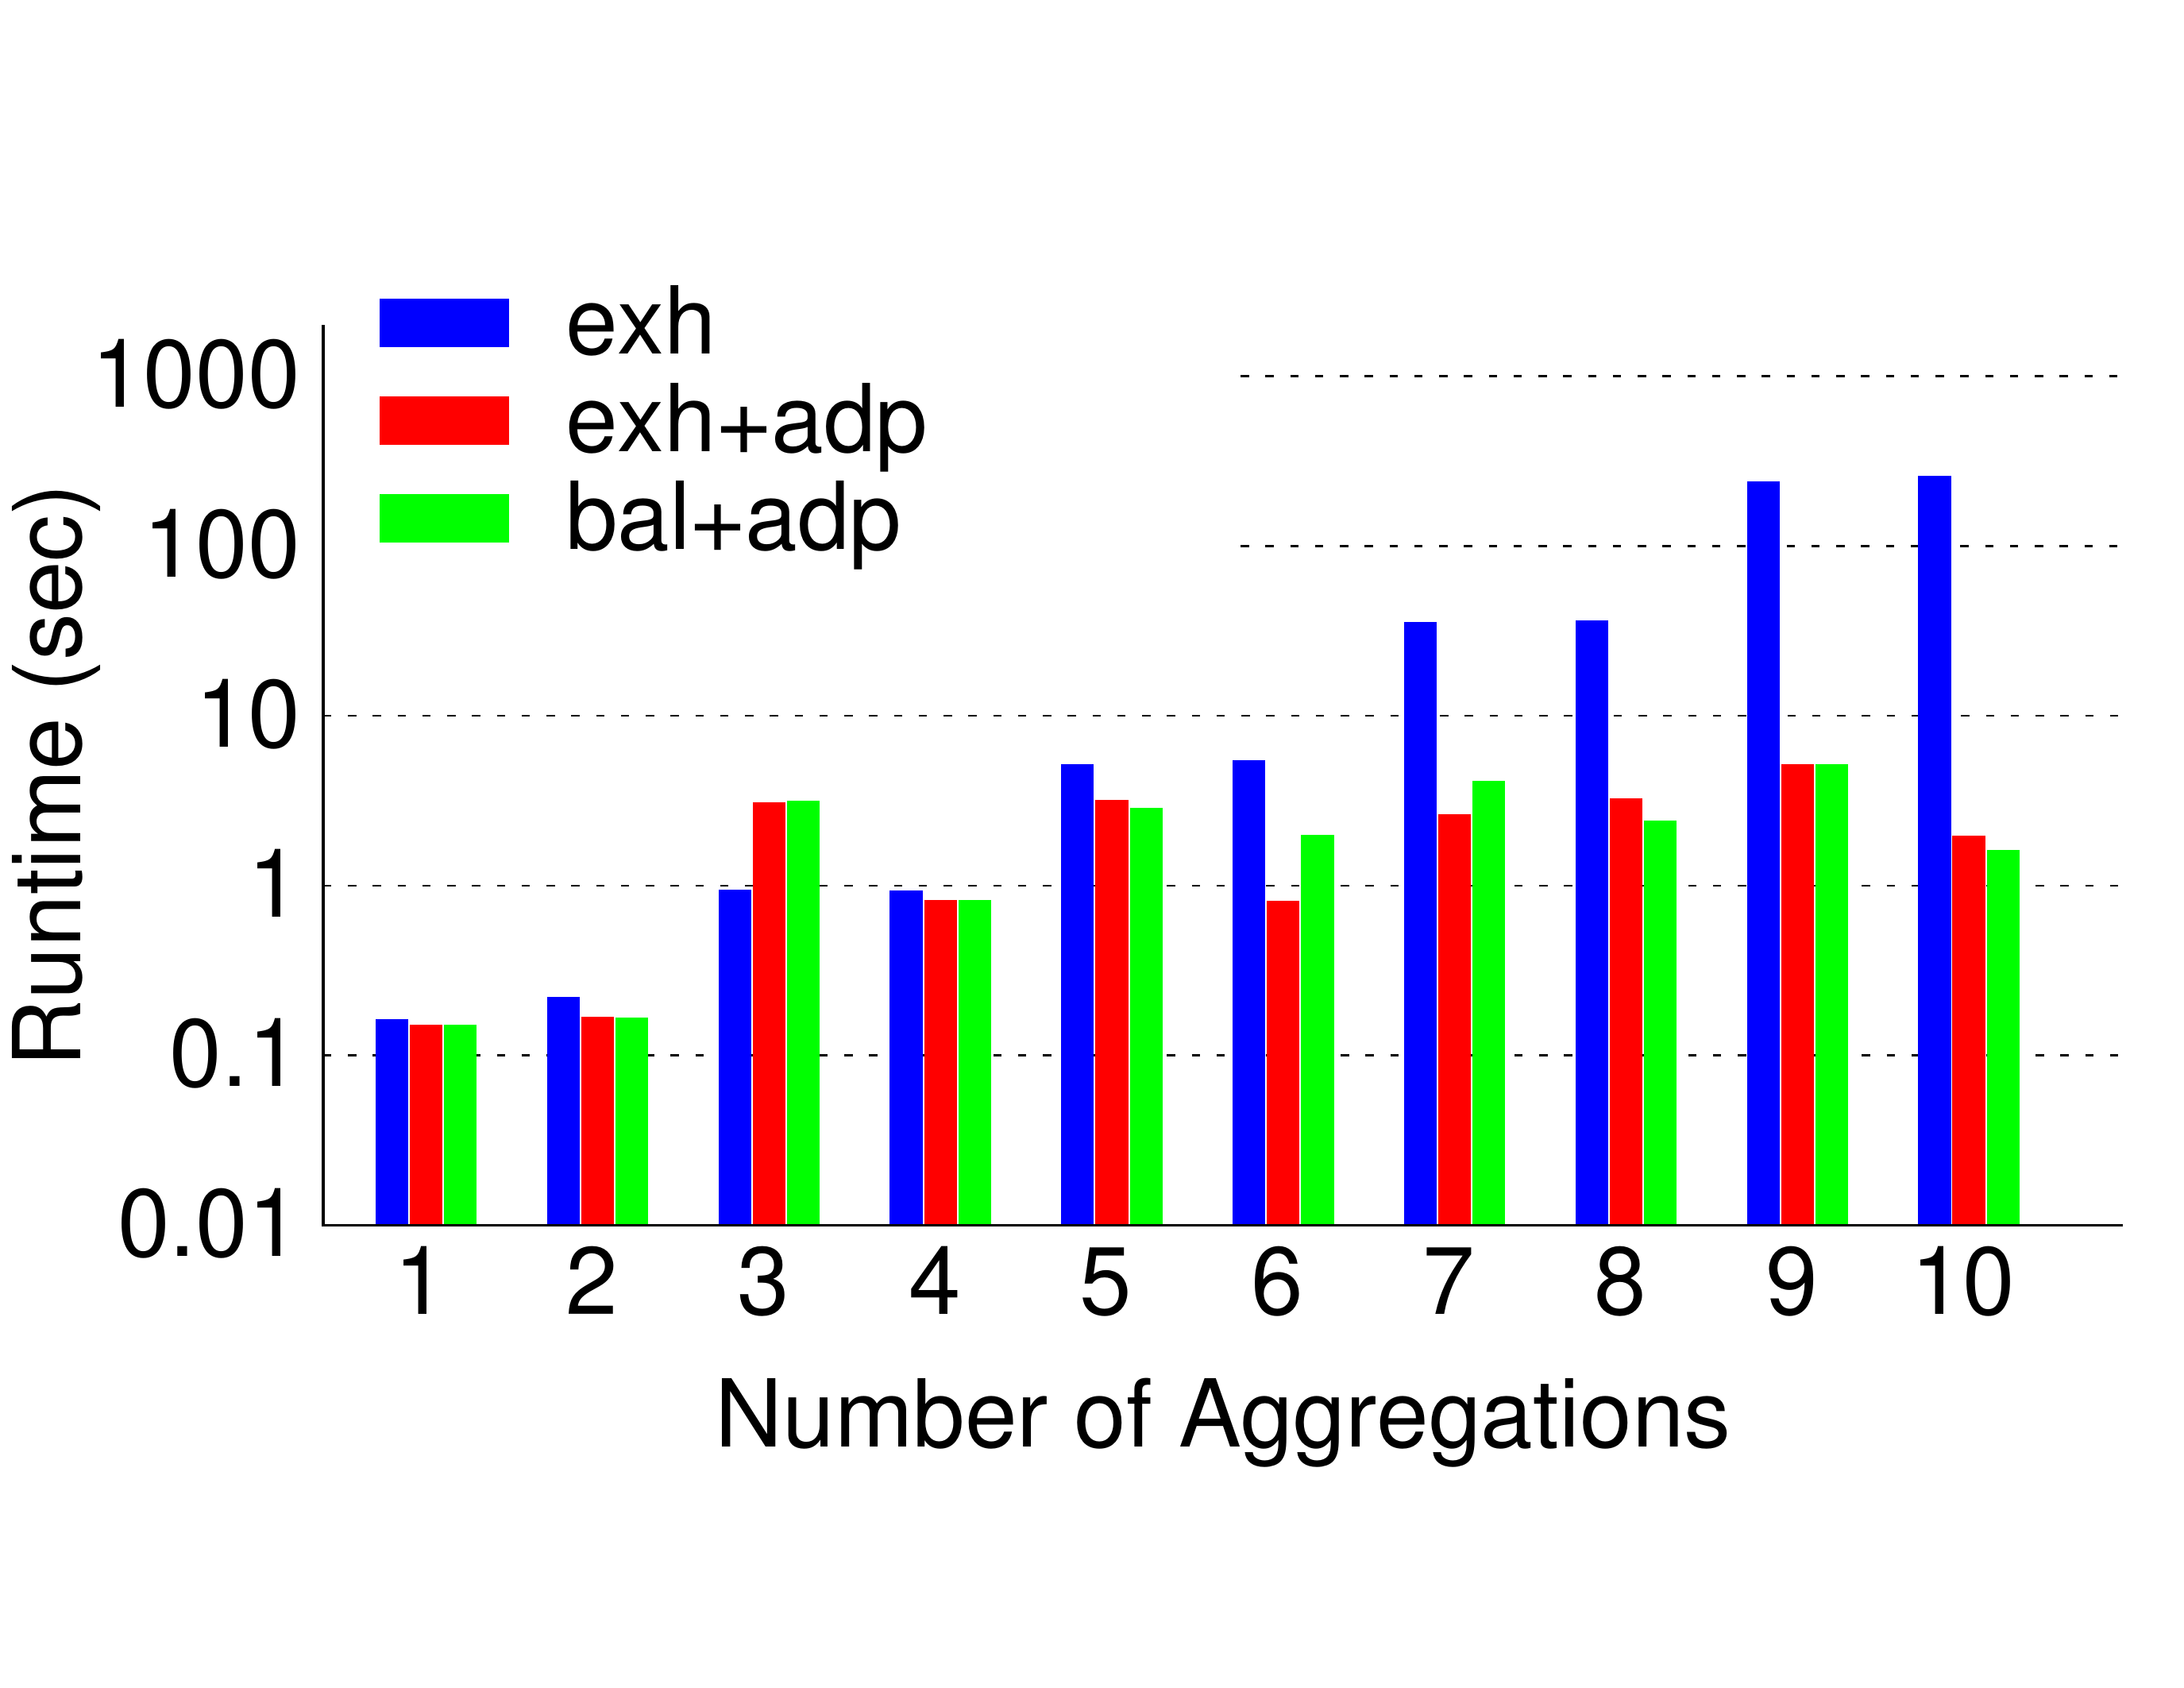}\\[-7mm]
  \caption{Simple Agg.  Runtime + Overhead - 1GB}
  \label{fig:simple-agg-runtime-overhead-sty}  
  \end{minipage}
%%%%%%%%%%%%%%%%%%%
  \begin{minipage}[b]{0.49\linewidth}
  \includegraphics[width=1\linewidth,trim=0 80pt 0 100pt, clip]{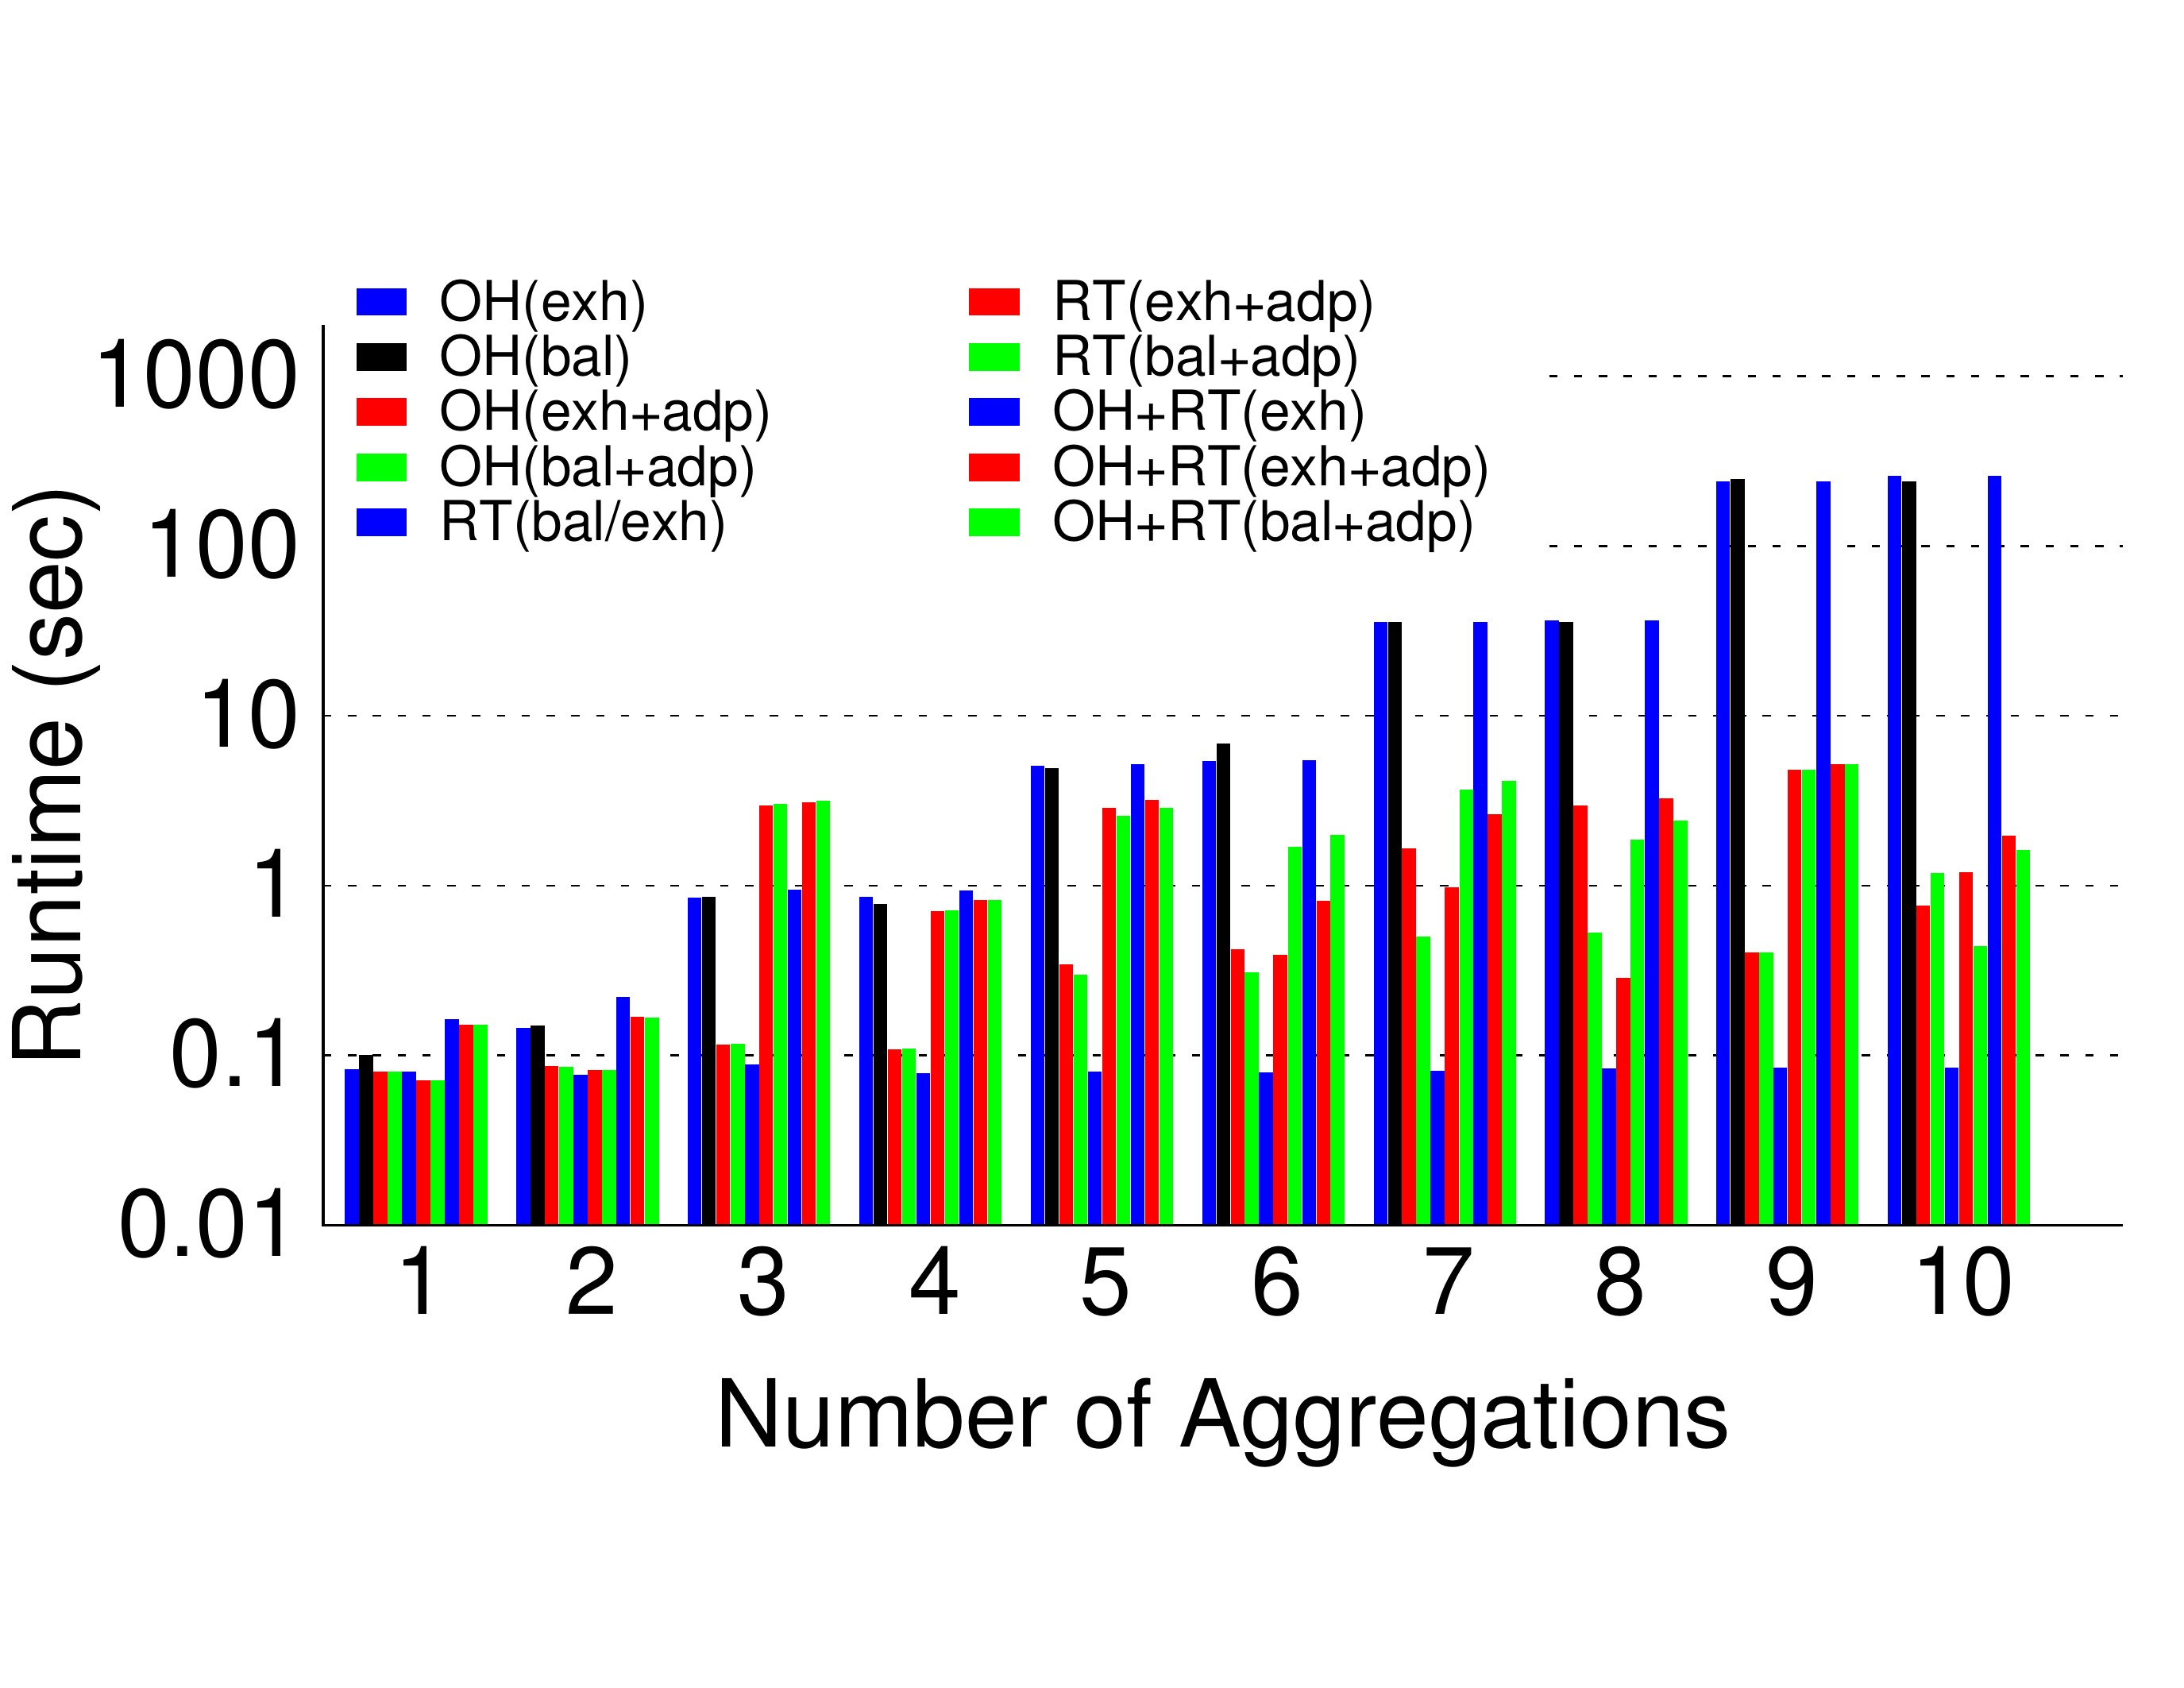}\\[-7mm] 
  \caption{Simple Agg.  All - 1GB}
  \label{fig:simple-agg-all-sty}
  \end{minipage}
\end{figure*}
% %%%%%%%%%%%%%%%%%%%%%%%%%%%%%%%%%%%%%%%%%%%%%%%%%%%%%%%%%%%%

%%%%%%%%%%%%%%%%%%%%%%%%%%%%%%%%%%%%%%%%%%%%%%%%%%%%%%%%%%%%
\begin{figure*}[t]
%%%%%%%%%%%%%%%%%%%%
  \begin{minipage}[b]{0.49\linewidth}
  \includegraphics[width=1\linewidth,trim=0 80pt 0 100pt, clip]{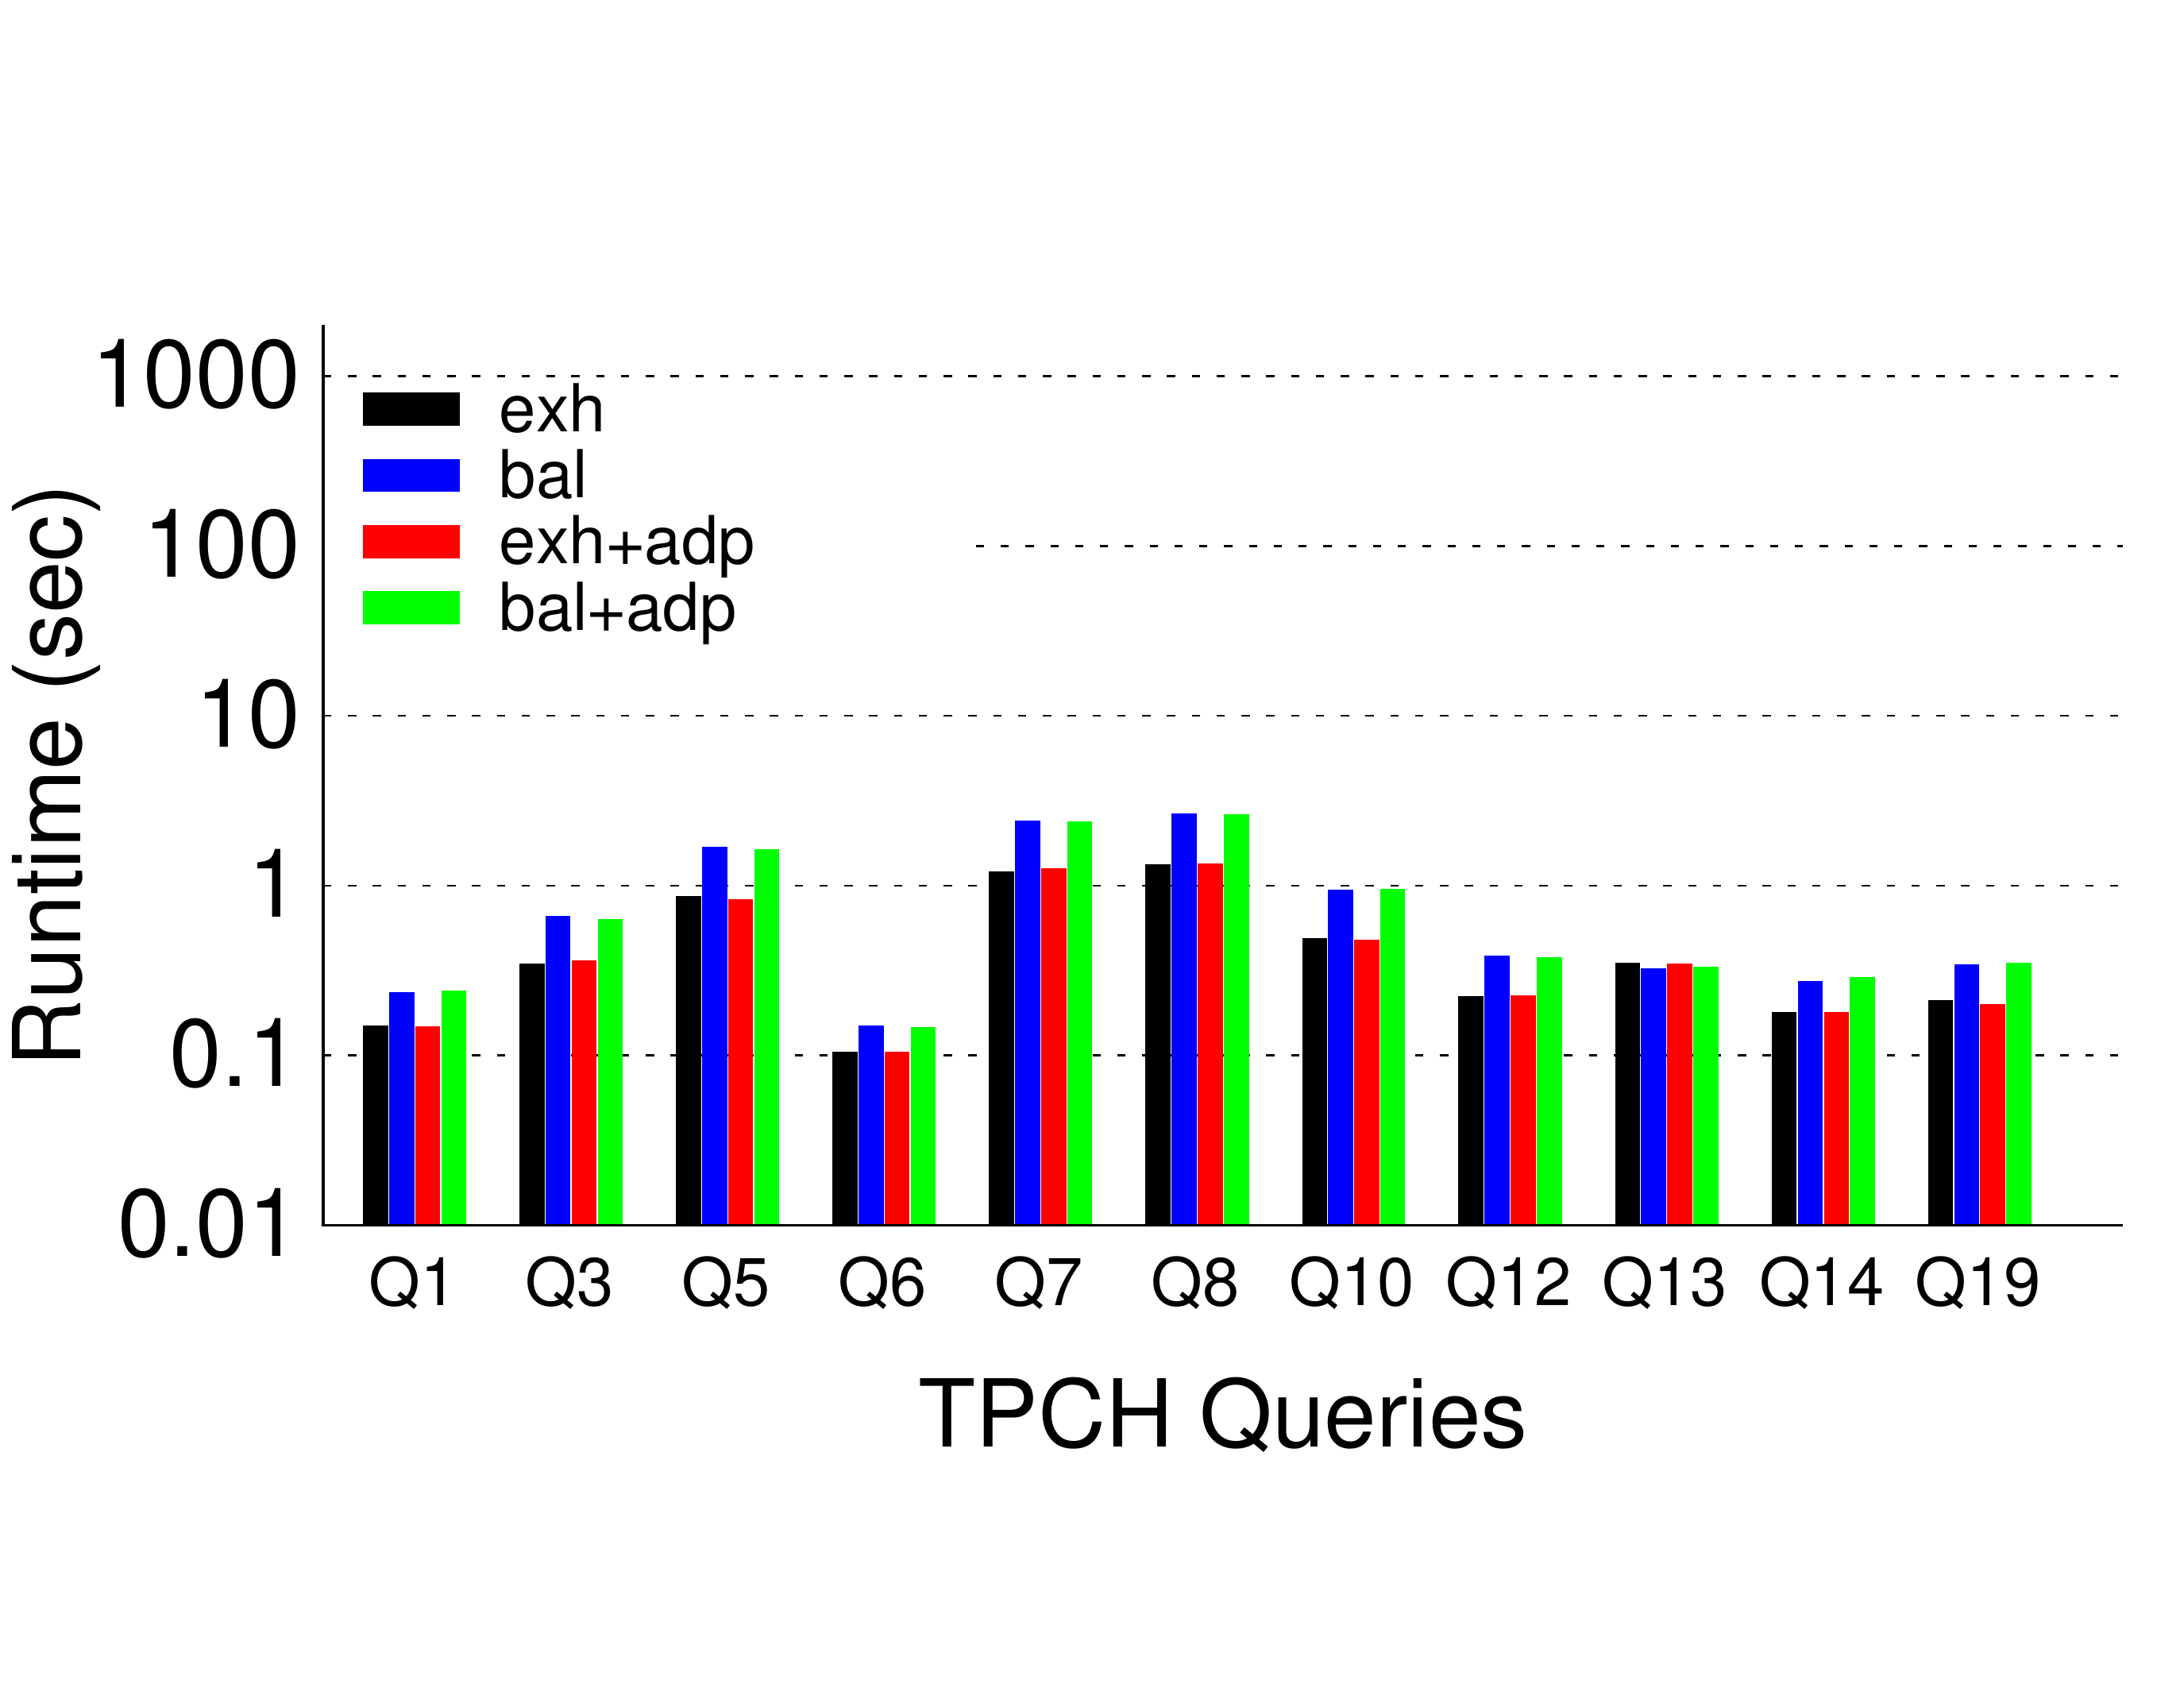}\\[-7mm]
  \caption{Exhaustive TPC-H. Overhead - 1GB}
  \label{fig:tpch-overhead-sty}  
  \end{minipage}
%%%%%%%%%%%%%%%%%%%
  \begin{minipage}[b]{0.49\linewidth}
  \includegraphics[width=1\linewidth,trim=0 80pt 0 100pt, clip]{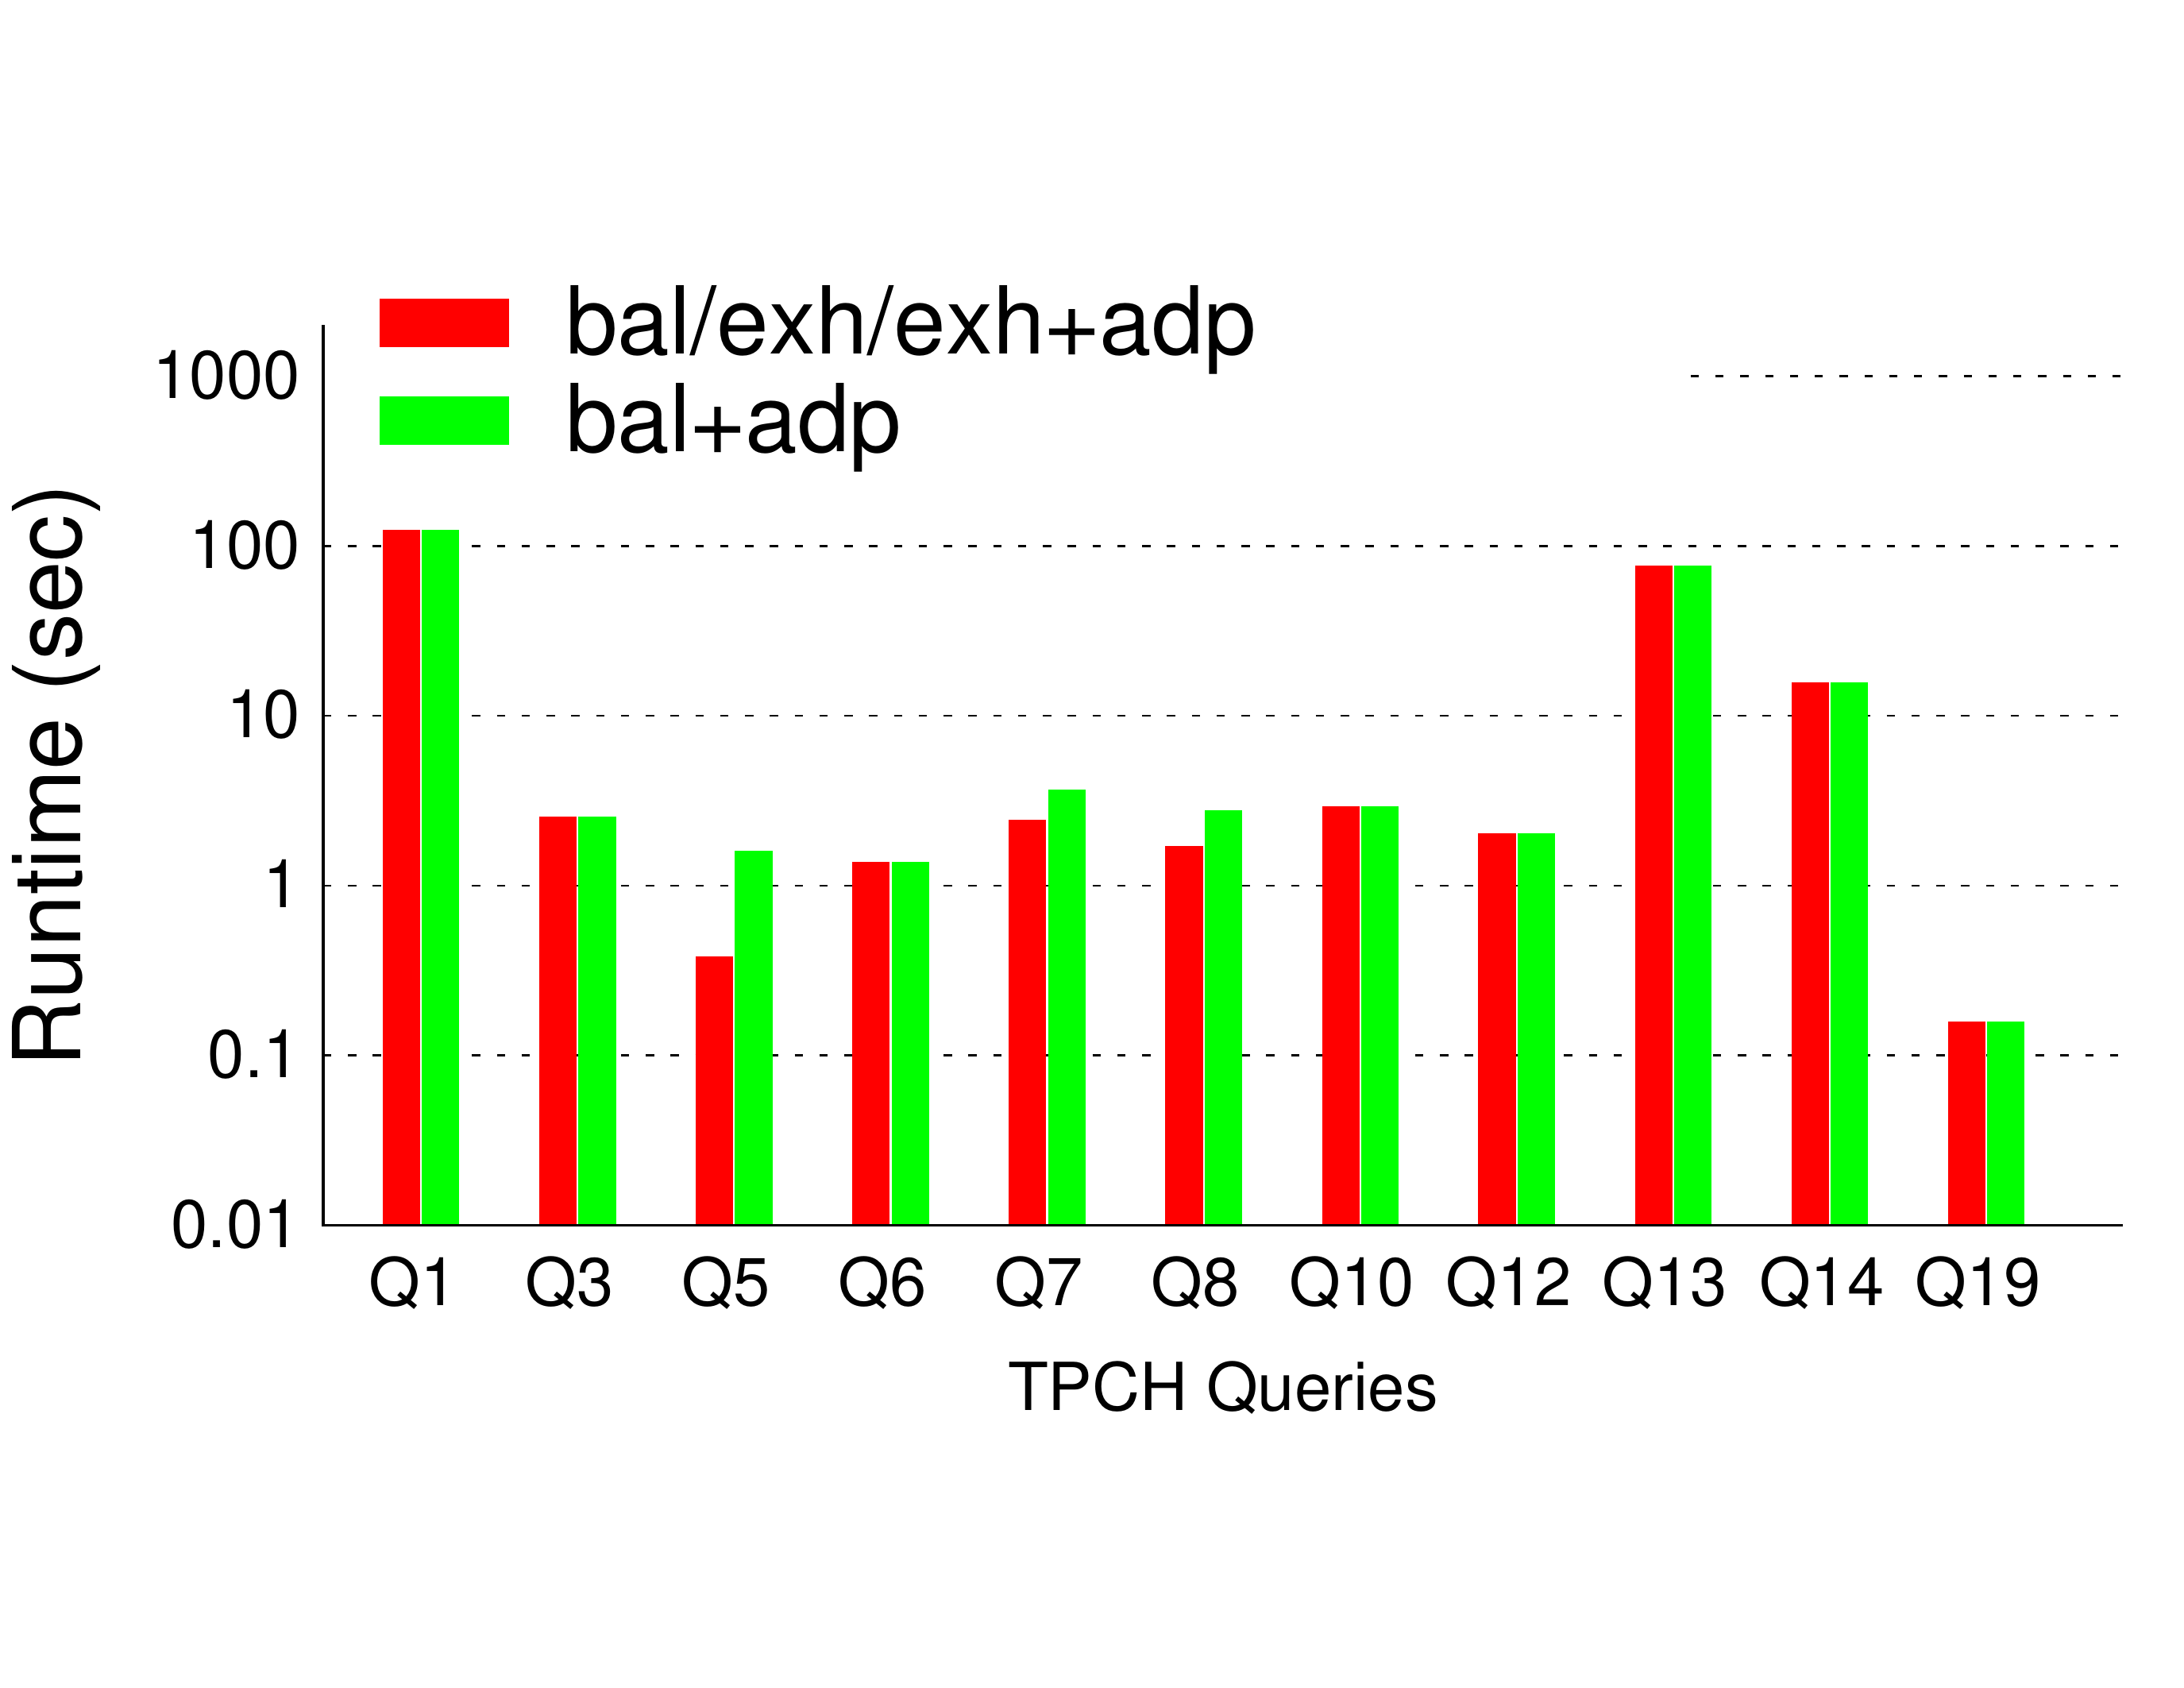}\\[-7mm] 
  \caption{TPC-H. Runtime - 1GB}
  \label{fig:tpch-runtime-sty}
  \end{minipage}
\end{figure*}
% %%%%%%%%%%%%%%%%%%%%%%%%%%%%%%%%%%%%%%%%%%%%%%%%%%%%%%%%%%%%

%%%%%%%%%%%%%%%%%%%%%%%%%%%%%%%%%%%%%%%%%%%%%%%%%%%%%%%%%%%%
\begin{figure*}[t]
%%%%%%%%%%%%%%%%%%%%
  \begin{minipage}[b]{0.49\linewidth}
  \includegraphics[width=1\linewidth,trim=0 80pt 0 100pt, clip]{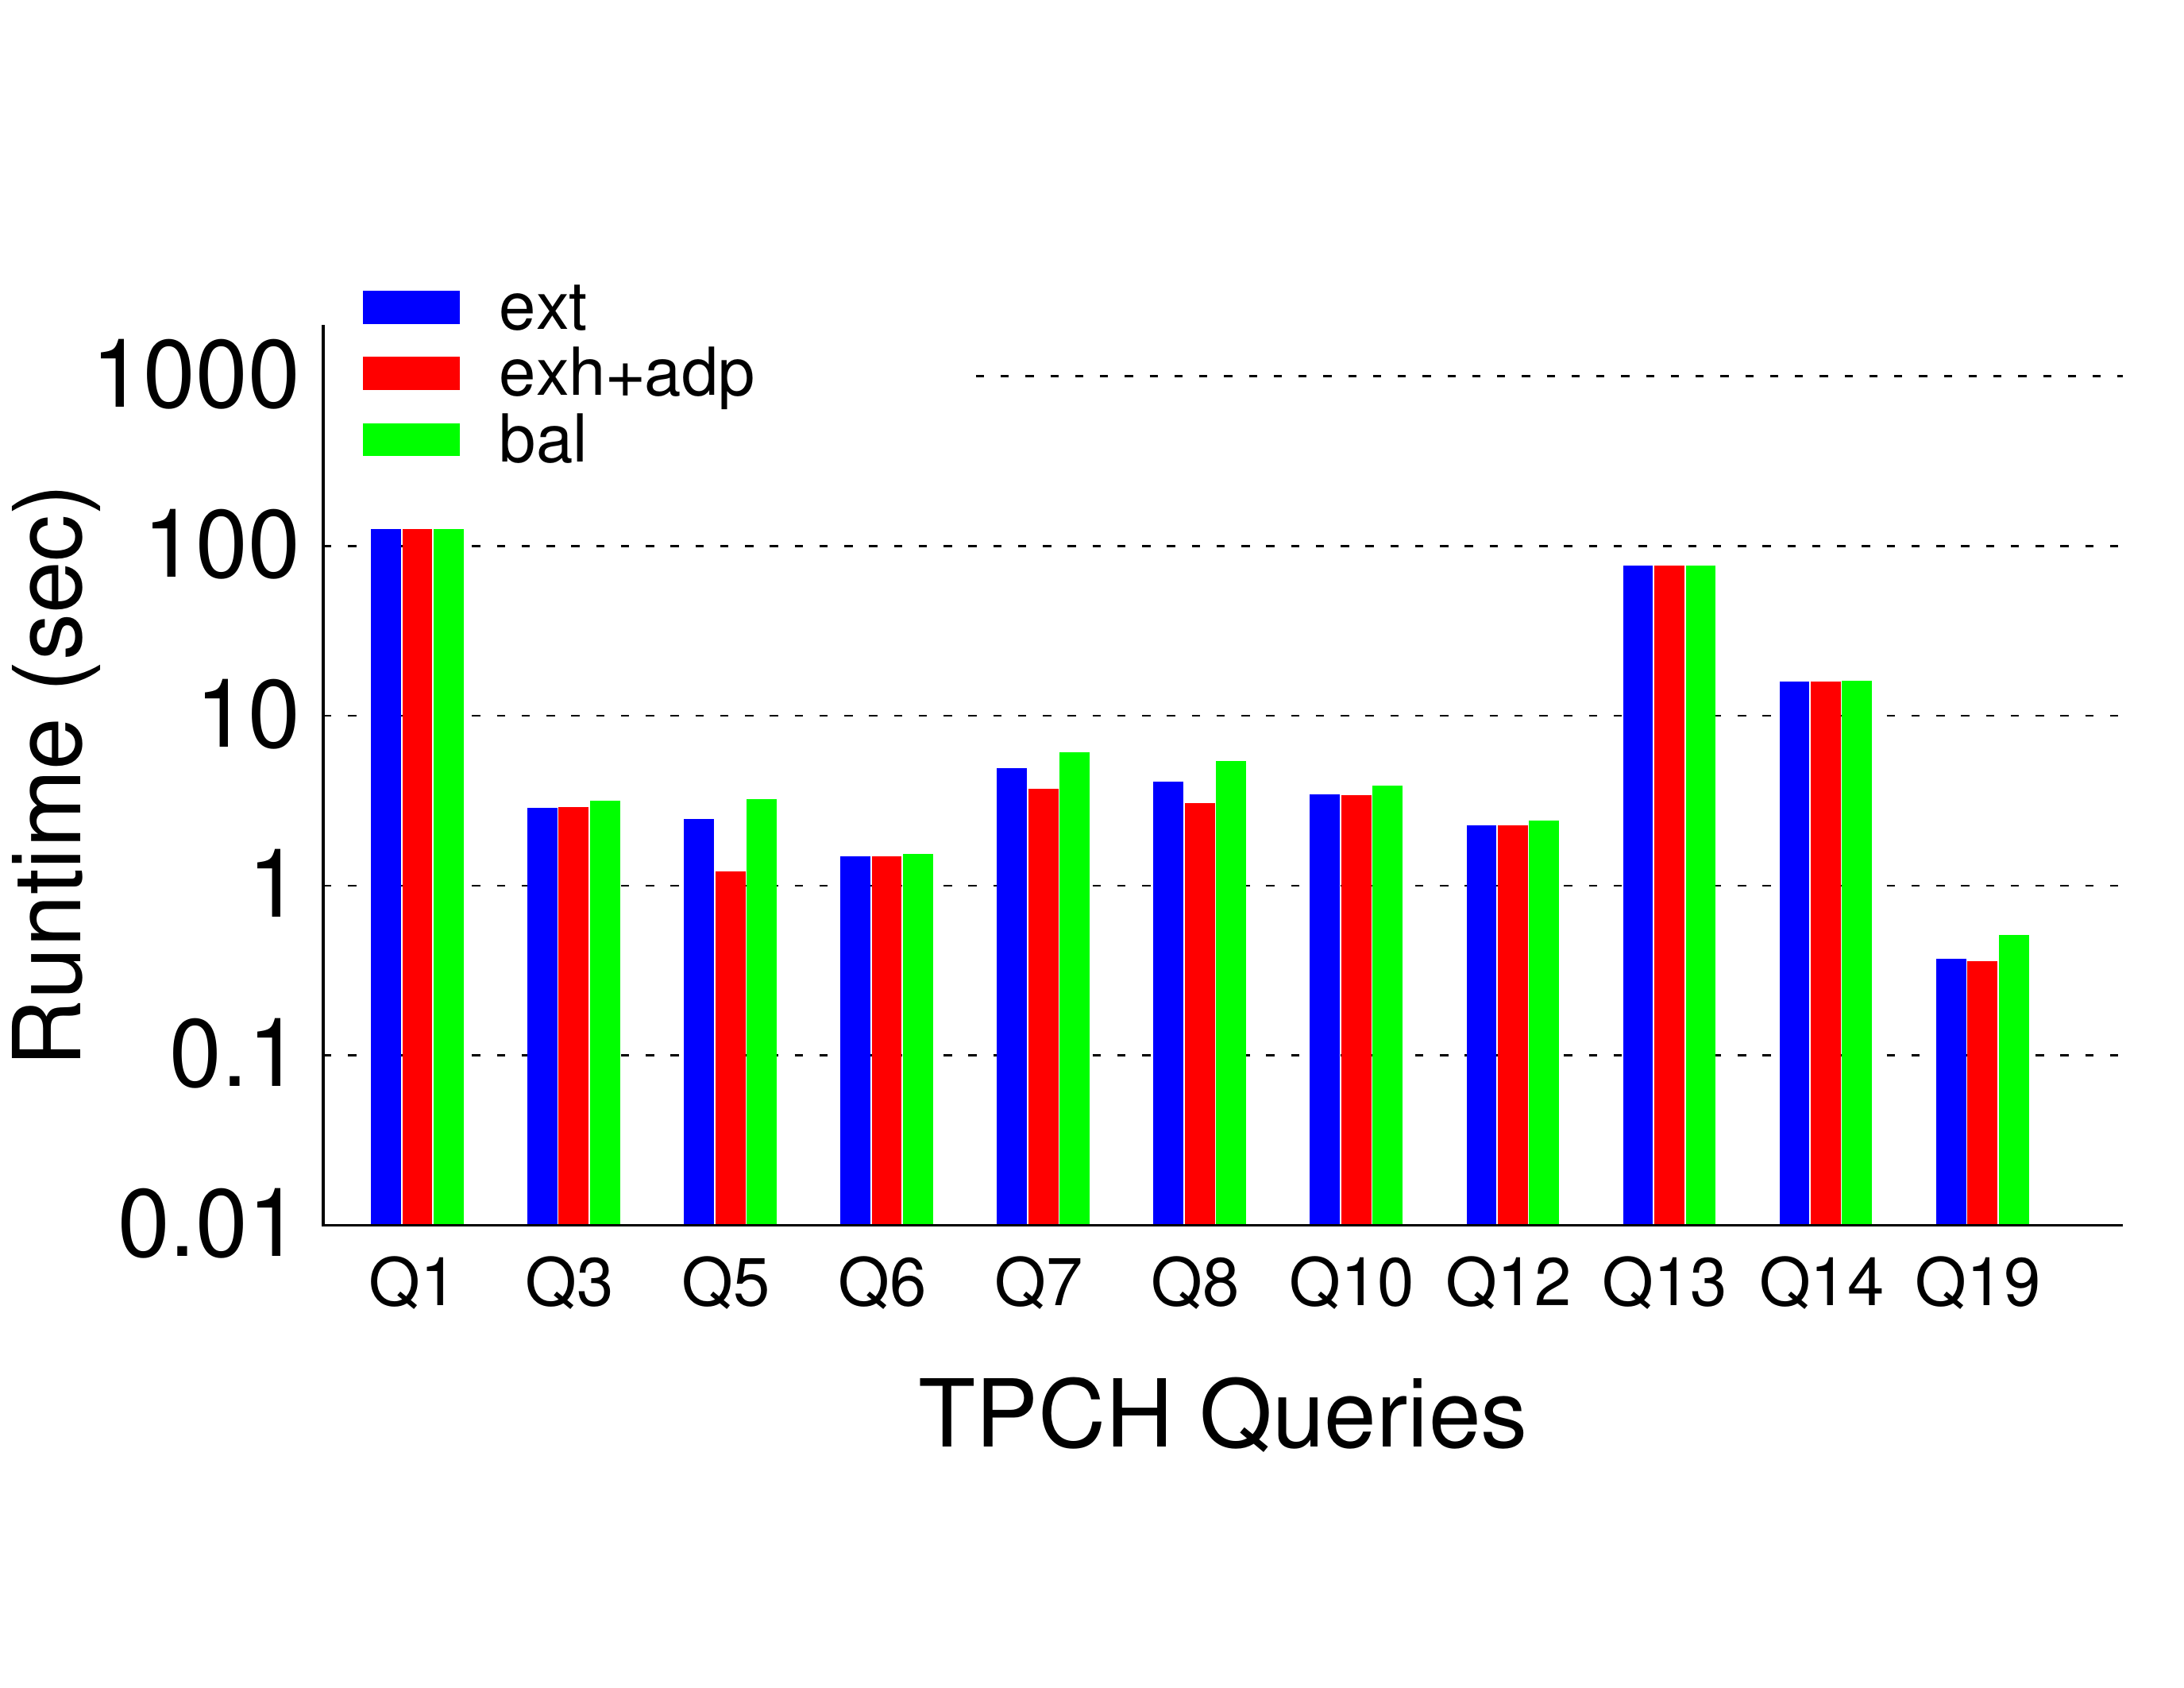}\\[-7mm]
  \caption{TPC-H.  Runtime + Overhead - 1GB}
  \label{fig:tpch-runtime-overhead-sty}  
  \end{minipage}
%%%%%%%%%%%%%%%%%%%
  \begin{minipage}[b]{0.49\linewidth}
  \includegraphics[width=1\linewidth,trim=0 50pt 0 100pt, clip]{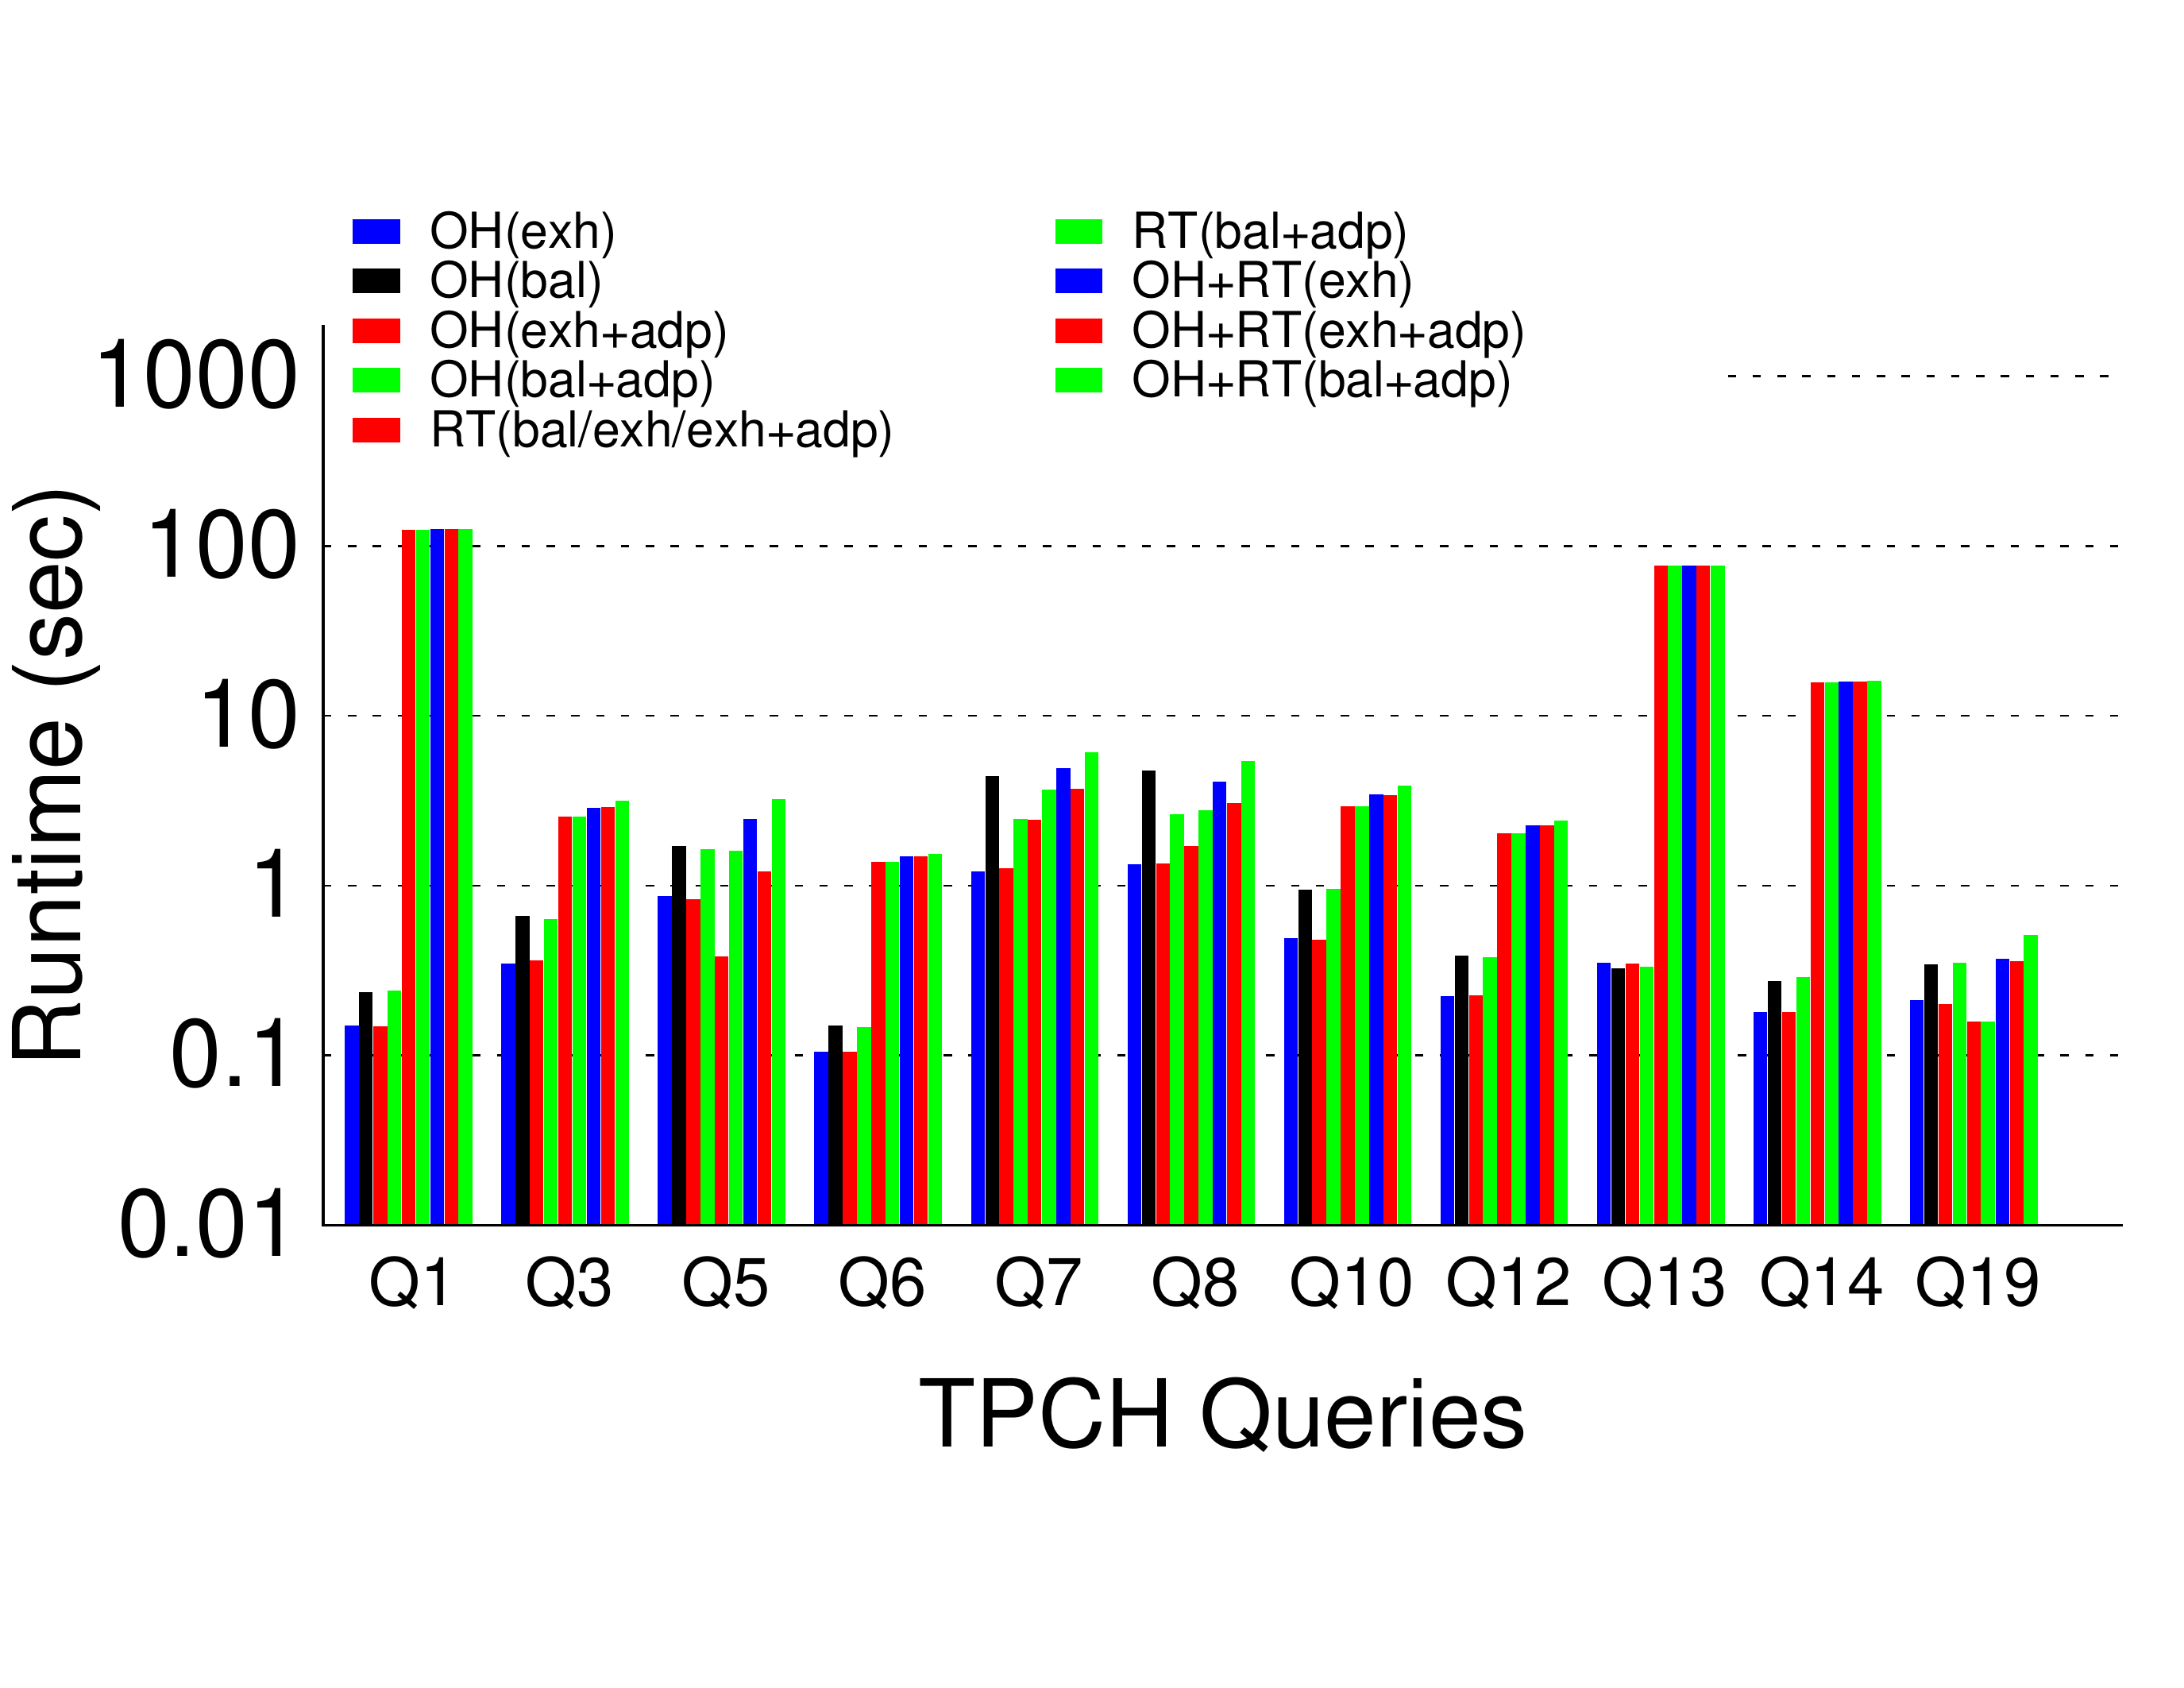}\\[-7mm] 
  \caption{TPC-H.  All - 1GB}
  \label{fig:tpch-all-sty}
  \end{minipage}
\end{figure*}
% %%%%%%%%%%%%%%%%%%%%%%%%%%%%%%%%%%%%%%%%%%%%%%%%%%%%%%%%%%%%

%%%%%%%%%%%%%%%%%%%%%%%%%%%%%%%%%%%%%%%%%%%%%%%%%%%%%%%%%%%%
\begin{figure*}[t]
%%%%%%%%%%%%%%%%%%%%
  \begin{minipage}[b]{0.49\linewidth}
  \includegraphics[width=1\linewidth,trim=0 80pt 0 100pt, clip]{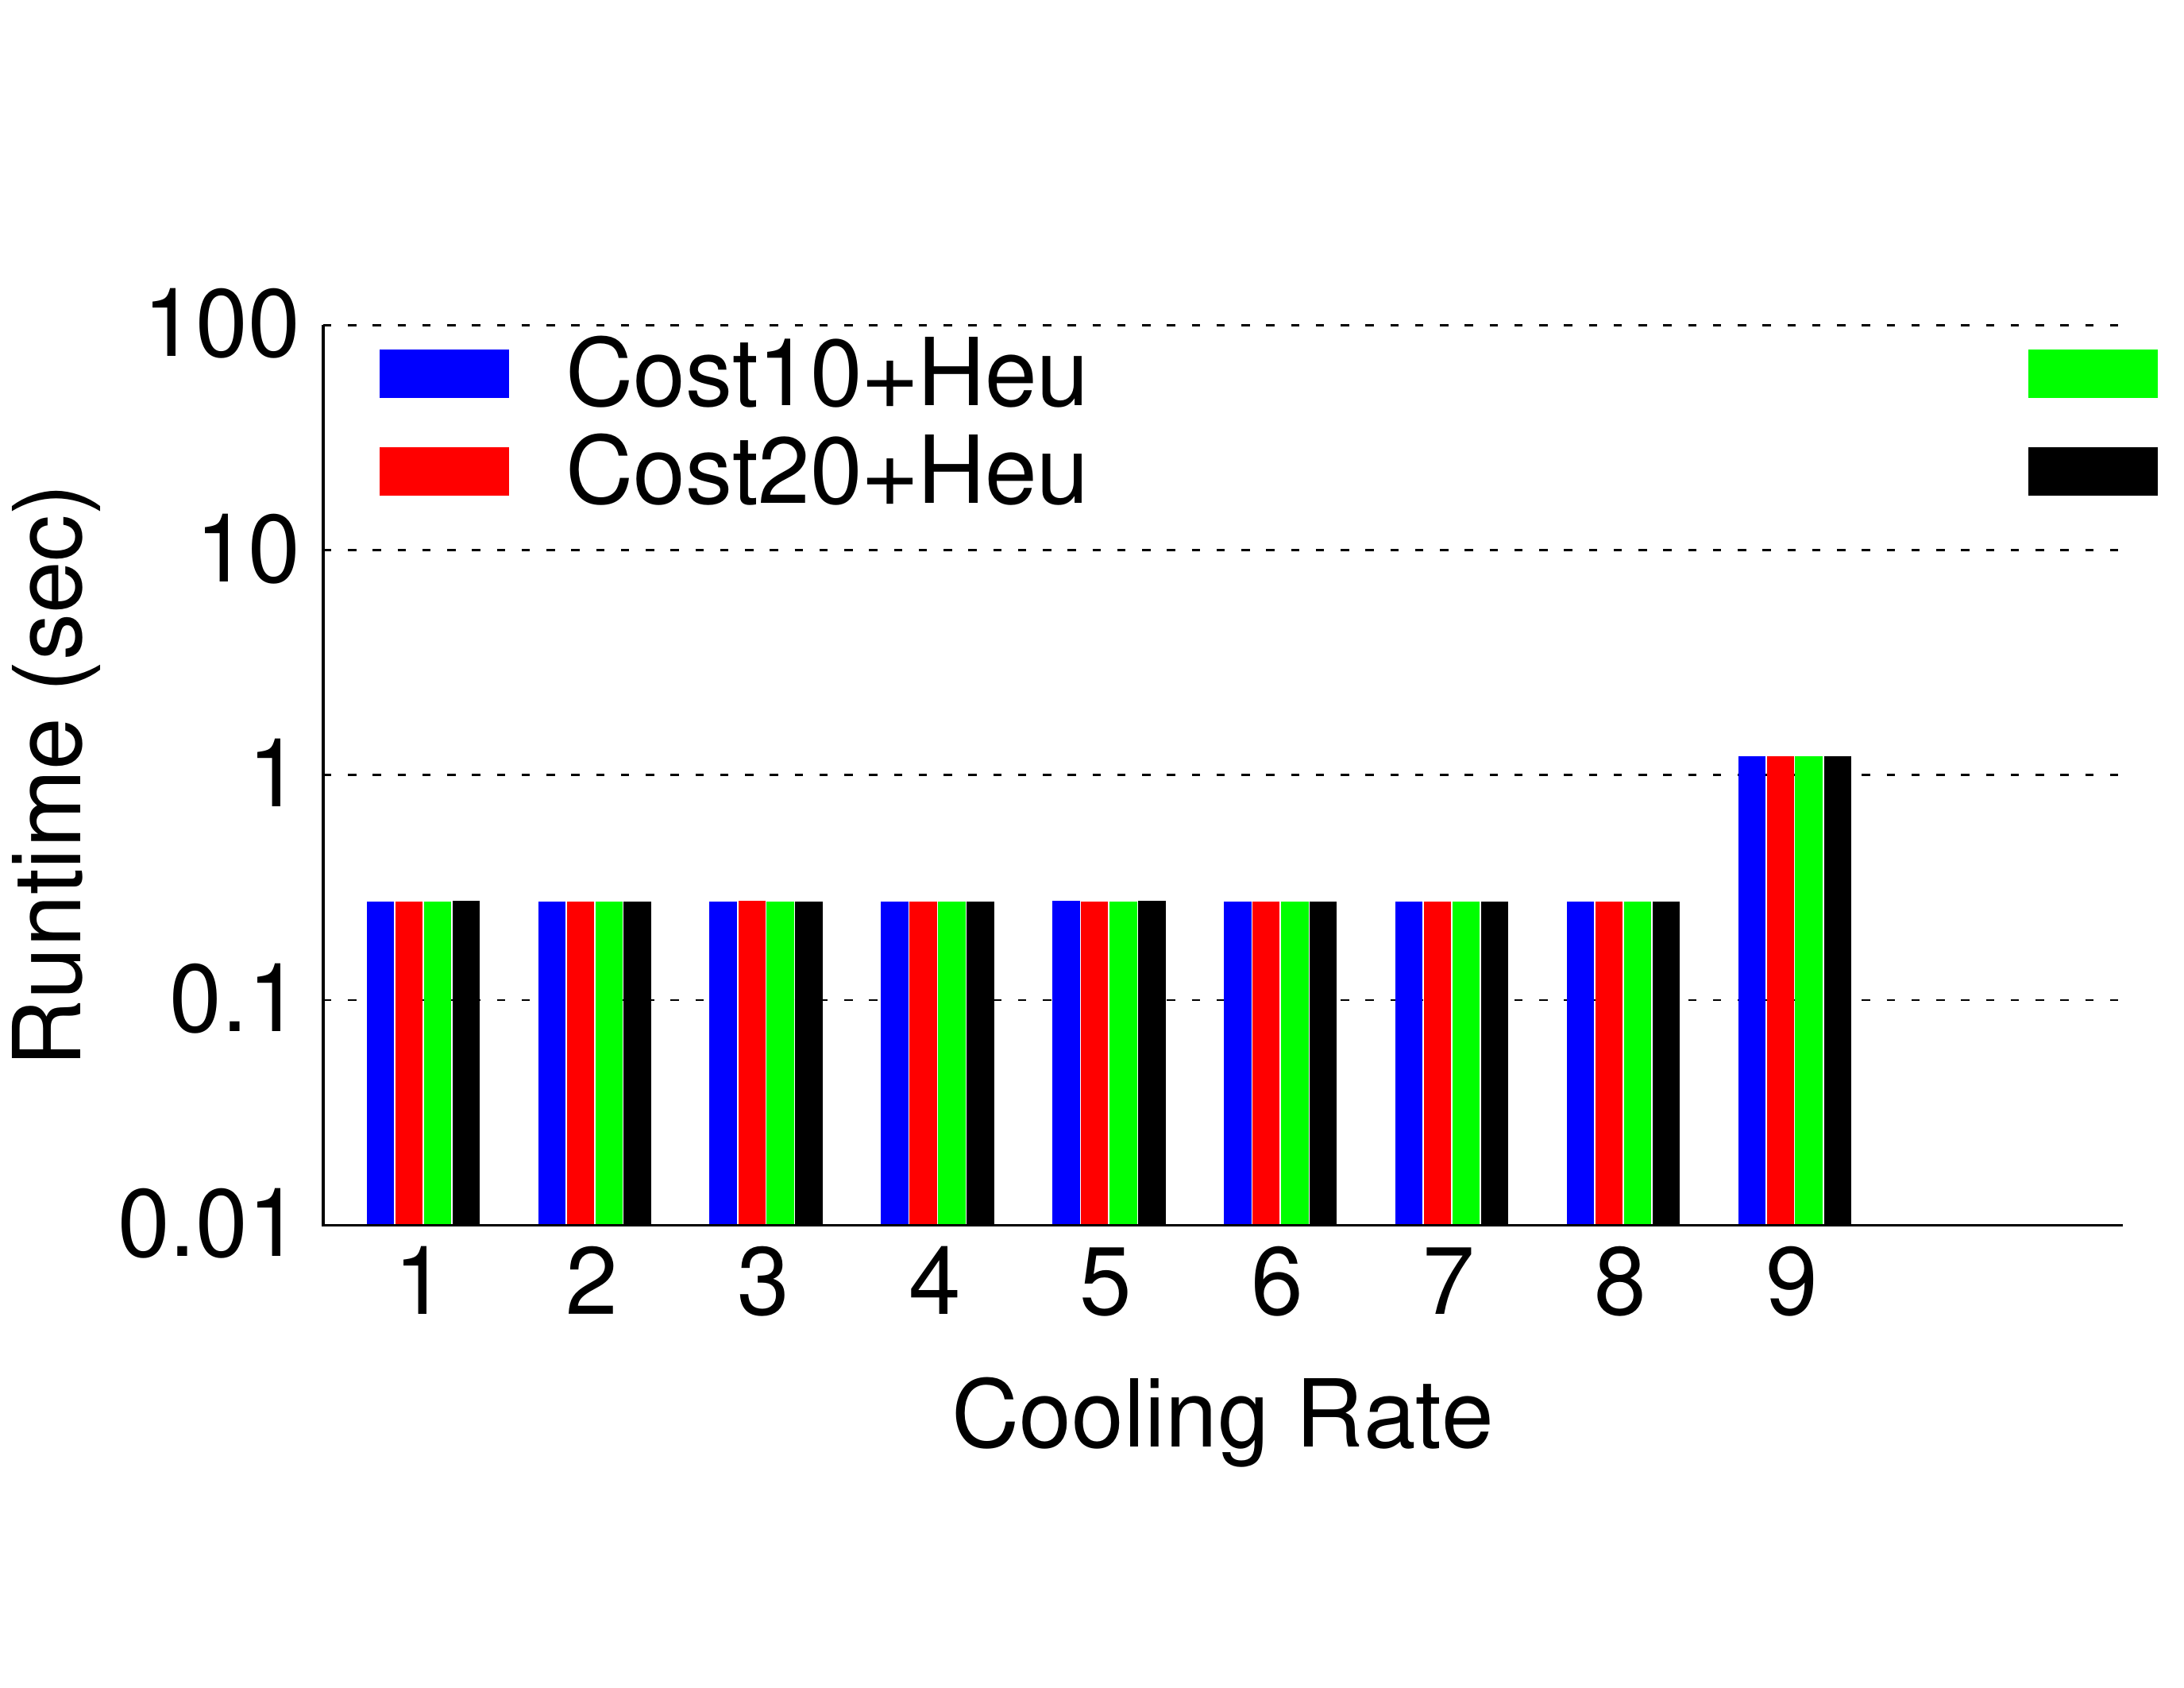}\\[-7mm]
  \caption{Simulate Annealing - Simple Agg 10. - 1GB}
  \label{fig:sim-simple-agg}  
  \end{minipage}
%%%%%%%%%%%%%%%%%%%
  \begin{minipage}[b]{0.49\linewidth}
 % \includegraphics[width=1\linewidth,trim=0 80pt 0 100pt, clip]{figs/experiments_v2/%bal_adp_simpleAgg_together_1GB.pdf}\\[-7mm] 
 % \caption{Balance Simple Agg.  Runtime + Overhead - 1GB}
%  \label{fig:bal-simple-agg-runtime-overhead}
  \end{minipage}
\end{figure*}
% %%%%%%%%%%%%%%%%%%%%%%%%%%%%%%%%%%%%%%%%%%%%%%%%%%%%%%%%%%%%

%\multicolumn{3}{>{\columncolor{red}}l}{\color{white}\textsf{LONDON}}
%%%%%%%%%%%%%%%%%%%%%%%%%%%%%%%%%%%%%%%%
\begin{table*}
\centering
  \begin{tabular}{|c|c|c|c|c|c|c|c|c|c|} \hline 
%     & \cellcolor[gray]{.9} Overhead &	\cellcolor[gray]{.9}Overhead & \cellcolor[gray]{.9}Overhead	& Overhead &	\cellcolor{yellow}Runtime	& Runtime &	O+R & O+R &	O+R \\ \hline 

 & \multicolumn{4}{>{\columncolor{red}}l}{\color{black}\textsf{Overhead}}  &	\multicolumn{2}{>{\columncolor{yellow}}l}{\color{black}\textsf{Runtime}} &	\multicolumn{3}{>{\columncolor{green}}l}{\color{black}\textsf{Overhead + Runtime}} \\ \hline 

\rowcolor[gray]{.9}  Queries & exh &	bal & exh+adp	& bal+adp &	bal/exh/exh+adp	& bal+adp &	exh & exh+adp &	bal+adp \\ \hline 
Q1 & 0.14875	& 0.235 & 0.1475 & 0.23925	& 124.7783447 & 124.7783447 & 124.9270947 & 124.9258447 &	125.0175947 \\ \hline
Q3 & 0.345 & 0.66 & 0.36	& 0.63	& 2.5248366 & 2.5248366 & 2.8698366	 & 2.8848366	& 3.1548366 \\ \hline
Q5 & 0.8625 & \cellcolor{green}1.706	& 0.83	& \cellcolor{green}1.64	& \cellcolor{yellow}0.38086142 &	\cellcolor{yellow}1.59660617 & 2.45910617 & 1.21086142	& 3.23660617 \\ \hline
Q6 & 0.105 &	0.149 & 0.10425 &  0.146 & 1.3802 & 1.3802 & 1.4852 & 1.48445	& 1.5262 \\ \hline
Q7 & 1.2115 & \cellcolor{green}4.3792 & 1.26 & \cellcolor{green}2.45 & \cellcolor{yellow}2.4452237 & \cellcolor{yellow}3.66511	& 4.87661 & 3.7052237 & 6.11511 \\ \hline
Q8 & 1.335	& \cellcolor{green}4.7635	& 1.3466	& \cellcolor{green}2.62	 & \cellcolor{yellow}1.6975495	& \cellcolor{yellow}2.7661241 & 4.1011241 & 3.0441495	& 5.3861241 \\ \hline
Q10 &	0.49	& 0.9415	 & 0.48 & 0.955 & 2.93360137 & 2.93360137 & 3.42360137 & 3.41360137 & 3.88860137 \\ \hline
Q12	& 0.22325 & 0.38675 & 0.225 & 0.38 & 2.0365688 & 2.0365688	& 2.2598188	& 2.2615688	& 2.4165688 \\ \hline
Q13	& 0.35	& 0.325 & 0.345 &	0.33	 & 76.243654	& 76.243654	& 76.593654	& 76.588654	& 76.573654 \\ \hline
Q14	& 0.18	& 0.273 & 0.18 & 0.29 & 15.70571533 & 15.70571533 & 15.88571533 & 15.88571533 &	15.99571533 \\ \hline
Q19	& 0.21	& 0.342 & 0.2 & 0.35 & 0.15767973	 & 0.15767973 & 0.36767973 & 0.35767973 & 0.50767973 \\ \hline
  \end{tabular}
\caption{TPC-H ALL}
\label{tab:tpch-all}

\end{table*}
%%%%%%%%%%%%%%%%%%%%%%%%%%%%%%%%%%%%%%%%

%%%%%%%%%%%%%%%%%%%%%%%%%%%%%%%%%%%%%%%%
\begin{table*}
\centering
  \begin{tabular}{|c|c|c|c|c|c|c|c|c|c|c|} \hline 
%     & \cellcolor[gray]{.9} Overhead &	\cellcolor[gray]{.9}Overhead & \cellcolor[gray]{.9}Overhead	& Overhead &	\cellcolor{yellow}Runtime	& Runtime &	O+R & O+R &	O+R \\ \hline 

 & \multicolumn{4}{>{\columncolor{red}}l}{\color{black}\textsf{Overhead}}  &	\multicolumn{3}{>{\columncolor{yellow}}l}{\color{black}\textsf{Runtime}} &	\multicolumn{3}{>{\columncolor{green}}l}{\color{black}\textsf{Overhead + Runtime}} \\ \hline 

\rowcolor[gray]{.9}  Queries & exh &	bal & exh+adp	& bal+adp &	bal/exh &	exh+adp  & bal+adp &	exh & exh+adp &	bal+adp \\ \hline 

1	& 0.08233 & 0.1&	0.08	&0.07966	&0.079961&	0.07126722	&0.07112027	&0.162291	&0.15126722&	0.15078027 \\ \hline 
2	&0.144	&0.149	&0.086	&0.085666&	0.076372&	0.08188944	&0.08157216	&0.220372	&0.16788944	& 0.16723816 \\ \hline 
3	&0.84833	&0.857	&0.115	&0.117&	0.088315	&2.96413497	&3.02005419	&\cellcolor{red}0.936645	&3.07913497	&3.13705419 \\ \hline 
4	&0.857	&0.776	&0.108	&0.109666	&0.078026	&0.70939694	&0.71094147	&0.935026	&0.81739694&	0.82060747 \\ \hline 
5	&5.095333	&4.889&	0.34466	&0.298	&0.079977	&2.85248187	&\cellcolor{green}2.5519704	&5.17531	&3.19714187	&2.8499704 \\ \hline 
6	&5.40233	&6.809	&0.42	&0.308333333	&0.07905	&\cellcolor{green}0.38856532	&1.68378421	&5.48138	&0.80856532&	1.992117543 \\ \hline 
7	&35.5	&35.662	&\cellcolor{yellow}1.653&	0.5	&0.080604&	\cellcolor{green}0.97281275	&3.64682914	&35.580604	&2.62581275	&4.14682914 \\ \hline 
8	&36.245&	35.43	&\cellcolor{yellow}2.965333	&0.53&	0.083664	&\cellcolor{green}0.28467627	&1.86783809	&36.328664&	3.25000927&	2.39783809 \\ \hline 
9	&239.7533	&246.8	&0.40333	&0.404	&0.084048	&4.77865129&	4.77460661	&239.837348	&5.18198129&	5.17860661 \\ \hline 
10	&257.67	&238.93	&0.76	&1.18	&0.084748	&1.19884658	&\cellcolor{green}0.43721765	&257.754748	&1.95884658	&1.61721765 \\ \hline 
  \end{tabular}
\caption{simpleAgg ALL}
\label{tab:simple-agg-all}

\end{table*}
%%%%%%%%%%%%%%%%%%%%%%%%%%%%%%%%%%%%%%%%

\begin{figure*}[t]
%%%%%%%%%%%%%%%%%%%% 
  \begin{minipage}[b]{0.24\linewidth}
\includegraphics[width=1\linewidth,trim=0 10pt 0 30pt, clip]{figs/experiments_v1/uSizeNumTupUpdated.pdf}\\
  \vspace{-4mm}
  %\caption{Updates/Transaction and History Size}
  %\label{fig:Updates/Transaction-and-History-Size}
  \end{minipage}
  %%%%%%%%%%%%%%%%%%%%
  \begin{minipage}[b]{0.24\linewidth}
\includegraphics[width=1\linewidth,trim=0 20pt 0 30pt, clip]{figs/experiments_v1/numTupUpdated.pdf}\\
  \vspace{-4mm}
  %\caption{Number Updates/Transaction}
  %\label{fig:Number-Updates/Transaction}
  \end{minipage}
  %%%%%%%%%%%%%%%%%%%% 
%%%%%%%%%%%%%%%%%%% 
  \begin{minipage}[b]{0.24\linewidth}
\includegraphics[width=1\linewidth,trim=0 20pt 0 30pt, clip]{figs/experiments_v1/uSizeNumTupUpdated_overhead.pdf}\\
  \vspace{-4mm}
  %\caption{TransactionOverhead1}
  %\label{fig:Transaction Overhead: Updates/Transaction and History Size}
  \end{minipage}
  %%%%%%%%%%%%%%%%%%%%
  \begin{minipage}[b]{0.24\linewidth}
\includegraphics[width=1\linewidth,trim=0 20pt 0 30pt, clip]{figs/experiments_v1/numTupUpdated_overhead.pdf}\\
  \vspace{-4mm}
  %\caption{TransactionOverhead2}
  %\label{fig:Transaction Overhead Number Updates/Transaction}
  \end{minipage}

  \caption{Transaction provenance}
  \label{fig:Transaction provenance}
\end{figure*}
%%%%%%%%%%%%%%%%%%%%
%%%%%%%%%%%%%%%%%%%%%%%%%%%%%%%%%%%%%%%%%%%%%%%%%%%%%%%%%%%%
%\begin{figure}[t]

%%% Local Variables:
%%% mode: latex
%%% TeX-master: "2016-prov-optimizer"
%%% End:
